# Supplementary material for: Systematic construction of spin liquids on the square lattice from tensor networks with SU(2) symmetry
Source: arXiv:1608.06003 ancillary file (2016-11-15)
Supplement: Supplementary file 1 [file Classification.pdf]

**SU(2)-symmetric translationally and rotationally-invariant  
Projected Entangled Pair States (PEPS) with bond dimension  $D \leq 6$**

$$\mathbf{S} = \mathbf{2}, \mathbf{n}_{\text{occ.}} = \{4\}$$

$$\left( \begin{array}{cccccc} \text{State} & 1 & 2 & 3 & 4 & 5 \\ \text{Sz} & 2 & 1 & 0 & -1 & -2 \\ \text{Rx} & 1 & 1 & 1 & 1 & 1 \\ \text{Ry} & 1 & 1 & 1 & 1 & 1 \\ \text{R} & 1 & 1 & 1 & 1 & 1 \\ \text{Landau} & \text{A1} & \text{A1} & \text{A1} & \text{A1} & \text{A1} \end{array} \right)$$

$$S = 1, \text{ n}_{\text{occ.}} = \{4\}$$

$$\left( \begin{array}{cccccccccc} \text{State} & 6 & 7 & 8 & 9 & 10 & 11 & 12 & 13 & 14 \\ \text{Sz} & 1 & 0 & -1 & 1 & 0 & -1 & 1 & 0 & -1 \\ \text{Rx} & 1 & 1 & 1 & 0 & 0 & 0 & 0 & 0 & 0 \\ \text{Ry} & 1 & 1 & 1 & 0 & 0 & 0 & 0 & 0 & 0 \\ \text{R} & -1 & -1 & -1 & i & i & i & -i & -i & -i \\ \text{Landau} & \text{B1} & \text{B1} & \text{B1} & \text{E} & \text{E} & \text{E} & \text{E} & \text{E} & \text{E} \end{array} \right)$$

$$\mathbf{S} = \mathbf{0}, \text{ n}_{\text{occ.}} = \{4\}$$

$$\left( \begin{array}{ccc} \text{State} & 15 & 16 \\ \text{Sz} & 0 & 0 \\ \text{Rx} & 1 & -1 \\ \text{Ry} & 1 & -1 \\ \text{R} & 1 & -1 \\ \text{Landau} & \text{A1} & \text{B2} \end{array} \right)$$

$$S = 4, \mathbf{n}_{\text{occ.}} = \{4\}$$

[illegible]

$$\mathbf{S} = \mathbf{3}, \mathbf{n}_{\text{occ.}} = \{4\}$$

[illegible]

$$S = 2, \text{ n}_{\text{occ.}} = \{4\}$$

| State  | 31 | 32 | 33 | 34 | 35 | 36 | 37 | 38 | 39 | 40 | 41 | 42 | 43 | 44 | 45 | 46 | 47  | 48  | 49  | 50  | 51  | 52   | 53   | 54   | 55   | 56   | 57 | 58 | 59 | 60 |
|--------|----|----|----|----|----|----|----|----|----|----|----|----|----|----|----|----|-----|-----|-----|-----|-----|------|------|------|------|------|----|----|----|----|
| Sz     | 2  | 1  | 0  | -1 | -2 | 2  | 1  | 0  | -1 | -2 | 2  | 1  | 0  | -1 | -2 | 2  | 1   | 0   | -1  | -2  | 2   | 1    | 0    | -1   | -2   | 2    | 1  | 0  | -1 | -2 |
| Rx     | 1  | 1  | 1  | 1  | 1  | 1  | 1  | 1  | 1  | 1  | 1  | 1  | 1  | 1  | 1  | 0  | 0   | 0   | 0   | 0   | 0   | 0    | 0    | 0    | 0    | 0    | -1 | -1 | -1 | -1 |
| Ry     | 1  | 1  | 1  | 1  | 1  | 1  | 1  | 1  | 1  | 1  | 1  | 1  | 1  | 1  | 1  | 0  | 0   | 0   | 0   | 0   | 0   | 0    | 0    | 0    | 0    | 0    | -1 | -1 | -1 | -1 |
| R      | 1  | 1  | 1  | 1  | 1  | 1  | 1  | 1  | 1  | 1  | 1  | -1 | -1 | -1 | -1 | -1 | $i$ | $i$ | $i$ | $i$ | $i$ | $-i$ | $-i$ | $-i$ | $-i$ | $-i$ | -1 | -1 | -1 | -1 |
| Landau | A1 | A1 | A1 | A1 | A1 | A1 | A1 | A1 | A1 | A1 | B1 | B1 | B1 | B1 | B1 | E  | E   | E   | E   | E   | E   | E    | E    | E    | E    | E    | B2 | B2 | B2 | B2 |

$$\mathbf{S} = \mathbf{1}, \mathbf{n}_{\text{occ.}} = \{4\}$$

$$\left( \begin{array}{c|cccccccccccccccccccc} \text{State} & 61 & 62 & 63 & 64 & 65 & 66 & 67 & 68 & 69 & 70 & 71 & 72 & 73 & 74 & 75 & 76 & 77 & 78 \\ \hline \text{Sz} & 1 & 0 & -1 & 1 & 0 & -1 & 1 & 0 & -1 & 1 & 0 & -1 & 1 & 0 & -1 & 1 & 0 & -1 \\ \text{Rx} & 1 & 1 & 1 & 0 & 0 & 0 & 0 & 0 & 0 & 0 & 0 & 0 & 0 & 0 & 0 & -1 & -1 & -1 \\ \text{Ry} & 1 & 1 & 1 & 0 & 0 & 0 & 0 & 0 & 0 & 0 & 0 & 0 & 0 & 0 & 0 & -1 & -1 & -1 \\ \text{R} & -1 & -1 & -1 & i & i & i & i & i & i & -i & -i & -i & -i & -i & -i & 1 & 1 & 1 \\ \text{Landau} & \text{B1} & \text{B1} & \text{B1} & \text{E} & \text{E} & \text{E} & \text{E} & \text{E} & \text{E} & \text{E} & \text{E} & \text{E} & \text{E} & \text{E} & \text{E} & \text{A2} & \text{A2} & \text{A2} \end{array} \right)$$



$$\mathbf{S} = \mathbf{0}, \text{ n}_{\text{occ.}} = \{4\}$$

$$\left( \begin{array}{cccc} \text{State} & 79 & 80 & 81 \\ \text{Sz} & 0 & 0 & 0 \\ \text{Rx} & 1 & 1 & -1 \\ \text{Ry} & 1 & 1 & -1 \\ \text{R} & 1 & 1 & -1 \\ \text{Landau} & \text{A1} & \text{A1} & \text{B2} \end{array} \right)$$

$$\mathbf{S} = \mathbf{2}, \mathbf{n}_{\text{occ.}} = \{4, \mathbf{0}\}$$

$$\left( \begin{array}{ccccc} \text{State} & 1 & 2 & 3 & 4 & 5 \\ \text{Sz} & 2 & 1 & 0 & -1 & -2 \\ \text{Rx} & 1 & 1 & 1 & 1 & 1 \\ \text{Ry} & 1 & 1 & 1 & 1 & 1 \\ \text{R} & 1 & 1 & 1 & 1 & 1 \\ \text{Landau} & \text{A1} & \text{A1} & \text{A1} & \text{A1} & \text{A1} \end{array} \right)$$





$$\mathbf{S} = \mathbf{1}, \mathbf{n}_{\text{occ.}} = \{\mathbf{2}, \mathbf{2}\}$$

$$\left( \begin{array}{c|cccccccccccccccccccc} \text{State} & 31 & 32 & 33 & 34 & 35 & 36 & 37 & 38 & 39 & 40 & 41 & 42 & 43 & 44 & 45 & 46 & 47 & 48 \\ \hline \text{Sz} & 1 & 0 & -1 & 1 & 0 & -1 & 1 & 0 & -1 & 1 & 0 & -1 & 1 & 0 & -1 & 1 & 0 & -1 \\ \text{Rx} & 1 & 1 & 1 & 1 & 1 & 1 & 1 & 1 & 1 & 0 & 0 & 0 & 0 & 0 & 0 & -1 & -1 & -1 \\ \text{Ry} & 1 & 1 & 1 & 1 & 1 & 1 & 1 & 1 & 1 & 0 & 0 & 0 & 0 & 0 & 0 & -1 & -1 & -1 \\ \text{R} & 1 & 1 & 1 & 1 & 1 & 1 & -1 & -1 & -1 & i & i & i & -i & -i & -i & -1 & -1 & -1 \\ \text{Landau} & \text{A1} & \text{A1} & \text{A1} & \text{A1} & \text{A1} & \text{A1} & \text{B1} & \text{B1} & \text{B1} & \text{E} & \text{E} & \text{E} & \text{E} & \text{E} & \text{E} & \text{B2} & \text{B2} & \text{B2} \end{array} \right)$$

$$\mathbf{S} = \mathbf{1}/\mathbf{2}, \text{ n}_{\text{occ.}} = \{\mathbf{3}, \mathbf{1}\}$$

| State  | 49            | 50             | 51            | 52             | 53            | 54             | 55            | 56             | 57            | 58             | 59            | 60             | 61            | 62             | 63            | 64             |
|--------|---------------|----------------|---------------|----------------|---------------|----------------|---------------|----------------|---------------|----------------|---------------|----------------|---------------|----------------|---------------|----------------|
| Sz     | $\frac{1}{2}$ | $-\frac{1}{2}$ | $\frac{1}{2}$ | $-\frac{1}{2}$ | $\frac{1}{2}$ | $-\frac{1}{2}$ | $\frac{1}{2}$ | $-\frac{1}{2}$ | $\frac{1}{2}$ | $-\frac{1}{2}$ | $\frac{1}{2}$ | $-\frac{1}{2}$ | $\frac{1}{2}$ | $-\frac{1}{2}$ | $\frac{1}{2}$ | $-\frac{1}{2}$ |
| Rx     | 1             | 1              | 1             | 1              | 0             | 0              | 0             | 0              | 0             | 0              | 0             | 0              | -1            | -1             | -1            | -1             |
| Ry     | 1             | 1              | 1             | 1              | 0             | 0              | 0             | 0              | 0             | 0              | 0             | 0              | -1            | -1             | -1            | -1             |
| R      | 1             | 1              | -1            | -1             | $i$           | $i$            | $i$           | $i$            | $-i$          | $-i$           | $-i$          | $-i$           | 1             | 1              | -1            | -1             |
| Landau | A1            | A1             | B1            | B1             | E             | E              | E             | E              | E             | E              | E             | E              | A2            | A2             | B2            | B2             |

$$\mathbf{S} = \mathbf{1}/\mathbf{2}, \text{ n}_{\text{occ.}} = \{\mathbf{1}, \mathbf{3}\}$$

$$\left( \begin{array}{cccccccccc} \text{State} & 65 & 66 & 67 & 68 & 69 & 70 & 71 & 72 \\ \text{Sz} & \frac{1}{2} & -\frac{1}{2} & \frac{1}{2} & -\frac{1}{2} & \frac{1}{2} & -\frac{1}{2} & \frac{1}{2} & -\frac{1}{2} \\ \text{Rx} & 1 & 1 & 1 & 1 & 0 & 0 & 0 & 0 \\ \text{Ry} & 1 & 1 & 1 & 1 & 0 & 0 & 0 & 0 \\ \text{R} & 1 & 1 & -1 & -1 & i & i & -i & -i \\ \text{Landau} & \text{A1} & \text{A1} & \text{B1} & \text{B1} & \text{E} & \text{E} & \text{E} & \text{E} \end{array} \right)$$

$$\mathbf{S} = \mathbf{0}, \text{ n}_{\text{occ.}} = \{4, 0\}$$

$$\left( \begin{array}{ccc} \text{State} & 73 & 74 \\ \text{Sz} & 0 & 0 \\ \text{Rx} & 1 & -1 \\ \text{Ry} & 1 & -1 \\ \text{R} & 1 & -1 \\ \text{Landau} & \text{A1} & \text{B2} \end{array} \right)$$



$$\mathbf{S} = \mathbf{0}, \mathbf{n}_{\text{occ.}} = \{\mathbf{2}, \mathbf{2}\}$$

$$\left( \begin{array}{cccccc} \text{State} & 75 & 76 & 77 & 78 & 79 & 80 \\ \text{Sz} & 0 & 0 & 0 & 0 & 0 & 0 \\ \text{Rx} & 1 & 0 & 0 & 0 & 0 & -1 \\ \text{Ry} & 1 & 0 & 0 & 0 & 0 & -1 \\ \text{R} & -1 & i & i & -i & -i & 1 \\ \text{Landau} & \text{B1} & \text{E} & \text{E} & \text{E} & \text{E} & \text{A2} \end{array} \right)$$

$$\mathbf{S} = \mathbf{0}, \text{ n}_{\text{occ.}} = \{0, 4\}$$

$$\left( \begin{array}{cc} \text{State} & 81 \\ \text{Sz} & 0 \\ \text{Rx} & 1 \\ \text{Ry} & 1 \\ \text{R} & 1 \\ \text{Landau} & \text{A1} \end{array} \right)$$

$$S = 6, \text{ n}_{\text{occ.}} = \{4\}$$

[illegible]

[illegible]

$$S = 4, \mathbf{n}_{\text{occ.}} = \{4\}$$

[illegible]

$$\mathbf{S} = \mathbf{3}, \mathbf{n}_{\text{occ.}} = \{4\}$$

$$\left( \begin{array}{cccc} \text{State} & 101 & 102 & 103 \\ \text{Sz} & 3 & 2 & 1 \\ \text{Rx} & 1 & 1 & 1 \\ \text{Ry} & 1 & 1 & 1 \\ \text{R} & 1 & 1 & 1 \\ \text{Landau} & \text{A1} & \text{A1} & \text{A1} \end{array} \right)$$



$$S = 1, \text{ n}_{\text{occ.}} = \{4\}$$

[illegible]



$$\mathbf{S} = \mathbf{0}, \text{ n}_{\text{occ.}} = \{4\}$$

$$\left( \begin{array}{ccccc} \text{State} & 253 & 254 & 255 & 256 \\ \text{Sz} & 0 & 0 & 0 & 0 \\ \text{Rx} & 1 & 1 & -1 & -1 \\ \text{Ry} & 1 & 1 & -1 & -1 \\ \text{R} & 1 & 1 & -1 & -1 \\ \text{Landau} & \text{A1} & \text{A1} & \text{B2} & \text{B2} \end{array} \right)$$





$$\mathbf{S} = \mathbf{3}, \mathbf{n}_{\text{occ.}} = \{\mathbf{3}, \mathbf{1}\}$$

[illegible]

$$\mathbf{S} = \mathbf{2}, \mathbf{n}_{\text{occ.}} = \{4, \mathbf{0}\}$$

| State  | 59 | 60 | 61 | 62 | 63 | 64 | 65 | 66 | 67 | 68 | 69 | 70 | 71 | 72 | 73 | 74  | 75  | 76  | 77  | 78  | 79   | 80   | 81   | 82   | 83   | 84 | 85 | 86 | 87 | 88 |
|--------|----|----|----|----|----|----|----|----|----|----|----|----|----|----|----|-----|-----|-----|-----|-----|------|------|------|------|------|----|----|----|----|----|
| Sz     | 2  | 1  | 0  | -1 | -2 | 2  | 1  | 0  | -1 | -2 | 2  | 1  | 0  | -1 | -2 | 2   | 1   | 0   | -1  | -2  | 2    | 1    | 0    | -1   | -2   | 2  | 1  | 0  | -1 | -2 |
| Rx     | 1  | 1  | 1  | 1  | 1  | 1  | 1  | 1  | 1  | 1  | 1  | 1  | 1  | 1  | 1  | 0   | 0   | 0   | 0   | 0   | 0    | 0    | 0    | 0    | 0    | -1 | -1 | -1 | -1 | -1 |
| Ry     | 1  | 1  | 1  | 1  | 1  | 1  | 1  | 1  | 1  | 1  | 1  | 1  | 1  | 1  | 1  | 0   | 0   | 0   | 0   | 0   | 0    | 0    | 0    | 0    | 0    | -1 | -1 | -1 | -1 | -1 |
| R      | 1  | 1  | 1  | 1  | 1  | 1  | 1  | 1  | 1  | 1  | -1 | -1 | -1 | -1 | -1 | $i$ | $i$ | $i$ | $i$ | $i$ | $-i$ | $-i$ | $-i$ | $-i$ | $-i$ | -1 | -1 | -1 | -1 | -1 |
| Landau | A1 | A1 | A1 | A1 | A1 | A1 | A1 | A1 | A1 | A1 | B1 | B1 | B1 | B1 | B1 | E   | E   | E   | E   | E   | E    | E    | E    | E    | E    | B2 | B2 | B2 | B2 | B2 |

$$\mathbf{S} = \mathbf{2}, \mathbf{n}_{\text{occ.}} = \{\mathbf{3}, \mathbf{1}\}$$

|        |    |    |    |    |    |    |    |    |    |    |          |          |          |          |          |          |          |          |          |          |            |            |            |            |            |            |            |            |            |     |     |     |     |     |     |     |     |     |     |     |    |
|--------|----|----|----|----|----|----|----|----|----|----|----------|----------|----------|----------|----------|----------|----------|----------|----------|----------|------------|------------|------------|------------|------------|------------|------------|------------|------------|-----|-----|-----|-----|-----|-----|-----|-----|-----|-----|-----|----|
| State  | 89 | 90 | 91 | 92 | 93 | 94 | 95 | 96 | 97 | 98 | 99       | 100      | 101      | 102      | 103      | 104      | 105      | 106      | 107      | 108      | 109        | 110        | 111        | 112        | 113        | 114        | 115        | 116        | 117        | 118 | 119 | 120 | 121 | 122 | 123 | 124 | 125 | 126 | 127 | 128 |    |
| Sz     | 2  | 1  | 0  | -1 | -2 | 2  | 1  | 0  | -1 | -2 | 2        | 1        | 0        | -1       | -2       | 2        | 1        | 0        | -1       | -2       | 2          | 1          | 0          | -1         | -2         | 2          | 1          | 0          | -1         | -2  | 2   | 1   | 0   | -1  | -2  | 2   | 1   | 0   | -1  | -2  |    |
| Rx     | 1  | 1  | 1  | 1  | 1  | 1  | 1  | 1  | 1  | 1  | 0        | 0        | 0        | 0        | 0        | 0        | 0        | 0        | 0        | 0        | 0          | 0          | 0          | 0          | 0          | 0          | 0          | 0          | 0          | 0   | -1  | -1  | -1  | -1  | -1  | -1  | -1  | -1  | -1  | -1  |    |
| Ry     | 1  | 1  | 1  | 1  | 1  | 1  | 1  | 1  | 1  | 1  | 0        | 0        | 0        | 0        | 0        | 0        | 0        | 0        | 0        | 0        | 0          | 0          | 0          | 0          | 0          | 0          | 0          | 0          | 0          | 0   | -1  | -1  | -1  | -1  | -1  | -1  | -1  | -1  | -1  | -1  |    |
| R      | 1  | 1  | 1  | 1  | 1  | -1 | -1 | -1 | -1 | -1 | <i>i</i> | <i>i</i> | <i>i</i> | <i>i</i> | <i>i</i> | <i>i</i> | <i>i</i> | <i>i</i> | <i>i</i> | <i>i</i> | - <i>i</i> | - <i>i</i> | - <i>i</i> | - <i>i</i> | - <i>i</i> | - <i>i</i> | - <i>i</i> | - <i>i</i> | - <i>i</i> | 1   | 1   | 1   | 1   | 1   | -1  | -1  | -1  | -1  | -1  |     |    |
| Landau | A1 | A1 | A1 | A1 | A1 | B1 | B1 | B1 | B1 | B1 | E        | E        | E        | E        | E        | E        | E        | E        | E        | E        | E          | E          | E          | E          | E          | E          | E          | E          | E          | E   | A2  | A2  | A2  | A2  | A2  | A2  | B2  | B2  | B2  | B2  | B2 |

$\mathbf{S} = \mathbf{2}, \mathbf{n}_{occ.} = \{\mathbf{2}, \mathbf{2}\}$

|        |     |     |     |     |     |     |     |     |     |     |     |     |     |     |     |     |     |     |     |     |     |     |     |     |     |     |     |     |     |     |
|--------|-----|-----|-----|-----|-----|-----|-----|-----|-----|-----|-----|-----|-----|-----|-----|-----|-----|-----|-----|-----|-----|-----|-----|-----|-----|-----|-----|-----|-----|-----|
| State  | 129 | 130 | 131 | 132 | 133 | 134 | 135 | 136 | 137 | 138 | 139 | 140 | 141 | 142 | 143 | 144 | 145 | 146 | 147 | 148 | 149 | 150 | 151 | 152 | 153 | 154 | 155 | 156 | 157 | 158 |
| Sz     | 2   | 1   | 0   | -1  | -2  | 2   | 1   | 0   | -1  | -2  | 2   | 1   | 0   | -1  | -2  | 2   | 1   | 0   | -1  | -2  | 2   | 1   | 0   | -1  | -2  | 2   | 1   | 0   | -1  | -2  |
| Rx     | 1   | 1   | 1   | 1   | 1   | 1   | 1   | 1   | 1   | 1   | 1   | 1   | 1   | 1   | 1   | 0   | 0   | 0   | 0   | 0   | 0   | 0   | 0   | 0   | 0   | 0   | -1  | -1  | -1  | -1  |
| Ry     | 1   | 1   | 1   | 1   | 1   | 1   | 1   | 1   | 1   | 1   | 1   | 1   | 1   | 1   | 1   | 0   | 0   | 0   | 0   | 0   | 0   | 0   | 0   | 0   | 0   | 0   | -1  | -1  | -1  | -1  |
| R      | 1   | 1   | 1   | 1   | 1   | 1   | 1   | 1   | 1   | 1   | 1   | -1  | -1  | -1  | -1  | -1  | i   | i   | i   | i   | i   | -i  | -i  | -i  | -i  | -i  | -1  | -1  | -1  | -1  |
| Landau | A1  | A1  | A1  | A1  | A1  | A1  | A1  | A1  | A1  | A1  | B1  | B1  | B1  | B1  | B1  | E   | E   | E   | E   | E   | E   | E   | E   | E   | E   | E   | B2  | B2  | B2  | B2  |

$$S = 1, \text{ n}_{\text{occ.}} = \{4, 0\}$$

$$\left( \begin{array}{c|cccccccccccccccccccccccc} \text{State} & 159 & 160 & 161 & 162 & 163 & 164 & 165 & 166 & 167 & 168 & 169 & 170 & 171 & 172 & 173 & 174 & 175 & 176 \\ \hline \text{Sz} & 1 & 0 & -1 & 1 & 0 & -1 & 1 & 0 & -1 & 1 & 0 & -1 & 1 & 0 & -1 & 1 & 0 & -1 \\ \text{Rx} & 1 & 1 & 1 & 0 & 0 & 0 & 0 & 0 & 0 & 0 & 0 & 0 & 0 & 0 & 0 & -1 & -1 & -1 \\ \text{Ry} & 1 & 1 & 1 & 0 & 0 & 0 & 0 & 0 & 0 & 0 & 0 & 0 & 0 & 0 & 0 & -1 & -1 & -1 \\ \text{R} & -1 & -1 & -1 & i & i & i & i & i & i & -i & -i & -i & -i & -i & -i & 1 & 1 & 1 \\ \text{Landau} & \text{B1} & \text{B1} & \text{B1} & \text{E} & \text{E} & \text{E} & \text{E} & \text{E} & \text{E} & \text{E} & \text{E} & \text{E} & \text{E} & \text{E} & \text{E} & \text{A2} & \text{A2} & \text{A2} \end{array} \right)$$



$\mathbf{S} = \mathbf{1}, \mathbf{n}_{\text{occ.}} = \{\mathbf{3}, \mathbf{1}\}$

| State  | 177 | 178 | 179 | 180 | 181 | 182 | 183 | 184 | 185 | 186 | 187 | 188 | 189 | 190 | 191 | 192 | 193 | 194 | 195 | 196 | 197 | 198 | 199  | 200  | 201  | 202  | 203  | 204  | 205  | 206 | 207 | 208 | 209 | 210 | 211 | 212 |
|--------|-----|-----|-----|-----|-----|-----|-----|-----|-----|-----|-----|-----|-----|-----|-----|-----|-----|-----|-----|-----|-----|-----|------|------|------|------|------|------|------|-----|-----|-----|-----|-----|-----|-----|
| Sz     | 1   | 0   | -1  | 1   | 0   | -1  | 1   | 0   | -1  | 1   | 0   | -1  | 1   | 0   | -1  | 1   | 0   | -1  | 1   | 0   | -1  | 1   | 0    | -1   | 1    | 0    | -1   | 1    | 0    | -1  | 1   | 0   | -1  | 1   | 0   | -1  |
| Rx     | 1   | 1   | 1   | 1   | 1   | 1   | 1   | 1   | 1   | 1   | 1   | 1   | 0   | 0   | 0   | 0   | 0   | 0   | 0   | 0   | 0   | 0   | 0    | 0    | 0    | 0    | 0    | 0    | 0    | 0   | -1  | -1  | -1  | -1  | -1  | -1  |
| Ry     | 1   | 1   | 1   | 1   | 1   | 1   | 1   | 1   | 1   | 1   | 1   | 1   | 0   | 0   | 0   | 0   | 0   | 0   | 0   | 0   | 0   | 0   | 0    | 0    | 0    | 0    | 0    | 0    | 0    | 0   | -1  | -1  | -1  | -1  | -1  | -1  |
| R      | 1   | 1   | 1   | 1   | 1   | 1   | -1  | -1  | -1  | -1  | -1  | -1  | $i$ | $i$ | $i$ | $i$ | $i$ | $i$ | $i$ | $i$ | $i$ | $i$ | $-i$ | $-i$ | $-i$ | $-i$ | $-i$ | $-i$ | $-i$ | 1   | 1   | 1   | -1  | -1  | -1  |     |
| Landau | A1  | A1  | A1  | A1  | A1  | A1  | B1  | B1  | B1  | B1  | B1  | B1  | E   | E   | E   | E   | E   | E   | E   | E   | E   | E   | E    | E    | E    | E    | E    | E    | E    | E   | A2  | A2  | A2  | B2  | B2  | B2  |

$$S = 1, \text{ n}_{\text{occ.}} = \{2, 2\}$$

$$\left( \begin{array}{cccccccccccccccccccccccc} \text{State} & 213 & 214 & 215 & 216 & 217 & 218 & 219 & 220 & 221 & 222 & 223 & 224 & 225 & 226 & 227 & 228 & 229 & 230 \\ \text{Sz} & 1 & 0 & -1 & 1 & 0 & -1 & 1 & 0 & -1 & 1 & 0 & -1 & 1 & 0 & -1 & 1 & 0 & -1 \\ \text{Rx} & 1 & 1 & 1 & 0 & 0 & 0 & 0 & 0 & 0 & 0 & 0 & 0 & 0 & 0 & 0 & -1 & -1 & -1 \\ \text{Ry} & 1 & 1 & 1 & 0 & 0 & 0 & 0 & 0 & 0 & 0 & 0 & 0 & 0 & 0 & 0 & -1 & -1 & -1 \\ \text{R} & -1 & -1 & -1 & i & i & i & i & i & i & -i & -i & -i & -i & -i & -i & 1 & 1 & 1 \\ \text{Landau} & \text{B1} & \text{B1} & \text{B1} & \text{E} & \text{E} & \text{E} & \text{E} & \text{E} & \text{E} & \text{E} & \text{E} & \text{E} & \text{E} & \text{E} & \text{E} & \text{A2} & \text{A2} & \text{A2} \end{array} \right)$$



$$\mathbf{S} = \mathbf{0}, \text{ n}_{\text{occ.}} = \{4, \mathbf{0}\}$$

$$\left( \begin{array}{cccc} \text{State} & 243 & 244 & 245 \\ \text{Sz} & 0 & 0 & 0 \\ \text{Rx} & 1 & 1 & -1 \\ \text{Ry} & 1 & 1 & -1 \\ \text{R} & 1 & 1 & -1 \\ \text{Landau} & \text{A1} & \text{A1} & \text{B2} \end{array} \right)$$

$$\mathbf{S} = \mathbf{0}, \text{ n}_{\text{occ.}} = \{\mathbf{3}, \mathbf{1}\}$$

$$\left( \begin{array}{ccccc} \text{State} & 246 & 247 & 248 & 249 \\ \text{Sz} & 0 & 0 & 0 & 0 \\ \text{Rx} & 0 & 0 & -1 & -1 \\ \text{Ry} & 0 & 0 & -1 & -1 \\ \text{R} & i & -i & 1 & -1 \\ \text{Landau} & \text{E} & \text{E} & \text{A2} & \text{B2} \end{array} \right)$$

$$\mathbf{S} = \mathbf{0}, \mathbf{n}_{\text{occ.}} = \{\mathbf{2}, \mathbf{2}\}$$

| State  | 250 | 251 | 252 | 253 | 254  | 255 |
|--------|-----|-----|-----|-----|------|-----|
| Sz     | 0   | 0   | 0   | 0   | 0    | 0   |
| Rx     | 1   | 1   | 1   | 0   | 0    | -1  |
| Ry     | 1   | 1   | 1   | 0   | 0    | -1  |
| R      | 1   | 1   | -1  | $i$ | $-i$ | -1  |
| Landau | A1  | A1  | B1  | E   | E    | B2  |

$$\mathbf{S} = \mathbf{0}, \text{ n}_{\text{occ.}} = \{0, 4\}$$

$$\left( \begin{array}{cc} \text{State} & 256 \\ \text{Sz} & 0 \\ \text{Rx} & 1 \\ \text{Ry} & 1 \\ \text{R} & 1 \\ \text{Landau} & \text{A1} \end{array} \right)$$

$$\mathbf{S} = \mathbf{2}, \mathbf{n}_{\text{occ.}} = \{4, \mathbf{0}\}$$

$$\left( \begin{array}{ccccc} \text{State} & 1 & 2 & 3 & 4 & 5 \\ \text{Sz} & 2 & 1 & 0 & -1 & -2 \\ \text{Rx} & 1 & 1 & 1 & 1 & 1 \\ \text{Ry} & 1 & 1 & 1 & 1 & 1 \\ \text{R} & 1 & 1 & 1 & 1 & 1 \\ \text{Landau} & \text{A1} & \text{A1} & \text{A1} & \text{A1} & \text{A1} \end{array} \right)$$





$$\mathbf{S} = \mathbf{2}, \mathbf{n}_{\text{occ.}} = \{\mathbf{2}, \mathbf{2}\}$$

| State  | 26 | 27 | 28 | 29 | 30 | 31 | 32 | 33 | 34 | 35 | 36 | 37 | 38 | 39 | 40 | 41  | 42  | 43  | 44  | 45  | 46   | 47   | 48   | 49   | 50   | 51 | 52 | 53 | 54 | 55 |
|--------|----|----|----|----|----|----|----|----|----|----|----|----|----|----|----|-----|-----|-----|-----|-----|------|------|------|------|------|----|----|----|----|----|
| Sz     | 2  | 1  | 0  | -1 | -2 | 2  | 1  | 0  | -1 | -2 | 2  | 1  | 0  | -1 | -2 | 2   | 1   | 0   | -1  | -2  | 2    | 1    | 0    | -1   | -2   | 2  | 1  | 0  | -1 | -2 |
| Rx     | 1  | 1  | 1  | 1  | 1  | 1  | 1  | 1  | 1  | 1  | 1  | 1  | 1  | 1  | 1  | 0   | 0   | 0   | 0   | 0   | 0    | 0    | 0    | 0    | 0    | -1 | -1 | -1 | -1 | -1 |
| Ry     | 1  | 1  | 1  | 1  | 1  | 1  | 1  | 1  | 1  | 1  | 1  | 1  | 1  | 1  | 1  | 0   | 0   | 0   | 0   | 0   | 0    | 0    | 0    | 0    | 0    | -1 | -1 | -1 | -1 | -1 |
| R      | 1  | 1  | 1  | 1  | 1  | 1  | 1  | 1  | 1  | 1  | -1 | -1 | -1 | -1 | -1 | $i$ | $i$ | $i$ | $i$ | $i$ | $-i$ | $-i$ | $-i$ | $-i$ | $-i$ | -1 | -1 | -1 | -1 | -1 |
| Landau | A1 | A1 | A1 | A1 | A1 | A1 | A1 | A1 | A1 | A1 | B1 | B1 | B1 | B1 | B1 | E   | E   | E   | E   | E   | E    | E    | E    | E    | E    | B2 | B2 | B2 | B2 | B2 |

$$S = 2, \text{ n}_{\text{occ.}} = \{1, 3\}$$

[illegible]

$$\mathbf{S} = \mathbf{2}, \mathbf{n}_{\text{occ.}} = \{0, 4\}$$

$$\left( \begin{array}{cccccc} \text{State} & 76 & 77 & 78 & 79 & 80 \\ \text{Sz} & 2 & 1 & 0 & -1 & -2 \\ \text{Rx} & 1 & 1 & 1 & 1 & 1 \\ \text{Ry} & 1 & 1 & 1 & 1 & 1 \\ \text{R} & 1 & 1 & 1 & 1 & 1 \\ \text{Landau} & \text{A1} & \text{A1} & \text{A1} & \text{A1} & \text{A1} \end{array} \right)$$



$\mathbf{S} = \mathbf{1}, \mathbf{n}_{\text{occ.}} = \{\mathbf{3}, \mathbf{1}\}$

|        |    |    |    |    |    |    |    |    |    |    |     |     |     |     |     |     |     |     |     |     |     |      |      |      |      |      |      |      |      |      |     |     |     |     |     |     |    |
|--------|----|----|----|----|----|----|----|----|----|----|-----|-----|-----|-----|-----|-----|-----|-----|-----|-----|-----|------|------|------|------|------|------|------|------|------|-----|-----|-----|-----|-----|-----|----|
| State  | 90 | 91 | 92 | 93 | 94 | 95 | 96 | 97 | 98 | 99 | 100 | 101 | 102 | 103 | 104 | 105 | 106 | 107 | 108 | 109 | 110 | 111  | 112  | 113  | 114  | 115  | 116  | 117  | 118  | 119  | 120 | 121 | 122 | 123 | 124 | 125 |    |
| Sz     | 1  | 0  | -1 | 1  | 0  | -1 | 1  | 0  | -1 | 1  | 0   | -1  | 1   | 0   | -1  | 1   | 0   | -1  | 1   | 0   | -1  | 1    | 0    | -1   | 1    | 0    | -1   | 1    | 0    | -1   | 1   | 0   | -1  | 1   | 0   | -1  |    |
| Rx     | 1  | 1  | 1  | 1  | 1  | 1  | 1  | 1  | 1  | 1  | 1   | 1   | 0   | 0   | 0   | 0   | 0   | 0   | 0   | 0   | 0   | 0    | 0    | 0    | 0    | 0    | 0    | 0    | 0    | 0    | -1  | -1  | -1  | -1  | -1  | -1  |    |
| Ry     | 1  | 1  | 1  | 1  | 1  | 1  | 1  | 1  | 1  | 1  | 1   | 1   | 0   | 0   | 0   | 0   | 0   | 0   | 0   | 0   | 0   | 0    | 0    | 0    | 0    | 0    | 0    | 0    | 0    | 0    | 0   | -1  | -1  | -1  | -1  | -1  | -1 |
| R      | 1  | 1  | 1  | 1  | 1  | 1  | -1 | -1 | -1 | -1 | -1  | -1  | $i$ | $i$ | $i$ | $i$ | $i$ | $i$ | $i$ | $i$ | $i$ | $-i$ | $-i$ | $-i$ | $-i$ | $-i$ | $-i$ | $-i$ | $-i$ | $-i$ | 1   | 1   | 1   | -1  | -1  | -1  |    |
| Landau | A1 | A1 | A1 | A1 | A1 | A1 | B1 | B1 | B1 | B1 | B1  | B1  | E   | E   | E   | E   | E   | E   | E   | E   | E   | E    | E    | E    | E    | E    | E    | E    | E    | E    | A2  | A2  | A2  | B2  | B2  | B2  |    |

$$\mathbf{S} = \mathbf{1}, \mathbf{n}_{\text{occ.}}$$

$$\left( \begin{array}{c} \text{State} \\ \text{Sz} \\ \text{Rx} \\ \text{Ry} \\ \text{R} \\ \text{Landau} \end{array} \right)$$

[illegible]

$\mathbf{S} = \mathbf{1}, \mathbf{n}_{occ.} = \{\mathbf{1}, \mathbf{3}\}$

|        |     |     |     |     |     |     |     |     |     |     |     |     |          |          |          |          |          |          |          |          |          |            |            |            |            |            |            |            |            |     |     |     |     |     |     |     |
|--------|-----|-----|-----|-----|-----|-----|-----|-----|-----|-----|-----|-----|----------|----------|----------|----------|----------|----------|----------|----------|----------|------------|------------|------------|------------|------------|------------|------------|------------|-----|-----|-----|-----|-----|-----|-----|
| State  | 180 | 181 | 182 | 183 | 184 | 185 | 186 | 187 | 188 | 189 | 190 | 191 | 192      | 193      | 194      | 195      | 196      | 197      | 198      | 199      | 200      | 201        | 202        | 203        | 204        | 205        | 206        | 207        | 208        | 209 | 210 | 211 | 212 | 213 | 214 | 215 |
| Sz     | 1   | 0   | -1  | 1   | 0   | -1  | 1   | 0   | -1  | 1   | 0   | -1  | 1        | 0        | -1       | 1        | 0        | -1       | 1        | 0        | -1       | 1          | 0          | -1         | 1          | 0          | -1         | 1          | 0          | -1  | 1   | 0   | -1  | 1   | 0   | -1  |
| Rx     | 1   | 1   | 1   | 1   | 1   | 1   | 1   | 1   | 1   | 1   | 1   | 1   | 0        | 0        | 0        | 0        | 0        | 0        | 0        | 0        | 0        | 0          | 0          | 0          | 0          | 0          | 0          | 0          | 0          | 0   | -1  | -1  | -1  | -1  | -1  | -1  |
| Ry     | 1   | 1   | 1   | 1   | 1   | 1   | 1   | 1   | 1   | 1   | 1   | 1   | 0        | 0        | 0        | 0        | 0        | 0        | 0        | 0        | 0        | 0          | 0          | 0          | 0          | 0          | 0          | 0          | 0          | 0   | -1  | -1  | -1  | -1  | -1  | -1  |
| R      | 1   | 1   | 1   | 1   | 1   | 1   | -1  | -1  | -1  | -1  | -1  | -1  | <i>i</i> | <i>i</i> | <i>i</i> | <i>i</i> | <i>i</i> | <i>i</i> | <i>i</i> | <i>i</i> | <i>i</i> | - <i>i</i> | - <i>i</i> | - <i>i</i> | - <i>i</i> | - <i>i</i> | - <i>i</i> | - <i>i</i> | - <i>i</i> | 1   | 1   | 1   | -1  | -1  | -1  |     |
| Landau | A1  | A1  | A1  | A1  | A1  | A1  | B1  | B1  | B1  | B1  | B1  | B1  | E        | E        | E        | E        | E        | E        | E        | E        | E        | E          | E          | E          | E          | E          | E          | E          | E          | E   | A2  | A2  | A2  | B2  | B2  | B2  |





$$\mathbf{S} = \mathbf{0}, \text{ n}_{\text{occ.}} = \{4, \mathbf{0}\}$$

$$\left( \begin{array}{ccc} \text{State} & 225 & 226 \\ \text{Sz} & 0 & 0 \\ \text{Rx} & 1 & -1 \\ \text{Ry} & 1 & -1 \\ \text{R} & 1 & -1 \\ \text{Landau} & \text{A1} & \text{B2} \end{array} \right)$$

$$\mathbf{S} = \mathbf{0}, \text{ n}_{\text{occ.}} = \{3, 1\}$$

$$\left( \begin{array}{c|cccccccccc} \text{State} & 227 & 228 & 229 & 230 & 231 & 232 & 233 & 234 \\ \hline \text{Sz} & 0 & 0 & 0 & 0 & 0 & 0 & 0 & 0 \\ \text{Rx} & 1 & 1 & 0 & 0 & 0 & 0 & -1 & -1 \\ \text{Ry} & 1 & 1 & 0 & 0 & 0 & 0 & -1 & -1 \\ \text{R} & 1 & -1 & i & i & -i & -i & 1 & -1 \\ \text{Landau} & A1 & B1 & E & E & E & E & A2 & B2 \end{array} \right)$$

$$\mathbf{S} = \mathbf{0}, \mathbf{n}_{\text{occ.}} = \{\mathbf{2}, \mathbf{2}\}$$

| State  | 235 | 236 | 237 | 238 | 239 | 240 | 241  | 242  | 243 | 244 | 245 | 246 |
|--------|-----|-----|-----|-----|-----|-----|------|------|-----|-----|-----|-----|
| Sz     | 0   | 0   | 0   | 0   | 0   | 0   | 0    | 0    | 0   | 0   | 0   | 0   |
| Rx     | 1   | 1   | 1   | 1   | 0   | 0   | 0    | 0    | -1  | -1  | -1  | -1  |
| Ry     | 1   | 1   | 1   | 1   | 0   | 0   | 0    | 0    | -1  | -1  | -1  | -1  |
| R      | 1   | 1   | 1   | -1  | $i$ | $i$ | $-i$ | $-i$ | 1   | -1  | -1  | -1  |
| Landau | A1  | A1  | A1  | B1  | E   | E   | E    | E    | A2  | B2  | B2  | B2  |

$$\mathbf{S} = \mathbf{0}, \text{ n}_{\text{occ.}} = \{1, 3\}$$

| State  | 247 | 248 | 249 | 250 | 251  | 252  | 253 | 254 |
|--------|-----|-----|-----|-----|------|------|-----|-----|
| Sz     | 0   | 0   | 0   | 0   | 0    | 0    | 0   | 0   |
| Rx     | 1   | 1   | 0   | 0   | 0    | 0    | -1  | -1  |
| Ry     | 1   | 1   | 0   | 0   | 0    | 0    | -1  | -1  |
| R      | 1   | -1  | $i$ | $i$ | $-i$ | $-i$ | 1   | -1  |
| Landau | A1  | B1  | E   | E   | E    | E    | A2  | B2  |

$$\mathbf{S} = \mathbf{0}, \text{ n}_{\text{occ.}} = \{0, 4\}$$

$$\left( \begin{array}{ccc} \text{State} & 255 & 256 \\ \text{Sz} & 0 & 0 \\ \text{Rx} & 1 & -1 \\ \text{Ry} & 1 & -1 \\ \text{R} & 1 & -1 \\ \text{Landau} & \text{A1} & \text{B2} \end{array} \right)$$

$$\mathbf{S} = \mathbf{2}, \mathbf{n}_{\text{occ.}} = \{4, \mathbf{0}, \mathbf{0}\}$$

$$\left( \begin{array}{ccccc} \text{State} & 1 & 2 & 3 & 4 & 5 \\ \text{Sz} & 2 & 1 & 0 & -1 & -2 \\ \text{Rx} & 1 & 1 & 1 & 1 & 1 \\ \text{Ry} & 1 & 1 & 1 & 1 & 1 \\ \text{R} & 1 & 1 & 1 & 1 & 1 \\ \text{Landau} & \text{A1} & \text{A1} & \text{A1} & \text{A1} & \text{A1} \end{array} \right)$$









$$\mathbf{S} = \mathbf{1}, \mathbf{n}_{\text{occ.}} = \{\mathbf{2}, \mathbf{2}, \mathbf{0}\}$$

$$\left( \begin{array}{c|cccccccccccccccccccc} \text{State} & 47 & 48 & 49 & 50 & 51 & 52 & 53 & 54 & 55 & 56 & 57 & 58 & 59 & 60 & 61 & 62 & 63 & 64 \\ \hline \text{Sz} & 1 & 0 & -1 & 1 & 0 & -1 & 1 & 0 & -1 & 1 & 0 & -1 & 1 & 0 & -1 & 1 & 0 & -1 \\ \text{Rx} & 1 & 1 & 1 & 1 & 1 & 1 & 1 & 1 & 1 & 0 & 0 & 0 & 0 & 0 & 0 & -1 & -1 & -1 \\ \text{Ry} & 1 & 1 & 1 & 1 & 1 & 1 & 1 & 1 & 1 & 0 & 0 & 0 & 0 & 0 & 0 & -1 & -1 & -1 \\ \text{R} & 1 & 1 & 1 & 1 & 1 & 1 & -1 & -1 & -1 & i & i & i & -i & -i & -i & -1 & -1 & -1 \\ \text{Landau} & \text{A1} & \text{A1} & \text{A1} & \text{A1} & \text{A1} & \text{A1} & \text{B1} & \text{B1} & \text{B1} & \text{E} & \text{E} & \text{E} & \text{E} & \text{E} & \text{E} & \text{B2} & \text{B2} & \text{B2} \end{array} \right)$$

$$\mathbf{S} = \mathbf{1}, \mathbf{n}_{\text{occ.}} = \{\mathbf{2}, \mathbf{1}, \mathbf{1}\}$$

| State  | 65 | 66 | 67 | 68 | 69 | 70 | 71 | 72 | 73 | 74 | 75 | 76 | 77  | 78  | 79  | 80  | 81  | 82  | 83  | 84  | 85  | 86  | 87   | 88   | 89   | 90   | 91   | 92   | 93   | 94 | 95 | 96 | 97 | 98 | 99 | 100 |
|--------|----|----|----|----|----|----|----|----|----|----|----|----|-----|-----|-----|-----|-----|-----|-----|-----|-----|-----|------|------|------|------|------|------|------|----|----|----|----|----|----|-----|
| Sz     | 1  | 0  | -1 | 1  | 0  | -1 | 1  | 0  | -1 | 1  | 0  | -1 | 1   | 0   | -1  | 1   | 0   | -1  | 1   | 0   | -1  | 1   | 0    | -1   | 1    | 0    | -1   | 1    | 0    | -1 | 1  | 0  | -1 | 1  | 0  | -1  |
| Rx     | 1  | 1  | 1  | 1  | 1  | 1  | 1  | 1  | 1  | 1  | 1  | 1  | 0   | 0   | 0   | 0   | 0   | 0   | 0   | 0   | 0   | 0   | 0    | 0    | 0    | 0    | 0    | 0    | 0    | 0  | -1 | -1 | -1 | -1 | -1 | -1  |
| Ry     | 1  | 1  | 1  | 1  | 1  | 1  | 1  | 1  | 1  | 1  | 1  | 1  | 0   | 0   | 0   | 0   | 0   | 0   | 0   | 0   | 0   | 0   | 0    | 0    | 0    | 0    | 0    | 0    | 0    | 0  | -1 | -1 | -1 | -1 | -1 | -1  |
| R      | 1  | 1  | 1  | 1  | 1  | 1  | -1 | -1 | -1 | -1 | -1 | -1 | $i$ | $i$ | $i$ | $i$ | $i$ | $i$ | $i$ | $i$ | $i$ | $i$ | $-i$ | $-i$ | $-i$ | $-i$ | $-i$ | $-i$ | $-i$ | 1  | 1  | 1  | -1 | -1 | -1 |     |
| Landau | A1 | A1 | A1 | A1 | A1 | A1 | B1 | B1 | B1 | B1 | B1 | B1 | E   | E   | E   | E   | E   | E   | E   | E   | E   | E   | E    | E    | E    | E    | E    | E    | E    | E  | A2 | A2 | A2 | B2 | B2 | B2  |

$$S = 1, \text{ n}_{\text{occ.}} = \{2, 0, 2\}$$

[illegible]





$$\mathbf{S} = \mathbf{1}/2, \mathbf{n}_{\text{occ.}} = \{\mathbf{1}, \mathbf{3}, \mathbf{0}\}$$

$$\left( \begin{array}{cccccccccc} \text{State} & 151 & 152 & 153 & 154 & 155 & 156 & 157 & 158 \\ \text{Sz} & \frac{1}{2} & -\frac{1}{2} & \frac{1}{2} & -\frac{1}{2} & \frac{1}{2} & -\frac{1}{2} & \frac{1}{2} & -\frac{1}{2} \\ \text{Rx} & 1 & 1 & 1 & 1 & 0 & 0 & 0 & 0 \\ \text{Ry} & 1 & 1 & 1 & 1 & 0 & 0 & 0 & 0 \\ \text{R} & 1 & 1 & -1 & -1 & i & i & -i & -i \\ \text{Landau} & \text{A1} & \text{A1} & \text{B1} & \text{B1} & \text{E} & \text{E} & \text{E} & \text{E} \end{array} \right)$$



$$\mathbf{S} = \mathbf{1}/2, \mathbf{n}_{\text{occ.}} = \{\mathbf{1}, \mathbf{2}, \mathbf{1}\}$$

| State  | 159           | 160            | 161           | 162            | 163           | 164            | 165           | 166            | 167           | 168            | 169           | 170            | 171           | 172            | 173           | 174            | 175           | 176            | 177           | 178            | 179           | 180            | 181           | 182            |
|--------|---------------|----------------|---------------|----------------|---------------|----------------|---------------|----------------|---------------|----------------|---------------|----------------|---------------|----------------|---------------|----------------|---------------|----------------|---------------|----------------|---------------|----------------|---------------|----------------|
| Sz     | $\frac{1}{2}$ | $-\frac{1}{2}$ | $\frac{1}{2}$ | $-\frac{1}{2}$ | $\frac{1}{2}$ | $-\frac{1}{2}$ | $\frac{1}{2}$ | $-\frac{1}{2}$ | $\frac{1}{2}$ | $-\frac{1}{2}$ | $\frac{1}{2}$ | $-\frac{1}{2}$ | $\frac{1}{2}$ | $-\frac{1}{2}$ | $\frac{1}{2}$ | $-\frac{1}{2}$ | $\frac{1}{2}$ | $-\frac{1}{2}$ | $\frac{1}{2}$ | $-\frac{1}{2}$ | $\frac{1}{2}$ | $-\frac{1}{2}$ | $\frac{1}{2}$ | $-\frac{1}{2}$ |
| Rx     | 1             | 1              | 1             | 1              | 1             | 1              | 1             | 1              | 0             | 0              | 0             | 0              | 0             | 0              | 0             | 0              | 0             | 0              | 0             | 0              | -1            | -1             | -1            | -1             |
| Ry     | 1             | 1              | 1             | 1              | 1             | 1              | 1             | 1              | 0             | 0              | 0             | 0              | 0             | 0              | 0             | 0              | 0             | 0              | 0             | 0              | -1            | -1             | -1            | -1             |
| R      | 1             | 1              | 1             | 1              | -1            | -1             | -1            | -1             | $i$           | $i$            | $i$           | $i$            | $i$           | $i$            | $-i$          | $-i$           | $-i$          | $-i$           | $-i$          | $-i$           | 1             | 1              | -1            | -1             |
| Landau | A1            | A1             | A1            | A1             | B1            | B1             | B1            | B1             | E             | E              | E             | E              | E             | E              | E             | E              | E             | E              | E             | E              | A2            | A2             | B2            | B2             |

$$\mathbf{S} = \mathbf{1}/2, \mathbf{n}_{\text{occ.}} = \{\mathbf{1}, \mathbf{1}, \mathbf{2}\}$$

| State  | 183           | 184            | 185           | 186            | 187           | 188            | 189           | 190            | 191           | 192            | 193           | 194            | 195           | 196            | 197           | 198            | 199           | 200            | 201           | 202            | 203           | 204            | 205           | 206            |
|--------|---------------|----------------|---------------|----------------|---------------|----------------|---------------|----------------|---------------|----------------|---------------|----------------|---------------|----------------|---------------|----------------|---------------|----------------|---------------|----------------|---------------|----------------|---------------|----------------|
| Sz     | $\frac{1}{2}$ | $-\frac{1}{2}$ | $\frac{1}{2}$ | $-\frac{1}{2}$ | $\frac{1}{2}$ | $-\frac{1}{2}$ | $\frac{1}{2}$ | $-\frac{1}{2}$ | $\frac{1}{2}$ | $-\frac{1}{2}$ | $\frac{1}{2}$ | $-\frac{1}{2}$ | $\frac{1}{2}$ | $-\frac{1}{2}$ | $\frac{1}{2}$ | $-\frac{1}{2}$ | $\frac{1}{2}$ | $-\frac{1}{2}$ | $\frac{1}{2}$ | $-\frac{1}{2}$ | $\frac{1}{2}$ | $-\frac{1}{2}$ | $\frac{1}{2}$ | $-\frac{1}{2}$ |
| Rx     | 1             | 1              | 1             | 1              | 1             | 1              | 1             | 1              | 0             | 0              | 0             | 0              | 0             | 0              | 0             | 0              | 0             | 0              | 0             | 0              | -1            | -1             | -1            | -1             |
| Ry     | 1             | 1              | 1             | 1              | 1             | 1              | 1             | 1              | 0             | 0              | 0             | 0              | 0             | 0              | 0             | 0              | 0             | 0              | 0             | 0              | -1            | -1             | -1            | -1             |
| R      | 1             | 1              | 1             | 1              | -1            | -1             | -1            | -1             | $i$           | $i$            | $i$           | $i$            | $i$           | $i$            | $-i$          | $-i$           | $-i$          | $-i$           | $-i$          | $-i$           | 1             | 1              | -1            | -1             |
| Landau | A1            | A1             | A1            | A1             | B1            | B1             | B1            | B1             | E             | E              | E             | E              | E             | E              | E             | E              | E             | E              | E             | E              | A2            | A2             | B2            | B2             |

$$\mathbf{S} = \mathbf{1}/\mathbf{2}, \text{ n}_{\text{occ.}} = \{\mathbf{1}, \mathbf{0}, \mathbf{3}\}$$

$$\left( \begin{array}{c|cccccccc} \text{State} & 207 & 208 & 209 & 210 & 211 & 212 & 213 & 214 \\ \hline \text{Sz} & \frac{1}{2} & -\frac{1}{2} & \frac{1}{2} & -\frac{1}{2} & \frac{1}{2} & -\frac{1}{2} & \frac{1}{2} & -\frac{1}{2} \\ \text{Rx} & 1 & 1 & 1 & 1 & 0 & 0 & 0 & 0 \\ \text{Ry} & 1 & 1 & 1 & 1 & 0 & 0 & 0 & 0 \\ \text{R} & 1 & 1 & -1 & -1 & i & i & -i & -i \\ \text{Landau} & \text{A1} & \text{A1} & \text{B1} & \text{B1} & \text{E} & \text{E} & \text{E} & \text{E} \end{array} \right)$$

$$\mathbf{S} = \mathbf{0}, \mathbf{n}_{\text{occ.}} = \{4, \mathbf{0}, \mathbf{0}\}$$

$$\left( \begin{array}{ccc} \text{State} & 215 & 216 \\ \text{Sz} & 0 & 0 \\ \text{Rx} & 1 & -1 \\ \text{Ry} & 1 & -1 \\ \text{R} & 1 & -1 \\ \text{Landau} & \text{A1} & \text{B2} \end{array} \right)$$

$$\mathbf{S} = \mathbf{0}, \text{ n}_{\text{occ.}} = \{\mathbf{2}, \mathbf{2}, \mathbf{0}\}$$

| State  | 217 | 218 | 219 | 220  | 221  | 222 |
|--------|-----|-----|-----|------|------|-----|
| Sz     | 0   | 0   | 0   | 0    | 0    | 0   |
| Rx     | 1   | 0   | 0   | 0    | 0    | -1  |
| Ry     | 1   | 0   | 0   | 0    | 0    | -1  |
| R      | -1  | $i$ | $i$ | $-i$ | $-i$ | 1   |
| Landau | B1  | E   | E   | E    | E    | A2  |

$$\mathbf{S} = \mathbf{0}, \mathbf{n}_{\text{occ.}} = \{\mathbf{2}, \mathbf{1}, \mathbf{1}\}$$

$$\left( \begin{array}{c|cccccccccccccc} \text{State} & 223 & 224 & 225 & 226 & 227 & 228 & 229 & 230 & 231 & 232 & 233 & 234 \\ \hline \text{Sz} & 0 & 0 & 0 & 0 & 0 & 0 & 0 & 0 & 0 & 0 & 0 & 0 \\ \text{Rx} & 1 & 1 & 0 & 0 & 0 & 0 & 0 & 0 & -1 & -1 & -1 & -1 \\ \text{Ry} & 1 & 1 & 0 & 0 & 0 & 0 & 0 & 0 & -1 & -1 & -1 & -1 \\ \text{R} & 1 & -1 & i & i & i & -i & -i & -i & 1 & 1 & -1 & -1 \\ \text{Landau} & \text{A1} & \text{B1} & \text{E} & \text{E} & \text{E} & \text{E} & \text{E} & \text{E} & \text{A2} & \text{A2} & \text{B2} & \text{B2} \end{array} \right)$$

$$\mathbf{S} = \mathbf{0}, \text{ n}_{\text{occ.}} = \{\mathbf{2}, \mathbf{0}, \mathbf{2}\}$$

| State  | 235 | 236 | 237 | 238  | 239  | 240 |
|--------|-----|-----|-----|------|------|-----|
| Sz     | 0   | 0   | 0   | 0    | 0    | 0   |
| Rx     | 1   | 0   | 0   | 0    | 0    | -1  |
| Ry     | 1   | 0   | 0   | 0    | 0    | -1  |
| R      | -1  | $i$ | $i$ | $-i$ | $-i$ | 1   |
| Landau | B1  | E   | E   | E    | E    | A2  |

$$\mathbf{S} = \mathbf{0}, \text{ n}_{\text{occ.}} = \{0, 4, 0\}$$

$$\left( \begin{array}{cc} \text{State} & 241 \\ \text{Sz} & 0 \\ \text{Rx} & 1 \\ \text{Ry} & 1 \\ \text{R} & 1 \\ \text{Landau} & \text{A1} \end{array} \right)$$



$$\mathbf{S} = \mathbf{0}, \text{ n}_{\text{occ.}} = \{\mathbf{0}, \mathbf{3}, \mathbf{1}\}$$

$$\left( \begin{array}{ccccc} \text{State} & 242 & 243 & 244 & 245 \\ \text{Sz} & 0 & 0 & 0 & 0 \\ \text{Rx} & 1 & 1 & 0 & 0 \\ \text{Ry} & 1 & 1 & 0 & 0 \\ \text{R} & 1 & -1 & i & -i \\ \text{Landau} & \text{A1} & \text{B1} & \text{E} & \text{E} \end{array} \right)$$

$$\mathbf{S} = \mathbf{0}, \mathbf{n}_{\text{occ.}} = \{\mathbf{0}, \mathbf{2}, \mathbf{2}\}$$

| State  | 246 | 247 | 248 | 249 | 250  | 251 |
|--------|-----|-----|-----|-----|------|-----|
| Sz     | 0   | 0   | 0   | 0   | 0    | 0   |
| Rx     | 1   | 1   | 1   | 0   | 0    | -1  |
| Ry     | 1   | 1   | 1   | 0   | 0    | -1  |
| R      | 1   | 1   | -1  | $i$ | $-i$ | -1  |
| Landau | A1  | A1  | B1  | E   | E    | B2  |

$$\mathbf{S} = \mathbf{0}, \text{ n}_{\text{occ.}} = \{\mathbf{0}, \mathbf{1}, \mathbf{3}\}$$

$$\left( \begin{array}{ccccc} \text{State} & 252 & 253 & 254 & 255 \\ \text{Sz} & 0 & 0 & 0 & 0 \\ \text{Rx} & 1 & 1 & 0 & 0 \\ \text{Ry} & 1 & 1 & 0 & 0 \\ \text{R} & 1 & -1 & i & -i \\ \text{Landau} & \text{A1} & \text{B1} & \text{E} & \text{E} \end{array} \right)$$

$$\mathbf{S} = \mathbf{0}, \text{ n}_{\text{occ.}} = \{0, 0, 4\}$$

$$\left( \begin{array}{cc} \text{State} & 256 \\ \text{Sz} & 0 \\ \text{Rx} & 1 \\ \text{Ry} & 1 \\ \text{R} & 1 \\ \text{Landau} & \text{A1} \end{array} \right)$$

$$S = 8, \text{ n}_{\text{occ.}} = \{4\}$$

[illegible]





$$S = 5, n_{\text{acc}} = \{4\}$$



$$\mathbf{S} = A \quad \mathbf{n} = \{A\}$$



$$S = 2, n_{\text{acc}} = \{4\}$$

$\mathbf{S} = \mathbf{1}, \mathbf{n}_{\text{occ.}} = \{4\}$

|        |     |     |     |     |     |     |          |          |          |          |          |          |          |          |          |          |          |          |            |            |            |            |            |            |            |            |            |            |            |            |     |     |     |     |     |     |    |    |
|--------|-----|-----|-----|-----|-----|-----|----------|----------|----------|----------|----------|----------|----------|----------|----------|----------|----------|----------|------------|------------|------------|------------|------------|------------|------------|------------|------------|------------|------------|------------|-----|-----|-----|-----|-----|-----|----|----|
| State  | 585 | 586 | 587 | 588 | 589 | 590 | 591      | 592      | 593      | 594      | 595      | 596      | 597      | 598      | 599      | 600      | 601      | 602      | 603        | 604        | 605        | 606        | 607        | 608        | 609        | 610        | 611        | 612        | 613        | 614        | 615 | 616 | 617 | 618 | 619 | 620 |    |    |
| Sz     | 1   | 0   | -1  | 1   | 0   | -1  | 1        | 0        | -1       | 1        | 0        | -1       | 1        | 0        | -1       | 1        | 0        | -1       | 1          | 0          | -1         | 1          | 0          | -1         | 1          | 0          | -1         | 1          | 0          | -1         | 1   | 0   | -1  | 1   | 0   | -1  |    |    |
| Rx     | 1   | 1   | 1   | 1   | 1   | 1   | 0        | 0        | 0        | 0        | 0        | 0        | 0        | 0        | 0        | 0        | 0        | 0        | 0          | 0          | 0          | 0          | 0          | 0          | 0          | 0          | 0          | 0          | 0          | 0          | -1  | -1  | -1  | -1  | -1  | -1  |    |    |
| Ry     | 1   | 1   | 1   | 1   | 1   | 1   | 0        | 0        | 0        | 0        | 0        | 0        | 0        | 0        | 0        | 0        | 0        | 0        | 0          | 0          | 0          | 0          | 0          | 0          | 0          | 0          | 0          | 0          | 0          | 0          | 0   | -1  | -1  | -1  | -1  | -1  | -1 |    |
| R      | -1  | -1  | -1  | -1  | -1  | -1  | <i>i</i> | <i>i</i> | <i>i</i> | <i>i</i> | <i>i</i> | <i>i</i> | <i>i</i> | <i>i</i> | <i>i</i> | <i>i</i> | <i>i</i> | <i>i</i> | - <i>i</i> | - <i>i</i> | - <i>i</i> | - <i>i</i> | - <i>i</i> | - <i>i</i> | - <i>i</i> | - <i>i</i> | - <i>i</i> | - <i>i</i> | - <i>i</i> | - <i>i</i> | 1   | 1   | 1   | 1   | 1   | 1   |    |    |
| Landau | B1  | B1  | B1  | B1  | B1  | B1  | E        | E        | E        | E        | E        | E        | E        | E        | E        | E        | E        | E        | E          | E          | E          | E          | E          | E          | E          | E          | E          | E          | E          | E          | E   | E   | A2  | A2  | A2  | A2  | A2 | A2 |

$$\mathbf{S} = \mathbf{0}, \mathbf{n}_{\text{occ.}} = \{4\}$$

$$\left( \begin{array}{cccccc} \text{State} & 621 & 622 & 623 & 624 & 625 \\ Sz & 0 & 0 & 0 & 0 & 0 \\ Rx & 1 & 1 & 1 & -1 & -1 \\ Ry & 1 & 1 & 1 & -1 & -1 \\ R & 1 & 1 & 1 & -1 & -1 \\ \text{Landau} & A1 & A1 & A1 & B2 & B2 \end{array} \right)$$

$$S = 6, \text{ n}_{\text{occ.}} = \{4, 0\}$$

[illegible]









$$\mathbf{S} = \mathbf{7}/\mathbf{2}, \mathbf{n}_{\text{occ.}} = \{\mathbf{3}, \mathbf{1}\}$$

[illegible]



$\mathbf{S} = \mathbf{3}, \mathbf{n}_{\text{occ.}} = \{\mathbf{2}, \mathbf{2}\}$

| State  | 275 | 276 | 277 | 278 | 279 | 280 | 281 | 282 | 283 | 284 | 285 | 286 | 287 | 288 | 289 | 290 | 291 | 292 | 293 | 294 | 295 | 296      | 297      | 298      | 299      | 300      | 301      | 302      | 303        | 304        | 305        | 306        | 307        | 308        | 309        | 310 | 311 | 312 | 313 | 314 | 315 | 316 |    |    |
|--------|-----|-----|-----|-----|-----|-----|-----|-----|-----|-----|-----|-----|-----|-----|-----|-----|-----|-----|-----|-----|-----|----------|----------|----------|----------|----------|----------|----------|------------|------------|------------|------------|------------|------------|------------|-----|-----|-----|-----|-----|-----|-----|----|----|
| Sz     | 3   | 2   | 1   | 0   | -1  | -2  | -3  | 3   | 2   | 1   | 0   | -1  | -2  | -3  | 3   | 2   | 1   | 0   | -1  | -2  | -3  | 3        | 2        | 1        | 0        | -1       | -2       | -3       | 3          | 2          | 1          | 0          | -1         | -2         | -3         | 3   | 2   | 1   | 0   | -1  | -2  | -3  |    |    |
| Rx     | 1   | 1   | 1   | 1   | 1   | 1   | 1   | 1   | 1   | 1   | 1   | 1   | 1   | 1   | 1   | 1   | 1   | 1   | 1   | 1   | 1   | 0        | 0        | 0        | 0        | 0        | 0        | 0        | 0          | 0          | 0          | 0          | 0          | 0          | 0          | 0   | -1  | -1  | -1  | -1  | -1  | -1  | -1 |    |
| Ry     | 1   | 1   | 1   | 1   | 1   | 1   | 1   | 1   | 1   | 1   | 1   | 1   | 1   | 1   | 1   | 1   | 1   | 1   | 1   | 1   | 1   | 0        | 0        | 0        | 0        | 0        | 0        | 0        | 0          | 0          | 0          | 0          | 0          | 0          | 0          | 0   | 0   | -1  | -1  | -1  | -1  | -1  | -1 | -1 |
| R      | 1   | 1   | 1   | 1   | 1   | 1   | 1   | 1   | 1   | 1   | 1   | 1   | 1   | 1   | -1  | -1  | -1  | -1  | -1  | -1  | -1  | <i>i</i> | <i>i</i> | <i>i</i> | <i>i</i> | <i>i</i> | <i>i</i> | <i>i</i> | - <i>i</i> | - <i>i</i> | - <i>i</i> | - <i>i</i> | - <i>i</i> | - <i>i</i> | - <i>i</i> | -1  | -1  | -1  | -1  | -1  | -1  | -1  |    |    |
| Landau | A1  | A1  | A1  | A1  | A1  | A1  | A1  | A1  | A1  | A1  | A1  | A1  | A1  | A1  | B1  | B1  | B1  | B1  | B1  | B1  | B1  | E        | E        | E        | E        | E        | E        | E        | E          | E          | E          | E          | E          | E          | E          | E   | E   | B2  | B2  | B2  | B2  | B2  | B2 | B2 |

$$\mathbf{S} = \mathbf{5}/\mathbf{2}, \mathbf{n}_{\text{occ.}} = \{\mathbf{3}, \mathbf{1}\}$$

[illegible]



$\mathbf{S} = \mathbf{2}, \mathbf{n}_{occ.} = \{\mathbf{2}, \mathbf{2}\}$

|        |     |     |     |     |     |     |     |     |     |     |     |     |     |     |     |      |      |      |      |      |      |      |      |      |      |     |     |     |     |     |    |
|--------|-----|-----|-----|-----|-----|-----|-----|-----|-----|-----|-----|-----|-----|-----|-----|------|------|------|------|------|------|------|------|------|------|-----|-----|-----|-----|-----|----|
| State  | 444 | 445 | 446 | 447 | 448 | 449 | 450 | 451 | 452 | 453 | 454 | 455 | 456 | 457 | 458 | 459  | 460  | 461  | 462  | 463  | 464  | 465  | 466  | 467  | 468  | 469 | 470 | 471 | 472 | 473 |    |
| Sz     | 2   | 1   | 0   | -1  | -2  | 2   | 1   | 0   | -1  | -2  | 2   | 1   | 0   | -1  | -2  | 2    | 1    | 0    | -1   | -2   | 2    | 1    | 0    | -1   | -2   | 2   | 1   | 0   | -1  | -2  |    |
| Rx     | 1   | 1   | 1   | 1   | 1   | 0   | 0   | 0   | 0   | 0   | 0   | 0   | 0   | 0   | 0   | 0    | 0    | 0    | 0    | 0    | 0    | 0    | 0    | 0    | 0    | 0   | -1  | -1  | -1  | -1  |    |
| Ry     | 1   | 1   | 1   | 1   | 1   | 0   | 0   | 0   | 0   | 0   | 0   | 0   | 0   | 0   | 0   | 0    | 0    | 0    | 0    | 0    | 0    | 0    | 0    | 0    | 0    | 0   | -1  | -1  | -1  | -1  |    |
| R      | -1  | -1  | -1  | -1  | -1  | $i$ | $i$ | $i$ | $i$ | $i$ | $i$ | $i$ | $i$ | $i$ | $i$ | $-i$ | $-i$ | $-i$ | $-i$ | $-i$ | $-i$ | $-i$ | $-i$ | $-i$ | $-i$ | 1   | 1   | 1   | 1   | 1   |    |
| Landau | B1  | B1  | B1  | B1  | B1  | E   | E   | E   | E   | E   | E   | E   | E   | E   | E   | E    | E    | E    | E    | E    | E    | E    | E    | E    | E    | E   | A2  | A2  | A2  | A2  | A2 |

$$\mathbf{S} = \mathbf{3}/\mathbf{2}, \mathbf{n}_{\text{occ.}} = \{\mathbf{3}, \mathbf{1}\}$$

[illegible]



$$\mathbf{S} = \mathbf{3}/\mathbf{2}, \mathbf{n}_{\text{occ.}} = \{\mathbf{1}, \mathbf{3}\}$$

| State  | 538           | 539           | 540            | 541            | 542           | 543           | 544            | 545            | 546           | 547           | 548            | 549            | 550           | 551           | 552            | 553            |
|--------|---------------|---------------|----------------|----------------|---------------|---------------|----------------|----------------|---------------|---------------|----------------|----------------|---------------|---------------|----------------|----------------|
| Sz     | $\frac{3}{2}$ | $\frac{1}{2}$ | $-\frac{1}{2}$ | $-\frac{3}{2}$ | $\frac{3}{2}$ | $\frac{1}{2}$ | $-\frac{1}{2}$ | $-\frac{3}{2}$ | $\frac{3}{2}$ | $\frac{1}{2}$ | $-\frac{1}{2}$ | $-\frac{3}{2}$ | $\frac{3}{2}$ | $\frac{1}{2}$ | $-\frac{1}{2}$ | $-\frac{3}{2}$ |
| Rx     | 1             | 1             | 1              | 1              | 1             | 1             | 1              | 1              | 0             | 0             | 0              | 0              | 0             | 0             | 0              | 0              |
| Ry     | 1             | 1             | 1              | 1              | 1             | 1             | 1              | 1              | 0             | 0             | 0              | 0              | 0             | 0             | 0              | 0              |
| R      | 1             | 1             | 1              | 1              | -1            | -1            | -1             | -1             | $i$           | $i$           | $i$            | $i$            | $-i$          | $-i$          | $-i$           | $-i$           |
| Landau | A1            | A1            | A1             | A1             | B1            | B1            | B1             | B1             | E             | E             | E              | E              | E             | E             | E              | E              |

$$\mathbf{S} = \mathbf{1}, \mathbf{n}_{\text{occ.}} = \{4, 0\}$$

| State  | 554 | 555 | 556 | 557 | 558 | 559 | 560 | 561 | 562 | 563 | 564 | 565 | 566 | 567 | 568 | 569 | 570  | 571  | 572  | 573  | 574  | 575  | 576  | 577  | 578 | 579 | 580 |    |
|--------|-----|-----|-----|-----|-----|-----|-----|-----|-----|-----|-----|-----|-----|-----|-----|-----|------|------|------|------|------|------|------|------|-----|-----|-----|----|
| Sz     | 1   | 0   | -1  | 1   | 0   | -1  | 1   | 0   | -1  | 1   | 0   | -1  | 1   | 0   | -1  | 1   | 0    | -1   | 1    | 0    | -1   | 1    | 0    | -1   | 1   | 0   | -1  |    |
| Rx     | 1   | 1   | 1   | 1   | 1   | 1   | 0   | 0   | 0   | 0   | 0   | 0   | 0   | 0   | 0   | 0   | 0    | 0    | 0    | 0    | 0    | 0    | 0    | 0    | -1  | -1  | -1  |    |
| Ry     | 1   | 1   | 1   | 1   | 1   | 1   | 0   | 0   | 0   | 0   | 0   | 0   | 0   | 0   | 0   | 0   | 0    | 0    | 0    | 0    | 0    | 0    | 0    | 0    | -1  | -1  | -1  |    |
| R      | -1  | -1  | -1  | -1  | -1  | -1  | $i$ | $i$ | $i$ | $i$ | $i$ | $i$ | $i$ | $i$ | $i$ | $i$ | $-i$ | $-i$ | $-i$ | $-i$ | $-i$ | $-i$ | $-i$ | $-i$ | 1   | 1   | 1   |    |
| Landau | B1  | B1  | B1  | B1  | B1  | B1  | E   | E   | E   | E   | E   | E   | E   | E   | E   | E   | E    | E    | E    | E    | E    | E    | E    | E    | E   | A2  | A2  | A2 |

$$S = 1, \text{ n}_{\text{occ.}} = \{2, 2\}$$

[illegible]

$$\mathbf{S} = \mathbf{1}/\mathbf{2}, \text{ } \mathbf{n}_{\text{occ.}} = \{\mathbf{3}, \mathbf{1}\}$$

| State  | 599           | 600            | 601           | 602            | 603           | 604            | 605           | 606            | 607           | 608            | 609           | 610            | 611           | 612            | 613           | 614            |    |    |
|--------|---------------|----------------|---------------|----------------|---------------|----------------|---------------|----------------|---------------|----------------|---------------|----------------|---------------|----------------|---------------|----------------|----|----|
| Sz     | $\frac{1}{2}$ | $-\frac{1}{2}$ | $\frac{1}{2}$ | $-\frac{1}{2}$ | $\frac{1}{2}$ | $-\frac{1}{2}$ | $\frac{1}{2}$ | $-\frac{1}{2}$ | $\frac{1}{2}$ | $-\frac{1}{2}$ | $\frac{1}{2}$ | $-\frac{1}{2}$ | $\frac{1}{2}$ | $-\frac{1}{2}$ | $\frac{1}{2}$ | $-\frac{1}{2}$ |    |    |
| Rx     | 1             | 1              | 1             | 1              | 0             | 0              | 0             | 0              | 0             | 0              | 0             | 0              | -1            | -1             | -1            | -1             |    |    |
| Ry     | 1             | 1              | 1             | 1              | 0             | 0              | 0             | 0              | 0             | 0              | 0             | 0              | -1            | -1             | -1            | -1             |    |    |
| R      | 1             | 1              | -1            | -1             | $i$           | $i$            | $i$           | $i$            | $-i$          | $-i$           | $-i$          | $-i$           | 1             | 1              | -1            | -1             |    |    |
| Landau | A1            | A1             | B1            | B1             | E             | E              | E             | E              | E             | E              | E             | E              | E             | E              | A2            | A2             | B2 | B2 |

$$\mathbf{S} = \mathbf{0}, \mathbf{n}_{\text{occ.}} = \{4, \mathbf{0}\}$$

$$\left( \begin{array}{ccccc} \text{State} & 615 & 616 & 617 & 618 \\ \text{Sz} & 0 & 0 & 0 & 0 \\ \text{Rx} & 1 & 1 & -1 & -1 \\ \text{Ry} & 1 & 1 & -1 & -1 \\ \text{R} & 1 & 1 & -1 & -1 \\ \text{Landau} & \text{A1} & \text{A1} & \text{B2} & \text{B2} \end{array} \right)$$

$$\mathbf{S} = \mathbf{0}, \text{ n}_{\text{occ.}} = \{\mathbf{2}, \mathbf{2}\}$$

| State  | 619 | 620      | 621      | 622        | 623        | 624 |
|--------|-----|----------|----------|------------|------------|-----|
| Sz     | 0   | 0        | 0        | 0          | 0          | 0   |
| Rx     | 1   | 0        | 0        | 0          | 0          | -1  |
| Ry     | 1   | 0        | 0        | 0          | 0          | -1  |
| R      | -1  | <i>i</i> | <i>i</i> | - <i>i</i> | - <i>i</i> | 1   |
| Landau | B1  | E        | E        | E          | E          | A2  |

$$\mathbf{S} = \mathbf{0}, \text{ n}_{\text{occ.}} = \{0, 4\}$$

$$\left( \begin{array}{cc} \text{State} & 625 \\ \text{Sz} & 0 \\ \text{Rx} & 1 \\ \text{Ry} & 1 \\ \text{R} & 1 \\ \text{Landau} & \text{A1} \end{array} \right)$$





$$\mathbf{S} = 7/2, \text{ n}_{\text{occ.}} = \{3, 1\}$$

[illegible]

$$S = 3, \text{ n}_{\text{occ.}} = \{4, 0\}$$

[illegible]

$$\mathbf{S} = \mathbf{3}, \mathbf{n}_{\text{occ.}} = \{\mathbf{2}, \mathbf{2}\}$$

|        |    |    |    |    |    |    |    |    |    |    |    |    |    |    |    |    |    |    |    |    |    |    |    |    |    |    |    |    |    |    |    |    |    |    |    |    |    |     |     |     |     |     |    |    |    |
|--------|----|----|----|----|----|----|----|----|----|----|----|----|----|----|----|----|----|----|----|----|----|----|----|----|----|----|----|----|----|----|----|----|----|----|----|----|----|-----|-----|-----|-----|-----|----|----|----|
| State  | 63 | 64 | 65 | 66 | 67 | 68 | 69 | 70 | 71 | 72 | 73 | 74 | 75 | 76 | 77 | 78 | 79 | 80 | 81 | 82 | 83 | 84 | 85 | 86 | 87 | 88 | 89 | 90 | 91 | 92 | 93 | 94 | 95 | 96 | 97 | 98 | 99 | 100 | 101 | 102 | 103 | 104 |    |    |    |
| Sz     | 3  | 2  | 1  | 0  | -1 | -2 | -3 | 3  | 2  | 1  | 0  | -1 | -2 | -3 | 3  | 2  | 1  | 0  | -1 | -2 | -3 | 3  | 2  | 1  | 0  | -1 | -2 | -3 | 3  | 2  | 1  | 0  | -1 | -2 | -3 | 3  | 2  | 1   | 0   | -1  | -2  | -3  |    |    |    |
| Rx     | 1  | 1  | 1  | 1  | 1  | 1  | 1  | 1  | 1  | 1  | 1  | 1  | 1  | 1  | 1  | 1  | 1  | 1  | 1  | 1  | 1  | 1  | 1  | 1  | 0  | 0  | 0  | 0  | 0  | 0  | 0  | 0  | 0  | 0  | 0  | 0  | -1 | -1  | -1  | -1  | -1  | -1  | -1 |    |    |
| Ry     | 1  | 1  | 1  | 1  | 1  | 1  | 1  | 1  | 1  | 1  | 1  | 1  | 1  | 1  | 1  | 1  | 1  | 1  | 1  | 1  | 1  | 1  | 1  | 1  | 0  | 0  | 0  | 0  | 0  | 0  | 0  | 0  | 0  | 0  | 0  | 0  | 0  | 0   | 0   | -1  | -1  | -1  | -1 | -1 | -1 |
| R      | 1  | 1  | 1  | 1  | 1  | 1  | 1  | 1  | 1  | 1  | 1  | 1  | 1  | 1  | -1 | -1 | -1 | -1 | -1 | -1 | -1 | -1 | -1 | i  | i  | i  | i  | i  | i  | -i | -i | -i | -i | -i | -i | -i | -1 | -1  | -1  | -1  | -1  | -1  | -1 |    |    |
| Landau | A1 | A1 | A1 | A1 | A1 | A1 | A1 | A1 | A1 | A1 | A1 | A1 | A1 | A1 | B1 | B1 | B1 | B1 | B1 | B1 | B1 | B1 | E  | E  | E  | E  | E  | E  | E  | E  | E  | E  | E  | E  | E  | E  | E  | B2  | B2  | B2  | B2  | B2  | B2 | B2 |    |

$$\mathbf{S} = \mathbf{5}/2, \mathbf{n}_{\text{occ.}} =$$

|        |               |
|--------|---------------|
| State  | 105           |
| Sz     | $\frac{5}{2}$ |
| Rx     | 1             |
| Ry     | 1             |
| R      | 1             |
| Landau | A1            |

[illegible]



$\mathbf{S} = \mathbf{2}, \mathbf{n}_{occ.} = \{4, \mathbf{0}\}$

| State  | 201 | 202 | 203 | 204 | 205 | 206 | 207 | 208 | 209 | 210 | 211 | 212 | 213 | 214 | 215 | 216 | 217 | 218 | 219 | 220 | 221  | 222  | 223  | 224  | 225  | 226  | 227 | 228 | 229 | 230 |
|--------|-----|-----|-----|-----|-----|-----|-----|-----|-----|-----|-----|-----|-----|-----|-----|-----|-----|-----|-----|-----|------|------|------|------|------|------|-----|-----|-----|-----|
| Sz     | 2   | 1   | 0   | -1  | -2  | 2   | 1   | 0   | -1  | -2  | 2   | 1   | 0   | -1  | -2  | 2   | 1   | 0   | -1  | -2  | 2    | 1    | 0    | -1   | -2   | 2    | 1   | 0   | -1  | -2  |
| Rx     | 1   | 1   | 1   | 1   | 1   | 1   | 1   | 1   | 1   | 1   | 1   | 1   | 1   | 1   | 1   | 0   | 0   | 0   | 0   | 0   | 0    | 0    | 0    | 0    | 0    | 0    | -1  | -1  | -1  | -1  |
| Ry     | 1   | 1   | 1   | 1   | 1   | 1   | 1   | 1   | 1   | 1   | 1   | 1   | 1   | 1   | 1   | 0   | 0   | 0   | 0   | 0   | 0    | 0    | 0    | 0    | 0    | 0    | -1  | -1  | -1  | -1  |
| R      | 1   | 1   | 1   | 1   | 1   | 1   | 1   | 1   | 1   | 1   | -1  | -1  | -1  | -1  | -1  | $i$ | $i$ | $i$ | $i$ | $i$ | $-i$ | $-i$ | $-i$ | $-i$ | $-i$ | $-i$ | -1  | -1  | -1  | -1  |
| Landau | A1  | A1  | A1  | A1  | A1  | A1  | A1  | A1  | A1  | A1  | B1  | B1  | B1  | B1  | B1  | E   | E   | E   | E   | E   | E    | E    | E    | E    | E    | E    | B2  | B2  | B2  | B2  |

$$S = 2, n_{\text{acc}} = \{2, 2\}$$

[illegible]

$$\mathbf{S} = \mathbf{2}, \mathbf{n}_{\text{occ.}} = \{0, 4\}$$

$$\left( \begin{array}{cccccc} \text{State} & 321 & 322 & 323 & 324 & 325 \\ \text{Sz} & 2 & 1 & 0 & -1 & -2 \\ \text{Rx} & 1 & 1 & 1 & 1 & 1 \\ \text{Ry} & 1 & 1 & 1 & 1 & 1 \\ \text{R} & 1 & 1 & 1 & 1 & 1 \\ \text{Landau} & \text{A1} & \text{A1} & \text{A1} & \text{A1} & \text{A1} \end{array} \right)$$





$$\mathbf{S} = \mathbf{3}/\mathbf{2}, \mathbf{n}_{\text{occ.}} = \{\mathbf{1}, \mathbf{3}\}$$

| State  | 406           | 407           | 408            | 409            | 410           | 411           | 412            | 413            | 414           | 415           | 416            | 417            | 418           | 419           | 420            | 421            | 422           | 423           | 424            | 425            | 426           | 427           | 428            | 429            | 430           | 431           | 432            | 433            | 434           | 435           | 436            | 437            | 438           | 439           | 440            | 441            | 442           | 443           | 444            | 445            | 446           | 447           | 448            | 449            | 450 | 451 | 452 | 453 |    |    |
|--------|---------------|---------------|----------------|----------------|---------------|---------------|----------------|----------------|---------------|---------------|----------------|----------------|---------------|---------------|----------------|----------------|---------------|---------------|----------------|----------------|---------------|---------------|----------------|----------------|---------------|---------------|----------------|----------------|---------------|---------------|----------------|----------------|---------------|---------------|----------------|----------------|---------------|---------------|----------------|----------------|---------------|---------------|----------------|----------------|-----|-----|-----|-----|----|----|
| Sz     | $\frac{3}{2}$ | $\frac{1}{2}$ | $-\frac{1}{2}$ | $-\frac{3}{2}$ | $\frac{3}{2}$ | $\frac{1}{2}$ | $-\frac{1}{2}$ | $-\frac{3}{2}$ | $\frac{3}{2}$ | $\frac{1}{2}$ | $-\frac{1}{2}$ | $-\frac{3}{2}$ | $\frac{3}{2}$ | $\frac{1}{2}$ | $-\frac{1}{2}$ | $-\frac{3}{2}$ | $\frac{3}{2}$ | $\frac{1}{2}$ | $-\frac{1}{2}$ | $-\frac{3}{2}$ | $\frac{3}{2}$ | $\frac{1}{2}$ | $-\frac{1}{2}$ | $-\frac{3}{2}$ | $\frac{3}{2}$ | $\frac{1}{2}$ | $-\frac{1}{2}$ | $-\frac{3}{2}$ | $\frac{3}{2}$ | $\frac{1}{2}$ | $-\frac{1}{2}$ | $-\frac{3}{2}$ | $\frac{3}{2}$ | $\frac{1}{2}$ | $-\frac{1}{2}$ | $-\frac{3}{2}$ | $\frac{3}{2}$ | $\frac{1}{2}$ | $-\frac{1}{2}$ | $-\frac{3}{2}$ | $\frac{3}{2}$ | $\frac{1}{2}$ | $-\frac{1}{2}$ | $-\frac{3}{2}$ |     |     |     |     |    |    |
| Rx     | 1             | 1             | 1              | 1              | 1             | 1             | 1              | 1              | 1             | 1             | 1              | 1              | 1             | 1             | 1              | 1              | 0             | 0             | 0              | 0              | 0             | 0             | 0              | 0              | 0             | 0             | 0              | 0              | 0             | 0             | 0              | 0              | 0             | 0             | 0              | 0              | 0             | 0             | 0              | -1             | -1            | -1            | -1             | -1             | -1  | -1  | -1  |     |    |    |
| Ry     | 1             | 1             | 1              | 1              | 1             | 1             | 1              | 1              | 1             | 1             | 1              | 1              | 1             | 1             | 1              | 1              | 0             | 0             | 0              | 0              | 0             | 0             | 0              | 0              | 0             | 0             | 0              | 0              | 0             | 0             | 0              | 0              | 0             | 0             | 0              | 0              | 0             | 0             | 0              | 0              | 0             | 0             | -1             | -1             | -1  | -1  | -1  | -1  | -1 | -1 |
| R      | 1             | 1             | 1              | 1              | 1             | 1             | 1              | 1              | -1            | -1            | -1             | -1             | -1            | -1            | -1             | -1             | $i$           | $i$           | $i$            | $i$            | $i$           | $i$           | $i$            | $i$            | $i$           | $i$           | $i$            | $i$            | $-i$          | $-i$          | $-i$           | $-i$           | $-i$          | $-i$          | $-i$           | $-i$           | $-i$          | $-i$          | $-i$           | 1              | 1             | 1             | 1              | -1             | -1  | -1  | -1  |     |    |    |
| Landau | A1            | A1            | A1             | A1             | A1            | A1            | A1             | A1             | B1            | B1            | B1             | B1             | B1            | B1            | B1             | B1             | E             | E             | E              | E              | E             | E             | E              | E              | E             | E             | E              | E              | E             | E             | E              | E              | E             | E             | E              | E              | E             | E             | E              | E              | A2            | A2            | A2             | A2             | B2  | B2  | B2  | B2  |    |    |

$$S = 1, \text{ n}_{\text{occ.}} = \{4, 0\}$$

$$\left( \begin{array}{cccccccccccccccccccccccc} \text{State} & 454 & 455 & 456 & 457 & 458 & 459 & 460 & 461 & 462 & 463 & 464 & 465 & 466 & 467 & 468 & 469 & 470 & 471 \\ \text{Sz} & 1 & 0 & -1 & 1 & 0 & -1 & 1 & 0 & -1 & 1 & 0 & -1 & 1 & 0 & -1 & 1 & 0 & -1 \\ \text{Rx} & 1 & 1 & 1 & 0 & 0 & 0 & 0 & 0 & 0 & 0 & 0 & 0 & 0 & 0 & 0 & -1 & -1 & -1 \\ \text{Ry} & 1 & 1 & 1 & 0 & 0 & 0 & 0 & 0 & 0 & 0 & 0 & 0 & 0 & 0 & 0 & -1 & -1 & -1 \\ \text{R} & -1 & -1 & -1 & i & i & i & i & i & i & -i & -i & -i & -i & -i & -i & 1 & 1 & 1 \\ \text{Landau} & \text{B1} & \text{B1} & \text{B1} & \text{E} & \text{E} & \text{E} & \text{E} & \text{E} & \text{E} & \text{E} & \text{E} & \text{E} & \text{E} & \text{E} & \text{E} & \text{A2} & \text{A2} & \text{A2} \end{array} \right)$$





$$\mathbf{S} = \mathbf{1}/2, \mathbf{n}_{\text{occ.}} = \{\mathbf{3}, \mathbf{1}\}$$

| State  | 553           | 554            | 555           | 556            | 557           | 558            | 559           | 560            | 561           | 562            | 563           | 564            | 565           | 566            | 567           | 568            | 569           | 570            | 571           | 572            | 573           | 574            | 575           | 576            | 577           | 578            | 579           | 580            | 581           | 582            | 583 | 584 |
|--------|---------------|----------------|---------------|----------------|---------------|----------------|---------------|----------------|---------------|----------------|---------------|----------------|---------------|----------------|---------------|----------------|---------------|----------------|---------------|----------------|---------------|----------------|---------------|----------------|---------------|----------------|---------------|----------------|---------------|----------------|-----|-----|
| Sz     | $\frac{1}{2}$ | $-\frac{1}{2}$ | $\frac{1}{2}$ | $-\frac{1}{2}$ | $\frac{1}{2}$ | $-\frac{1}{2}$ | $\frac{1}{2}$ | $-\frac{1}{2}$ | $\frac{1}{2}$ | $-\frac{1}{2}$ | $\frac{1}{2}$ | $-\frac{1}{2}$ | $\frac{1}{2}$ | $-\frac{1}{2}$ | $\frac{1}{2}$ | $-\frac{1}{2}$ | $\frac{1}{2}$ | $-\frac{1}{2}$ | $\frac{1}{2}$ | $-\frac{1}{2}$ | $\frac{1}{2}$ | $-\frac{1}{2}$ | $\frac{1}{2}$ | $-\frac{1}{2}$ | $\frac{1}{2}$ | $-\frac{1}{2}$ | $\frac{1}{2}$ | $-\frac{1}{2}$ | $\frac{1}{2}$ | $-\frac{1}{2}$ |     |     |
| Rx     | 1             | 1              | 1             | 1              | 1             | 1              | 1             | 1              | 0             | 0              | 0             | 0              | 0             | 0              | 0             | 0              | 0             | 0              | 0             | 0              | 0             | 0              | 0             | 0              | -1            | -1             | -1            | -1             | -1            | -1             | -1  |     |
| Ry     | 1             | 1              | 1             | 1              | 1             | 1              | 1             | 1              | 0             | 0              | 0             | 0              | 0             | 0              | 0             | 0              | 0             | 0              | 0             | 0              | 0             | 0              | 0             | 0              | -1            | -1             | -1            | -1             | -1            | -1             | -1  |     |
| R      | 1             | 1              | 1             | 1              | -1            | -1             | -1            | -1             | $i$           | $i$            | $i$           | $i$            | $i$           | $i$            | $i$           | $i$            | $-i$          | $-i$           | $-i$          | $-i$           | $-i$          | $-i$           | $-i$          | $-i$           | 1             | 1              | 1             | 1              | -1            | -1             | -1  |     |
| Landau | A1            | A1             | A1            | A1             | B1            | B1             | B1            | B1             | E             | E              | E             | E              | E             | E              | E             | E              | E             | E              | E             | E              | E             | E              | E             | E              | A2            | A2             | A2            | A2             | B2            | B2             | B2  | B2  |

$$\mathbf{S} = \mathbf{1}/2, \mathbf{n}_{\text{occ.}} = \{\mathbf{1}, \mathbf{3}\}$$

| State  | 585           | 586            | 587           | 588            | 589           | 590            | 591           | 592            | 593           | 594            | 595           | 596            | 597           | 598            | 599           | 600            | 601           | 602            | 603           | 604            | 605           | 606            | 607           | 608            |
|--------|---------------|----------------|---------------|----------------|---------------|----------------|---------------|----------------|---------------|----------------|---------------|----------------|---------------|----------------|---------------|----------------|---------------|----------------|---------------|----------------|---------------|----------------|---------------|----------------|
| Sz     | $\frac{1}{2}$ | $-\frac{1}{2}$ | $\frac{1}{2}$ | $-\frac{1}{2}$ | $\frac{1}{2}$ | $-\frac{1}{2}$ | $\frac{1}{2}$ | $-\frac{1}{2}$ | $\frac{1}{2}$ | $-\frac{1}{2}$ | $\frac{1}{2}$ | $-\frac{1}{2}$ | $\frac{1}{2}$ | $-\frac{1}{2}$ | $\frac{1}{2}$ | $-\frac{1}{2}$ | $\frac{1}{2}$ | $-\frac{1}{2}$ | $\frac{1}{2}$ | $-\frac{1}{2}$ | $\frac{1}{2}$ | $-\frac{1}{2}$ | $\frac{1}{2}$ | $-\frac{1}{2}$ |
| Rx     | 1             | 1              | 1             | 1              | 1             | 1              | 1             | 1              | 0             | 0              | 0             | 0              | 0             | 0              | 0             | 0              | 0             | 0              | 0             | 0              | -1            | -1             | -1            | -1             |
| Ry     | 1             | 1              | 1             | 1              | 1             | 1              | 1             | 1              | 0             | 0              | 0             | 0              | 0             | 0              | 0             | 0              | 0             | 0              | 0             | 0              | -1            | -1             | -1            | -1             |
| R      | 1             | 1              | 1             | 1              | -1            | -1             | -1            | -1             | $i$           | $i$            | $i$           | $i$            | $i$           | $i$            | $-i$          | $-i$           | $-i$          | $-i$           | $-i$          | $-i$           | 1             | 1              | -1            | -1             |
| Landau | A1            | A1             | A1            | A1             | B1            | B1             | B1            | B1             | E             | E              | E             | E              | E             | E              | E             | E              | E             | E              | E             | E              | A2            | A2             | B2            | B2             |

$$\mathbf{S} = \mathbf{0}, \text{ n}_{\text{occ.}} = \{4, \mathbf{0}\}$$

$$\left( \begin{array}{cccc} \text{State} & 609 & 610 & 611 \\ \text{Sz} & 0 & 0 & 0 \\ \text{Rx} & 1 & 1 & -1 \\ \text{Ry} & 1 & 1 & -1 \\ \text{R} & 1 & 1 & -1 \\ \text{Landau} & \text{A1} & \text{A1} & \text{B2} \end{array} \right)$$



$$\mathbf{S} = \mathbf{0}, \text{ n}_{\text{occ.}} = \{\mathbf{2}, \mathbf{2}\}$$

$$\left( \begin{array}{cccccccccccccc} \text{State} & 612 & 613 & 614 & 615 & 616 & 617 & 618 & 619 & 620 & 621 & 622 & 623 \\ \text{Sz} & 0 & 0 & 0 & 0 & 0 & 0 & 0 & 0 & 0 & 0 & 0 & 0 \\ \text{Rx} & 1 & 1 & 0 & 0 & 0 & 0 & 0 & 0 & 0 & 0 & -1 & -1 \\ \text{Ry} & 1 & 1 & 0 & 0 & 0 & 0 & 0 & 0 & 0 & 0 & -1 & -1 \\ \text{R} & -1 & -1 & i & i & i & i & -i & -i & -i & -i & 1 & 1 \\ \text{Landau} & \text{B1} & \text{B1} & \text{E} & \text{E} & \text{E} & \text{E} & \text{E} & \text{E} & \text{E} & \text{E} & \text{A2} & \text{A2} \end{array} \right)$$

$$\mathbf{S} = \mathbf{0}, \text{ n}_{\text{occ.}} = \{0, 4\}$$

$$\left( \begin{array}{ccc} \text{State} & 624 & 625 \\ \text{Sz} & 0 & 0 \\ \text{Rx} & 1 & -1 \\ \text{Ry} & 1 & -1 \\ \text{R} & 1 & -1 \\ \text{Landau} & \text{A1} & \text{B2} \end{array} \right)$$



$$S = 3, \text{ n}_{\text{occ.}} = \{4, 0, 0\}$$

[illegible]

$$\mathbf{S} = \mathbf{3}, \mathbf{n}_{\text{occ.}} = \{\mathbf{3}, \mathbf{1}, \mathbf{0}\}$$

[illegible]

$$\mathbf{S} = \mathbf{3}, \mathbf{n}_{\text{occ.}} = \{\mathbf{3}, \mathbf{0}, \mathbf{1}\}$$

[illegible]

$$\mathbf{S} = \mathbf{2}, \mathbf{n}_{\text{occ.}} = \{4, 0, 0\}$$

| State  | 87 | 88 | 89 | 90 | 91 | 92 | 93 | 94 | 95 | 96 | 97 | 98 | 99 | 100 | 101 | 102      | 103      | 104      | 105      | 106      | 107        | 108        | 109        | 110        | 111        | 112 | 113 | 114 | 115 | 116 |
|--------|----|----|----|----|----|----|----|----|----|----|----|----|----|-----|-----|----------|----------|----------|----------|----------|------------|------------|------------|------------|------------|-----|-----|-----|-----|-----|
| Sz     | 2  | 1  | 0  | -1 | -2 | 2  | 1  | 0  | -1 | -2 | 2  | 1  | 0  | -1  | -2  | 2        | 1        | 0        | -1       | -2       | 2          | 1          | 0          | -1         | -2         | 2   | 1   | 0   | -1  | -2  |
| Rx     | 1  | 1  | 1  | 1  | 1  | 1  | 1  | 1  | 1  | 1  | 1  | 1  | 1  | 1   | 1   | 0        | 0        | 0        | 0        | 0        | 0          | 0          | 0          | 0          | 0          | 0   | -1  | -1  | -1  | -1  |
| Ry     | 1  | 1  | 1  | 1  | 1  | 1  | 1  | 1  | 1  | 1  | 1  | 1  | 1  | 1   | 1   | 0        | 0        | 0        | 0        | 0        | 0          | 0          | 0          | 0          | 0          | 0   | -1  | -1  | -1  | -1  |
| R      | 1  | 1  | 1  | 1  | 1  | 1  | 1  | 1  | 1  | 1  | -1 | -1 | -1 | -1  | -1  | <i>i</i> | <i>i</i> | <i>i</i> | <i>i</i> | <i>i</i> | - <i>i</i> | - <i>i</i> | - <i>i</i> | - <i>i</i> | - <i>i</i> | -1  | -1  | -1  | -1  | -1  |
| Landau | A1 | A1 | A1 | A1 | A1 | A1 | A1 | A1 | A1 | A1 | B1 | B1 | B1 | B1  | B1  | E        | E        | E        | E        | E        | E          | E          | E          | E          | E          | E   | B2  | B2  | B2  | B2  |

$$\mathbf{S} = \mathbf{2}, \mathbf{n}_{\text{occ.}} = \{\mathbf{3}, \mathbf{1}, \mathbf{0}\}$$

|        |     |     |     |     |     |     |     |     |     |     |          |          |          |          |          |          |          |          |          |          |            |            |            |            |            |            |            |            |            |     |     |     |     |     |     |     |     |     |     |     |    |
|--------|-----|-----|-----|-----|-----|-----|-----|-----|-----|-----|----------|----------|----------|----------|----------|----------|----------|----------|----------|----------|------------|------------|------------|------------|------------|------------|------------|------------|------------|-----|-----|-----|-----|-----|-----|-----|-----|-----|-----|-----|----|
| State  | 117 | 118 | 119 | 120 | 121 | 122 | 123 | 124 | 125 | 126 | 127      | 128      | 129      | 130      | 131      | 132      | 133      | 134      | 135      | 136      | 137        | 138        | 139        | 140        | 141        | 142        | 143        | 144        | 145        | 146 | 147 | 148 | 149 | 150 | 151 | 152 | 153 | 154 | 155 | 156 |    |
| Sz     | 2   | 1   | 0   | -1  | -2  | 2   | 1   | 0   | -1  | -2  | 2        | 1        | 0        | -1       | -2       | 2        | 1        | 0        | -1       | -2       | 2          | 1          | 0          | -1         | -2         | 2          | 1          | 0          | -1         | -2  | 2   | 1   | 0   | -1  | -2  | 2   | 1   | 0   | -1  | -2  |    |
| Rx     | 1   | 1   | 1   | 1   | 1   | 1   | 1   | 1   | 1   | 1   | 0        | 0        | 0        | 0        | 0        | 0        | 0        | 0        | 0        | 0        | 0          | 0          | 0          | 0          | 0          | 0          | 0          | 0          | 0          | 0   | 0   | -1  | -1  | -1  | -1  | -1  | -1  | -1  | -1  | -1  |    |
| Ry     | 1   | 1   | 1   | 1   | 1   | 1   | 1   | 1   | 1   | 1   | 0        | 0        | 0        | 0        | 0        | 0        | 0        | 0        | 0        | 0        | 0          | 0          | 0          | 0          | 0          | 0          | 0          | 0          | 0          | 0   | 0   | 0   | 0   | -1  | -1  | -1  | -1  | -1  | -1  | -1  | -1 |
| R      | 1   | 1   | 1   | 1   | 1   | -1  | -1  | -1  | -1  | -1  | <i>i</i> | <i>i</i> | <i>i</i> | <i>i</i> | <i>i</i> | <i>i</i> | <i>i</i> | <i>i</i> | <i>i</i> | <i>i</i> | - <i>i</i> | - <i>i</i> | - <i>i</i> | - <i>i</i> | - <i>i</i> | - <i>i</i> | - <i>i</i> | - <i>i</i> | - <i>i</i> | 1   | 1   | 1   | 1   | 1   | -1  | -1  | -1  | -1  | -1  |     |    |
| Landau | A1  | A1  | A1  | A1  | A1  | B1  | B1  | B1  | B1  | B1  | E        | E        | E        | E        | E        | E        | E        | E        | E        | E        | E          | E          | E          | E          | E          | E          | E          | E          | E          | E   | E   | A2  | A2  | A2  | A2  | A2  | B2  | B2  | B2  | B2  | B2 |



$$\mathbf{S} = \mathbf{2}, \mathbf{n}_{\text{occ.}} = \{\mathbf{3}, \mathbf{0}, \mathbf{1}\}$$

|        |     |     |     |     |     |     |     |     |     |     |          |          |          |          |          |          |          |          |          |          |            |            |            |            |            |            |            |            |            |     |     |     |     |     |     |     |     |     |     |     |    |
|--------|-----|-----|-----|-----|-----|-----|-----|-----|-----|-----|----------|----------|----------|----------|----------|----------|----------|----------|----------|----------|------------|------------|------------|------------|------------|------------|------------|------------|------------|-----|-----|-----|-----|-----|-----|-----|-----|-----|-----|-----|----|
| State  | 157 | 158 | 159 | 160 | 161 | 162 | 163 | 164 | 165 | 166 | 167      | 168      | 169      | 170      | 171      | 172      | 173      | 174      | 175      | 176      | 177        | 178        | 179        | 180        | 181        | 182        | 183        | 184        | 185        | 186 | 187 | 188 | 189 | 190 | 191 | 192 | 193 | 194 | 195 | 196 |    |
| Sz     | 2   | 1   | 0   | -1  | -2  | 2   | 1   | 0   | -1  | -2  | 2        | 1        | 0        | -1       | -2       | 2        | 1        | 0        | -1       | -2       | 2          | 1          | 0          | -1         | -2         | 2          | 1          | 0          | -1         | -2  | 2   | 1   | 0   | -1  | -2  | 2   | 1   | 0   | -1  | -2  |    |
| Rx     | 1   | 1   | 1   | 1   | 1   | 1   | 1   | 1   | 1   | 1   | 0        | 0        | 0        | 0        | 0        | 0        | 0        | 0        | 0        | 0        | 0          | 0          | 0          | 0          | 0          | 0          | 0          | 0          | 0          | 0   | 0   | -1  | -1  | -1  | -1  | -1  | -1  | -1  | -1  | -1  |    |
| Ry     | 1   | 1   | 1   | 1   | 1   | 1   | 1   | 1   | 1   | 1   | 0        | 0        | 0        | 0        | 0        | 0        | 0        | 0        | 0        | 0        | 0          | 0          | 0          | 0          | 0          | 0          | 0          | 0          | 0          | 0   | 0   | 0   | -1  | -1  | -1  | -1  | -1  | -1  | -1  | -1  | -1 |
| R      | 1   | 1   | 1   | 1   | 1   | -1  | -1  | -1  | -1  | -1  | <i>i</i> | <i>i</i> | <i>i</i> | <i>i</i> | <i>i</i> | <i>i</i> | <i>i</i> | <i>i</i> | <i>i</i> | <i>i</i> | - <i>i</i> | - <i>i</i> | - <i>i</i> | - <i>i</i> | - <i>i</i> | - <i>i</i> | - <i>i</i> | - <i>i</i> | - <i>i</i> | 1   | 1   | 1   | 1   | 1   | -1  | -1  | -1  | -1  | -1  |     |    |
| Landau | A1  | A1  | A1  | A1  | A1  | B1  | B1  | B1  | B1  | B1  | E        | E        | E        | E        | E        | E        | E        | E        | E        | E        | E          | E          | E          | E          | E          | E          | E          | E          | E          | E   | E   | A2  | A2  | A2  | A2  | A2  | B2  | B2  | B2  | B2  | B2 |

$$\mathbf{S} = \mathbf{2}, \mathbf{n}_{\text{occ.}} = \{\mathbf{2}, \mathbf{2}, \mathbf{0}\}$$

| State  | 197 | 198 | 199 | 200 | 201 | 202 | 203 | 204 | 205 | 206 | 207 | 208 | 209 | 210 | 211 | 212 | 213 | 214 | 215 | 216 | 217  | 218  | 219  | 220  | 221  | 222  | 223 | 224 | 225 | 226 |
|--------|-----|-----|-----|-----|-----|-----|-----|-----|-----|-----|-----|-----|-----|-----|-----|-----|-----|-----|-----|-----|------|------|------|------|------|------|-----|-----|-----|-----|
| Sz     | 2   | 1   | 0   | -1  | -2  | 2   | 1   | 0   | -1  | -2  | 2   | 1   | 0   | -1  | -2  | 2   | 1   | 0   | -1  | -2  | 2    | 1    | 0    | -1   | -2   | 2    | 1   | 0   | -1  | -2  |
| Rx     | 1   | 1   | 1   | 1   | 1   | 1   | 1   | 1   | 1   | 1   | 1   | 1   | 1   | 1   | 1   | 0   | 0   | 0   | 0   | 0   | 0    | 0    | 0    | 0    | 0    | 0    | -1  | -1  | -1  | -1  |
| Ry     | 1   | 1   | 1   | 1   | 1   | 1   | 1   | 1   | 1   | 1   | 1   | 1   | 1   | 1   | 1   | 0   | 0   | 0   | 0   | 0   | 0    | 0    | 0    | 0    | 0    | 0    | -1  | -1  | -1  | -1  |
| R      | 1   | 1   | 1   | 1   | 1   | 1   | 1   | 1   | 1   | 1   | -1  | -1  | -1  | -1  | -1  | $i$ | $i$ | $i$ | $i$ | $i$ | $-i$ | $-i$ | $-i$ | $-i$ | $-i$ | $-i$ | -1  | -1  | -1  | -1  |
| Landau | A1  | A1  | A1  | A1  | A1  | A1  | A1  | A1  | A1  | A1  | B1  | B1  | B1  | B1  | B1  | E   | E   | E   | E   | E   | E    | E    | E    | E    | E    | E    | B2  | B2  | B2  | B2  |

$$\mathbf{S} = \mathbf{2}, \mathbf{n}_{\text{occ.}} = \{\mathbf{2}, \mathbf{1}, \mathbf{1}\}$$

[illegible]

$$\mathbf{S} = \mathbf{2}, \mathbf{n}_{\text{occ.}} = \{\mathbf{2}, \mathbf{0}, \mathbf{2}\}$$

| State  | 287 | 288 | 289 | 290 | 291 | 292 | 293 | 294 | 295 | 296 | 297 | 298 | 299 | 300 | 301 | 302 | 303      | 304      | 305      | 306      | 307      | 308        | 309        | 310        | 311        | 312        | 313 | 314 | 315 | 316 |
|--------|-----|-----|-----|-----|-----|-----|-----|-----|-----|-----|-----|-----|-----|-----|-----|-----|----------|----------|----------|----------|----------|------------|------------|------------|------------|------------|-----|-----|-----|-----|
| Sz     | 2   | 1   | 0   | -1  | -2  | 2   | 1   | 0   | -1  | -2  | 2   | 1   | 0   | -1  | -2  | 2   | 1        | 0        | -1       | -2       | 2        | 1          | 0          | -1         | -2         | 2          | 1   | 0   | -1  | -2  |
| Rx     | 1   | 1   | 1   | 1   | 1   | 1   | 1   | 1   | 1   | 1   | 1   | 1   | 1   | 1   | 1   | 1   | 0        | 0        | 0        | 0        | 0        | 0          | 0          | 0          | 0          | 0          | -1  | -1  | -1  | -1  |
| Ry     | 1   | 1   | 1   | 1   | 1   | 1   | 1   | 1   | 1   | 1   | 1   | 1   | 1   | 1   | 1   | 1   | 0        | 0        | 0        | 0        | 0        | 0          | 0          | 0          | 0          | 0          | -1  | -1  | -1  | -1  |
| R      | 1   | 1   | 1   | 1   | 1   | 1   | 1   | 1   | 1   | 1   | 1   | -1  | -1  | -1  | -1  | -1  | <i>i</i> | <i>i</i> | <i>i</i> | <i>i</i> | <i>i</i> | - <i>i</i> | - <i>i</i> | - <i>i</i> | - <i>i</i> | - <i>i</i> | -1  | -1  | -1  | -1  |
| Landau | A1  | A1  | A1  | A1  | A1  | A1  | A1  | A1  | A1  | A1  | B1  | B1  | B1  | B1  | B1  | B1  | E        | E        | E        | E        | E        | E          | E          | E          | E          | E          | B2  | B2  | B2  | B2  |

$$S = 1, \text{ n}_{\text{occ.}} = \{4, 0, 0\}$$

[illegible]

$\mathbf{S} = \mathbf{1}, \mathbf{n}_{\text{occ.}} = \{\mathbf{3}, \mathbf{1}, \mathbf{0}\}$

| State  | 335 | 336 | 337 | 338 | 339 | 340 | 341 | 342 | 343 | 344 | 345 | 346 | 347 | 348 | 349 | 350 | 351 | 352 | 353 | 354 | 355 | 356 | 357  | 358  | 359  | 360  | 361  | 362  | 363  | 364  | 365 | 366 | 367 | 368 | 369 | 370 |    |
|--------|-----|-----|-----|-----|-----|-----|-----|-----|-----|-----|-----|-----|-----|-----|-----|-----|-----|-----|-----|-----|-----|-----|------|------|------|------|------|------|------|------|-----|-----|-----|-----|-----|-----|----|
| Sz     | 1   | 0   | -1  | 1   | 0   | -1  | 1   | 0   | -1  | 1   | 0   | -1  | 1   | 0   | -1  | 1   | 0   | -1  | 1   | 0   | -1  | 1   | 0    | -1   | 1    | 0    | -1   | 1    | 0    | -1   | 1   | 0   | -1  | 1   | 0   | -1  |    |
| Rx     | 1   | 1   | 1   | 1   | 1   | 1   | 1   | 1   | 1   | 1   | 1   | 1   | 0   | 0   | 0   | 0   | 0   | 0   | 0   | 0   | 0   | 0   | 0    | 0    | 0    | 0    | 0    | 0    | 0    | 0    | 0   | -1  | -1  | -1  | -1  | -1  |    |
| Ry     | 1   | 1   | 1   | 1   | 1   | 1   | 1   | 1   | 1   | 1   | 1   | 1   | 0   | 0   | 0   | 0   | 0   | 0   | 0   | 0   | 0   | 0   | 0    | 0    | 0    | 0    | 0    | 0    | 0    | 0    | 0   | -1  | -1  | -1  | -1  | -1  |    |
| R      | 1   | 1   | 1   | 1   | 1   | 1   | -1  | -1  | -1  | -1  | -1  | -1  | $i$ | $i$ | $i$ | $i$ | $i$ | $i$ | $i$ | $i$ | $i$ | $i$ | $-i$ | $-i$ | $-i$ | $-i$ | $-i$ | $-i$ | $-i$ | $-i$ | 1   | 1   | 1   | -1  | -1  | -1  |    |
| Landau | A1  | A1  | A1  | A1  | A1  | A1  | B1  | B1  | B1  | B1  | B1  | B1  | E   | E   | E   | E   | E   | E   | E   | E   | E   | E   | E    | E    | E    | E    | E    | E    | E    | E    | E   | A2  | A2  | A2  | B2  | B2  | B2 |

$\mathbf{S} = \mathbf{1}, \mathbf{n}_{\text{occ.}} = \{\mathbf{3}, \mathbf{0}, \mathbf{1}\}$

|        |     |     |     |     |     |     |     |     |     |     |     |     |     |     |     |     |     |     |     |     |     |      |      |      |      |      |      |      |      |      |     |     |     |     |     |     |
|--------|-----|-----|-----|-----|-----|-----|-----|-----|-----|-----|-----|-----|-----|-----|-----|-----|-----|-----|-----|-----|-----|------|------|------|------|------|------|------|------|------|-----|-----|-----|-----|-----|-----|
| State  | 371 | 372 | 373 | 374 | 375 | 376 | 377 | 378 | 379 | 380 | 381 | 382 | 383 | 384 | 385 | 386 | 387 | 388 | 389 | 390 | 391 | 392  | 393  | 394  | 395  | 396  | 397  | 398  | 399  | 400  | 401 | 402 | 403 | 404 | 405 | 406 |
| Sz     | 1   | 0   | -1  | 1   | 0   | -1  | 1   | 0   | -1  | 1   | 0   | -1  | 1   | 0   | -1  | 1   | 0   | -1  | 1   | 0   | -1  | 1    | 0    | -1   | 1    | 0    | -1   | 1    | 0    | -1   | 1   | 0   | -1  | 1   | 0   | -1  |
| Rx     | 1   | 1   | 1   | 1   | 1   | 1   | 1   | 1   | 1   | 1   | 1   | 1   | 0   | 0   | 0   | 0   | 0   | 0   | 0   | 0   | 0   | 0    | 0    | 0    | 0    | 0    | 0    | 0    | 0    | 0    | -1  | -1  | -1  | -1  | -1  | -1  |
| Ry     | 1   | 1   | 1   | 1   | 1   | 1   | 1   | 1   | 1   | 1   | 1   | 1   | 0   | 0   | 0   | 0   | 0   | 0   | 0   | 0   | 0   | 0    | 0    | 0    | 0    | 0    | 0    | 0    | 0    | 0    | -1  | -1  | -1  | -1  | -1  | -1  |
| R      | 1   | 1   | 1   | 1   | 1   | 1   | -1  | -1  | -1  | -1  | -1  | -1  | $i$ | $i$ | $i$ | $i$ | $i$ | $i$ | $i$ | $i$ | $i$ | $-i$ | $-i$ | $-i$ | $-i$ | $-i$ | $-i$ | $-i$ | $-i$ | $-i$ | 1   | 1   | 1   | -1  | -1  | -1  |
| Landau | A1  | A1  | A1  | A1  | A1  | A1  | B1  | B1  | B1  | B1  | B1  | B1  | E   | E   | E   | E   | E   | E   | E   | E   | E   | E    | E    | E    | E    | E    | E    | E    | E    | E    | A2  | A2  | A2  | B2  | B2  | B2  |

$$S = 1, \text{ n}_{\text{occ.}} = \{2, 2, 0\}$$

$$\left( \begin{array}{c|cccccccccccccccccccc} \text{State} & 407 & 408 & 409 & 410 & 411 & 412 & 413 & 414 & 415 & 416 & 417 & 418 & 419 & 420 & 421 & 422 & 423 & 424 \\ \hline \text{Sz} & 1 & 0 & -1 & 1 & 0 & -1 & 1 & 0 & -1 & 1 & 0 & -1 & 1 & 0 & -1 & 1 & 0 & -1 \\ \text{Rx} & 1 & 1 & 1 & 0 & 0 & 0 & 0 & 0 & 0 & 0 & 0 & 0 & 0 & 0 & 0 & -1 & -1 & -1 \\ \text{Ry} & 1 & 1 & 1 & 0 & 0 & 0 & 0 & 0 & 0 & 0 & 0 & 0 & 0 & 0 & 0 & -1 & -1 & -1 \\ \text{R} & -1 & -1 & -1 & i & i & i & i & i & i & -i & -i & -i & -i & -i & -i & 1 & 1 & 1 \\ \text{Landau} & \text{B1} & \text{B1} & \text{B1} & \text{E} & \text{E} & \text{E} & \text{E} & \text{E} & \text{E} & \text{E} & \text{E} & \text{E} & \text{E} & \text{E} & \text{E} & \text{A2} & \text{A2} & \text{A2} \end{array} \right)$$



$\mathbf{S} = \mathbf{1}, \mathbf{n}_{\text{occ.}} = \{\mathbf{2}, \mathbf{1}, \mathbf{1}\}$

|        |     |     |     |     |     |     |          |          |          |          |          |          |          |          |          |            |            |            |            |            |            |            |            |            |     |     |     |     |     |     |     |     |     |     |     |     |
|--------|-----|-----|-----|-----|-----|-----|----------|----------|----------|----------|----------|----------|----------|----------|----------|------------|------------|------------|------------|------------|------------|------------|------------|------------|-----|-----|-----|-----|-----|-----|-----|-----|-----|-----|-----|-----|
| State  | 425 | 426 | 427 | 428 | 429 | 430 | 431      | 432      | 433      | 434      | 435      | 436      | 437      | 438      | 439      | 440        | 441        | 442        | 443        | 444        | 445        | 446        | 447        | 448        | 449 | 450 | 451 | 452 | 453 | 454 | 455 | 456 | 457 | 458 | 459 | 460 |
| Sz     | 1   | 0   | -1  | 1   | 0   | -1  | 1        | 0        | -1       | 1        | 0        | -1       | 1        | 0        | -1       | 1          | 0          | -1         | 1          | 0          | -1         | 1          | 0          | -1         | 1   | 0   | -1  | 1   | 0   | -1  | 1   | 0   | -1  | 1   | 0   | -1  |
| Rx     | 1   | 1   | 1   | 1   | 1   | 1   | 0        | 0        | 0        | 0        | 0        | 0        | 0        | 0        | 0        | 0          | 0          | 0          | 0          | 0          | 0          | 0          | 0          | 0          | -1  | -1  | -1  | -1  | -1  | -1  | -1  | -1  | -1  | -1  | -1  | -1  |
| Ry     | 1   | 1   | 1   | 1   | 1   | 1   | 0        | 0        | 0        | 0        | 0        | 0        | 0        | 0        | 0        | 0          | 0          | 0          | 0          | 0          | 0          | 0          | 0          | 0          | -1  | -1  | -1  | -1  | -1  | -1  | -1  | -1  | -1  | -1  | -1  | -1  |
| R      | 1   | 1   | 1   | -1  | -1  | -1  | <i>i</i> | <i>i</i> | <i>i</i> | <i>i</i> | <i>i</i> | <i>i</i> | <i>i</i> | <i>i</i> | <i>i</i> | - <i>i</i> | - <i>i</i> | - <i>i</i> | - <i>i</i> | - <i>i</i> | - <i>i</i> | - <i>i</i> | - <i>i</i> | - <i>i</i> | 1   | 1   | 1   | 1   | 1   | 1   | -1  | -1  | -1  | -1  | -1  |     |
| Landau | A1  | A1  | A1  | B1  | B1  | B1  | E        | E        | E        | E        | E        | E        | E        | E        | E        | E          | E          | E          | E          | E          | E          | E          | E          | E          | E   | A2  | A2  | A2  | A2  | A2  | A2  | B2  | B2  | B2  | B2  | B2  |

$$S = 1, \text{ n}_{\text{occ.}} = \{2, 0, 2\}$$

$$\left( \begin{array}{c|cccccccccccccccccccccccc} \text{State} & 461 & 462 & 463 & 464 & 465 & 466 & 467 & 468 & 469 & 470 & 471 & 472 & 473 & 474 & 475 & 476 & 477 & 478 \\ \hline \text{Sz} & 1 & 0 & -1 & 1 & 0 & -1 & 1 & 0 & -1 & 1 & 0 & -1 & 1 & 0 & -1 & 1 & 0 & -1 \\ \text{Rx} & 1 & 1 & 1 & 0 & 0 & 0 & 0 & 0 & 0 & 0 & 0 & 0 & 0 & 0 & 0 & -1 & -1 & -1 \\ \text{Ry} & 1 & 1 & 1 & 0 & 0 & 0 & 0 & 0 & 0 & 0 & 0 & 0 & 0 & 0 & 0 & -1 & -1 & -1 \\ \text{R} & -1 & -1 & -1 & i & i & i & i & i & i & -i & -i & -i & -i & -i & -i & 1 & 1 & 1 \\ \text{Landau} & \text{B1} & \text{B1} & \text{B1} & \text{E} & \text{E} & \text{E} & \text{E} & \text{E} & \text{E} & \text{E} & \text{E} & \text{E} & \text{E} & \text{E} & \text{E} & \text{A2} & \text{A2} & \text{A2} \end{array} \right)$$

$$\mathbf{S} = \mathbf{1}, \mathbf{n}_{\text{occ.}} = \{\mathbf{1}, \mathbf{3}, \mathbf{0}\}$$

$$\left( \begin{array}{c} \text{State} \\ \text{Sz} \\ \text{Rx} \\ \text{Ry} \\ \text{R} \\ \text{Landau} \end{array} \begin{array}{cccccccccccccccc} 479 & 480 & 481 & 482 & 483 & 484 & 485 & 486 & 487 & 488 & 489 & 490 \\ 1 & 0 & -1 & 1 & 0 & -1 & 1 & 0 & -1 & 1 & 0 & -1 \\ 1 & 1 & 1 & 1 & 1 & 1 & 0 & 0 & 0 & 0 & 0 & 0 \\ 1 & 1 & 1 & 1 & 1 & 1 & 0 & 0 & 0 & 0 & 0 & 0 \\ 1 & 1 & 1 & -1 & -1 & -1 & i & i & i & -i & -i & -i \\ A1 & A1 & A1 & B1 & B1 & B1 & E & E & E & E & E & E \end{array} \right)$$

$\mathbf{S} = \mathbf{1}, \mathbf{n}_{\text{occ.}} = \{\mathbf{1}, \mathbf{2}, \mathbf{1}\}$

| State  | 491 | 492 | 493 | 494 | 495 | 496 | 497 | 498 | 499 | 500 | 501 | 502 | 503      | 504      | 505      | 506      | 507      | 508      | 509      | 510      | 511      | 512        | 513        | 514        | 515        | 516        | 517        | 518        | 519        | 520 | 521 | 522 | 523 | 524 | 525 | 526 |
|--------|-----|-----|-----|-----|-----|-----|-----|-----|-----|-----|-----|-----|----------|----------|----------|----------|----------|----------|----------|----------|----------|------------|------------|------------|------------|------------|------------|------------|------------|-----|-----|-----|-----|-----|-----|-----|
| Sz     | 1   | 0   | -1  | 1   | 0   | -1  | 1   | 0   | -1  | 1   | 0   | -1  | 1        | 0        | -1       | 1        | 0        | -1       | 1        | 0        | -1       | 1          | 0          | -1         | 1          | 0          | -1         | 1          | 0          | -1  | 1   | 0   | -1  | 1   | 0   | -1  |
| Rx     | 1   | 1   | 1   | 1   | 1   | 1   | 1   | 1   | 1   | 1   | 1   | 1   | 0        | 0        | 0        | 0        | 0        | 0        | 0        | 0        | 0        | 0          | 0          | 0          | 0          | 0          | 0          | 0          | 0          | -1  | -1  | -1  | -1  | -1  | -1  |     |
| Ry     | 1   | 1   | 1   | 1   | 1   | 1   | 1   | 1   | 1   | 1   | 1   | 1   | 0        | 0        | 0        | 0        | 0        | 0        | 0        | 0        | 0        | 0          | 0          | 0          | 0          | 0          | 0          | 0          | 0          | 0   | -1  | -1  | -1  | -1  | -1  | -1  |
| R      | 1   | 1   | 1   | 1   | 1   | 1   | -1  | -1  | -1  | -1  | -1  | -1  | <i>i</i> | <i>i</i> | <i>i</i> | <i>i</i> | <i>i</i> | <i>i</i> | <i>i</i> | <i>i</i> | <i>i</i> | - <i>i</i> | - <i>i</i> | - <i>i</i> | - <i>i</i> | - <i>i</i> | - <i>i</i> | - <i>i</i> | - <i>i</i> | 1   | 1   | 1   | -1  | -1  | -1  |     |
| Landau | A1  | A1  | A1  | A1  | A1  | A1  | B1  | B1  | B1  | B1  | B1  | B1  | E        | E        | E        | E        | E        | E        | E        | E        | E        | E          | E          | E          | E          | E          | E          | E          | E          | A2  | A2  | A2  | B2  | B2  | B2  |     |

$\mathbf{S} = \mathbf{1}, \mathbf{n}_{\text{occ.}} = \{\mathbf{1}, \mathbf{1}, \mathbf{2}\}$

|        |     |     |     |     |     |     |     |     |     |     |     |     |     |     |     |     |     |     |     |     |     |     |      |      |      |      |      |      |      |      |     |     |     |     |     |     |
|--------|-----|-----|-----|-----|-----|-----|-----|-----|-----|-----|-----|-----|-----|-----|-----|-----|-----|-----|-----|-----|-----|-----|------|------|------|------|------|------|------|------|-----|-----|-----|-----|-----|-----|
| State  | 527 | 528 | 529 | 530 | 531 | 532 | 533 | 534 | 535 | 536 | 537 | 538 | 539 | 540 | 541 | 542 | 543 | 544 | 545 | 546 | 547 | 548 | 549  | 550  | 551  | 552  | 553  | 554  | 555  | 556  | 557 | 558 | 559 | 560 | 561 | 562 |
| Sz     | 1   | 0   | -1  | 1   | 0   | -1  | 1   | 0   | -1  | 1   | 0   | -1  | 1   | 0   | -1  | 1   | 0   | -1  | 1   | 0   | -1  | 1   | 0    | -1   | 1    | 0    | -1   | 1    | 0    | -1   | 1   | 0   | -1  | 1   | 0   | -1  |
| Rx     | 1   | 1   | 1   | 1   | 1   | 1   | 1   | 1   | 1   | 1   | 1   | 1   | 0   | 0   | 0   | 0   | 0   | 0   | 0   | 0   | 0   | 0   | 0    | 0    | 0    | 0    | 0    | 0    | 0    | 0    | -1  | -1  | -1  | -1  | -1  | -1  |
| Ry     | 1   | 1   | 1   | 1   | 1   | 1   | 1   | 1   | 1   | 1   | 1   | 1   | 0   | 0   | 0   | 0   | 0   | 0   | 0   | 0   | 0   | 0   | 0    | 0    | 0    | 0    | 0    | 0    | 0    | 0    | -1  | -1  | -1  | -1  | -1  | -1  |
| R      | 1   | 1   | 1   | 1   | 1   | 1   | -1  | -1  | -1  | -1  | -1  | -1  | $i$ | $i$ | $i$ | $i$ | $i$ | $i$ | $i$ | $i$ | $i$ | $i$ | $-i$ | $-i$ | $-i$ | $-i$ | $-i$ | $-i$ | $-i$ | $-i$ | 1   | 1   | 1   | -1  | -1  | -1  |
| Landau | A1  | A1  | A1  | A1  | A1  | A1  | B1  | B1  | B1  | B1  | B1  | B1  | E   | E   | E   | E   | E   | E   | E   | E   | E   | E   | E    | E    | E    | E    | E    | E    | E    | E    | A2  | A2  | A2  | B2  | B2  | B2  |



$$\mathbf{S} = \mathbf{0}, \text{ n}_{\text{occ.}} = \{4, \mathbf{0}, \mathbf{0}\}$$

$$\left( \begin{array}{cccc} \text{State} & 575 & 576 & 577 \\ \text{Sz} & 0 & 0 & 0 \\ \text{Rx} & 1 & 1 & -1 \\ \text{Ry} & 1 & 1 & -1 \\ \text{R} & 1 & 1 & -1 \\ \text{Landau} & \text{A1} & \text{A1} & \text{B2} \end{array} \right)$$

$$\mathbf{S} = \mathbf{0}, \text{ n}_{\text{occ.}} = \{\mathbf{3}, \mathbf{1}, \mathbf{0}\}$$

$$\left( \begin{array}{ccccc} \text{State} & 578 & 579 & 580 & 581 \\ \text{Sz} & 0 & 0 & 0 & 0 \\ \text{Rx} & 0 & 0 & -1 & -1 \\ \text{Ry} & 0 & 0 & -1 & -1 \\ \text{R} & i & -i & 1 & -1 \\ \text{Landau} & \text{E} & \text{E} & \text{A2} & \text{B2} \end{array} \right)$$



$$\mathbf{S} = \mathbf{0}, \text{ n}_{\text{occ.}} = \{\mathbf{3}, \mathbf{0}, \mathbf{1}\}$$

$$\left( \begin{array}{ccccc} \text{State} & 582 & 583 & 584 & 585 \\ \text{Sz} & 0 & 0 & 0 & 0 \\ \text{Rx} & 0 & 0 & -1 & -1 \\ \text{Ry} & 0 & 0 & -1 & -1 \\ \text{R} & i & -i & 1 & -1 \\ \text{Landau} & \text{E} & \text{E} & \text{A2} & \text{B2} \end{array} \right)$$

$$\mathbf{S} = \mathbf{0}, \text{ n}_{\text{occ.}} = \{\mathbf{2}, \mathbf{2}, \mathbf{0}\}$$

| State  | 586 | 587 | 588 | 589 | 590  | 591 |
|--------|-----|-----|-----|-----|------|-----|
| Sz     | 0   | 0   | 0   | 0   | 0    | 0   |
| Rx     | 1   | 1   | 1   | 0   | 0    | -1  |
| Ry     | 1   | 1   | 1   | 0   | 0    | -1  |
| R      | 1   | 1   | -1  | $i$ | $-i$ | -1  |
| Landau | A1  | A1  | B1  | E   | E    | B2  |

$$\mathbf{S} = \mathbf{0}, \mathbf{n}_{\text{occ.}} = \{\mathbf{2}, \mathbf{1}, \mathbf{1}\}$$

| State  | 592 | 593 | 594 | 595 | 596 | 597 | 598 | 599  | 600  | 601  | 602 | 603 |
|--------|-----|-----|-----|-----|-----|-----|-----|------|------|------|-----|-----|
| Sz     | 0   | 0   | 0   | 0   | 0   | 0   | 0   | 0    | 0    | 0    | 0   | 0   |
| Rx     | 1   | 1   | 1   | 1   | 0   | 0   | 0   | 0    | 0    | 0    | -1  | -1  |
| Ry     | 1   | 1   | 1   | 1   | 0   | 0   | 0   | 0    | 0    | 0    | -1  | -1  |
| R      | 1   | 1   | -1  | -1  | $i$ | $i$ | $i$ | $-i$ | $-i$ | $-i$ | 1   | -1  |
| Landau | A1  | A1  | B1  | B1  | E   | E   | E   | E    | E    | E    | A2  | B2  |

$$\mathbf{S} = \mathbf{0}, \mathbf{n}_{\text{occ.}} = \{\mathbf{2}, \mathbf{0}, \mathbf{2}\}$$

| State  | 604 | 605 | 606 | 607 | 608  | 609 |
|--------|-----|-----|-----|-----|------|-----|
| Sz     | 0   | 0   | 0   | 0   | 0    | 0   |
| Rx     | 1   | 1   | 1   | 0   | 0    | -1  |
| Ry     | 1   | 1   | 1   | 0   | 0    | -1  |
| R      | 1   | 1   | -1  | $i$ | $-i$ | -1  |
| Landau | A1  | A1  | B1  | E   | E    | B2  |

$$\mathbf{S} = \mathbf{0}, \text{ n}_{\text{occ.}} = \{0, 4, 0\}$$

$$\left( \begin{array}{cc} \text{State} & 610 \\ \text{Sz} & 0 \\ \text{Rx} & 1 \\ \text{Ry} & 1 \\ \text{R} & 1 \\ \text{Landau} & \text{A1} \end{array} \right)$$

$$\mathbf{S} = \mathbf{0}, \text{ n}_{\text{occ.}} = \{\mathbf{0}, \mathbf{3}, \mathbf{1}\}$$

$$\left( \begin{array}{ccccc} \text{State} & 611 & 612 & 613 & 614 \\ \text{Sz} & 0 & 0 & 0 & 0 \\ \text{Rx} & 1 & 1 & 0 & 0 \\ \text{Ry} & 1 & 1 & 0 & 0 \\ \text{R} & 1 & -1 & i & -i \\ \text{Landau} & \text{A1} & \text{B1} & \text{E} & \text{E} \end{array} \right)$$

$$\mathbf{S} = \mathbf{0}, \mathbf{n}_{\text{occ.}} = \{\mathbf{0}, \mathbf{2}, \mathbf{2}\}$$

| State  | 615 | 616 | 617 | 618 | 619  | 620 |
|--------|-----|-----|-----|-----|------|-----|
| Sz     | 0   | 0   | 0   | 0   | 0    | 0   |
| Rx     | 1   | 1   | 1   | 0   | 0    | -1  |
| Ry     | 1   | 1   | 1   | 0   | 0    | -1  |
| R      | 1   | 1   | -1  | $i$ | $-i$ | -1  |
| Landau | A1  | A1  | B1  | E   | E    | B2  |

$$\mathbf{S} = \mathbf{0}, \text{ n}_{\text{occ.}} = \{\mathbf{0}, \mathbf{1}, \mathbf{3}\}$$

$$\left( \begin{array}{ccccc} \text{State} & 621 & 622 & 623 & 624 \\ \text{Sz} & 0 & 0 & 0 & 0 \\ \text{Rx} & 1 & 1 & 0 & 0 \\ \text{Ry} & 1 & 1 & 0 & 0 \\ \text{R} & 1 & -1 & i & -i \\ \text{Landau} & \text{A1} & \text{B1} & \text{E} & \text{E} \end{array} \right)$$



$$\mathbf{S} = \mathbf{0}, \text{ n}_{\text{occ.}} = \{0, 0, 4\}$$

$$\left( \begin{array}{cc} \text{State} & 625 \\ \text{Sz} & 0 \\ \text{Rx} & 1 \\ \text{Ry} & 1 \\ \text{R} & 1 \\ \text{Landau} & \text{A1} \end{array} \right)$$

$$\mathbf{S} = \mathbf{2}, \mathbf{n}_{\text{occ.}} = \{4, 0, 0\}$$

$$\left( \begin{array}{ccccc} \text{State} & 1 & 2 & 3 & 4 & 5 \\ \text{Sz} & 2 & 1 & 0 & -1 & -2 \\ \text{Rx} & 1 & 1 & 1 & 1 & 1 \\ \text{Ry} & 1 & 1 & 1 & 1 & 1 \\ \text{R} & 1 & 1 & 1 & 1 & 1 \\ \text{Landau} & \text{A1} & \text{A1} & \text{A1} & \text{A1} & \text{A1} \end{array} \right)$$



$$\mathbf{S} = \mathbf{2}, \mathbf{n}_{\text{occ.}} = \{\mathbf{2}, \mathbf{2}, \mathbf{0}\}$$

| State  | 26 | 27 | 28 | 29 | 30 | 31 | 32 | 33 | 34 | 35 | 36 | 37 | 38 | 39 | 40 | 41       | 42       | 43       | 44       | 45       | 46         | 47         | 48         | 49         | 50         | 51 | 52 | 53 | 54 | 55 |
|--------|----|----|----|----|----|----|----|----|----|----|----|----|----|----|----|----------|----------|----------|----------|----------|------------|------------|------------|------------|------------|----|----|----|----|----|
| Sz     | 2  | 1  | 0  | -1 | -2 | 2  | 1  | 0  | -1 | -2 | 2  | 1  | 0  | -1 | -2 | 2        | 1        | 0        | -1       | -2       | 2          | 1          | 0          | -1         | -2         | 2  | 1  | 0  | -1 | -2 |
| Rx     | 1  | 1  | 1  | 1  | 1  | 1  | 1  | 1  | 1  | 1  | 1  | 1  | 1  | 1  | 1  | 0        | 0        | 0        | 0        | 0        | 0          | 0          | 0          | 0          | 0          | -1 | -1 | -1 | -1 | -1 |
| Ry     | 1  | 1  | 1  | 1  | 1  | 1  | 1  | 1  | 1  | 1  | 1  | 1  | 1  | 1  | 1  | 0        | 0        | 0        | 0        | 0        | 0          | 0          | 0          | 0          | 0          | -1 | -1 | -1 | -1 | -1 |
| R      | 1  | 1  | 1  | 1  | 1  | 1  | 1  | 1  | 1  | 1  | -1 | -1 | -1 | -1 | -1 | <i>i</i> | <i>i</i> | <i>i</i> | <i>i</i> | <i>i</i> | - <i>i</i> | - <i>i</i> | - <i>i</i> | - <i>i</i> | - <i>i</i> | -1 | -1 | -1 | -1 | -1 |
| Landau | A1 | A1 | A1 | A1 | A1 | A1 | A1 | A1 | A1 | A1 | B1 | B1 | B1 | B1 | B1 | E        | E        | E        | E        | E        | E          | E          | E          | E          | E          | B2 | B2 | B2 | B2 | B2 |

$$\mathbf{S} = \mathbf{2}, \mathbf{n}_{\text{occ.}} = \{1, 3, 0\}$$

[illegible]

$$\mathbf{S} = \mathbf{2}, \mathbf{n}_{\text{occ.}} = \{\mathbf{0}, \mathbf{4}, \mathbf{0}\}$$

$$\left( \begin{array}{cccccc} \text{State} & 76 & 77 & 78 & 79 & 80 \\ \text{Sz} & 2 & 1 & 0 & -1 & -2 \\ \text{Rx} & 1 & 1 & 1 & 1 & 1 \\ \text{Ry} & 1 & 1 & 1 & 1 & 1 \\ \text{R} & 1 & 1 & 1 & 1 & 1 \\ \text{Landau} & \text{A1} & \text{A1} & \text{A1} & \text{A1} & \text{A1} \end{array} \right)$$

$$\mathbf{S} = \mathbf{3}/\mathbf{2}, \text{ n}_{\text{occ.}} = \{\mathbf{3}, \mathbf{0}, \mathbf{1}\}$$

| State  | 81            | 82            | 83             | 84             | 85            | 86            | 87             | 88             | 89            | 90            | 91             | 92             | 93            | 94            | 95             | 96             |
|--------|---------------|---------------|----------------|----------------|---------------|---------------|----------------|----------------|---------------|---------------|----------------|----------------|---------------|---------------|----------------|----------------|
| Sz     | $\frac{3}{2}$ | $\frac{1}{2}$ | $-\frac{1}{2}$ | $-\frac{3}{2}$ | $\frac{3}{2}$ | $\frac{1}{2}$ | $-\frac{1}{2}$ | $-\frac{3}{2}$ | $\frac{3}{2}$ | $\frac{1}{2}$ | $-\frac{1}{2}$ | $-\frac{3}{2}$ | $\frac{3}{2}$ | $\frac{1}{2}$ | $-\frac{1}{2}$ | $-\frac{3}{2}$ |
| Rx     | 1             | 1             | 1              | 1              | 1             | 1             | 1              | 1              | 0             | 0             | 0              | 0              | 0             | 0             | 0              | 0              |
| Ry     | 1             | 1             | 1              | 1              | 1             | 1             | 1              | 1              | 0             | 0             | 0              | 0              | 0             | 0             | 0              | 0              |
| R      | 1             | 1             | 1              | 1              | -1            | -1            | -1             | -1             | $i$           | $i$           | $i$            | $i$            | $-i$          | $-i$          | $-i$           | $-i$           |
| Landau | A1            | A1            | A1             | A1             | B1            | B1            | B1             | B1             | E             | E             | E              | E              | E             | E             | E              | E              |

$$\mathbf{S} = \mathbf{3}/\mathbf{2}, \mathbf{n}_{\text{occ.}} = \{\mathbf{2}, \mathbf{1}, \mathbf{1}\}$$

$$\left( \begin{array}{cc} \text{State} & 97 \quad 98 \quad 99 \quad 100 \quad 101 \quad 102 \quad 103 \quad 104 \quad 105 \quad 106 \quad 107 \quad 108 \quad 109 \quad 110 \quad 111 \quad 112 \quad 113 \quad 114 \quad 115 \quad 116 \quad 117 \quad 118 \quad 119 \quad 120 \quad 121 \quad 122 \quad 123 \quad 124 \quad 125 \quad 126 \quad 127 \quad 128 \quad 129 \quad 130 \quad 131 \quad 132 \quad 133 \quad 134 \quad 135 \quad 136 \quad 137 \quad 138 \quad 139 \quad 140 \quad 141 \quad 142 \quad 143 \quad 144 \\ \text{Sz} & \frac{3}{2} \quad \frac{1}{2} \quad -\frac{1}{2} \quad -\frac{3}{2} \quad \frac{3}{2} \quad \frac{1}{2} \quad -\frac{1}{2} \quad -\frac{3}{2} \quad \frac{3}{2} \quad \frac{1}{2} \quad -\frac{1}{2} \quad -\frac{3}{2} \quad \frac{3}{2} \quad \frac{1}{2} \quad -\frac{1}{2} \quad -\frac{3}{2} \quad \frac{3}{2} \quad \frac{1}{2} \quad -\frac{1}{2} \quad -\frac{3}{2} \quad \frac{3}{2} \quad \frac{1}{2} \quad -\frac{1}{2} \quad -\frac{3}{2} \quad \frac{3}{2} \quad \frac{1}{2} \quad -\frac{1}{2} \quad -\frac{3}{2} \quad \frac{3}{2} \quad \frac{1}{2} \quad -\frac{1}{2} \quad -\frac{3}{2} \quad \frac{3}{2} \quad \frac{1}{2} \quad -\frac{1}{2} \quad -\frac{3}{2} \quad \frac{3}{2} \quad \frac{1}{2} \quad -\frac{1}{2} \quad -\frac{3}{2} \quad \frac{3}{2} \quad \frac{1}{2} \quad -\frac{1}{2} \quad -\frac{3}{2} \\ \text{Rx} & 1 \quad 1 \quad 1 \quad 1 \quad 1 \quad 1 \quad 1 \quad 1 \quad 1 \quad 1 \quad 1 \quad 1 \quad 1 \quad 1 \quad 1 \quad 1 \quad 0 \quad 0 \quad 0 \quad 0 \quad 0 \quad 0 \quad 0 \quad 0 \quad 0 \quad 0 \quad 0 \quad 0 \quad 0 \quad 0 \quad 0 \quad 0 \quad 0 \quad 0 \quad 0 \quad 0 \quad 0 \quad 0 \quad 0 \quad -1 \quad -1 \quad -1 \quad -1 \quad -1 \quad -1 \quad -1 \quad -1 \\ \text{Ry} & 1 \quad 1 \quad 1 \quad 1 \quad 1 \quad 1 \quad 1 \quad 1 \quad 1 \quad 1 \quad 1 \quad 1 \quad 1 \quad 1 \quad 1 \quad 1 \quad 0 \quad 0 \quad 0 \quad 0 \quad 0 \quad 0 \quad 0 \quad 0 \quad 0 \quad 0 \quad 0 \quad 0 \quad 0 \quad 0 \quad 0 \quad 0 \quad 0 \quad 0 \quad 0 \quad 0 \quad 0 \quad 0 \quad 0 \quad -1 \quad -1 \quad -1 \quad -1 \quad -1 \quad -1 \quad -1 \quad -1 \\ \text{R} & 1 \quad 1 \quad 1 \quad 1 \quad 1 \quad 1 \quad 1 \quad 1 \quad 1 \quad -1 \quad -1 \quad -1 \quad -1 \quad -1 \quad -1 \quad -1 \quad -1 \quad i \quad i \quad i \quad i \quad i \quad i \quad i \quad i \quad i \quad i \quad i \quad -i \quad -i \quad -i \quad -i \quad -i \quad -i \quad -i \quad -i \quad -i \quad -i \quad 1 \quad 1 \quad 1 \quad 1 \quad -1 \quad -1 \quad -1 \quad -1 \\ \text{Landau} & \text{A1} \quad \text{A1} \quad \text{A1} \quad \text{A1} \quad \text{A1} \quad \text{A1} \quad \text{A1} \quad \text{A1} \quad \text{A1} \quad \text{B1} \quad \text{B1} \quad \text{B1} \quad \text{B1} \quad \text{B1} \quad \text{B1} \quad \text{B1} \quad \text{B1} \quad \text{E} \quad \text{E} \quad \text{E} \quad \text{E} \quad \text{E} \quad \text{E} \quad \text{E} \quad \text{E} \quad \text{E} \quad \text{E} \quad \text{E} \quad \text{E} \quad \text{E} \quad \text{E} \quad \text{E} \quad \text{E} \quad \text{E} \quad \text{E} \quad \text{E} \quad \text{E} \quad \text{E} \quad \text{E} \quad \text{E} \quad \text{A2} \quad \text{A2} \quad \text{A2} \quad \text{A2} \quad \text{B2} \quad \text{B2} \quad \text{B2} \quad \text{B2} \end{array} \right)$$



$$\mathbf{S} = \mathbf{3}/\mathbf{2}, \mathbf{n}_{\text{occ.}} = \{\mathbf{1}, \mathbf{2}, \mathbf{1}\}$$

|        | 145           | 146           | 147            | 148            | 149           | 150           | 151            | 152            | 153           | 154           | 155            | 156            | 157           | 158           | 159            | 160            | 161           | 162           | 163            | 164            | 165           | 166           | 167            | 168            | 169           | 170           | 171            | 172            | 173           | 174           | 175            | 176            | 177           | 178           | 179            | 180            | 181           | 182           | 183            | 184            | 185           | 186           | 187            | 188            | 189           | 190           | 191            | 192            |    |    |    |
|--------|---------------|---------------|----------------|----------------|---------------|---------------|----------------|----------------|---------------|---------------|----------------|----------------|---------------|---------------|----------------|----------------|---------------|---------------|----------------|----------------|---------------|---------------|----------------|----------------|---------------|---------------|----------------|----------------|---------------|---------------|----------------|----------------|---------------|---------------|----------------|----------------|---------------|---------------|----------------|----------------|---------------|---------------|----------------|----------------|---------------|---------------|----------------|----------------|----|----|----|
| State  | 145           | 146           | 147            | 148            | 149           | 150           | 151            | 152            | 153           | 154           | 155            | 156            | 157           | 158           | 159            | 160            | 161           | 162           | 163            | 164            | 165           | 166           | 167            | 168            | 169           | 170           | 171            | 172            | 173           | 174           | 175            | 176            | 177           | 178           | 179            | 180            | 181           | 182           | 183            | 184            | 185           | 186           | 187            | 188            | 189           | 190           | 191            | 192            |    |    |    |
| Sz     | $\frac{3}{2}$ | $\frac{1}{2}$ | $-\frac{1}{2}$ | $-\frac{3}{2}$ | $\frac{3}{2}$ | $\frac{1}{2}$ | $-\frac{1}{2}$ | $-\frac{3}{2}$ | $\frac{3}{2}$ | $\frac{1}{2}$ | $-\frac{1}{2}$ | $-\frac{3}{2}$ | $\frac{3}{2}$ | $\frac{1}{2}$ | $-\frac{1}{2}$ | $-\frac{3}{2}$ | $\frac{3}{2}$ | $\frac{1}{2}$ | $-\frac{1}{2}$ | $-\frac{3}{2}$ | $\frac{3}{2}$ | $\frac{1}{2}$ | $-\frac{1}{2}$ | $-\frac{3}{2}$ | $\frac{3}{2}$ | $\frac{1}{2}$ | $-\frac{1}{2}$ | $-\frac{3}{2}$ | $\frac{3}{2}$ | $\frac{1}{2}$ | $-\frac{1}{2}$ | $-\frac{3}{2}$ | $\frac{3}{2}$ | $\frac{1}{2}$ | $-\frac{1}{2}$ | $-\frac{3}{2}$ | $\frac{3}{2}$ | $\frac{1}{2}$ | $-\frac{1}{2}$ | $-\frac{3}{2}$ | $\frac{3}{2}$ | $\frac{1}{2}$ | $-\frac{1}{2}$ | $-\frac{3}{2}$ | $\frac{3}{2}$ | $\frac{1}{2}$ | $-\frac{1}{2}$ | $-\frac{3}{2}$ |    |    |    |
| Rx     | 1             | 1             | 1              | 1              | 1             | 1             | 1              | 1              | 1             | 1             | 1              | 1              | 1             | 1             | 1              | 1              | 0             | 0             | 0              | 0              | 0             | 0             | 0              | 0              | 0             | 0             | 0              | 0              | 0             | 0             | 0              | 0              | 0             | 0             | 0              | 0              | 0             | 0             | 0              | -1             | -1            | -1            | -1             | -1             | -1            | -1            | -1             | -1             | -1 |    |    |
| Ry     | 1             | 1             | 1              | 1              | 1             | 1             | 1              | 1              | 1             | 1             | 1              | 1              | 1             | 1             | 1              | 1              | 0             | 0             | 0              | 0              | 0             | 0             | 0              | 0              | 0             | 0             | 0              | 0              | 0             | 0             | 0              | 0              | 0             | 0             | 0              | 0              | 0             | 0             | 0              | 0              | 0             | -1            | -1             | -1             | -1            | -1            | -1             | -1             | -1 | -1 | -1 |
| R      | 1             | 1             | 1              | 1              | 1             | 1             | 1              | 1              | -1            | -1            | -1             | -1             | -1            | -1            | -1             | -1             | $i$           | $i$           | $i$            | $i$            | $i$           | $i$           | $i$            | $i$            | $i$           | $i$           | $i$            | $i$            | $-i$          | $-i$          | $-i$           | $-i$           | $-i$          | $-i$          | $-i$           | $-i$           | $-i$          | $-i$          | $-i$           | 1              | 1             | 1             | 1              | -1             | -1            | -1            | -1             | -1             | -1 |    |    |
| Landau | A1            | A1            | A1             | A1             | A1            | A1            | A1             | A1             | B1            | B1            | B1             | B1             | B1            | B1            | B1             | B1             | E             | E             | E              | E              | E             | E             | E              | E              | E             | E             | E              | E              | E             | E             | E              | E              | E             | E             | E              | E              | E             | E             | E              | A2             | A2            | A2            | A2             | B2             | B2            | B2            | B2             | B2             | B2 |    |    |

$$\mathbf{S} = \mathbf{3}/\mathbf{2}, \text{ n}_{\text{occ.}} = \{\mathbf{0}, \mathbf{3}, \mathbf{1}\}$$

| State  | 193           | 194           | 195            | 196            | 197           | 198           | 199            | 200            | 201           | 202           | 203            | 204            | 205           | 206           | 207            | 208            |
|--------|---------------|---------------|----------------|----------------|---------------|---------------|----------------|----------------|---------------|---------------|----------------|----------------|---------------|---------------|----------------|----------------|
| Sz     | $\frac{3}{2}$ | $\frac{1}{2}$ | $-\frac{1}{2}$ | $-\frac{3}{2}$ | $\frac{3}{2}$ | $\frac{1}{2}$ | $-\frac{1}{2}$ | $-\frac{3}{2}$ | $\frac{3}{2}$ | $\frac{1}{2}$ | $-\frac{1}{2}$ | $-\frac{3}{2}$ | $\frac{3}{2}$ | $\frac{1}{2}$ | $-\frac{1}{2}$ | $-\frac{3}{2}$ |
| Rx     | 1             | 1             | 1              | 1              | 1             | 1             | 1              | 1              | 0             | 0             | 0              | 0              | 0             | 0             | 0              | 0              |
| Ry     | 1             | 1             | 1              | 1              | 1             | 1             | 1              | 1              | 0             | 0             | 0              | 0              | 0             | 0             | 0              | 0              |
| R      | 1             | 1             | 1              | 1              | -1            | -1            | -1             | -1             | $i$           | $i$           | $i$            | $i$            | $-i$          | $-i$          | $-i$           | $-i$           |
| Landau | A1            | A1            | A1             | A1             | B1            | B1            | B1             | B1             | E             | E             | E              | E              | E             | E             | E              | E              |



$\mathbf{S} = \mathbf{1}, \mathbf{n}_{\text{occ.}} = \{\mathbf{3}, \mathbf{1}, \mathbf{0}\}$

|        |     |     |     |     |     |     |     |     |     |     |     |     |     |     |     |     |     |     |     |     |     |      |      |      |      |      |      |      |      |     |     |     |     |     |     |     |
|--------|-----|-----|-----|-----|-----|-----|-----|-----|-----|-----|-----|-----|-----|-----|-----|-----|-----|-----|-----|-----|-----|------|------|------|------|------|------|------|------|-----|-----|-----|-----|-----|-----|-----|
| State  | 218 | 219 | 220 | 221 | 222 | 223 | 224 | 225 | 226 | 227 | 228 | 229 | 230 | 231 | 232 | 233 | 234 | 235 | 236 | 237 | 238 | 239  | 240  | 241  | 242  | 243  | 244  | 245  | 246  | 247 | 248 | 249 | 250 | 251 | 252 | 253 |
| Sz     | 1   | 0   | -1  | 1   | 0   | -1  | 1   | 0   | -1  | 1   | 0   | -1  | 1   | 0   | -1  | 1   | 0   | -1  | 1   | 0   | -1  | 1    | 0    | -1   | 1    | 0    | -1   | 1    | 0    | -1  | 1   | 0   | -1  | 1   | 0   | -1  |
| Rx     | 1   | 1   | 1   | 1   | 1   | 1   | 1   | 1   | 1   | 1   | 1   | 1   | 0   | 0   | 0   | 0   | 0   | 0   | 0   | 0   | 0   | 0    | 0    | 0    | 0    | 0    | 0    | 0    | 0    | 0   | -1  | -1  | -1  | -1  | -1  | -1  |
| Ry     | 1   | 1   | 1   | 1   | 1   | 1   | 1   | 1   | 1   | 1   | 1   | 1   | 0   | 0   | 0   | 0   | 0   | 0   | 0   | 0   | 0   | 0    | 0    | 0    | 0    | 0    | 0    | 0    | 0    | 0   | -1  | -1  | -1  | -1  | -1  | -1  |
| R      | 1   | 1   | 1   | 1   | 1   | 1   | -1  | -1  | -1  | -1  | -1  | -1  | $i$ | $i$ | $i$ | $i$ | $i$ | $i$ | $i$ | $i$ | $i$ | $-i$ | $-i$ | $-i$ | $-i$ | $-i$ | $-i$ | $-i$ | $-i$ | 1   | 1   | 1   | -1  | -1  | -1  |     |
| Landau | A1  | A1  | A1  | A1  | A1  | A1  | B1  | B1  | B1  | B1  | B1  | B1  | E   | E   | E   | E   | E   | E   | E   | E   | E   | E    | E    | E    | E    | E    | E    | E    | E    | E   | A2  | A2  | A2  | B2  | B2  | B2  |

$$\mathbf{S} = \mathbf{1}, \mathbf{n}_{\text{occ.}} = \{\mathbf{2}, \mathbf{2}, \mathbf{0}\}$$

[illegible]

$$S = 1, \text{ n}_{\text{occ.}} = \{2, 0, 2\}$$

[illegible]

$\mathbf{S} = \mathbf{1}, \mathbf{n}_{\text{occ.}} = \{\mathbf{1}, \mathbf{3}, \mathbf{0}\}$

|        |     |     |     |     |     |     |     |     |     |     |     |     |     |     |     |     |     |     |     |     |     |     |      |      |      |      |      |      |      |      |     |     |     |     |     |     |
|--------|-----|-----|-----|-----|-----|-----|-----|-----|-----|-----|-----|-----|-----|-----|-----|-----|-----|-----|-----|-----|-----|-----|------|------|------|------|------|------|------|------|-----|-----|-----|-----|-----|-----|
| State  | 326 | 327 | 328 | 329 | 330 | 331 | 332 | 333 | 334 | 335 | 336 | 337 | 338 | 339 | 340 | 341 | 342 | 343 | 344 | 345 | 346 | 347 | 348  | 349  | 350  | 351  | 352  | 353  | 354  | 355  | 356 | 357 | 358 | 359 | 360 | 361 |
| Sz     | 1   | 0   | -1  | 1   | 0   | -1  | 1   | 0   | -1  | 1   | 0   | -1  | 1   | 0   | -1  | 1   | 0   | -1  | 1   | 0   | -1  | 1   | 0    | -1   | 1    | 0    | -1   | 1    | 0    | -1   | 1   | 0   | -1  | 1   | 0   | -1  |
| Rx     | 1   | 1   | 1   | 1   | 1   | 1   | 1   | 1   | 1   | 1   | 1   | 1   | 0   | 0   | 0   | 0   | 0   | 0   | 0   | 0   | 0   | 0   | 0    | 0    | 0    | 0    | 0    | 0    | 0    | 0    | -1  | -1  | -1  | -1  | -1  | -1  |
| Ry     | 1   | 1   | 1   | 1   | 1   | 1   | 1   | 1   | 1   | 1   | 1   | 1   | 0   | 0   | 0   | 0   | 0   | 0   | 0   | 0   | 0   | 0   | 0    | 0    | 0    | 0    | 0    | 0    | 0    | 0    | -1  | -1  | -1  | -1  | -1  | -1  |
| R      | 1   | 1   | 1   | 1   | 1   | 1   | -1  | -1  | -1  | -1  | -1  | -1  | $i$ | $i$ | $i$ | $i$ | $i$ | $i$ | $i$ | $i$ | $i$ | $i$ | $-i$ | $-i$ | $-i$ | $-i$ | $-i$ | $-i$ | $-i$ | $-i$ | 1   | 1   | 1   | -1  | -1  | -1  |
| Landau | A1  | A1  | A1  | A1  | A1  | A1  | B1  | B1  | B1  | B1  | B1  | B1  | E   | E   | E   | E   | E   | E   | E   | E   | E   | E   | E    | E    | E    | E    | E    | E    | E    | E    | A2  | A2  | A2  | B2  | B2  | B2  |

| $\mathbf{S} = \mathbf{1}, \mathbf{n}_{\text{occ.}} = \{\mathbf{1}, \mathbf{1}, \mathbf{2}\}$ |     |     |     |     |     |     |     |     |     |     |     |     |     |     |     |     |     |     |     |     |     |     |      |      |      |      |      |      |      |      |     |     |     |     |     |     |
|----------------------------------------------------------------------------------------------|-----|-----|-----|-----|-----|-----|-----|-----|-----|-----|-----|-----|-----|-----|-----|-----|-----|-----|-----|-----|-----|-----|------|------|------|------|------|------|------|------|-----|-----|-----|-----|-----|-----|
| State                                                                                        | 362 | 363 | 364 | 365 | 366 | 367 | 368 | 369 | 370 | 371 | 372 | 373 | 374 | 375 | 376 | 377 | 378 | 379 | 380 | 381 | 382 | 383 | 384  | 385  | 386  | 387  | 388  | 389  | 390  | 391  | 392 | 393 | 394 | 395 | 396 | 397 |
| Sz                                                                                           | 1   | 0   | -1  | 1   | 0   | -1  | 1   | 0   | -1  | 1   | 0   | -1  | 1   | 0   | -1  | 1   | 0   | -1  | 1   | 0   | -1  | 1   | 0    | -1   | 1    | 0    | -1   | 1    | 0    | -1   | 1   | 0   | -1  | 1   | 0   | -1  |
| Rx                                                                                           | 1   | 1   | 1   | 1   | 1   | 1   | 1   | 1   | 1   | 1   | 1   | 1   | 0   | 0   | 0   | 0   | 0   | 0   | 0   | 0   | 0   | 0   | 0    | 0    | 0    | 0    | 0    | 0    | 0    | 0    | -1  | -1  | -1  | -1  | -1  | -1  |
| Ry                                                                                           | 1   | 1   | 1   | 1   | 1   | 1   | 1   | 1   | 1   | 1   | 1   | 1   | 0   | 0   | 0   | 0   | 0   | 0   | 0   | 0   | 0   | 0   | 0    | 0    | 0    | 0    | 0    | 0    | 0    | 0    | -1  | -1  | -1  | -1  | -1  | -1  |
| R                                                                                            | 1   | 1   | 1   | 1   | 1   | 1   | -1  | -1  | -1  | -1  | -1  | -1  | $i$ | $i$ | $i$ | $i$ | $i$ | $i$ | $i$ | $i$ | $i$ | $i$ | $-i$ | $-i$ | $-i$ | $-i$ | $-i$ | $-i$ | $-i$ | $-i$ | 1   | 1   | 1   | -1  | -1  | -1  |
| Landau                                                                                       | A1  | A1  | A1  | A1  | A1  | A1  | B1  | B1  | B1  | B1  | B1  | B1  | E   | E   | E   | E   | E   | E   | E   | E   | E   | E   | E    | E    | E    | E    | E    | E    | E    | E    | A2  | A2  | A2  | B2  | B2  | B2  |





$$S = 1, \text{ n}_{\text{occ.}} = \{0, 2, 2\}$$

[illegible]





$\mathbf{S} = \mathbf{1}/\mathbf{2}, \mathbf{n}_{occ.} = \{\mathbf{1}, \mathbf{2}, \mathbf{1}\}$

|  |        |               |                |               |                |               |                |               |                |               |                |               |                |               |                |               |                |               |                |               |                |               |                |               |                |               |                |               |                |               |                |               |                |               |                |               |                |               |                |               |                |               |                |               |                |     |     |     |     |
|--|--------|---------------|----------------|---------------|----------------|---------------|----------------|---------------|----------------|---------------|----------------|---------------|----------------|---------------|----------------|---------------|----------------|---------------|----------------|---------------|----------------|---------------|----------------|---------------|----------------|---------------|----------------|---------------|----------------|---------------|----------------|---------------|----------------|---------------|----------------|---------------|----------------|---------------|----------------|---------------|----------------|---------------|----------------|---------------|----------------|-----|-----|-----|-----|
|  | State  | 489           | 490            | 491           | 492            | 493           | 494            | 495           | 496            | 497           | 498            | 499           | 500            | 501           | 502            | 503           | 504            | 505           | 506            | 507           | 508            | 509           | 510            | 511           | 512            | 513           | 514            | 515           | 516            | 517           | 518            | 519           | 520            | 521           | 522            | 523           | 524            | 525           | 526            | 527           | 528            | 529           | 530            | 531           | 532            | 533 | 534 | 535 | 536 |
|  | Sz     | $\frac{1}{2}$ | $-\frac{1}{2}$ | $\frac{1}{2}$ | $-\frac{1}{2}$ | $\frac{1}{2}$ | $-\frac{1}{2}$ | $\frac{1}{2}$ | $-\frac{1}{2}$ | $\frac{1}{2}$ | $-\frac{1}{2}$ | $\frac{1}{2}$ | $-\frac{1}{2}$ | $\frac{1}{2}$ | $-\frac{1}{2}$ | $\frac{1}{2}$ | $-\frac{1}{2}$ | $\frac{1}{2}$ | $-\frac{1}{2}$ | $\frac{1}{2}$ | $-\frac{1}{2}$ | $\frac{1}{2}$ | $-\frac{1}{2}$ | $\frac{1}{2}$ | $-\frac{1}{2}$ | $\frac{1}{2}$ | $-\frac{1}{2}$ | $\frac{1}{2}$ | $-\frac{1}{2}$ | $\frac{1}{2}$ | $-\frac{1}{2}$ | $\frac{1}{2}$ | $-\frac{1}{2}$ | $\frac{1}{2}$ | $-\frac{1}{2}$ | $\frac{1}{2}$ | $-\frac{1}{2}$ | $\frac{1}{2}$ | $-\frac{1}{2}$ | $\frac{1}{2}$ | $-\frac{1}{2}$ | $\frac{1}{2}$ | $-\frac{1}{2}$ | $\frac{1}{2}$ | $-\frac{1}{2}$ |     |     |     |     |
|  | Rx     | 1             | 1              | 1             | 1              | 1             | 1              | 1             | 1              | 1             | 1              | 1             | 1              | 0             | 0              | 0             | 0              | 0             | 0              | 0             | 0              | 0             | 0              | 0             | 0              | 0             | 0              | 0             | 0              | 0             | 0              | 0             | 0              | 0             | -1             | -1            | -1             | -1            | -1             | -1            | -1             | -1            | -1             | -1            | -1             | -1  | -1  |     |     |
|  | Ry     | 1             | 1              | 1             | 1              | 1             | 1              | 1             | 1              | 1             | 1              | 1             | 1              | 0             | 0              | 0             | 0              | 0             | 0              | 0             | 0              | 0             | 0              | 0             | 0              | 0             | 0              | 0             | 0              | 0             | 0              | 0             | 0              | 0             | 0              | 0             | -1             | -1            | -1             | -1            | -1             | -1            | -1             | -1            | -1             | -1  | -1  | -1  |     |
|  | R      | 1             | 1              | 1             | 1              | 1             | 1              | -1            | -1             | -1            | -1             | -1            | -1             | i             | i              | i             | i              | i             | i              | i             | i              | i             | i              | i             | i              | -i            | -i             | -i            | -i             | -i            | -i             | -i            | -i             | -i            | -i             | -i            | 1              | 1             | 1              | 1             | 1              | 1             | -1             | -1            | -1             | -1  | -1  | -1  |     |
|  | Landau | A1            | A1             | A1            | A1             | A1            | A1             | B1            | B1             | B1            | B1             | B1            | B1             | E             | E              | E             | E              | E             | E              | E             | E              | E             | E              | E             | E              | E             | E              | E             | E              | E             | E              | E             | E              | E             | E              | E             | E              | A2            | A2             | A2            | A2             | A2            | A2             | B2            | B2             | B2  | B2  | B2  | B2  |

$$\mathbf{S} = \mathbf{1}/\mathbf{2}, \mathbf{n}_{\text{occ.}} = \{\mathbf{1}, \mathbf{0}, \mathbf{3}\}$$

$$\left( \begin{array}{c|cccccccc} \text{State} & 537 & 538 & 539 & 540 & 541 & 542 & 543 & 544 \\ \hline \text{Sz} & \frac{1}{2} & -\frac{1}{2} & \frac{1}{2} & -\frac{1}{2} & \frac{1}{2} & -\frac{1}{2} & \frac{1}{2} & -\frac{1}{2} \\ \text{Rx} & 1 & 1 & 1 & 1 & 0 & 0 & 0 & 0 \\ \text{Ry} & 1 & 1 & 1 & 1 & 0 & 0 & 0 & 0 \\ \text{R} & 1 & 1 & -1 & -1 & i & i & -i & -i \\ \text{Landau} & \text{A1} & \text{A1} & \text{B1} & \text{B1} & \text{E} & \text{E} & \text{E} & \text{E} \end{array} \right)$$



$$\mathbf{S} = \mathbf{1}/\mathbf{2}, \text{ n}_{\text{occ.}} = \{\mathbf{0}, \mathbf{1}, \mathbf{3}\}$$

$$\left( \begin{array}{c|cccccccc} \text{State} & 561 & 562 & 563 & 564 & 565 & 566 & 567 & 568 \\ \hline \text{Sz} & \frac{1}{2} & -\frac{1}{2} & \frac{1}{2} & -\frac{1}{2} & \frac{1}{2} & -\frac{1}{2} & \frac{1}{2} & -\frac{1}{2} \\ \text{Rx} & 1 & 1 & 1 & 1 & 0 & 0 & 0 & 0 \\ \text{Ry} & 1 & 1 & 1 & 1 & 0 & 0 & 0 & 0 \\ \text{R} & 1 & 1 & -1 & -1 & i & i & -i & -i \\ \text{Landau} & \text{A1} & \text{A1} & \text{B1} & \text{B1} & \text{E} & \text{E} & \text{E} & \text{E} \end{array} \right)$$



$$\mathbf{S} = \mathbf{0}, \mathbf{n}_{\text{occ.}} = \{4, \mathbf{0}, \mathbf{0}\}$$

$$\left( \begin{array}{ccc} \text{State} & 569 & 570 \\ \text{Sz} & 0 & 0 \\ \text{Rx} & 1 & -1 \\ \text{Ry} & 1 & -1 \\ \text{R} & 1 & -1 \\ \text{Landau} & \text{A1} & \text{B2} \end{array} \right)$$

$$\mathbf{S} = \mathbf{0}, \mathbf{n}_{\text{occ.}} = \{\mathbf{3}, \mathbf{1}, \mathbf{0}\}$$

| State  | 571 | 572 | 573 | 574 | 575  | 576  | 577 | 578 |
|--------|-----|-----|-----|-----|------|------|-----|-----|
| Sz     | 0   | 0   | 0   | 0   | 0    | 0    | 0   | 0   |
| Rx     | 1   | 1   | 0   | 0   | 0    | 0    | -1  | -1  |
| Ry     | 1   | 1   | 0   | 0   | 0    | 0    | -1  | -1  |
| R      | 1   | -1  | $i$ | $i$ | $-i$ | $-i$ | 1   | -1  |
| Landau | A1  | B1  | E   | E   | E    | E    | A2  | B2  |

$$\mathbf{S} = \mathbf{0}, \mathbf{n}_{\text{occ.}} = \{\mathbf{2}, \mathbf{2}, \mathbf{0}\}$$

| State  | 579 | 580 | 581 | 582 | 583 | 584 | 585  | 586  | 587 | 588 | 589 | 590 |
|--------|-----|-----|-----|-----|-----|-----|------|------|-----|-----|-----|-----|
| Sz     | 0   | 0   | 0   | 0   | 0   | 0   | 0    | 0    | 0   | 0   | 0   | 0   |
| Rx     | 1   | 1   | 1   | 1   | 0   | 0   | 0    | 0    | -1  | -1  | -1  | -1  |
| Ry     | 1   | 1   | 1   | 1   | 0   | 0   | 0    | 0    | -1  | -1  | -1  | -1  |
| R      | 1   | 1   | 1   | -1  | $i$ | $i$ | $-i$ | $-i$ | 1   | -1  | -1  | -1  |
| Landau | A1  | A1  | A1  | B1  | E   | E   | E    | E    | A2  | B2  | B2  | B2  |

$$\mathbf{S} = \mathbf{0}, \text{ n}_{\text{occ.}} = \{\mathbf{2}, \mathbf{0}, \mathbf{2}\}$$

| State  | 591 | 592      | 593      | 594        | 595        | 596 |
|--------|-----|----------|----------|------------|------------|-----|
| Sz     | 0   | 0        | 0        | 0          | 0          | 0   |
| Rx     | 1   | 0        | 0        | 0          | 0          | -1  |
| Ry     | 1   | 0        | 0        | 0          | 0          | -1  |
| R      | -1  | <i>i</i> | <i>i</i> | - <i>i</i> | - <i>i</i> | 1   |
| Landau | B1  | E        | E        | E          | E          | A2  |

$$\mathbf{S} = \mathbf{0}, \text{ n}_{\text{occ.}} = \{1, 3, 0\}$$

| State  | 597 | 598 | 599 | 600 | 601  | 602  | 603 | 604 |
|--------|-----|-----|-----|-----|------|------|-----|-----|
| Sz     | 0   | 0   | 0   | 0   | 0    | 0    | 0   | 0   |
| Rx     | 1   | 1   | 0   | 0   | 0    | 0    | -1  | -1  |
| Ry     | 1   | 1   | 0   | 0   | 0    | 0    | -1  | -1  |
| R      | 1   | -1  | $i$ | $i$ | $-i$ | $-i$ | 1   | -1  |
| Landau | A1  | B1  | E   | E   | E    | E    | A2  | B2  |

$$\mathbf{S} = \mathbf{0}, \text{ n}_{\text{occ.}} = \{1, 1, 2\}$$

| State  | 605 | 606 | 607 | 608 | 609 | 610 | 611 | 612  | 613  | 614  | 615 | 616 |
|--------|-----|-----|-----|-----|-----|-----|-----|------|------|------|-----|-----|
| Sz     | 0   | 0   | 0   | 0   | 0   | 0   | 0   | 0    | 0    | 0    | 0   | 0   |
| Rx     | 1   | 1   | 1   | 1   | 0   | 0   | 0   | 0    | 0    | 0    | -1  | -1  |
| Ry     | 1   | 1   | 1   | 1   | 0   | 0   | 0   | 0    | 0    | 0    | -1  | -1  |
| R      | 1   | 1   | -1  | -1  | $i$ | $i$ | $i$ | $-i$ | $-i$ | $-i$ | 1   | -1  |
| Landau | A1  | A1  | B1  | B1  | E   | E   | E   | E    | E    | E    | A2  | B2  |

$$\mathbf{S} = \mathbf{0}, \text{ n}_{\text{occ.}} = \{\mathbf{0}, 4, \mathbf{0}\}$$

$$\left( \begin{array}{ccc} \text{State} & 617 & 618 \\ \text{Sz} & 0 & 0 \\ \text{Rx} & 1 & -1 \\ \text{Ry} & 1 & -1 \\ \text{R} & 1 & -1 \\ \text{Landau} & \text{A1} & \text{B2} \end{array} \right)$$

$$\mathbf{S} = \mathbf{0}, \mathbf{n}_{\text{occ.}} = \{\mathbf{0}, \mathbf{2}, \mathbf{2}\}$$

| State  | 619 | 620 | 621 | 622  | 623  | 624 |
|--------|-----|-----|-----|------|------|-----|
| Sz     | 0   | 0   | 0   | 0    | 0    | 0   |
| Rx     | 1   | 0   | 0   | 0    | 0    | -1  |
| Ry     | 1   | 0   | 0   | 0    | 0    | -1  |
| R      | -1  | $i$ | $i$ | $-i$ | $-i$ | 1   |
| Landau | B1  | E   | E   | E    | E    | A2  |



$$\mathbf{S} = \mathbf{0}, \text{ n}_{\text{occ.}} = \{0, 0, 4\}$$

$$\left( \begin{array}{cc} \text{State} & 625 \\ \text{Sz} & 0 \\ \text{Rx} & 1 \\ \text{Ry} & 1 \\ \text{R} & 1 \\ \text{Landau} & \text{A1} \end{array} \right)$$

$$\mathbf{S} = \mathbf{2}, \mathbf{n}_{\text{occ.}} = \{4, \mathbf{0}, \mathbf{0}, \mathbf{0}\}$$

$$\left( \begin{array}{ccccc} \text{State} & 1 & 2 & 3 & 4 & 5 \\ \text{Sz} & 2 & 1 & 0 & -1 & -2 \\ \text{Rx} & 1 & 1 & 1 & 1 & 1 \\ \text{Ry} & 1 & 1 & 1 & 1 & 1 \\ \text{R} & 1 & 1 & 1 & 1 & 1 \\ \text{Landau} & \text{A1} & \text{A1} & \text{A1} & \text{A1} & \text{A1} \end{array} \right)$$





$$\mathbf{S} = \mathbf{3}/\mathbf{2}, \mathbf{n}_{\text{occ.}} = \{\mathbf{3}, \mathbf{0}, \mathbf{0}, \mathbf{1}\}$$

| State  | 38            | 39            | 40             | 41             | 42            | 43            | 44             | 45             | 46            | 47            | 48             | 49             | 50            | 51            | 52             | 53             |
|--------|---------------|---------------|----------------|----------------|---------------|---------------|----------------|----------------|---------------|---------------|----------------|----------------|---------------|---------------|----------------|----------------|
| Sz     | $\frac{3}{2}$ | $\frac{1}{2}$ | $-\frac{1}{2}$ | $-\frac{3}{2}$ | $\frac{3}{2}$ | $\frac{1}{2}$ | $-\frac{1}{2}$ | $-\frac{3}{2}$ | $\frac{3}{2}$ | $\frac{1}{2}$ | $-\frac{1}{2}$ | $-\frac{3}{2}$ | $\frac{3}{2}$ | $\frac{1}{2}$ | $-\frac{1}{2}$ | $-\frac{3}{2}$ |
| Rx     | 1             | 1             | 1              | 1              | 1             | 1             | 1              | 1              | 0             | 0             | 0              | 0              | 0             | 0             | 0              | 0              |
| Ry     | 1             | 1             | 1              | 1              | 1             | 1             | 1              | 1              | 0             | 0             | 0              | 0              | 0             | 0             | 0              | 0              |
| R      | 1             | 1             | 1              | 1              | -1            | -1            | -1             | -1             | $i$           | $i$           | $i$            | $i$            | $-i$          | $-i$          | $-i$           | $-i$           |
| Landau | A1            | A1            | A1             | A1             | B1            | B1            | B1             | B1             | E             | E             | E              | E              | E             | E             | E              | E              |



$$\mathbf{S} = \mathbf{1}, \mathbf{n}_{\text{occ.}} = \{\mathbf{2}, \mathbf{2}, \mathbf{0}, \mathbf{0}\}$$

$$\left( \begin{array}{c|cccccccccccccccccccc} \text{State} & 63 & 64 & 65 & 66 & 67 & 68 & 69 & 70 & 71 & 72 & 73 & 74 & 75 & 76 & 77 & 78 & 79 & 80 \\ \hline \text{Sz} & 1 & 0 & -1 & 1 & 0 & -1 & 1 & 0 & -1 & 1 & 0 & -1 & 1 & 0 & -1 & 1 & 0 & -1 \\ \text{Rx} & 1 & 1 & 1 & 1 & 1 & 1 & 1 & 1 & 1 & 0 & 0 & 0 & 0 & 0 & 0 & -1 & -1 & -1 \\ \text{Ry} & 1 & 1 & 1 & 1 & 1 & 1 & 1 & 1 & 1 & 0 & 0 & 0 & 0 & 0 & 0 & -1 & -1 & -1 \\ \text{R} & 1 & 1 & 1 & 1 & 1 & 1 & -1 & -1 & -1 & i & i & i & -i & -i & -i & -1 & -1 & -1 \\ \text{Landau} & \text{A1} & \text{A1} & \text{A1} & \text{A1} & \text{A1} & \text{A1} & \text{B1} & \text{B1} & \text{B1} & \text{E} & \text{E} & \text{E} & \text{E} & \text{E} & \text{E} & \text{B2} & \text{B2} & \text{B2} \end{array} \right)$$

$$\mathbf{S} = \mathbf{1}, \mathbf{n}_{\text{occ.}} = \{\mathbf{2}, \mathbf{1}, \mathbf{1}, \mathbf{0}\}$$

| State  | 81 | 82 | 83 | 84 | 85 | 86 | 87 | 88 | 89 | 90 | 91 | 92 | 93       | 94       | 95       | 96       | 97       | 98       | 99       | 100      | 101      | 102        | 103        | 104        | 105        | 106        | 107        | 108        | 109        | 110        | 111 | 112 | 113 | 114 | 115 | 116 |
|--------|----|----|----|----|----|----|----|----|----|----|----|----|----------|----------|----------|----------|----------|----------|----------|----------|----------|------------|------------|------------|------------|------------|------------|------------|------------|------------|-----|-----|-----|-----|-----|-----|
| Sz     | 1  | 0  | -1 | 1  | 0  | -1 | 1  | 0  | -1 | 1  | 0  | -1 | 1        | 0        | -1       | 1        | 0        | -1       | 1        | 0        | -1       | 1          | 0          | -1         | 1          | 0          | -1         | 1          | 0          | -1         | 1   | 0   | -1  | 1   | 0   | -1  |
| Rx     | 1  | 1  | 1  | 1  | 1  | 1  | 1  | 1  | 1  | 1  | 1  | 1  | 0        | 0        | 0        | 0        | 0        | 0        | 0        | 0        | 0        | 0          | 0          | 0          | 0          | 0          | 0          | 0          | 0          | 0          | -1  | -1  | -1  | -1  | -1  | -1  |
| Ry     | 1  | 1  | 1  | 1  | 1  | 1  | 1  | 1  | 1  | 1  | 1  | 1  | 0        | 0        | 0        | 0        | 0        | 0        | 0        | 0        | 0        | 0          | 0          | 0          | 0          | 0          | 0          | 0          | 0          | 0          | -1  | -1  | -1  | -1  | -1  | -1  |
| R      | 1  | 1  | 1  | 1  | 1  | 1  | -1 | -1 | -1 | -1 | -1 | -1 | <i>i</i> | <i>i</i> | <i>i</i> | <i>i</i> | <i>i</i> | <i>i</i> | <i>i</i> | <i>i</i> | <i>i</i> | - <i>i</i> | - <i>i</i> | - <i>i</i> | - <i>i</i> | - <i>i</i> | - <i>i</i> | - <i>i</i> | - <i>i</i> | - <i>i</i> | 1   | 1   | 1   | -1  | -1  | -1  |
| Landau | A1 | A1 | A1 | A1 | A1 | A1 | B1 | B1 | B1 | B1 | B1 | B1 | E        | E        | E        | E        | E        | E        | E        | E        | E        | E          | E          | E          | E          | E          | E          | E          | E          | E          | A2  | A2  | A2  | B2  | B2  | B2  |



$$\mathbf{S} = \mathbf{1}, \mathbf{n}_{\text{occ.}} = \{\mathbf{2}, \mathbf{1}, \mathbf{0}, \mathbf{1}\}$$

| State  | 117 | 118 | 119 | 120 | 121 | 122 | 123 | 124 | 125 | 126 | 127 | 128 | 129      | 130      | 131      | 132      | 133      | 134      | 135      | 136      | 137      | 138      | 139        | 140        | 141        | 142        | 143        | 144        | 145        | 146 | 147 | 148 | 149 | 150 | 151 | 152 |
|--------|-----|-----|-----|-----|-----|-----|-----|-----|-----|-----|-----|-----|----------|----------|----------|----------|----------|----------|----------|----------|----------|----------|------------|------------|------------|------------|------------|------------|------------|-----|-----|-----|-----|-----|-----|-----|
| Sz     | 1   | 0   | -1  | 1   | 0   | -1  | 1   | 0   | -1  | 1   | 0   | -1  | 1        | 0        | -1       | 1        | 0        | -1       | 1        | 0        | -1       | 1        | 0          | -1         | 1          | 0          | -1         | 1          | 0          | -1  | 1   | 0   | -1  | 1   | 0   | -1  |
| Rx     | 1   | 1   | 1   | 1   | 1   | 1   | 1   | 1   | 1   | 1   | 1   | 1   | 0        | 0        | 0        | 0        | 0        | 0        | 0        | 0        | 0        | 0        | 0          | 0          | 0          | 0          | 0          | 0          | 0          | 0   | -1  | -1  | -1  | -1  | -1  | -1  |
| Ry     | 1   | 1   | 1   | 1   | 1   | 1   | 1   | 1   | 1   | 1   | 1   | 1   | 0        | 0        | 0        | 0        | 0        | 0        | 0        | 0        | 0        | 0        | 0          | 0          | 0          | 0          | 0          | 0          | 0          | 0   | -1  | -1  | -1  | -1  | -1  | -1  |
| R      | 1   | 1   | 1   | 1   | 1   | 1   | -1  | -1  | -1  | -1  | -1  | -1  | <i>i</i> | <i>i</i> | <i>i</i> | <i>i</i> | <i>i</i> | <i>i</i> | <i>i</i> | <i>i</i> | <i>i</i> | <i>i</i> | - <i>i</i> | - <i>i</i> | - <i>i</i> | - <i>i</i> | - <i>i</i> | - <i>i</i> | - <i>i</i> | 1   | 1   | 1   | -1  | -1  | -1  |     |
| Landau | A1  | A1  | A1  | A1  | A1  | A1  | B1  | B1  | B1  | B1  | B1  | B1  | E        | E        | E        | E        | E        | E        | E        | E        | E        | E        | E          | E          | E          | E          | E          | E          | E          | E   | A2  | A2  | A2  | B2  | B2  | B2  |

$$\mathbf{S} = \mathbf{1}, \mathbf{n}_{\text{occ.}} = \{2, 0, 2, 0\}$$

[illegible]

$$\mathbf{S} = \mathbf{1}, \mathbf{n}_{\text{occ.}} = \{\mathbf{2}, \mathbf{0}, \mathbf{1}, \mathbf{1}\}$$

| State  | 171 | 172 | 173 | 174 | 175 | 176 | 177 | 178 | 179 | 180 | 181 | 182 | 183 | 184 | 185 | 186 | 187 | 188 | 189 | 190 | 191 | 192 | 193  | 194  | 195  | 196  | 197  | 198  | 199  | 200  | 201 | 202 | 203 | 204 | 205 | 206 |
|--------|-----|-----|-----|-----|-----|-----|-----|-----|-----|-----|-----|-----|-----|-----|-----|-----|-----|-----|-----|-----|-----|-----|------|------|------|------|------|------|------|------|-----|-----|-----|-----|-----|-----|
| Sz     | 1   | 0   | -1  | 1   | 0   | -1  | 1   | 0   | -1  | 1   | 0   | -1  | 1   | 0   | -1  | 1   | 0   | -1  | 1   | 0   | -1  | 1   | 0    | -1   | 1    | 0    | -1   | 1    | 0    | -1   | 1   | 0   | -1  | 1   | 0   | -1  |
| Rx     | 1   | 1   | 1   | 1   | 1   | 1   | 1   | 1   | 1   | 1   | 1   | 1   | 0   | 0   | 0   | 0   | 0   | 0   | 0   | 0   | 0   | 0   | 0    | 0    | 0    | 0    | 0    | 0    | 0    | 0    | -1  | -1  | -1  | -1  | -1  | -1  |
| Ry     | 1   | 1   | 1   | 1   | 1   | 1   | 1   | 1   | 1   | 1   | 1   | 1   | 0   | 0   | 0   | 0   | 0   | 0   | 0   | 0   | 0   | 0   | 0    | 0    | 0    | 0    | 0    | 0    | 0    | 0    | -1  | -1  | -1  | -1  | -1  | -1  |
| R      | 1   | 1   | 1   | 1   | 1   | 1   | -1  | -1  | -1  | -1  | -1  | -1  | $i$ | $i$ | $i$ | $i$ | $i$ | $i$ | $i$ | $i$ | $i$ | $i$ | $-i$ | $-i$ | $-i$ | $-i$ | $-i$ | $-i$ | $-i$ | $-i$ | 1   | 1   | 1   | -1  | -1  | -1  |
| Landau | A1  | A1  | A1  | A1  | A1  | A1  | B1  | B1  | B1  | B1  | B1  | B1  | E   | E   | E   | E   | E   | E   | E   | E   | E   | E   | E    | E    | E    | E    | E    | E    | E    | E    | A2  | A2  | A2  | B2  | B2  | B2  |





$$\mathbf{S} = \mathbf{1}/2, \mathbf{n}_{\text{occ.}} = \{\mathbf{3}, \mathbf{0}, \mathbf{1}, \mathbf{0}\}$$

| State  | 241           | 242            | 243           | 244            | 245           | 246            | 247           | 248            | 249           | 250            | 251           | 252            | 253           | 254            | 255           | 256            |    |    |
|--------|---------------|----------------|---------------|----------------|---------------|----------------|---------------|----------------|---------------|----------------|---------------|----------------|---------------|----------------|---------------|----------------|----|----|
| Sz     | $\frac{1}{2}$ | $-\frac{1}{2}$ | $\frac{1}{2}$ | $-\frac{1}{2}$ | $\frac{1}{2}$ | $-\frac{1}{2}$ | $\frac{1}{2}$ | $-\frac{1}{2}$ | $\frac{1}{2}$ | $-\frac{1}{2}$ | $\frac{1}{2}$ | $-\frac{1}{2}$ | $\frac{1}{2}$ | $-\frac{1}{2}$ | $\frac{1}{2}$ | $-\frac{1}{2}$ |    |    |
| Rx     | 1             | 1              | 1             | 1              | 0             | 0              | 0             | 0              | 0             | 0              | 0             | 0              | -1            | -1             | -1            | -1             |    |    |
| Ry     | 1             | 1              | 1             | 1              | 0             | 0              | 0             | 0              | 0             | 0              | 0             | 0              | -1            | -1             | -1            | -1             |    |    |
| R      | 1             | 1              | -1            | -1             | $i$           | $i$            | $i$           | $i$            | $-i$          | $-i$           | $-i$          | $-i$           | 1             | 1              | -1            | -1             |    |    |
| Landau | A1            | A1             | B1            | B1             | E             | E              | E             | E              | E             | E              | E             | E              | E             | E              | A2            | A2             | B2 | B2 |



$$\mathbf{S} = \mathbf{1}/\mathbf{2}, \mathbf{n}_{\text{occ.}} = \{\mathbf{1}, \mathbf{3}, \mathbf{0}, \mathbf{0}\}$$

| State  | 273           | 274            | 275           | 276            | 277           | 278            | 279           | 280            |
|--------|---------------|----------------|---------------|----------------|---------------|----------------|---------------|----------------|
| Sz     | $\frac{1}{2}$ | $-\frac{1}{2}$ | $\frac{1}{2}$ | $-\frac{1}{2}$ | $\frac{1}{2}$ | $-\frac{1}{2}$ | $\frac{1}{2}$ | $-\frac{1}{2}$ |
| Rx     | 1             | 1              | 1             | 1              | 0             | 0              | 0             | 0              |
| Ry     | 1             | 1              | 1             | 1              | 0             | 0              | 0             | 0              |
| R      | 1             | 1              | -1            | -1             | $i$           | $i$            | $-i$          | $-i$           |
| Landau | A1            | A1             | B1            | B1             | E             | E              | E             | E              |



$$\mathbf{S} = \mathbf{1}/2, \mathbf{n}_{\text{occ.}} = \{\mathbf{1}, \mathbf{2}, \mathbf{1}, \mathbf{0}\}$$

| State  | 281           | 282            | 283           | 284            | 285           | 286            | 287           | 288            | 289           | 290            | 291           | 292            | 293           | 294            | 295           | 296            | 297           | 298            | 299           | 300            | 301           | 302            | 303           | 304            |
|--------|---------------|----------------|---------------|----------------|---------------|----------------|---------------|----------------|---------------|----------------|---------------|----------------|---------------|----------------|---------------|----------------|---------------|----------------|---------------|----------------|---------------|----------------|---------------|----------------|
| Sz     | $\frac{1}{2}$ | $-\frac{1}{2}$ | $\frac{1}{2}$ | $-\frac{1}{2}$ | $\frac{1}{2}$ | $-\frac{1}{2}$ | $\frac{1}{2}$ | $-\frac{1}{2}$ | $\frac{1}{2}$ | $-\frac{1}{2}$ | $\frac{1}{2}$ | $-\frac{1}{2}$ | $\frac{1}{2}$ | $-\frac{1}{2}$ | $\frac{1}{2}$ | $-\frac{1}{2}$ | $\frac{1}{2}$ | $-\frac{1}{2}$ | $\frac{1}{2}$ | $-\frac{1}{2}$ | $\frac{1}{2}$ | $-\frac{1}{2}$ | $\frac{1}{2}$ | $-\frac{1}{2}$ |
| Rx     | 1             | 1              | 1             | 1              | 1             | 1              | 1             | 1              | 0             | 0              | 0             | 0              | 0             | 0              | 0             | 0              | 0             | 0              | 0             | 0              | -1            | -1             | -1            | -1             |
| Ry     | 1             | 1              | 1             | 1              | 1             | 1              | 1             | 1              | 0             | 0              | 0             | 0              | 0             | 0              | 0             | 0              | 0             | 0              | 0             | 0              | -1            | -1             | -1            | -1             |
| R      | 1             | 1              | 1             | 1              | -1            | -1             | -1            | -1             | $i$           | $i$            | $i$           | $i$            | $i$           | $i$            | $-i$          | $-i$           | $-i$          | $-i$           | $-i$          | $-i$           | 1             | 1              | -1            | -1             |
| Landau | A1            | A1             | A1            | A1             | B1            | B1             | B1            | B1             | E             | E              | E             | E              | E             | E              | E             | E              | E             | E              | E             | E              | A2            | A2             | B2            | B2             |

$$\mathbf{S} = \mathbf{1}/2, \mathbf{n}_{\text{occ.}} = \{1, 2, 0, 1\}$$

| State  | 305           | 306            | 307           | 308            | 309           | 310            | 311           | 312            | 313           | 314            | 315           | 316            | 317           | 318            | 319           | 320            | 321           | 322            | 323           | 324            | 325           | 326            | 327           | 328            |
|--------|---------------|----------------|---------------|----------------|---------------|----------------|---------------|----------------|---------------|----------------|---------------|----------------|---------------|----------------|---------------|----------------|---------------|----------------|---------------|----------------|---------------|----------------|---------------|----------------|
| Sz     | $\frac{1}{2}$ | $-\frac{1}{2}$ | $\frac{1}{2}$ | $-\frac{1}{2}$ | $\frac{1}{2}$ | $-\frac{1}{2}$ | $\frac{1}{2}$ | $-\frac{1}{2}$ | $\frac{1}{2}$ | $-\frac{1}{2}$ | $\frac{1}{2}$ | $-\frac{1}{2}$ | $\frac{1}{2}$ | $-\frac{1}{2}$ | $\frac{1}{2}$ | $-\frac{1}{2}$ | $\frac{1}{2}$ | $-\frac{1}{2}$ | $\frac{1}{2}$ | $-\frac{1}{2}$ | $\frac{1}{2}$ | $-\frac{1}{2}$ | $\frac{1}{2}$ | $-\frac{1}{2}$ |
| Rx     | 1             | 1              | 1             | 1              | 1             | 1              | 1             | 1              | 0             | 0              | 0             | 0              | 0             | 0              | 0             | 0              | 0             | 0              | 0             | 0              | -1            | -1             | -1            | -1             |
| Ry     | 1             | 1              | 1             | 1              | 1             | 1              | 1             | 1              | 0             | 0              | 0             | 0              | 0             | 0              | 0             | 0              | 0             | 0              | 0             | 0              | -1            | -1             | -1            | -1             |
| R      | 1             | 1              | 1             | 1              | -1            | -1             | -1            | -1             | $i$           | $i$            | $i$           | $i$            | $i$           | $i$            | $-i$          | $-i$           | $-i$          | $-i$           | $-i$          | $-i$           | 1             | 1              | -1            | -1             |
| Landau | A1            | A1             | A1            | A1             | B1            | B1             | B1            | B1             | E             | E              | E             | E              | E             | E              | E             | E              | E             | E              | E             | E              | A2            | A2             | B2            | B2             |

$$\mathbf{S} = \mathbf{1}/2, \mathbf{n}_{\text{occ.}} = \{\mathbf{1}, \mathbf{1}, \mathbf{2}, \mathbf{0}\}$$

| State  | 329           | 330            | 331           | 332            | 333           | 334            | 335           | 336            | 337           | 338            | 339           | 340            | 341           | 342            | 343           | 344            | 345           | 346            | 347           | 348            | 349           | 350            | 351           | 352            |
|--------|---------------|----------------|---------------|----------------|---------------|----------------|---------------|----------------|---------------|----------------|---------------|----------------|---------------|----------------|---------------|----------------|---------------|----------------|---------------|----------------|---------------|----------------|---------------|----------------|
| Sz     | $\frac{1}{2}$ | $-\frac{1}{2}$ | $\frac{1}{2}$ | $-\frac{1}{2}$ | $\frac{1}{2}$ | $-\frac{1}{2}$ | $\frac{1}{2}$ | $-\frac{1}{2}$ | $\frac{1}{2}$ | $-\frac{1}{2}$ | $\frac{1}{2}$ | $-\frac{1}{2}$ | $\frac{1}{2}$ | $-\frac{1}{2}$ | $\frac{1}{2}$ | $-\frac{1}{2}$ | $\frac{1}{2}$ | $-\frac{1}{2}$ | $\frac{1}{2}$ | $-\frac{1}{2}$ | $\frac{1}{2}$ | $-\frac{1}{2}$ | $\frac{1}{2}$ | $-\frac{1}{2}$ |
| Rx     | 1             | 1              | 1             | 1              | 1             | 1              | 1             | 1              | 0             | 0              | 0             | 0              | 0             | 0              | 0             | 0              | 0             | 0              | 0             | 0              | -1            | -1             | -1            | -1             |
| Ry     | 1             | 1              | 1             | 1              | 1             | 1              | 1             | 1              | 0             | 0              | 0             | 0              | 0             | 0              | 0             | 0              | 0             | 0              | 0             | 0              | -1            | -1             | -1            | -1             |
| R      | 1             | 1              | 1             | 1              | -1            | -1             | -1            | -1             | $i$           | $i$            | $i$           | $i$            | $i$           | $i$            | $-i$          | $-i$           | $-i$          | $-i$           | $-i$          | $-i$           | 1             | 1              | -1            | -1             |
| Landau | A1            | A1             | A1            | A1             | B1            | B1             | B1            | B1             | E             | E              | E             | E              | E             | E              | E             | E              | E             | E              | E             | E              | A2            | A2             | B2            | B2             |

$$\mathbf{S} = \mathbf{1}/2, \mathbf{n}_{\text{occ.}} = \{1, 1, 1, 1\}$$

|        | 353           | 354            | 355           | 356            | 357           | 358            | 359           | 360            | 361           | 362            | 363           | 364            | 365           | 366            | 367           | 368            | 369           | 370            | 371           | 372            | 373           | 374            | 375           | 376            | 377           | 378            | 379           | 380            | 381           | 382            | 383           | 384            | 385           | 386            | 387           | 388            | 389           | 390            | 391           | 392            | 393           | 394            | 395           | 396            | 397           | 398            | 399 | 400 |    |    |
|--------|---------------|----------------|---------------|----------------|---------------|----------------|---------------|----------------|---------------|----------------|---------------|----------------|---------------|----------------|---------------|----------------|---------------|----------------|---------------|----------------|---------------|----------------|---------------|----------------|---------------|----------------|---------------|----------------|---------------|----------------|---------------|----------------|---------------|----------------|---------------|----------------|---------------|----------------|---------------|----------------|---------------|----------------|---------------|----------------|---------------|----------------|-----|-----|----|----|
| State  | 353           | 354            | 355           | 356            | 357           | 358            | 359           | 360            | 361           | 362            | 363           | 364            | 365           | 366            | 367           | 368            | 369           | 370            | 371           | 372            | 373           | 374            | 375           | 376            | 377           | 378            | 379           | 380            | 381           | 382            | 383           | 384            | 385           | 386            | 387           | 388            | 389           | 390            | 391           | 392            | 393           | 394            | 395           | 396            | 397           | 398            | 399 | 400 |    |    |
| Sz     | $\frac{1}{2}$ | $-\frac{1}{2}$ | $\frac{1}{2}$ | $-\frac{1}{2}$ | $\frac{1}{2}$ | $-\frac{1}{2}$ | $\frac{1}{2}$ | $-\frac{1}{2}$ | $\frac{1}{2}$ | $-\frac{1}{2}$ | $\frac{1}{2}$ | $-\frac{1}{2}$ | $\frac{1}{2}$ | $-\frac{1}{2}$ | $\frac{1}{2}$ | $-\frac{1}{2}$ | $\frac{1}{2}$ | $-\frac{1}{2}$ | $\frac{1}{2}$ | $-\frac{1}{2}$ | $\frac{1}{2}$ | $-\frac{1}{2}$ | $\frac{1}{2}$ | $-\frac{1}{2}$ | $\frac{1}{2}$ | $-\frac{1}{2}$ | $\frac{1}{2}$ | $-\frac{1}{2}$ | $\frac{1}{2}$ | $-\frac{1}{2}$ | $\frac{1}{2}$ | $-\frac{1}{2}$ | $\frac{1}{2}$ | $-\frac{1}{2}$ | $\frac{1}{2}$ | $-\frac{1}{2}$ | $\frac{1}{2}$ | $-\frac{1}{2}$ | $\frac{1}{2}$ | $-\frac{1}{2}$ | $\frac{1}{2}$ | $-\frac{1}{2}$ | $\frac{1}{2}$ | $-\frac{1}{2}$ | $\frac{1}{2}$ | $-\frac{1}{2}$ |     |     |    |    |
| Rx     | 1             | 1              | 1             | 1              | 1             | 1              | 1             | 1              | 1             | 1              | 1             | 1              | 0             | 0              | 0             | 0              | 0             | 0              | 0             | 0              | 0             | 0              | 0             | 0              | 0             | 0              | 0             | 0              | 0             | 0              | 0             | 0              | 0             | 0              | 0             | 0              | -1            | -1             | -1            | -1             | -1            | -1             | -1            | -1             | -1            | -1             | -1  |     |    |    |
| Ry     | 1             | 1              | 1             | 1              | 1             | 1              | 1             | 1              | 1             | 1              | 1             | 1              | 0             | 0              | 0             | 0              | 0             | 0              | 0             | 0              | 0             | 0              | 0             | 0              | 0             | 0              | 0             | 0              | 0             | 0              | 0             | 0              | 0             | 0              | 0             | 0              | 0             | -1             | -1            | -1             | -1            | -1             | -1            | -1             | -1            | -1             | -1  | -1  |    |    |
| R      | 1             | 1              | 1             | 1              | 1             | 1              | -1            | -1             | -1            | -1             | -1            | -1             | $i$           | $i$            | $i$           | $i$            | $i$           | $i$            | $i$           | $i$            | $i$           | $i$            | $i$           | $i$            | $i$           | $i$            | $-i$          | $-i$           | $-i$          | $-i$           | $-i$          | $-i$           | $-i$          | $-i$           | $-i$          | $-i$           | 1             | 1              | 1             | 1              | 1             | 1              | -1            | -1             | -1            | -1             | -1  | -1  |    |    |
| Landau | A1            | A1             | A1            | A1             | A1            | A1             | B1            | B1             | B1            | B1             | B1            | B1             | E             | E              | E             | E              | E             | E              | E             | E              | E             | E              | E             | E              | E             | E              | E             | E              | E             | E              | E             | E              | E             | E              | E             | E              | E             | E              | A2            | A2             | A2            | A2             | A2            | A2             | B2            | B2             | B2  | B2  | B2 | B2 |

$$\mathbf{S} = \mathbf{1}/2, \mathbf{n}_{\text{occ.}} = \{\mathbf{1}, \mathbf{1}, \mathbf{0}, \mathbf{2}\}$$

| State  | 401           | 402            | 403           | 404            | 405           | 406            | 407           | 408            | 409           | 410            | 411           | 412            | 413           | 414            | 415           | 416            | 417           | 418            | 419           | 420            | 421           | 422            | 423           | 424            |
|--------|---------------|----------------|---------------|----------------|---------------|----------------|---------------|----------------|---------------|----------------|---------------|----------------|---------------|----------------|---------------|----------------|---------------|----------------|---------------|----------------|---------------|----------------|---------------|----------------|
| Sz     | $\frac{1}{2}$ | $-\frac{1}{2}$ | $\frac{1}{2}$ | $-\frac{1}{2}$ | $\frac{1}{2}$ | $-\frac{1}{2}$ | $\frac{1}{2}$ | $-\frac{1}{2}$ | $\frac{1}{2}$ | $-\frac{1}{2}$ | $\frac{1}{2}$ | $-\frac{1}{2}$ | $\frac{1}{2}$ | $-\frac{1}{2}$ | $\frac{1}{2}$ | $-\frac{1}{2}$ | $\frac{1}{2}$ | $-\frac{1}{2}$ | $\frac{1}{2}$ | $-\frac{1}{2}$ | $\frac{1}{2}$ | $-\frac{1}{2}$ | $\frac{1}{2}$ | $-\frac{1}{2}$ |
| Rx     | 1             | 1              | 1             | 1              | 1             | 1              | 1             | 1              | 0             | 0              | 0             | 0              | 0             | 0              | 0             | 0              | 0             | 0              | 0             | 0              | -1            | -1             | -1            | -1             |
| Ry     | 1             | 1              | 1             | 1              | 1             | 1              | 1             | 1              | 0             | 0              | 0             | 0              | 0             | 0              | 0             | 0              | 0             | 0              | 0             | 0              | -1            | -1             | -1            | -1             |
| R      | 1             | 1              | 1             | 1              | -1            | -1             | -1            | -1             | $i$           | $i$            | $i$           | $i$            | $i$           | $i$            | $-i$          | $-i$           | $-i$          | $-i$           | $-i$          | $-i$           | 1             | 1              | -1            | -1             |
| Landau | A1            | A1             | A1            | A1             | B1            | B1             | B1            | B1             | E             | E              | E             | E              | E             | E              | E             | E              | E             | E              | E             | E              | A2            | A2             | B2            | B2             |

$$\mathbf{S} = \mathbf{1}/\mathbf{2}, \mathbf{n}_{\text{occ.}} = \{\mathbf{1}, \mathbf{0}, \mathbf{3}, \mathbf{0}\}$$

$$\left( \begin{array}{c|cccccccc} \text{State} & 425 & 426 & 427 & 428 & 429 & 430 & 431 & 432 \\ \hline \text{Sz} & \frac{1}{2} & -\frac{1}{2} & \frac{1}{2} & -\frac{1}{2} & \frac{1}{2} & -\frac{1}{2} & \frac{1}{2} & -\frac{1}{2} \\ \text{Rx} & 1 & 1 & 1 & 1 & 0 & 0 & 0 & 0 \\ \text{Ry} & 1 & 1 & 1 & 1 & 0 & 0 & 0 & 0 \\ \text{R} & 1 & 1 & -1 & -1 & i & i & -i & -i \\ \text{Landau} & \text{A1} & \text{A1} & \text{B1} & \text{B1} & \text{E} & \text{E} & \text{E} & \text{E} \end{array} \right)$$

$$\mathbf{S} = \mathbf{1}/2, \mathbf{n}_{\text{occ.}} = \{1, 0, 2, 1\}$$

| State  | 433           | 434            | 435           | 436            | 437           | 438            | 439           | 440            | 441           | 442            | 443           | 444            | 445           | 446            | 447           | 448            | 449           | 450            | 451           | 452            | 453           | 454            | 455           | 456            |
|--------|---------------|----------------|---------------|----------------|---------------|----------------|---------------|----------------|---------------|----------------|---------------|----------------|---------------|----------------|---------------|----------------|---------------|----------------|---------------|----------------|---------------|----------------|---------------|----------------|
| Sz     | $\frac{1}{2}$ | $-\frac{1}{2}$ | $\frac{1}{2}$ | $-\frac{1}{2}$ | $\frac{1}{2}$ | $-\frac{1}{2}$ | $\frac{1}{2}$ | $-\frac{1}{2}$ | $\frac{1}{2}$ | $-\frac{1}{2}$ | $\frac{1}{2}$ | $-\frac{1}{2}$ | $\frac{1}{2}$ | $-\frac{1}{2}$ | $\frac{1}{2}$ | $-\frac{1}{2}$ | $\frac{1}{2}$ | $-\frac{1}{2}$ | $\frac{1}{2}$ | $-\frac{1}{2}$ | $\frac{1}{2}$ | $-\frac{1}{2}$ | $\frac{1}{2}$ | $-\frac{1}{2}$ |
| Rx     | 1             | 1              | 1             | 1              | 1             | 1              | 1             | 1              | 0             | 0              | 0             | 0              | 0             | 0              | 0             | 0              | 0             | 0              | 0             | 0              | -1            | -1             | -1            | -1             |
| Ry     | 1             | 1              | 1             | 1              | 1             | 1              | 1             | 1              | 0             | 0              | 0             | 0              | 0             | 0              | 0             | 0              | 0             | 0              | 0             | 0              | -1            | -1             | -1            | -1             |
| R      | 1             | 1              | 1             | 1              | -1            | -1             | -1            | -1             | $i$           | $i$            | $i$           | $i$            | $i$           | $i$            | $-i$          | $-i$           | $-i$          | $-i$           | $-i$          | $-i$           | 1             | 1              | -1            | -1             |
| Landau | A1            | A1             | A1            | A1             | B1            | B1             | B1            | B1             | E             | E              | E             | E              | E             | E              | E             | E              | E             | E              | E             | E              | A2            | A2             | B2            | B2             |

$$\mathbf{S} = \mathbf{1}/2, \mathbf{n}_{\text{occ.}} = \{\mathbf{1}, \mathbf{0}, \mathbf{1}, \mathbf{2}\}$$

| State  | 457           | 458            | 459           | 460            | 461           | 462            | 463           | 464            | 465           | 466            | 467           | 468            | 469           | 470            | 471           | 472            | 473           | 474            | 475           | 476            | 477           | 478            | 479           | 480            |
|--------|---------------|----------------|---------------|----------------|---------------|----------------|---------------|----------------|---------------|----------------|---------------|----------------|---------------|----------------|---------------|----------------|---------------|----------------|---------------|----------------|---------------|----------------|---------------|----------------|
| Sz     | $\frac{1}{2}$ | $-\frac{1}{2}$ | $\frac{1}{2}$ | $-\frac{1}{2}$ | $\frac{1}{2}$ | $-\frac{1}{2}$ | $\frac{1}{2}$ | $-\frac{1}{2}$ | $\frac{1}{2}$ | $-\frac{1}{2}$ | $\frac{1}{2}$ | $-\frac{1}{2}$ | $\frac{1}{2}$ | $-\frac{1}{2}$ | $\frac{1}{2}$ | $-\frac{1}{2}$ | $\frac{1}{2}$ | $-\frac{1}{2}$ | $\frac{1}{2}$ | $-\frac{1}{2}$ | $\frac{1}{2}$ | $-\frac{1}{2}$ | $\frac{1}{2}$ | $-\frac{1}{2}$ |
| Rx     | 1             | 1              | 1             | 1              | 1             | 1              | 1             | 1              | 0             | 0              | 0             | 0              | 0             | 0              | 0             | 0              | 0             | 0              | 0             | 0              | -1            | -1             | -1            | -1             |
| Ry     | 1             | 1              | 1             | 1              | 1             | 1              | 1             | 1              | 0             | 0              | 0             | 0              | 0             | 0              | 0             | 0              | 0             | 0              | 0             | 0              | -1            | -1             | -1            | -1             |
| R      | 1             | 1              | 1             | 1              | -1            | -1             | -1            | -1             | $i$           | $i$            | $i$           | $i$            | $i$           | $i$            | $-i$          | $-i$           | $-i$          | $-i$           | $-i$          | $-i$           | 1             | 1              | -1            | -1             |
| Landau | A1            | A1             | A1            | A1             | B1            | B1             | B1            | B1             | E             | E              | E             | E              | E             | E              | E             | E              | E             | E              | E             | E              | A2            | A2             | B2            | B2             |



$$\mathbf{S} = \mathbf{1}/\mathbf{2}, \mathbf{n}_{\text{occ.}} = \{\mathbf{1}, \mathbf{0}, \mathbf{0}, \mathbf{3}\}$$

$$\left( \begin{array}{c|cccccccc} \text{State} & 481 & 482 & 483 & 484 & 485 & 486 & 487 & 488 \\ \hline \text{Sz} & \frac{1}{2} & -\frac{1}{2} & \frac{1}{2} & -\frac{1}{2} & \frac{1}{2} & -\frac{1}{2} & \frac{1}{2} & -\frac{1}{2} \\ \text{Rx} & 1 & 1 & 1 & 1 & 0 & 0 & 0 & 0 \\ \text{Ry} & 1 & 1 & 1 & 1 & 0 & 0 & 0 & 0 \\ \text{R} & 1 & 1 & -1 & -1 & i & i & -i & -i \\ \text{Landau} & \text{A1} & \text{A1} & \text{B1} & \text{B1} & \text{E} & \text{E} & \text{E} & \text{E} \end{array} \right)$$

$$\mathbf{S} = \mathbf{0}, \mathbf{n}_{\text{occ.}} = \{4, \mathbf{0}, \mathbf{0}, \mathbf{0}\}$$

$$\left( \begin{array}{ccc} \text{State} & 489 & 490 \\ \text{Sz} & 0 & 0 \\ \text{Rx} & 1 & -1 \\ \text{Ry} & 1 & -1 \\ \text{R} & 1 & -1 \\ \text{Landau} & \text{A1} & \text{B2} \end{array} \right)$$

$$\mathbf{S} = \mathbf{0}, \mathbf{n}_{\text{occ.}} = \{\mathbf{2}, \mathbf{2}, \mathbf{0}, \mathbf{0}\}$$

| State  | 491 | 492 | 493 | 494  | 495  | 496 |
|--------|-----|-----|-----|------|------|-----|
| Sz     | 0   | 0   | 0   | 0    | 0    | 0   |
| Rx     | 1   | 0   | 0   | 0    | 0    | -1  |
| Ry     | 1   | 0   | 0   | 0    | 0    | -1  |
| R      | -1  | $i$ | $i$ | $-i$ | $-i$ | 1   |
| Landau | B1  | E   | E   | E    | E    | A2  |

$$\mathbf{S} = \mathbf{0}, \mathbf{n}_{\text{occ.}} = \{\mathbf{2}, \mathbf{1}, \mathbf{1}, \mathbf{0}\}$$

$$\left( \begin{array}{cccccccccccccc} \text{State} & 497 & 498 & 499 & 500 & 501 & 502 & 503 & 504 & 505 & 506 & 507 & 508 \\ \text{Sz} & 0 & 0 & 0 & 0 & 0 & 0 & 0 & 0 & 0 & 0 & 0 & 0 \\ \text{Rx} & 1 & 1 & 0 & 0 & 0 & 0 & 0 & 0 & -1 & -1 & -1 & -1 \\ \text{Ry} & 1 & 1 & 0 & 0 & 0 & 0 & 0 & 0 & -1 & -1 & -1 & -1 \\ \text{R} & 1 & -1 & i & i & i & -i & -i & -i & 1 & 1 & -1 & -1 \\ \text{Landau} & \text{A1} & \text{B1} & \text{E} & \text{E} & \text{E} & \text{E} & \text{E} & \text{E} & \text{A2} & \text{A2} & \text{B2} & \text{B2} \end{array} \right)$$



$$\mathbf{S} = \mathbf{0}, \mathbf{n}_{\text{occ.}} = \{\mathbf{2}, \mathbf{0}, \mathbf{2}, \mathbf{0}\}$$

$$\left( \begin{array}{ccccccccc} \text{State} & 521 & 522 & 523 & 524 & 525 & 526 \\ \text{Sz} & 0 & 0 & 0 & 0 & 0 & 0 \\ \text{Rx} & 1 & 0 & 0 & 0 & 0 & -1 \\ \text{Ry} & 1 & 0 & 0 & 0 & 0 & -1 \\ \text{R} & -1 & i & i & -i & -i & 1 \\ \text{Landau} & \text{B1} & \text{E} & \text{E} & \text{E} & \text{E} & \text{A2} \end{array} \right)$$

$$\mathbf{S} = \mathbf{0}, \mathbf{n}_{\text{occ.}} = \{\mathbf{2}, \mathbf{0}, \mathbf{1}, \mathbf{1}\}$$

| State  | 527 | 528 | 529 | 530 | 531 | 532  | 533  | 534  | 535 | 536 | 537 | 538 |
|--------|-----|-----|-----|-----|-----|------|------|------|-----|-----|-----|-----|
| Sz     | 0   | 0   | 0   | 0   | 0   | 0    | 0    | 0    | 0   | 0   | 0   | 0   |
| Rx     | 1   | 1   | 0   | 0   | 0   | 0    | 0    | 0    | -1  | -1  | -1  | -1  |
| Ry     | 1   | 1   | 0   | 0   | 0   | 0    | 0    | 0    | -1  | -1  | -1  | -1  |
| R      | 1   | -1  | $i$ | $i$ | $i$ | $-i$ | $-i$ | $-i$ | 1   | 1   | -1  | -1  |
| Landau | A1  | B1  | E   | E   | E   | E    | E    | E    | A2  | A2  | B2  | B2  |

$$\mathbf{S} = \mathbf{0}, \mathbf{n}_{\text{occ.}} = \{\mathbf{2}, \mathbf{0}, \mathbf{0}, \mathbf{2}\}$$

$$\left( \begin{array}{ccccccccc} \text{State} & 539 & 540 & 541 & 542 & 543 & 544 \\ \text{Sz} & 0 & 0 & 0 & 0 & 0 & 0 \\ \text{Rx} & 1 & 0 & 0 & 0 & 0 & -1 \\ \text{Ry} & 1 & 0 & 0 & 0 & 0 & -1 \\ \text{R} & -1 & i & i & -i & -i & 1 \\ \text{Landau} & \text{B1} & \text{E} & \text{E} & \text{E} & \text{E} & \text{A2} \end{array} \right)$$



$$\mathbf{S} = \mathbf{0}, \text{ n}_{\text{occ.}} = \{0, 4, 0, 0\}$$

$$\left( \begin{array}{cc} \text{State} & 545 \\ \text{Sz} & 0 \\ \text{Rx} & 1 \\ \text{Ry} & 1 \\ \text{R} & 1 \\ \text{Landau} & \text{A1} \end{array} \right)$$

$$\mathbf{S} = \mathbf{0}, \mathbf{n}_{\text{occ.}} = \{\mathbf{0}, \mathbf{3}, \mathbf{1}, \mathbf{0}\}$$

$$\left( \begin{array}{ccccc} \text{State} & 546 & 547 & 548 & 549 \\ \text{Sz} & 0 & 0 & 0 & 0 \\ \text{Rx} & 1 & 1 & 0 & 0 \\ \text{Ry} & 1 & 1 & 0 & 0 \\ \text{R} & 1 & -1 & i & -i \\ \text{Landau} & \text{A1} & \text{B1} & \text{E} & \text{E} \end{array} \right)$$

$$\mathbf{S} = \mathbf{0}, \mathbf{n}_{\text{occ.}} = \{\mathbf{0}, \mathbf{3}, \mathbf{0}, \mathbf{1}\}$$

$$\left( \begin{array}{ccccc} \text{State} & 550 & 551 & 552 & 553 \\ \text{Sz} & 0 & 0 & 0 & 0 \\ \text{Rx} & 1 & 1 & 0 & 0 \\ \text{Ry} & 1 & 1 & 0 & 0 \\ \text{R} & 1 & -1 & i & -i \\ \text{Landau} & \text{A1} & \text{B1} & \text{E} & \text{E} \end{array} \right)$$

$$\mathbf{S} = \mathbf{0}, \mathbf{n}_{\text{occ.}} = \{\mathbf{0}, \mathbf{2}, \mathbf{2}, \mathbf{0}\}$$

| State  | 554 | 555 | 556 | 557 | 558  | 559 |
|--------|-----|-----|-----|-----|------|-----|
| Sz     | 0   | 0   | 0   | 0   | 0    | 0   |
| Rx     | 1   | 1   | 1   | 0   | 0    | -1  |
| Ry     | 1   | 1   | 1   | 0   | 0    | -1  |
| R      | 1   | 1   | -1  | $i$ | $-i$ | -1  |
| Landau | A1  | A1  | B1  | E   | E    | B2  |

$$\mathbf{S} = \mathbf{0}, \mathbf{n}_{\text{occ.}} = \{\mathbf{0}, \mathbf{2}, \mathbf{1}, \mathbf{1}\}$$

| State  | 560 | 561 | 562 | 563 | 564 | 565 | 566 | 567  | 568  | 569  | 570 | 571 |
|--------|-----|-----|-----|-----|-----|-----|-----|------|------|------|-----|-----|
| Sz     | 0   | 0   | 0   | 0   | 0   | 0   | 0   | 0    | 0    | 0    | 0   | 0   |
| Rx     | 1   | 1   | 1   | 1   | 0   | 0   | 0   | 0    | 0    | 0    | -1  | -1  |
| Ry     | 1   | 1   | 1   | 1   | 0   | 0   | 0   | 0    | 0    | 0    | -1  | -1  |
| R      | 1   | 1   | -1  | -1  | $i$ | $i$ | $i$ | $-i$ | $-i$ | $-i$ | 1   | -1  |
| Landau | A1  | A1  | B1  | B1  | E   | E   | E   | E    | E    | E    | A2  | B2  |

$$\mathbf{S} = \mathbf{0}, \mathbf{n}_{\text{occ.}} = \{\mathbf{0}, \mathbf{2}, \mathbf{0}, \mathbf{2}\}$$

$$\left( \begin{array}{cccccc} \text{State} & 572 & 573 & 574 & 575 & 576 & 577 \\ \text{Sz} & 0 & 0 & 0 & 0 & 0 & 0 \\ \text{Rx} & 1 & 1 & 1 & 0 & 0 & -1 \\ \text{Ry} & 1 & 1 & 1 & 0 & 0 & -1 \\ \text{R} & 1 & 1 & -1 & i & -i & -1 \\ \text{Landau} & \text{A1} & \text{A1} & \text{B1} & \text{E} & \text{E} & \text{B2} \end{array} \right)$$

$$\mathbf{S} = \mathbf{0}, \mathbf{n}_{\text{occ.}} = \{\mathbf{0}, \mathbf{1}, \mathbf{3}, \mathbf{0}\}$$

$$\left( \begin{array}{ccccc} \text{State} & 578 & 579 & 580 & 581 \\ \text{Sz} & 0 & 0 & 0 & 0 \\ \text{Rx} & 1 & 1 & 0 & 0 \\ \text{Ry} & 1 & 1 & 0 & 0 \\ \text{R} & 1 & -1 & i & -i \\ \text{Landau} & \text{A1} & \text{B1} & \text{E} & \text{E} \end{array} \right)$$

$$\mathbf{S} = \mathbf{0}, \mathbf{n}_{\text{occ.}} = \{\mathbf{0}, \mathbf{1}, \mathbf{2}, \mathbf{1}\}$$

$$\left( \begin{array}{cccccccccccccc} \text{State} & 582 & 583 & 584 & 585 & 586 & 587 & 588 & 589 & 590 & 591 & 592 & 593 \\ \text{Sz} & 0 & 0 & 0 & 0 & 0 & 0 & 0 & 0 & 0 & 0 & 0 & 0 \\ \text{Rx} & 1 & 1 & 1 & 1 & 0 & 0 & 0 & 0 & 0 & 0 & -1 & -1 \\ \text{Ry} & 1 & 1 & 1 & 1 & 0 & 0 & 0 & 0 & 0 & 0 & -1 & -1 \\ \text{R} & 1 & 1 & -1 & -1 & i & i & i & -i & -i & -i & 1 & -1 \\ \text{Landau} & \text{A1} & \text{A1} & \text{B1} & \text{B1} & \text{E} & \text{E} & \text{E} & \text{E} & \text{E} & \text{E} & \text{A2} & \text{B2} \end{array} \right)$$



$$\mathbf{S} = \mathbf{0}, \mathbf{n}_{\text{occ.}} = \{\mathbf{0}, \mathbf{1}, \mathbf{1}, \mathbf{2}\}$$

$$\left( \begin{array}{cccccccccccccc} \text{State} & 594 & 595 & 596 & 597 & 598 & 599 & 600 & 601 & 602 & 603 & 604 & 605 \\ \text{Sz} & 0 & 0 & 0 & 0 & 0 & 0 & 0 & 0 & 0 & 0 & 0 & 0 \\ \text{Rx} & 1 & 1 & 1 & 1 & 0 & 0 & 0 & 0 & 0 & 0 & -1 & -1 \\ \text{Ry} & 1 & 1 & 1 & 1 & 0 & 0 & 0 & 0 & 0 & 0 & -1 & -1 \\ \text{R} & 1 & 1 & -1 & -1 & i & i & i & -i & -i & -i & 1 & -1 \\ \text{Landau} & \text{A1} & \text{A1} & \text{B1} & \text{B1} & \text{E} & \text{E} & \text{E} & \text{E} & \text{E} & \text{E} & \text{A2} & \text{B2} \end{array} \right)$$

$$\mathbf{S} = \mathbf{0}, \text{ n}_{\text{occ.}} = \{\mathbf{0}, \mathbf{0}, \mathbf{4}, \mathbf{0}\}$$

$$\left( \begin{array}{cc} \text{State} & 606 \\ \text{Sz} & 0 \\ \text{Rx} & 1 \\ \text{Ry} & 1 \\ \text{R} & 1 \\ \text{Landau} & \text{A1} \end{array} \right)$$

$$\mathbf{S} = \mathbf{0}, \mathbf{n}_{\text{occ.}} = \{\mathbf{0}, \mathbf{1}, \mathbf{0}, \mathbf{3}\}$$

$$\left( \begin{array}{ccccc} \text{State} & 607 & 608 & 609 & 610 \\ \text{Sz} & 0 & 0 & 0 & 0 \\ \text{Rx} & 1 & 1 & 0 & 0 \\ \text{Ry} & 1 & 1 & 0 & 0 \\ \text{R} & 1 & -1 & i & -i \\ \text{Landau} & \text{A1} & \text{B1} & \text{E} & \text{E} \end{array} \right)$$

$$\mathbf{S} = \mathbf{0}, \text{ n}_{\text{occ.}} = \{\mathbf{0}, \mathbf{0}, \mathbf{3}, \mathbf{1}\}$$

$$\left( \begin{array}{ccccc} \text{State} & 611 & 612 & 613 & 614 \\ \text{Sz} & 0 & 0 & 0 & 0 \\ \text{Rx} & 1 & 1 & 0 & 0 \\ \text{Ry} & 1 & 1 & 0 & 0 \\ \text{R} & 1 & -1 & i & -i \\ \text{Landau} & \text{A1} & \text{B1} & \text{E} & \text{E} \end{array} \right)$$

$$\mathbf{S} = \mathbf{0}, \mathbf{n}_{\text{occ.}} = \{\mathbf{0}, \mathbf{0}, \mathbf{2}, \mathbf{2}\}$$

$$\left( \begin{array}{ccccccccc} \text{State} & 615 & 616 & 617 & 618 & 619 & 620 \\ \text{Sz} & 0 & 0 & 0 & 0 & 0 & 0 \\ \text{Rx} & 1 & 1 & 1 & 0 & 0 & -1 \\ \text{Ry} & 1 & 1 & 1 & 0 & 0 & -1 \\ \text{R} & 1 & 1 & -1 & i & -i & -1 \\ \text{Landau} & \text{A1} & \text{A1} & \text{B1} & \text{E} & \text{E} & \text{B2} \end{array} \right)$$

$$\mathbf{S} = \mathbf{0}, \mathbf{n}_{\text{occ.}} = \{\mathbf{0}, \mathbf{0}, 1, \mathbf{3}\}$$

$$\left( \begin{array}{ccccc} \text{State} & 621 & 622 & 623 & 624 \\ \text{Sz} & 0 & 0 & 0 & 0 \\ \text{Rx} & 1 & 1 & 0 & 0 \\ \text{Ry} & 1 & 1 & 0 & 0 \\ \text{R} & 1 & -1 & i & -i \\ \text{Landau} & \text{A1} & \text{B1} & \text{E} & \text{E} \end{array} \right)$$

$$\mathbf{S} = \mathbf{0}, \text{ n}_{\text{occ.}} = \{0, 0, 0, 4\}$$

$$\left( \begin{array}{cc} \text{State} & 625 \\ \text{Sz} & 0 \\ \text{Rx} & 1 \\ \text{Ry} & 1 \\ \text{R} & 1 \\ \text{Landau} & \text{A1} \end{array} \right)$$

$$S = 10, \text{ n}_{\text{occ.}} = \{4\}$$

[illegible]





$$S = 8, n_{occ} = \{4\}$$

[illegible]

$$S = 7 \quad n = 14$$

$$S = \{s_1, \dots, s_n\} = [A]$$



$$n_2 = 1 \Rightarrow [1]$$

$$C = 2 \times 10^{-4} \text{ m} = [4]$$

$$S = 2 \quad n = 4$$



$$\mathbf{S} = \mathbf{1}, \mathbf{n}_{\text{occ.}} = \{4\}$$

| State  | 1246 | 1247 | 1248 | 1249 | 1250 | 1251 | 1252 | 1253 | 1254 | 1255 | 1256 | 1257 | 1258 | 1259 | 1260 | 1261 | 1262 | 1263 | 1264 | 1265 | 1266 | 1267 | 1268 | 1269 | 1270 | 1271 | 1272 | 1273 | 1274 | 1275 | 1276 | 1277 | 1278 | 1279 | 1280 | 1281 | 1282 | 1283 | 1284 | 1285 | 1286 | 1287 | 1288 | 1289 | 1290 |    |    |
|--------|------|------|------|------|------|------|------|------|------|------|------|------|------|------|------|------|------|------|------|------|------|------|------|------|------|------|------|------|------|------|------|------|------|------|------|------|------|------|------|------|------|------|------|------|------|----|----|
| Sz     | 1    | 0    | -1   | 1    | 0    | -1   | 1    | 0    | -1   | 1    | 0    | -1   | 1    | 0    | -1   | 1    | 0    | -1   | 1    | 0    | -1   | 1    | 0    | -1   | 1    | 0    | -1   | 1    | 0    | -1   | 1    | 0    | -1   | 1    | 0    | -1   | 1    | 0    | -1   | 1    | 0    | -1   |      |      |      |    |    |
| Rx     | 1    | 1    | 1    | 1    | 1    | 1    | 1    | 1    | 1    | 0    | 0    | 0    | 0    | 0    | 0    | 0    | 0    | 0    | 0    | 0    | 0    | 0    | 0    | 0    | 0    | 0    | 0    | 0    | 0    | 0    | 0    | 0    | 0    | 0    | 0    | 0    | 0    | 0    | -1   | -1   | -1   | -1   | -1   | -1   |      |    |    |
| Ry     | 1    | 1    | 1    | 1    | 1    | 1    | 1    | 1    | 1    | 0    | 0    | 0    | 0    | 0    | 0    | 0    | 0    | 0    | 0    | 0    | 0    | 0    | 0    | 0    | 0    | 0    | 0    | 0    | 0    | 0    | 0    | 0    | 0    | 0    | 0    | 0    | 0    | 0    | 0    | -1   | -1   | -1   | -1   | -1   | -1   |    |    |
| R      | -1   | -1   | -1   | -1   | -1   | -1   | -1   | -1   | -1   | $i$  | $i$  | $i$  | $i$  | $i$  | $i$  | $i$  | $i$  | $i$  | $i$  | $i$  | $i$  | $i$  | $i$  | $i$  | $i$  | $-i$ | $-i$ | $-i$ | $-i$ | $-i$ | $-i$ | $-i$ | $-i$ | $-i$ | $-i$ | $-i$ | $-i$ | $-i$ | 1    | 1    | 1    | 1    | 1    | 1    |      |    |    |
| Landau | B1   | B1   | B1   | B1   | B1   | B1   | B1   | B1   | B1   | E    | E    | E    | E    | E    | E    | E    | E    | E    | E    | E    | E    | E    | E    | E    | E    | E    | E    | E    | E    | E    | E    | E    | E    | E    | E    | E    | E    | E    | E    | E    | E    | A2   | A2   | A2   | A2   | A2 | A2 |

$$\mathbf{S} = \mathbf{0}, \mathbf{n}_{\text{occ.}} = \{4\}$$

| State  | 1291 | 1292 | 1293 | 1294 | 1295 | 1296 |
|--------|------|------|------|------|------|------|
| Sz     | 0    | 0    | 0    | 0    | 0    | 0    |
| Rx     | 1    | 1    | 1    | -1   | -1   | -1   |
| Ry     | 1    | 1    | 1    | -1   | -1   | -1   |
| R      | 1    | 1    | 1    | -1   | -1   | -1   |
| Landau | A1   | A1   | A1   | B2   | B2   | B2   |

$$S = 8, \text{ n}_{\text{occ.}} = \{4, 0\}$$

[illegible]

[illegible]



$$\mathbf{S} = \mathbf{6}, \mathbf{n}_{\text{occ.}}$$

$$\left( \begin{array}{c} \text{State} \\ \text{Sz} \\ \text{Rx} \\ \text{Ry} \\ \text{R} \\ \text{Landau} \end{array} \right)$$

[illegible]

$$S = 5 \quad n_{\text{max}} = \{4 \ 0\}$$







$$S = 4, \quad n_{\text{max}} = \{3, 1\}$$

$$\mathbf{S} = 4, \mathbf{n}_{\text{occ}}$$

$$\left( \begin{array}{c} \text{State} \\ \text{Sz} \\ \text{Rx} \\ \text{Ry} \\ \text{R} \\ \text{Landau} \end{array} \right)$$

[illegible]



$$S = 3, n_{\text{max}} = \{3, 1\}$$

$$\mathbf{S} = \mathbf{3}, \mathbf{n}_{\text{occ.}} = \{\mathbf{2}, \mathbf{2}\}$$

|        |     |     |     |     |     |     |     |          |          |          |          |          |          |          |          |          |          |          |          |          |          |            |            |            |            |            |            |            |            |            |            |            |            |            |     |     |     |     |     |     |     |     |    |    |
|--------|-----|-----|-----|-----|-----|-----|-----|----------|----------|----------|----------|----------|----------|----------|----------|----------|----------|----------|----------|----------|----------|------------|------------|------------|------------|------------|------------|------------|------------|------------|------------|------------|------------|------------|-----|-----|-----|-----|-----|-----|-----|-----|----|----|
| State  | 919 | 920 | 921 | 922 | 923 | 924 | 925 | 926      | 927      | 928      | 929      | 930      | 931      | 932      | 933      | 934      | 935      | 936      | 937      | 938      | 939      | 940        | 941        | 942        | 943        | 944        | 945        | 946        | 947        | 948        | 949        | 950        | 951        | 952        | 953 | 954 | 955 | 956 | 957 | 958 | 959 | 960 |    |    |
| Sz     | 3   | 2   | 1   | 0   | -1  | -2  | -3  | 3        | 2        | 1        | 0        | -1       | -2       | -3       | 3        | 2        | 1        | 0        | -1       | -2       | -3       | 3          | 2          | 1          | 0          | -1         | -2         | -3         | 3          | 2          | 1          | 0          | -1         | -2         | -3  | 3   | 2   | 1   | 0   | -1  | -2  | -3  |    |    |
| Rx     | 1   | 1   | 1   | 1   | 1   | 1   | 1   | 0        | 0        | 0        | 0        | 0        | 0        | 0        | 0        | 0        | 0        | 0        | 0        | 0        | 0        | 0          | 0          | 0          | 0          | 0          | 0          | 0          | 0          | 0          | 0          | 0          | 0          | 0          | 0   | -1  | -1  | -1  | -1  | -1  | -1  | -1  |    |    |
| Ry     | 1   | 1   | 1   | 1   | 1   | 1   | 1   | 0        | 0        | 0        | 0        | 0        | 0        | 0        | 0        | 0        | 0        | 0        | 0        | 0        | 0        | 0          | 0          | 0          | 0          | 0          | 0          | 0          | 0          | 0          | 0          | 0          | 0          | 0          | 0   | 0   | -1  | -1  | -1  | -1  | -1  | -1  | -1 |    |
| R      | -1  | -1  | -1  | -1  | -1  | -1  | -1  | <i>i</i> | <i>i</i> | <i>i</i> | <i>i</i> | <i>i</i> | <i>i</i> | <i>i</i> | <i>i</i> | <i>i</i> | <i>i</i> | <i>i</i> | <i>i</i> | <i>i</i> | <i>i</i> | - <i>i</i> | - <i>i</i> | - <i>i</i> | - <i>i</i> | - <i>i</i> | - <i>i</i> | - <i>i</i> | - <i>i</i> | - <i>i</i> | - <i>i</i> | - <i>i</i> | - <i>i</i> | - <i>i</i> | 1   | 1   | 1   | 1   | 1   | 1   | 1   |     |    |    |
| Landau | B1  | B1  | B1  | B1  | B1  | B1  | B1  | E        | E        | E        | E        | E        | E        | E        | E        | E        | E        | E        | E        | E        | E        | E          | E          | E          | E          | E          | E          | E          | E          | E          | E          | E          | E          | E          | E   | E   | E   | A2  | A2  | A2  | A2  | A2  | A2 | A2 |

$$S = 2, n_{\text{acc}} = \{4, 0\}$$

[illegible]





$$\mathbf{S} = \mathbf{2}, \mathbf{n}_{\text{occ.}} = \{\mathbf{2}, \mathbf{2}\}$$

| State  | 1141 | 1142 | 1143 | 1144 | 1145 | 1146 | 1147 | 1148 | 1149 | 1150 | 1151 | 1152 | 1153 | 1154 | 1155 | 1156 | 1157 | 1158 | 1159 | 1160     | 1161     | 1162     | 1163     | 1164     | 1165       | 1166       | 1167       | 1168       | 1169       | 1170 |    |    |    |
|--------|------|------|------|------|------|------|------|------|------|------|------|------|------|------|------|------|------|------|------|----------|----------|----------|----------|----------|------------|------------|------------|------------|------------|------|----|----|----|
| Sz     | 2    | 1    | 0    | -1   | -2   | 2    | 1    | 0    | -1   | -2   | 2    | 1    | 0    | -1   | -2   | 2    | 1    | 0    | -1   | -2       | 2        | 1        | 0        | -1       | -2         | 2          | 1          | 0          | -1         | -2   |    |    |    |
| Rx     | 1    | 1    | 1    | 1    | 1    | 1    | 1    | 1    | 1    | 1    | 1    | 1    | 1    | 1    | 1    | 1    | 1    | 1    | 1    | 0        | 0        | 0        | 0        | 0        | 0          | 0          | 0          | -1         | -1         | -1   | -1 |    |    |
| Ry     | 1    | 1    | 1    | 1    | 1    | 1    | 1    | 1    | 1    | 1    | 1    | 1    | 1    | 1    | 1    | 1    | 1    | 1    | 1    | 0        | 0        | 0        | 0        | 0        | 0          | 0          | 0          | -1         | -1         | -1   | -1 |    |    |
| R      | 1    | 1    | 1    | 1    | 1    | 1    | 1    | 1    | 1    | 1    | 1    | -1   | -1   | -1   | -1   | -1   | -1   | -1   | -1   | <i>i</i> | <i>i</i> | <i>i</i> | <i>i</i> | <i>i</i> | - <i>i</i> | - <i>i</i> | - <i>i</i> | - <i>i</i> | - <i>i</i> | -1   | -1 | -1 | -1 |
| Landau | A1   | A1   | A1   | A1   | A1   | A1   | A1   | A1   | A1   | A1   | A1   | B1   | B1   | B1   | B1   | B1   | B1   | E    | E    | E        | E        | E        | E        | E        | E          | E          | E          | E          | B2         | B2   | B2 | B2 | B2 |



$$\mathbf{S} = \mathbf{1}, \mathbf{n}_{\text{occ.}} = \{4, \mathbf{0}\}$$

| State  | 1191 | 1192 | 1193 | 1194 | 1195 | 1196 | 1197     | 1198     | 1199     | 1200     | 1201     | 1202     | 1203     | 1204     | 1205     | 1206     | 1207     | 1208     | 1209     | 1210       | 1211       | 1212       | 1213       | 1214       | 1215       | 1216       | 1217       | 1218       | 1219       | 1220       | 1221 | 1222 | 1223 | 1224 | 1225 | 1226 |    |    |    |    |
|--------|------|------|------|------|------|------|----------|----------|----------|----------|----------|----------|----------|----------|----------|----------|----------|----------|----------|------------|------------|------------|------------|------------|------------|------------|------------|------------|------------|------------|------|------|------|------|------|------|----|----|----|----|
| Sz     | 1    | 0    | -1   | 1    | 0    | -1   | 1        | 0        | -1       | 1        | 0        | -1       | 1        | 0        | -1       | 1        | 0        | -1       | 1        | 0          | -1         | 1          | 0          | -1         | 1          | 0          | -1         | 1          | 0          | -1         | 1    | 0    | -1   | 1    | 0    | -1   |    |    |    |    |
| Rx     | 1    | 1    | 1    | 1    | 1    | 1    | 0        | 0        | 0        | 0        | 0        | 0        | 0        | 0        | 0        | 0        | 0        | 0        | 0        | 0          | 0          | 0          | 0          | 0          | 0          | 0          | 0          | 0          | 0          | 0          | 0    | -1   | -1   | -1   | -1   | -1   | -1 |    |    |    |
| Ry     | 1    | 1    | 1    | 1    | 1    | 1    | 0        | 0        | 0        | 0        | 0        | 0        | 0        | 0        | 0        | 0        | 0        | 0        | 0        | 0          | 0          | 0          | 0          | 0          | 0          | 0          | 0          | 0          | 0          | 0          | 0    | -1   | -1   | -1   | -1   | -1   | -1 |    |    |    |
| R      | -1   | -1   | -1   | -1   | -1   | -1   | <i>i</i> | <i>i</i> | <i>i</i> | <i>i</i> | <i>i</i> | <i>i</i> | <i>i</i> | <i>i</i> | <i>i</i> | <i>i</i> | <i>i</i> | <i>i</i> | <i>i</i> | - <i>i</i> | - <i>i</i> | - <i>i</i> | - <i>i</i> | - <i>i</i> | - <i>i</i> | - <i>i</i> | - <i>i</i> | - <i>i</i> | - <i>i</i> | - <i>i</i> | 1    | 1    | 1    | 1    | 1    | 1    |    |    |    |    |
| Landau | B1   | B1   | B1   | B1   | B1   | B1   | E        | E        | E        | E        | E        | E        | E        | E        | E        | E        | E        | E        | E        | E          | E          | E          | E          | E          | E          | E          | E          | E          | E          | E          | E    | E    | E    | E    | A2   | A2   | A2 | A2 | A2 | A2 |

$$\mathbf{S} = \mathbf{1}, \mathbf{n}_{\text{occ.}} = \{\mathbf{3}, \mathbf{1}\}$$

| State  | 1227 | 1228 | 1229 | 1230 | 1231 | 1232 | 1233 | 1234 | 1235 | 1236 | 1237 | 1238 | 1239 | 1240 | 1241 | 1242 | 1243 | 1244 | 1245 | 1246 | 1247 | 1248 | 1249 | 1250 | 1251 | 1252 | 1253 | 1254 | 1255 | 1256 | 1257 | 1258 | 1259 | 1260 | 1261 | 1262 |    |
|--------|------|------|------|------|------|------|------|------|------|------|------|------|------|------|------|------|------|------|------|------|------|------|------|------|------|------|------|------|------|------|------|------|------|------|------|------|----|
| Sz     | 1    | 0    | -1   | 1    | 0    | -1   | 1    | 0    | -1   | 1    | 0    | -1   | 1    | 0    | -1   | 1    | 0    | -1   | 1    | 0    | -1   | 1    | 0    | -1   | 1    | 0    | -1   | 1    | 0    | -1   | 1    | 0    | -1   | 1    | 0    | -1   |    |
| Rx     | 1    | 1    | 1    | 1    | 1    | 1    | 0    | 0    | 0    | 0    | 0    | 0    | 0    | 0    | 0    | 0    | 0    | 0    | 0    | 0    | 0    | 0    | 0    | 0    | 0    | -1   | -1   | -1   | -1   | -1   | -1   | -1   | -1   | -1   | -1   | -1   |    |
| Ry     | 1    | 1    | 1    | 1    | 1    | 1    | 0    | 0    | 0    | 0    | 0    | 0    | 0    | 0    | 0    | 0    | 0    | 0    | 0    | 0    | 0    | 0    | 0    | 0    | 0    | -1   | -1   | -1   | -1   | -1   | -1   | -1   | -1   | -1   | -1   | -1   |    |
| R      | 1    | 1    | 1    | -1   | -1   | -1   | $i$  | $i$  | $i$  | $i$  | $i$  | $i$  | $i$  | $i$  | $i$  | $-i$ | $-i$ | $-i$ | $-i$ | $-i$ | $-i$ | $-i$ | $-i$ | $-i$ | 1    | 1    | 1    | 1    | 1    | 1    | -1   | -1   | -1   | -1   | -1   | -1   |    |
| Landau | A1   | A1   | A1   | B1   | B1   | B1   | E    | E    | E    | E    | E    | E    | E    | E    | E    | E    | E    | E    | E    | E    | E    | E    | E    | E    | E    | A2   | A2   | A2   | A2   | A2   | A2   | B2   | B2   | B2   | B2   | B2   | B2 |

$$S = 1, \text{ n}_{\text{occ.}} = \{2, 2\}$$

$$\left( \begin{array}{c|cccccccccccccccccccc} \text{State} & 1263 & 1264 & 1265 & 1266 & 1267 & 1268 & 1269 & 1270 & 1271 & 1272 & 1273 & 1274 & 1275 & 1276 & 1277 & 1278 & 1279 & 1280 \\ \hline \text{Sz} & 1 & 0 & -1 & 1 & 0 & -1 & 1 & 0 & -1 & 1 & 0 & -1 & 1 & 0 & -1 & 1 & 0 & -1 \\ \text{Rx} & 1 & 1 & 1 & 0 & 0 & 0 & 0 & 0 & 0 & 0 & 0 & 0 & 0 & 0 & 0 & -1 & -1 & -1 \\ \text{Ry} & 1 & 1 & 1 & 0 & 0 & 0 & 0 & 0 & 0 & 0 & 0 & 0 & 0 & 0 & 0 & -1 & -1 & -1 \\ \text{R} & -1 & -1 & -1 & i & i & i & i & i & i & i & -i & -i & -i & -i & -i & 1 & 1 & 1 \\ \text{Landau} & \text{B1} & \text{B1} & \text{B1} & \text{E} & \text{E} & \text{E} & \text{E} & \text{E} & \text{E} & \text{E} & \text{E} & \text{E} & \text{E} & \text{E} & \text{E} & \text{A2} & \text{A2} & \text{A2} \end{array} \right)$$

$$\mathbf{S} = \mathbf{0}, \mathbf{n}_{\text{occ.}} = \{4, \mathbf{0}\}$$

| State  | 1281 | 1282 | 1283 | 1284 | 1285 |
|--------|------|------|------|------|------|
| Sz     | 0    | 0    | 0    | 0    | 0    |
| Rx     | 1    | 1    | 1    | -1   | -1   |
| Ry     | 1    | 1    | 1    | -1   | -1   |
| R      | 1    | 1    | 1    | -1   | -1   |
| Landau | A1   | A1   | A1   | B2   | B2   |

$$\mathbf{S} = \mathbf{0}, \text{ n}_{\text{occ.}} = \{\mathbf{3}, \mathbf{1}\}$$

$$\left( \begin{array}{ccccc} \text{State} & 1286 & 1287 & 1288 & 1289 \\ \text{Sz} & 0 & 0 & 0 & 0 \\ \text{Rx} & 1 & 1 & 0 & 0 \\ \text{Ry} & 1 & 1 & 0 & 0 \\ \text{R} & 1 & -1 & i & -i \\ \text{Landau} & \text{A1} & \text{B1} & \text{E} & \text{E} \end{array} \right)$$

$$\mathbf{S} = \mathbf{0}, \mathbf{n}_{\text{occ.}} = \{\mathbf{2}, \mathbf{2}\}$$

| State  | 1290 | 1291 | 1292 | 1293 | 1294 | 1295 |
|--------|------|------|------|------|------|------|
| Sz     | 0    | 0    | 0    | 0    | 0    | 0    |
| Rx     | 1    | 1    | 1    | 0    | 0    | -1   |
| Ry     | 1    | 1    | 1    | 0    | 0    | -1   |
| R      | 1    | 1    | -1   | $i$  | $-i$ | -1   |
| Landau | A1   | A1   | B1   | E    | E    | B2   |



$$\mathbf{S} = \mathbf{0}, \text{ n}_{\text{occ.}} = \{0, 4\}$$

$$\left( \begin{array}{cc} \text{State} & 1296 \\ \text{Sz} & 0 \\ \text{Rx} & 1 \\ \text{Ry} & 1 \\ \text{R} & 1 \\ \text{Landau} & \text{A1} \end{array} \right)$$

$$S = 6, \text{ n}_{\text{occ.}} = \{4, 0\}$$

[illegible]



[illegible]





$$\mathbf{S} = 4, \mathbf{n}_{\text{occ.}}$$

$$\left( \begin{array}{c} \text{State} \\ \text{Sz} \\ \text{Rx} \\ \text{Ry} \\ \text{R} \\ \text{Landau} \end{array} \right)$$

[illegible]







$$S = 3 \quad n_{\text{max}} = \{2, 2\}$$

$$\mathbf{S} = \mathbf{3}, \mathbf{n}_{\text{occ.}} = \{1, 3\}$$

[illegible]

$$\mathbf{S} = \mathbf{2}, \mathbf{n}_{\text{occ.}}$$

$$\left( \begin{array}{c} \text{State} \\ \text{Sz} \\ \text{Rx} \\ \text{Ry} \\ \text{R} \\ \text{Landau} \end{array} \right)$$

[illegible]



$$S = 2 \quad n = 2 \quad \lambda = 2$$



$$\mathbf{S} = \mathbf{2}, \mathbf{n}_{\text{occ.}} = \{\mathbf{0}, \mathbf{4}\}$$

| State  | 1046 | 1047 | 1048 | 1049 | 1050 |
|--------|------|------|------|------|------|
| Sz     | 2    | 1    | 0    | -1   | -2   |
| Rx     | 1    | 1    | 1    | 1    | 1    |
| Ry     | 1    | 1    | 1    | 1    | 1    |
| R      | 1    | 1    | 1    | 1    | 1    |
| Landau | A1   | A1   | A1   | A1   | A1   |



$$\mathbf{S} = \mathbf{1}, \mathbf{n}_{\text{occ.}} = \{4, \mathbf{0}\}$$

| State  | 1051 | 1052 | 1053 | 1054 | 1055 | 1056 | 1057 | 1058 | 1059 | 1060 | 1061 | 1062 | 1063 | 1064 | 1065 | 1066 | 1067 | 1068 | 1069 | 1070 | 1071 | 1072 | 1073 | 1074 | 1075 | 1076 | 1077 |
|--------|------|------|------|------|------|------|------|------|------|------|------|------|------|------|------|------|------|------|------|------|------|------|------|------|------|------|------|
| Sz     | 1    | 0    | -1   | 1    | 0    | -1   | 1    | 0    | -1   | 1    | 0    | -1   | 1    | 0    | -1   | 1    | 0    | -1   | 1    | 0    | -1   | 1    | 0    | -1   | 1    | 0    | -1   |
| Rx     | 1    | 1    | 1    | 1    | 1    | 1    | 0    | 0    | 0    | 0    | 0    | 0    | 0    | 0    | 0    | 0    | 0    | 0    | 0    | 0    | 0    | 0    | 0    | 0    | -1   | -1   | -1   |
| Ry     | 1    | 1    | 1    | 1    | 1    | 1    | 0    | 0    | 0    | 0    | 0    | 0    | 0    | 0    | 0    | 0    | 0    | 0    | 0    | 0    | 0    | 0    | 0    | 0    | -1   | -1   | -1   |
| R      | -1   | -1   | -1   | -1   | -1   | -1   | $i$  | $i$  | $i$  | $i$  | $i$  | $i$  | $i$  | $i$  | $i$  | $i$  | $-i$ | $-i$ | $-i$ | $-i$ | $-i$ | $-i$ | $-i$ | $-i$ | 1    | 1    | 1    |
| Landau | B1   | B1   | B1   | B1   | B1   | B1   | E    | E    | E    | E    | E    | E    | E    | E    | E    | E    | E    | E    | E    | E    | E    | E    | E    | E    | A2   | A2   | A2   |





$$\mathbf{S} = \mathbf{1}, \mathbf{n}_{\text{occ.}} = \{\mathbf{1}, \mathbf{3}\}$$

| State  | 1222 | 1223 | 1224 | 1225 | 1226 | 1227 | 1228 | 1229 | 1230 | 1231 | 1232 | 1233 | 1234 | 1235 | 1236 | 1237 | 1238 | 1239 | 1240 | 1241 | 1242 | 1243 | 1244 | 1245 | 1246 | 1247 | 1248 | 1249 | 1250 | 1251 | 1252 | 1253 | 1254 | 1255 | 1256 | 1257 |
|--------|------|------|------|------|------|------|------|------|------|------|------|------|------|------|------|------|------|------|------|------|------|------|------|------|------|------|------|------|------|------|------|------|------|------|------|------|
| Sz     | 1    | 0    | -1   | 1    | 0    | -1   | 1    | 0    | -1   | 1    | 0    | -1   | 1    | 0    | -1   | 1    | 0    | -1   | 1    | 0    | -1   | 1    | 0    | -1   | 1    | 0    | -1   | 1    | 0    | -1   | 1    | 0    | -1   | 1    | 0    | -1   |
| Rx     | 1    | 1    | 1    | 1    | 1    | 1    | 1    | 1    | 1    | 1    | 1    | 1    | 0    | 0    | 0    | 0    | 0    | 0    | 0    | 0    | 0    | 0    | 0    | 0    | 0    | 0    | 0    | 0    | 0    | 0    | 0    | -1   | -1   | -1   | -1   | -1   |
| Ry     | 1    | 1    | 1    | 1    | 1    | 1    | 1    | 1    | 1    | 1    | 1    | 1    | 0    | 0    | 0    | 0    | 0    | 0    | 0    | 0    | 0    | 0    | 0    | 0    | 0    | 0    | 0    | 0    | 0    | 0    | -1   | -1   | -1   | -1   | -1   |      |
| R      | 1    | 1    | 1    | 1    | 1    | 1    | 1    | -1   | -1   | -1   | -1   | -1   | $i$  | $i$  | $i$  | $i$  | $i$  | $i$  | $i$  | $i$  | $i$  | $i$  | $i$  | $-i$ | $-i$ | $-i$ | $-i$ | $-i$ | $-i$ | $-i$ | 1    | 1    | 1    | -1   | -1   | -1   |
| Landau | A1   | A1   | A1   | A1   | A1   | A1   | B1   | B1   | B1   | B1   | B1   | B1   | E    | E    | E    | E    | E    | E    | E    | E    | E    | E    | E    | E    | E    | E    | E    | E    | E    | E    | A2   | A2   | A2   | B2   | B2   | B2   |



$$\mathbf{S} = \mathbf{0}, \mathbf{n}_{\text{occ.}} = \{4, \mathbf{0}\}$$

| State  | 1267 | 1268 | 1269 | 1270 |
|--------|------|------|------|------|
| Sz     | 0    | 0    | 0    | 0    |
| Rx     | 1    | 1    | -1   | -1   |
| Ry     | 1    | 1    | -1   | -1   |
| R      | 1    | 1    | -1   | -1   |
| Landau | A1   | A1   | B2   | B2   |

$$\mathbf{S} = \mathbf{0}, \mathbf{n}_{\text{occ.}} = \{\mathbf{3}, \mathbf{1}\}$$

$$\left( \begin{array}{cccccccc} \text{State} & 1271 & 1272 & 1273 & 1274 & 1275 & 1276 & 1277 & 1278 \\ \text{Sz} & 0 & 0 & 0 & 0 & 0 & 0 & 0 & 0 \\ \text{Rx} & 1 & 1 & 0 & 0 & 0 & 0 & -1 & -1 \\ \text{Ry} & 1 & 1 & 0 & 0 & 0 & 0 & -1 & -1 \\ \text{R} & 1 & -1 & i & i & -i & -i & 1 & -1 \\ \text{Landau} & \text{A1} & \text{B1} & \text{E} & \text{E} & \text{E} & \text{E} & \text{A2} & \text{B2} \end{array} \right)$$

$$\mathbf{S} = \mathbf{0}, \mathbf{n}_{\text{occ.}} = \{\mathbf{2}, \mathbf{2}\}$$

| State  | 1279 | 1280 | 1281 | 1282 | 1283 | 1284 | 1285 | 1286 | 1287 | 1288 | 1289 | 1290 |
|--------|------|------|------|------|------|------|------|------|------|------|------|------|
| Sz     | 0    | 0    | 0    | 0    | 0    | 0    | 0    | 0    | 0    | 0    | 0    | 0    |
| Rx     | 1    | 1    | 1    | 1    | 0    | 0    | 0    | 0    | -1   | -1   | -1   | -1   |
| Ry     | 1    | 1    | 1    | 1    | 0    | 0    | 0    | 0    | -1   | -1   | -1   | -1   |
| R      | 1    | 1    | 1    | -1   | $i$  | $i$  | $-i$ | $-i$ | 1    | -1   | -1   | -1   |
| Landau | A1   | A1   | A1   | B1   | E    | E    | E    | E    | A2   | B2   | B2   | B2   |



$$\mathbf{S} = \mathbf{0}, \text{ n}_{\text{occ.}} = \{1, 3\}$$

$$\left( \begin{array}{ccccc} \text{State} & 1291 & 1292 & 1293 & 1294 \\ \text{Sz} & 0 & 0 & 0 & 0 \\ \text{Rx} & 1 & 1 & 0 & 0 \\ \text{Ry} & 1 & 1 & 0 & 0 \\ \text{R} & 1 & -1 & i & -i \\ \text{Landau} & \text{A1} & \text{B1} & \text{E} & \text{E} \end{array} \right)$$

$$\mathbf{S} = \mathbf{0}, \text{ n}_{\text{occ.}} = \{0, 4\}$$

$$\left( \begin{array}{ccc} \text{State} & 1295 & 1296 \\ \text{Sz} & 0 & 0 \\ \text{Rx} & 1 & -1 \\ \text{Ry} & 1 & -1 \\ \text{R} & 1 & -1 \\ \text{Landau} & \text{A1} & \text{B2} \end{array} \right)$$

$$S = 6, \text{ n}_{\text{occ.}} = \{4, 0, 0\}$$

[illegible]





$$\mathbf{S} = \mathbf{9}/\mathbf{2}, \mathbf{n}_{\text{occ.}} = \{\mathbf{3}, \mathbf{0}, \mathbf{1}\}$$

[illegible]











$\mathbf{S} = \mathbf{3}, \mathbf{n}_{\text{occ.}} = \{\mathbf{2}, \mathbf{2}, \mathbf{0}\}$

| State  | 379 | 380 | 381 | 382 | 383 | 384 | 385 | 386 | 387 | 388 | 389 | 390 | 391 | 392 | 393 | 394 | 395 | 396 | 397 | 398 | 399 | 400 | 401 | 402 | 403 | 404 | 405 | 406 | 407 | 408 | 409 | 410 | 411 | 412 | 413 | 414 | 415 | 416 | 417 | 418 | 419 | 420 |    |
|--------|-----|-----|-----|-----|-----|-----|-----|-----|-----|-----|-----|-----|-----|-----|-----|-----|-----|-----|-----|-----|-----|-----|-----|-----|-----|-----|-----|-----|-----|-----|-----|-----|-----|-----|-----|-----|-----|-----|-----|-----|-----|-----|----|
| Sz     | 3   | 2   | 1   | 0   | -1  | -2  | -3  | 3   | 2   | 1   | 0   | -1  | -2  | -3  | 3   | 2   | 1   | 0   | -1  | -2  | -3  | 3   | 2   | 1   | 0   | -1  | -2  | -3  | 3   | 2   | 1   | 0   | -1  | -2  | -3  | 3   | 2   | 1   | 0   | -1  | -2  | -3  |    |
| Rx     | 1   | 1   | 1   | 1   | 1   | 1   | 1   | 1   | 1   | 1   | 1   | 1   | 1   | 1   | 1   | 1   | 1   | 1   | 1   | 1   | 1   | 0   | 0   | 0   | 0   | 0   | 0   | 0   | 0   | 0   | 0   | 0   | 0   | 0   | 0   | -1  | -1  | -1  | -1  | -1  | -1  | -1  |    |
| Ry     | 1   | 1   | 1   | 1   | 1   | 1   | 1   | 1   | 1   | 1   | 1   | 1   | 1   | 1   | 1   | 1   | 1   | 1   | 1   | 1   | 1   | 0   | 0   | 0   | 0   | 0   | 0   | 0   | 0   | 0   | 0   | 0   | 0   | 0   | 0   | 0   | -1  | -1  | -1  | -1  | -1  | -1  | -1 |
| R      | 1   | 1   | 1   | 1   | 1   | 1   | 1   | 1   | 1   | 1   | 1   | 1   | 1   | 1   | -1  | -1  | -1  | -1  | -1  | -1  | -1  | i   | i   | i   | i   | i   | i   | i   | -i  | -i  | -i  | -i  | -i  | -i  | -i  | -1  | -1  | -1  | -1  | -1  | -1  | -1  |    |
| Landau | A1  | A1  | A1  | A1  | A1  | A1  | A1  | A1  | A1  | A1  | A1  | A1  | A1  | A1  | B1  | B1  | B1  | B1  | B1  | B1  | B1  | E   | E   | E   | E   | E   | E   | E   | E   | E   | E   | E   | E   | E   | E   | B2  | B2  | B2  | B2  | B2  | B2  | B2  |    |

[illegible]

$\mathbf{S} = \mathbf{3}, \mathbf{n}_{\text{occ.}} = \{\mathbf{2}, \mathbf{0}, \mathbf{2}\}$

| State  | 505 | 506 | 507 | 508 | 509 | 510 | 511 | 512 | 513 | 514 | 515 | 516 | 517 | 518 | 519 | 520 | 521 | 522 | 523 | 524 | 525 | 526      | 527      | 528      | 529      | 530      | 531      | 532      | 533        | 534        | 535        | 536        | 537        | 538        | 539        | 540 | 541 | 542 | 543 | 544 | 545 | 546 |    |    |
|--------|-----|-----|-----|-----|-----|-----|-----|-----|-----|-----|-----|-----|-----|-----|-----|-----|-----|-----|-----|-----|-----|----------|----------|----------|----------|----------|----------|----------|------------|------------|------------|------------|------------|------------|------------|-----|-----|-----|-----|-----|-----|-----|----|----|
| Sz     | 3   | 2   | 1   | 0   | -1  | -2  | -3  | 3   | 2   | 1   | 0   | -1  | -2  | -3  | 3   | 2   | 1   | 0   | -1  | -2  | -3  | 3        | 2        | 1        | 0        | -1       | -2       | -3       | 3          | 2          | 1          | 0          | -1         | -2         | -3         | 3   | 2   | 1   | 0   | -1  | -2  | -3  |    |    |
| Rx     | 1   | 1   | 1   | 1   | 1   | 1   | 1   | 1   | 1   | 1   | 1   | 1   | 1   | 1   | 1   | 1   | 1   | 1   | 1   | 1   | 1   | 0        | 0        | 0        | 0        | 0        | 0        | 0        | 0          | 0          | 0          | 0          | 0          | 0          | 0          | 0   | -1  | -1  | -1  | -1  | -1  | -1  | -1 |    |
| Ry     | 1   | 1   | 1   | 1   | 1   | 1   | 1   | 1   | 1   | 1   | 1   | 1   | 1   | 1   | 1   | 1   | 1   | 1   | 1   | 1   | 1   | 0        | 0        | 0        | 0        | 0        | 0        | 0        | 0          | 0          | 0          | 0          | 0          | 0          | 0          | 0   | 0   | -1  | -1  | -1  | -1  | -1  | -1 | -1 |
| R      | 1   | 1   | 1   | 1   | 1   | 1   | 1   | 1   | 1   | 1   | 1   | 1   | 1   | 1   | -1  | -1  | -1  | -1  | -1  | -1  | -1  | <i>i</i> | <i>i</i> | <i>i</i> | <i>i</i> | <i>i</i> | <i>i</i> | <i>i</i> | - <i>i</i> | - <i>i</i> | - <i>i</i> | - <i>i</i> | - <i>i</i> | - <i>i</i> | - <i>i</i> | -1  | -1  | -1  | -1  | -1  | -1  | -1  |    |    |
| Landau | A1  | A1  | A1  | A1  | A1  | A1  | A1  | A1  | A1  | A1  | A1  | A1  | A1  | A1  | B1  | B1  | B1  | B1  | B1  | B1  | B1  | E        | E        | E        | E        | E        | E        | E        | E          | E          | E          | E          | E          | E          | E          | B2  | B2  | B2  | B2  | B2  | B2  | B2  |    |    |





$$\mathbf{S} = \mathbf{2}, \mathbf{n}_{\text{occ.}} = \{4, 0, 0\}$$

[illegible]



$$\mathbf{S} = \mathbf{2}, \text{ n}_{\text{occ.}} = \{2, 2, 0\}$$

| State  | 746 | 747 | 748 | 749 | 750 | 751      | 752      | 753      | 754      | 755      | 756      | 757      | 758      | 759      | 760      | 761      | 762        | 763        | 764        | 765        | 766        | 767        | 768        | 769        | 770        | 771        | 772        | 773 | 774 | 775 |    |    |    |    |
|--------|-----|-----|-----|-----|-----|----------|----------|----------|----------|----------|----------|----------|----------|----------|----------|----------|------------|------------|------------|------------|------------|------------|------------|------------|------------|------------|------------|-----|-----|-----|----|----|----|----|
| Sz     | 2   | 1   | 0   | -1  | -2  | 2        | 1        | 0        | -1       | -2       | 2        | 1        | 0        | -1       | -2       | 2        | 1          | 0          | -1         | -2         | 2          | 1          | 0          | -1         | -2         | 2          | 1          | 0   | -1  | -2  |    |    |    |    |
| Rx     | 1   | 1   | 1   | 1   | 1   | 0        | 0        | 0        | 0        | 0        | 0        | 0        | 0        | 0        | 0        | 0        | 0          | 0          | 0          | 0          | 0          | 0          | 0          | 0          | 0          | 0          | 0          | -1  | -1  | -1  | -1 | -1 |    |    |
| Ry     | 1   | 1   | 1   | 1   | 1   | 0        | 0        | 0        | 0        | 0        | 0        | 0        | 0        | 0        | 0        | 0        | 0          | 0          | 0          | 0          | 0          | 0          | 0          | 0          | 0          | 0          | 0          | 0   | -1  | -1  | -1 | -1 | -1 |    |
| R      | -1  | -1  | -1  | -1  | -1  | <i>i</i> | <i>i</i> | <i>i</i> | <i>i</i> | <i>i</i> | <i>i</i> | <i>i</i> | <i>i</i> | <i>i</i> | <i>i</i> | <i>i</i> | - <i>i</i> | - <i>i</i> | - <i>i</i> | - <i>i</i> | - <i>i</i> | - <i>i</i> | - <i>i</i> | - <i>i</i> | - <i>i</i> | - <i>i</i> | - <i>i</i> | 1   | 1   | 1   | 1  | 1  |    |    |
| Landau | B1  | B1  | B1  | B1  | B1  | E        | E        | E        | E        | E        | E        | E        | E        | E        | E        | E        | E          | E          | E          | E          | E          | E          | E          | E          | E          | E          | E          | E   | E   | A2  | A2 | A2 | A2 | A2 |

$$\mathbf{S} = \mathbf{2}, \mathbf{n}_{\text{occ.}} = \{\mathbf{2}, \mathbf{1}, \mathbf{1}\}$$

[illegible]

$$\mathbf{S} = \mathbf{2}, \mathbf{n}_{\text{occ.}} = \{\mathbf{2}, \mathbf{0}, \mathbf{2}\}$$

| State  | 836 | 837 | 838 | 839 | 840 | 841      | 842      | 843      | 844      | 845      | 846      | 847      | 848      | 849      | 850      | 851      | 852        | 853        | 854        | 855        | 856        | 857        | 858        | 859        | 860        | 861        | 862 | 863 | 864 | 865 |    |
|--------|-----|-----|-----|-----|-----|----------|----------|----------|----------|----------|----------|----------|----------|----------|----------|----------|------------|------------|------------|------------|------------|------------|------------|------------|------------|------------|-----|-----|-----|-----|----|
| Sz     | 2   | 1   | 0   | -1  | -2  | 2        | 1        | 0        | -1       | -2       | 2        | 1        | 0        | -1       | -2       | 2        | 1          | 0          | -1         | -2         | 2          | 1          | 0          | -1         | -2         | 2          | 1   | 0   | -1  | -2  |    |
| Rx     | 1   | 1   | 1   | 1   | 1   | 0        | 0        | 0        | 0        | 0        | 0        | 0        | 0        | 0        | 0        | 0        | 0          | 0          | 0          | 0          | 0          | 0          | 0          | 0          | 0          | 0          | -1  | -1  | -1  | -1  |    |
| Ry     | 1   | 1   | 1   | 1   | 1   | 0        | 0        | 0        | 0        | 0        | 0        | 0        | 0        | 0        | 0        | 0        | 0          | 0          | 0          | 0          | 0          | 0          | 0          | 0          | 0          | 0          | -1  | -1  | -1  | -1  |    |
| R      | -1  | -1  | -1  | -1  | -1  | <i>i</i> | <i>i</i> | <i>i</i> | <i>i</i> | <i>i</i> | <i>i</i> | <i>i</i> | <i>i</i> | <i>i</i> | <i>i</i> | <i>i</i> | - <i>i</i> | - <i>i</i> | - <i>i</i> | - <i>i</i> | - <i>i</i> | - <i>i</i> | - <i>i</i> | - <i>i</i> | - <i>i</i> | - <i>i</i> | 1   | 1   | 1   | 1   |    |
| Landau | B1  | B1  | B1  | B1  | B1  | E        | E        | E        | E        | E        | E        | E        | E        | E        | E        | E        | E          | E          | E          | E          | E          | E          | E          | E          | E          | E          | A2  | A2  | A2  | A2  | A2 |





$$\mathbf{S} = \mathbf{3}/\mathbf{2}, \mathbf{n}_{\text{occ.}} = \{\mathbf{1}, \mathbf{3}, \mathbf{0}\}$$

| State  | 994           | 995           | 996            | 997            | 998           | 999           | 1000           | 1001           | 1002          | 1003          | 1004           | 1005           | 1006          | 1007          | 1008           | 1009           |
|--------|---------------|---------------|----------------|----------------|---------------|---------------|----------------|----------------|---------------|---------------|----------------|----------------|---------------|---------------|----------------|----------------|
| Sz     | $\frac{3}{2}$ | $\frac{1}{2}$ | $-\frac{1}{2}$ | $-\frac{3}{2}$ | $\frac{3}{2}$ | $\frac{1}{2}$ | $-\frac{1}{2}$ | $-\frac{3}{2}$ | $\frac{3}{2}$ | $\frac{1}{2}$ | $-\frac{1}{2}$ | $-\frac{3}{2}$ | $\frac{3}{2}$ | $\frac{1}{2}$ | $-\frac{1}{2}$ | $-\frac{3}{2}$ |
| Rx     | 1             | 1             | 1              | 1              | 1             | 1             | 1              | 1              | 0             | 0             | 0              | 0              | 0             | 0             | 0              | 0              |
| Ry     | 1             | 1             | 1              | 1              | 1             | 1             | 1              | 1              | 0             | 0             | 0              | 0              | 0             | 0             | 0              | 0              |
| R      | 1             | 1             | 1              | 1              | -1            | -1            | -1             | -1             | $i$           | $i$           | $i$            | $i$            | $-i$          | $-i$          | $-i$           | $-i$           |
| Landau | A1            | A1            | A1             | A1             | B1            | B1            | B1             | B1             | E             | E             | E              | E              | E             | E             | E              | E              |

$$\mathbf{S} = \mathbf{3}/\mathbf{2}, \mathbf{n}_{\text{occ.}} = \{\mathbf{1}, \mathbf{2}, \mathbf{1}\}$$

| State  | 1010          | 1011          | 1012           | 1013           | 1014          | 1015          | 1016           | 1017           | 1018          | 1019          | 1020           | 1021           | 1022          | 1023          | 1024           | 1025           | 1026          | 1027          | 1028           | 1029           | 1030          | 1031          | 1032           | 1033           | 1034          | 1035          | 1036           | 1037           | 1038          | 1039          | 1040           | 1041           | 1042          | 1043          | 1044           | 1045           | 1046          | 1047          | 1048           | 1049           | 1050          | 1051          | 1052           | 1053           | 1054 | 1055 | 1056 | 1057 |
|--------|---------------|---------------|----------------|----------------|---------------|---------------|----------------|----------------|---------------|---------------|----------------|----------------|---------------|---------------|----------------|----------------|---------------|---------------|----------------|----------------|---------------|---------------|----------------|----------------|---------------|---------------|----------------|----------------|---------------|---------------|----------------|----------------|---------------|---------------|----------------|----------------|---------------|---------------|----------------|----------------|---------------|---------------|----------------|----------------|------|------|------|------|
| Sz     | $\frac{3}{2}$ | $\frac{1}{2}$ | $-\frac{1}{2}$ | $-\frac{3}{2}$ | $\frac{3}{2}$ | $\frac{1}{2}$ | $-\frac{1}{2}$ | $-\frac{3}{2}$ | $\frac{3}{2}$ | $\frac{1}{2}$ | $-\frac{1}{2}$ | $-\frac{3}{2}$ | $\frac{3}{2}$ | $\frac{1}{2}$ | $-\frac{1}{2}$ | $-\frac{3}{2}$ | $\frac{3}{2}$ | $\frac{1}{2}$ | $-\frac{1}{2}$ | $-\frac{3}{2}$ | $\frac{3}{2}$ | $\frac{1}{2}$ | $-\frac{1}{2}$ | $-\frac{3}{2}$ | $\frac{3}{2}$ | $\frac{1}{2}$ | $-\frac{1}{2}$ | $-\frac{3}{2}$ | $\frac{3}{2}$ | $\frac{1}{2}$ | $-\frac{1}{2}$ | $-\frac{3}{2}$ | $\frac{3}{2}$ | $\frac{1}{2}$ | $-\frac{1}{2}$ | $-\frac{3}{2}$ | $\frac{3}{2}$ | $\frac{1}{2}$ | $-\frac{1}{2}$ | $-\frac{3}{2}$ | $\frac{3}{2}$ | $\frac{1}{2}$ | $-\frac{1}{2}$ | $-\frac{3}{2}$ |      |      |      |      |
| Rx     | 1             | 1             | 1              | 1              | 1             | 1             | 1              | 1              | 1             | 1             | 1              | 1              | 1             | 1             | 1              | 1              | 0             | 0             | 0              | 0              | 0             | 0             | 0              | 0              | 0             | 0             | 0              | 0              | 0             | 0             | 0              | 0              | 0             | 0             | 0              | 0              | 0             | 0             | -1             | -1             | -1            | -1            | -1             | -1             | -1   | -1   |      |      |
| Ry     | 1             | 1             | 1              | 1              | 1             | 1             | 1              | 1              | 1             | 1             | 1              | 1              | 1             | 1             | 1              | 1              | 0             | 0             | 0              | 0              | 0             | 0             | 0              | 0              | 0             | 0             | 0              | 0              | 0             | 0             | 0              | 0              | 0             | 0             | 0              | 0              | 0             | 0             | 0              | 0              | -1            | -1            | -1             | -1             | -1   | -1   | -1   | -1   |
| R      | 1             | 1             | 1              | 1              | 1             | 1             | 1              | 1              | -1            | -1            | -1             | -1             | -1            | -1            | -1             | -1             | $i$           | $i$           | $i$            | $i$            | $i$           | $i$           | $i$            | $i$            | $i$           | $i$           | $i$            | $i$            | $i$           | $-i$          | $-i$           | $-i$           | $-i$          | $-i$          | $-i$           | $-i$           | $-i$          | $-i$          | 1              | 1              | 1             | 1             | -1             | -1             | -1   | -1   |      |      |
| Landau | A1            | A1            | A1             | A1             | A1            | A1            | A1             | A1             | B1            | B1            | B1             | B1             | B1            | B1            | B1             | B1             | E             | E             | E              | E              | E             | E             | E              | E              | E             | E             | E              | E              | E             | E             | E              | E              | E             | E             | E              | E              | E             | E             | E              | A2             | A2            | A2            | A2             | B2             | B2   | B2   | B2   |      |

$$\mathbf{S} = \mathbf{3}/2, \mathbf{n}_{\text{occ.}} = \{\mathbf{1}, \mathbf{1}, \mathbf{2}\}$$

|        |               |               |                |                |               |               |                |                |               |               |                |                |               |               |                |                |               |               |                |                |               |               |                |                |               |               |                |                |               |               |                |                |               |               |                |                |               |               |                |                |               |               |                |                |               |               |                |                |    |    |
|--------|---------------|---------------|----------------|----------------|---------------|---------------|----------------|----------------|---------------|---------------|----------------|----------------|---------------|---------------|----------------|----------------|---------------|---------------|----------------|----------------|---------------|---------------|----------------|----------------|---------------|---------------|----------------|----------------|---------------|---------------|----------------|----------------|---------------|---------------|----------------|----------------|---------------|---------------|----------------|----------------|---------------|---------------|----------------|----------------|---------------|---------------|----------------|----------------|----|----|
| State  | 1058          | 1059          | 1060           | 1061           | 1062          | 1063          | 1064           | 1065           | 1066          | 1067          | 1068           | 1069           | 1070          | 1071          | 1072           | 1073           | 1074          | 1075          | 1076           | 1077           | 1078          | 1079          | 1080           | 1081           | 1082          | 1083          | 1084           | 1085           | 1086          | 1087          | 1088           | 1089           | 1090          | 1091          | 1092           | 1093           | 1094          | 1095          | 1096           | 1097           | 1098          | 1099          | 1100           | 1101           | 1102          | 1103          | 1104           | 1105           |    |    |
| Sz     | $\frac{3}{2}$ | $\frac{1}{2}$ | $-\frac{1}{2}$ | $-\frac{3}{2}$ | $\frac{3}{2}$ | $\frac{1}{2}$ | $-\frac{1}{2}$ | $-\frac{3}{2}$ | $\frac{3}{2}$ | $\frac{1}{2}$ | $-\frac{1}{2}$ | $-\frac{3}{2}$ | $\frac{3}{2}$ | $\frac{1}{2}$ | $-\frac{1}{2}$ | $-\frac{3}{2}$ | $\frac{3}{2}$ | $\frac{1}{2}$ | $-\frac{1}{2}$ | $-\frac{3}{2}$ | $\frac{3}{2}$ | $\frac{1}{2}$ | $-\frac{1}{2}$ | $-\frac{3}{2}$ | $\frac{3}{2}$ | $\frac{1}{2}$ | $-\frac{1}{2}$ | $-\frac{3}{2}$ | $\frac{3}{2}$ | $\frac{1}{2}$ | $-\frac{1}{2}$ | $-\frac{3}{2}$ | $\frac{3}{2}$ | $\frac{1}{2}$ | $-\frac{1}{2}$ | $-\frac{3}{2}$ | $\frac{3}{2}$ | $\frac{1}{2}$ | $-\frac{1}{2}$ | $-\frac{3}{2}$ | $\frac{3}{2}$ | $\frac{1}{2}$ | $-\frac{1}{2}$ | $-\frac{3}{2}$ | $\frac{3}{2}$ | $\frac{1}{2}$ | $-\frac{1}{2}$ | $-\frac{3}{2}$ |    |    |
| Rx     | 1             | 1             | 1              | 1              | 1             | 1             | 1              | 1              | 1             | 1             | 1              | 1              | 1             | 1             | 1              | 1              | 0             | 0             | 0              | 0              | 0             | 0             | 0              | 0              | 0             | 0             | 0              | 0              | 0             | 0             | 0              | 0              | 0             | 0             | 0              | 0              | 0             | 0             | 0              | -1             | -1            | -1            | -1             | -1             | -1            | -1            | -1             | -1             | -1 |    |
| Ry     | 1             | 1             | 1              | 1              | 1             | 1             | 1              | 1              | 1             | 1             | 1              | 1              | 1             | 1             | 1              | 1              | 0             | 0             | 0              | 0              | 0             | 0             | 0              | 0              | 0             | 0             | 0              | 0              | 0             | 0             | 0              | 0              | 0             | 0             | 0              | 0              | 0             | 0             | 0              | 0              | -1            | -1            | -1             | -1             | -1            | -1            | -1             | -1             | -1 | -1 |
| R      | 1             | 1             | 1              | 1              | 1             | 1             | 1              | 1              | -1            | -1            | -1             | -1             | -1            | -1            | -1             | -1             | $i$           | $i$           | $i$            | $i$            | $i$           | $i$           | $i$            | $i$            | $i$           | $i$           | $i$            | $i$            | $i$           | $i$           | $-i$           | $-i$           | $-i$          | $-i$          | $-i$           | $-i$           | $-i$          | $-i$          | $-i$           | $-i$           | 1             | 1             | 1              | 1              | -1            | -1            | -1             | -1             |    |    |
| Landau | A1            | A1            | A1             | A1             | A1            | A1            | A1             | A1             | B1            | B1            | B1             | B1             | B1            | B1            | B1             | B1             | E             | E             | E              | E              | E             | E             | E              | E              | E             | E             | E              | E              | E             | E             | E              | E              | E             | E             | E              | E              | E             | E             | E              | E              | A2            | A2            | A2             | A2             | B2            | B2            | B2             | B2             |    |    |



$$\mathbf{S} = \mathbf{3}/\mathbf{2}, \mathbf{n}_{\text{occ.}} = \{\mathbf{1}, \mathbf{0}, \mathbf{3}\}$$

| State  | 1106          | 1107          | 1108           | 1109           | 1110          | 1111          | 1112           | 1113           | 1114          | 1115          | 1116           | 1117           | 1118          | 1119          | 1120           | 1121           |
|--------|---------------|---------------|----------------|----------------|---------------|---------------|----------------|----------------|---------------|---------------|----------------|----------------|---------------|---------------|----------------|----------------|
| Sz     | $\frac{3}{2}$ | $\frac{1}{2}$ | $-\frac{1}{2}$ | $-\frac{3}{2}$ | $\frac{3}{2}$ | $\frac{1}{2}$ | $-\frac{1}{2}$ | $-\frac{3}{2}$ | $\frac{3}{2}$ | $\frac{1}{2}$ | $-\frac{1}{2}$ | $-\frac{3}{2}$ | $\frac{3}{2}$ | $\frac{1}{2}$ | $-\frac{1}{2}$ | $-\frac{3}{2}$ |
| Rx     | 1             | 1             | 1              | 1              | 1             | 1             | 1              | 1              | 0             | 0             | 0              | 0              | 0             | 0             | 0              | 0              |
| Ry     | 1             | 1             | 1              | 1              | 1             | 1             | 1              | 1              | 0             | 0             | 0              | 0              | 0             | 0             | 0              | 0              |
| R      | 1             | 1             | 1              | 1              | -1            | -1            | -1             | -1             | $i$           | $i$           | $i$            | $i$            | $-i$          | $-i$          | $-i$           | $-i$           |
| Landau | A1            | A1            | A1             | A1             | B1            | B1            | B1             | B1             | E             | E             | E              | E              | E             | E             | E              | E              |

$$\mathbf{S} = 1, \mathbf{n}_{\text{occ.}} = \{4, 0, 0\}$$

| State  | 1122 | 1123 | 1124 | 1125 | 1126 | 1127 | 1128 | 1129 | 1130 | 1131 | 1132 | 1133 | 1134 | 1135 | 1136 | 1137 | 1138 | 1139 | 1140 | 1141 | 1142 | 1143 | 1144 | 1145 | 1146 | 1147 | 1148 |
|--------|------|------|------|------|------|------|------|------|------|------|------|------|------|------|------|------|------|------|------|------|------|------|------|------|------|------|------|
| Sz     | 1    | 0    | -1   | 1    | 0    | -1   | 1    | 0    | -1   | 1    | 0    | -1   | 1    | 0    | -1   | 1    | 0    | -1   | 1    | 0    | -1   | 1    | 0    | -1   | 1    | 0    | -1   |
| Rx     | 1    | 1    | 1    | 1    | 1    | 1    | 0    | 0    | 0    | 0    | 0    | 0    | 0    | 0    | 0    | 0    | 0    | 0    | 0    | 0    | 0    | 0    | 0    | 0    | -1   | -1   | -1   |
| Ry     | 1    | 1    | 1    | 1    | 1    | 1    | 0    | 0    | 0    | 0    | 0    | 0    | 0    | 0    | 0    | 0    | 0    | 0    | 0    | 0    | 0    | 0    | 0    | 0    | -1   | -1   | -1   |
| R      | -1   | -1   | -1   | -1   | -1   | -1   | $i$  | $i$  | $i$  | $i$  | $i$  | $i$  | $i$  | $i$  | $i$  | $i$  | $-i$ | $-i$ | $-i$ | $-i$ | $-i$ | $-i$ | $-i$ | $-i$ | 1    | 1    | 1    |
| Landau | B1   | B1   | B1   | B1   | B1   | B1   | E    | E    | E    | E    | E    | E    | E    | E    | E    | E    | E    | E    | E    | E    | E    | E    | E    | E    | A2   | A2   | A2   |

$$S = 1, \text{ n}_{\text{occ.}} = \{2, 2, 0\}$$

$$\left( \begin{array}{c} \text{State} \\ \text{Sz} \\ \text{Rx} \\ \text{Ry} \\ \text{R} \\ \text{Landau} \end{array} \begin{array}{cccccccccccccccccccccccc} 1149 & 1150 & 1151 & 1152 & 1153 & 1154 & 1155 & 1156 & 1157 & 1158 & 1159 & 1160 & 1161 & 1162 & 1163 & 1164 & 1165 & 1166 \end{array} \right)$$

$$\mathbf{S} = \mathbf{1}, \mathbf{n}_{\text{occ.}} = \{\mathbf{2}, \mathbf{1}, \mathbf{1}\}$$

|        |      |      |      |      |      |      |      |      |      |      |      |      |      |      |      |      |      |      |      |      |      |      |      |      |      |      |      |      |      |      |      |      |      |      |      |      |    |
|--------|------|------|------|------|------|------|------|------|------|------|------|------|------|------|------|------|------|------|------|------|------|------|------|------|------|------|------|------|------|------|------|------|------|------|------|------|----|
| State  | 1167 | 1168 | 1169 | 1170 | 1171 | 1172 | 1173 | 1174 | 1175 | 1176 | 1177 | 1178 | 1179 | 1180 | 1181 | 1182 | 1183 | 1184 | 1185 | 1186 | 1187 | 1188 | 1189 | 1190 | 1191 | 1192 | 1193 | 1194 | 1195 | 1196 | 1197 | 1198 | 1199 | 1200 | 1201 | 1202 |    |
| Sz     | 1    | 0    | -1   | 1    | 0    | -1   | 1    | 0    | -1   | 1    | 0    | -1   | 1    | 0    | -1   | 1    | 0    | -1   | 1    | 0    | -1   | 1    | 0    | -1   | 1    | 0    | -1   | 1    | 0    | -1   | 1    | 0    | -1   | 1    | 0    | -1   |    |
| Rx     | 1    | 1    | 1    | 1    | 1    | 1    | 1    | 1    | 1    | 1    | 1    | 1    | 0    | 0    | 0    | 0    | 0    | 0    | 0    | 0    | 0    | 0    | 0    | 0    | 0    | 0    | 0    | 0    | 0    | 0    | 0    | -1   | -1   | -1   | -1   | -1   |    |
| Ry     | 1    | 1    | 1    | 1    | 1    | 1    | 1    | 1    | 1    | 1    | 1    | 1    | 0    | 0    | 0    | 0    | 0    | 0    | 0    | 0    | 0    | 0    | 0    | 0    | 0    | 0    | 0    | 0    | 0    | 0    | 0    | -1   | -1   | -1   | -1   | -1   |    |
| R      | 1    | 1    | 1    | 1    | 1    | 1    | 1    | -1   | -1   | -1   | -1   | -1   | $i$  | $i$  | $i$  | $i$  | $i$  | $i$  | $i$  | $i$  | $i$  | $i$  | $i$  | $-i$ | $-i$ | $-i$ | $-i$ | $-i$ | $-i$ | $-i$ | $-i$ | 1    | 1    | 1    | -1   | -1   | -1 |
| Landau | A1   | A1   | A1   | A1   | A1   | A1   | B1   | B1   | B1   | B1   | B1   | B1   | E    | E    | E    | E    | E    | E    | E    | E    | E    | E    | E    | E    | E    | E    | E    | E    | E    | E    | E    | A2   | A2   | A2   | B2   | B2   | B2 |

$$S = 1, \text{ n}_{\text{occ.}} = \{2, 0, 2\}$$

$$\left( \begin{array}{c|cccccccccccccccccccc} \text{State} & 1203 & 1204 & 1205 & 1206 & 1207 & 1208 & 1209 & 1210 & 1211 & 1212 & 1213 & 1214 & 1215 & 1216 & 1217 & 1218 & 1219 & 1220 \\ \hline \text{Sz} & 1 & 0 & -1 & 1 & 0 & -1 & 1 & 0 & -1 & 1 & 0 & -1 & 1 & 0 & -1 & 1 & 0 & -1 \\ \text{Rx} & 1 & 1 & 1 & 1 & 1 & 1 & 1 & 1 & 1 & 0 & 0 & 0 & 0 & 0 & 0 & -1 & -1 & -1 \\ \text{Ry} & 1 & 1 & 1 & 1 & 1 & 1 & 1 & 1 & 1 & 0 & 0 & 0 & 0 & 0 & 0 & -1 & -1 & -1 \\ \text{R} & 1 & 1 & 1 & 1 & 1 & 1 & -1 & -1 & -1 & i & i & i & -i & -i & -i & -1 & -1 & -1 \\ \text{Landau} & \text{A1} & \text{A1} & \text{A1} & \text{A1} & \text{A1} & \text{A1} & \text{B1} & \text{B1} & \text{B1} & \text{E} & \text{E} & \text{E} & \text{E} & \text{E} & \text{E} & \text{B2} & \text{B2} & \text{B2} \end{array} \right)$$

$$\mathbf{S} = \mathbf{1}/2, \mathbf{n}_{\text{occ.}} = \{\mathbf{3}, \mathbf{1}, \mathbf{0}\}$$

| State  | 1221          | 1222           | 1223          | 1224           | 1225          | 1226           | 1227          | 1228           | 1229          | 1230           | 1231          | 1232           | 1233          | 1234           | 1235          | 1236           |
|--------|---------------|----------------|---------------|----------------|---------------|----------------|---------------|----------------|---------------|----------------|---------------|----------------|---------------|----------------|---------------|----------------|
| Sz     | $\frac{1}{2}$ | $-\frac{1}{2}$ | $\frac{1}{2}$ | $-\frac{1}{2}$ | $\frac{1}{2}$ | $-\frac{1}{2}$ | $\frac{1}{2}$ | $-\frac{1}{2}$ | $\frac{1}{2}$ | $-\frac{1}{2}$ | $\frac{1}{2}$ | $-\frac{1}{2}$ | $\frac{1}{2}$ | $-\frac{1}{2}$ | $\frac{1}{2}$ | $-\frac{1}{2}$ |
| Rx     | 1             | 1              | 1             | 1              | 0             | 0              | 0             | 0              | 0             | 0              | 0             | 0              | -1            | -1             | -1            | -1             |
| Ry     | 1             | 1              | 1             | 1              | 0             | 0              | 0             | 0              | 0             | 0              | 0             | 0              | -1            | -1             | -1            | -1             |
| R      | 1             | 1              | -1            | -1             | $i$           | $i$            | $i$           | $i$            | $-i$          | $-i$           | $-i$          | $-i$           | 1             | 1              | -1            | -1             |
| Landau | A1            | A1             | B1            | B1             | E             | E              | E             | E              | E             | E              | E             | E              | A2            | A2             | B2            | B2             |



$$\mathbf{S} = \mathbf{0}, \mathbf{n}_{\text{occ.}} = \{4, \mathbf{0}, \mathbf{0}\}$$

| State  | 1253 | 1254 | 1255 | 1256 |
|--------|------|------|------|------|
| Sz     | 0    | 0    | 0    | 0    |
| Rx     | 1    | 1    | -1   | -1   |
| Ry     | 1    | 1    | -1   | -1   |
| R      | 1    | 1    | -1   | -1   |
| Landau | A1   | A1   | B2   | B2   |



$$\mathbf{S} = \mathbf{0}, \mathbf{n}_{\text{occ.}} = \{\mathbf{2}, \mathbf{2}, \mathbf{0}\}$$

| State  | 1257 | 1258 | 1259 | 1260 | 1261 | 1262 |
|--------|------|------|------|------|------|------|
| Sz     | 0    | 0    | 0    | 0    | 0    | 0    |
| Rx     | 1    | 0    | 0    | 0    | 0    | -1   |
| Ry     | 1    | 0    | 0    | 0    | 0    | -1   |
| R      | -1   | $i$  | $i$  | $-i$ | $-i$ | 1    |
| Landau | B1   | E    | E    | E    | E    | A2   |

$$\mathbf{S} = \mathbf{0}, \mathbf{n}_{\text{occ.}} = \{\mathbf{2}, \mathbf{1}, \mathbf{1}\}$$

| State  | 1263 | 1264 | 1265 | 1266 | 1267 | 1268 | 1269 | 1270 | 1271 | 1272 | 1273 | 1274 |
|--------|------|------|------|------|------|------|------|------|------|------|------|------|
| Sz     | 0    | 0    | 0    | 0    | 0    | 0    | 0    | 0    | 0    | 0    | 0    | 0    |
| Rx     | 1    | 1    | 0    | 0    | 0    | 0    | 0    | 0    | 0    | -1   | -1   | -1   |
| Ry     | 1    | 1    | 0    | 0    | 0    | 0    | 0    | 0    | 0    | -1   | -1   | -1   |
| R      | 1    | -1   | $i$  | $i$  | $i$  | $-i$ | $-i$ | $-i$ | 1    | 1    | -1   | -1   |
| Landau | A1   | B1   | E    | E    | E    | E    | E    | E    | A2   | A2   | B2   | B2   |

$$\mathbf{S} = \mathbf{0}, \mathbf{n}_{\text{occ.}} = \{\mathbf{2}, \mathbf{0}, \mathbf{2}\}$$

| State  | 1275 | 1276 | 1277 | 1278 | 1279 | 1280 |
|--------|------|------|------|------|------|------|
| Sz     | 0    | 0    | 0    | 0    | 0    | 0    |
| Rx     | 1    | 0    | 0    | 0    | 0    | -1   |
| Ry     | 1    | 0    | 0    | 0    | 0    | -1   |
| R      | -1   | $i$  | $i$  | $-i$ | $-i$ | 1    |
| Landau | B1   | E    | E    | E    | E    | A2   |

$$\mathbf{S} = \mathbf{0}, \text{ n}_{\text{occ.}} = \{0, 4, 0\}$$

$$\left( \begin{array}{cc} \text{State} & 1281 \\ \text{Sz} & 0 \\ \text{Rx} & 1 \\ \text{Ry} & 1 \\ \text{R} & 1 \\ \text{Landau} & \text{A1} \end{array} \right)$$

$$\mathbf{S} = \mathbf{0}, \text{ n}_{\text{occ.}} = \{\mathbf{0}, \mathbf{3}, \mathbf{1}\}$$

$$\left( \begin{array}{ccccc} \text{State} & 1282 & 1283 & 1284 & 1285 \\ \text{Sz} & 0 & 0 & 0 & 0 \\ \text{Rx} & 1 & 1 & 0 & 0 \\ \text{Ry} & 1 & 1 & 0 & 0 \\ \text{R} & 1 & -1 & i & -i \\ \text{Landau} & \text{A1} & \text{B1} & \text{E} & \text{E} \end{array} \right)$$

$$\mathbf{S} = \mathbf{0}, \mathbf{n}_{\text{occ.}} = \{\mathbf{0}, \mathbf{2}, \mathbf{2}\}$$

| State  | 1286 | 1287 | 1288 | 1289 | 1290 | 1291 |
|--------|------|------|------|------|------|------|
| Sz     | 0    | 0    | 0    | 0    | 0    | 0    |
| Rx     | 1    | 1    | 1    | 0    | 0    | -1   |
| Ry     | 1    | 1    | 1    | 0    | 0    | -1   |
| R      | 1    | 1    | -1   | $i$  | $-i$ | -1   |
| Landau | A1   | A1   | B1   | E    | E    | B2   |

$$\mathbf{S} = \mathbf{0}, \text{ n}_{\text{occ.}} = \{0, 1, 3\}$$

| State  | 1292 | 1293 | 1294 | 1295 |
|--------|------|------|------|------|
| Sz     | 0    | 0    | 0    | 0    |
| Rx     | 1    | 1    | 0    | 0    |
| Ry     | 1    | 1    | 0    | 0    |
| R      | 1    | -1   | $i$  | $-i$ |
| Landau | A1   | B1   | E    | E    |

$$\mathbf{S} = \mathbf{0}, \text{ n}_{\text{occ.}} = \{0, 0, 4\}$$

$$\left( \begin{array}{cc} \text{State} & 1296 \\ \text{Sz} & 0 \\ \text{Rx} & 1 \\ \text{Ry} & 1 \\ \text{R} & 1 \\ \text{Landau} & \text{A1} \end{array} \right)$$





[illegible]

$$\begin{aligned}
 & \mathbf{S} = 4, \quad \mathbf{n}_{\text{occ.}} = \{\mathbf{2}, \mathbf{2}\} \\
 & \left( \begin{array}{cc}
 \text{State} & 46 \quad 47 \quad 48 \quad 49 \quad 50 \quad 51 \quad 52 \quad 53 \quad 54 \quad 55 \quad 56 \quad 57 \quad 58 \quad 59 \quad 60 \quad 61 \quad 62 \quad 63 \quad 64 \quad 65 \quad 66 \quad 67 \quad 68 \quad 69 \quad 70 \quad 71 \quad 72 \quad 73 \quad 74 \quad 75 \quad 76 \quad 77 \quad 78 \quad 79 \quad 80 \quad 81 \quad 82 \quad 83 \quad 84 \quad 85 \quad 86 \quad 87 \quad 88 \quad 89 \quad 90 \quad 91 \quad 92 \quad 93 \quad 94 \quad 95 \quad 96 \quad 97 \quad 98 \quad 99 \\
 \text{Sz} & 4 \quad 3 \quad 2 \quad 1 \quad 0 \quad -1 \quad -2 \quad -3 \quad -4 \quad 4 \quad 3 \quad 2 \quad 1 \quad 0 \quad -1 \quad -2 \quad -3 \quad -4 \quad 4 \quad 3 \quad 2 \quad 1 \quad 0 \quad -1 \quad -2 \quad -3 \quad -4 \quad 4 \quad 3 \quad 2 \quad 1 \quad 0 \quad -1 \quad -2 \quad -3 \quad -4 \quad 4 \quad 3 \quad 2 \quad 1 \quad 0 \quad -1 \quad -2 \quad -3 \quad -4 \quad 4 \quad 3 \quad 2 \quad 1 \quad 0 \quad -1 \quad -2 \quad -3 \quad -4 \\
 \text{Rx} & 1 \quad 1 \quad 1 \quad 1 \quad 1 \quad 1 \quad 1 \quad 1 \quad 1 \quad 1 \quad 1 \quad 1 \quad 1 \quad 1 \quad 1 \quad 1 \quad 1 \quad 1 \quad 1 \quad 1 \quad 1 \quad 1 \quad 1 \quad 1 \quad 1 \quad 1 \quad 1 \quad 1 \quad 0 \quad 0 \quad 0 \quad 0 \quad 0 \quad 0 \quad 0 \quad 0 \quad 0 \quad 0 \quad 0 \quad 0 \quad 0 \quad 0 \quad 0 \quad 0 \quad 0 \quad 0 \quad -1 \quad -1 \quad -1 \quad -1 \quad -1 \quad -1 \quad -1 \quad -1 \quad -1 \\
 \text{Ry} & 1 \quad 1 \quad 1 \quad 1 \quad 1 \quad 1 \quad 1 \quad 1 \quad 1 \quad 1 \quad 1 \quad 1 \quad 1 \quad 1 \quad 1 \quad 1 \quad 1 \quad 1 \quad 1 \quad 1 \quad 1 \quad 1 \quad 1 \quad 1 \quad 1 \quad 1 \quad 1 \quad 1 \quad 0 \quad 0 \quad 0 \quad 0 \quad 0 \quad 0 \quad 0 \quad 0 \quad 0 \quad 0 \quad 0 \quad 0 \quad 0 \quad 0 \quad 0 \quad 0 \quad 0 \quad 0 \quad 0 \quad -1 \quad -1 \quad -1 \quad -1 \quad -1 \quad -1 \quad -1 \quad -1 \quad -1 \\
 \text{R} & 1 \quad 1 \quad 1 \quad 1 \quad 1 \quad 1 \quad 1 \quad 1 \quad 1 \quad 1 \quad 1 \quad 1 \quad 1 \quad 1 \quad 1 \quad 1 \quad 1 \quad 1 \quad 1 \quad 1 \quad -1 \quad -1 \quad -1 \quad -1 \quad -1 \quad -1 \quad -1 \quad -1 \quad -1 \quad i \quad i \quad i \quad i \quad i \quad i \quad i \quad i \quad i \quad -i \quad -i \quad -i \quad -i \quad -i \quad -i \quad -i \quad -i \quad -1 \quad -1 \quad -1 \quad -1 \quad -1 \quad -1 \quad -1 \quad -1 \quad -1 \\
 \text{Landau} & \text{A1} \quad \text{A1} \quad \text{A1} \quad \text{A1} \quad \text{A1} \quad \text{A1} \quad \text{A1} \quad \text{A1} \quad \text{A1} \quad \text{A1} \quad \text{A1} \quad \text{A1} \quad \text{A1} \quad \text{A1} \quad \text{A1} \quad \text{A1} \quad \text{A1} \quad \text{A1} \quad \text{A1} \quad \text{B1} \quad \text{B1} \quad \text{B1} \quad \text{B1} \quad \text{B1} \quad \text{B1} \quad \text{B1} \quad \text{B1} \quad \text{B1} \quad \text{B1} \quad \text{B1} \quad \text{B1} \quad \text{E} \quad \text{E} \quad \text{E} \quad \text{E} \quad \text{E} \quad \text{E} \quad \text{E} \quad \text{E} \quad \text{E} \quad \text{E} \quad \text{E} \quad \text{E} \quad \text{E} \quad \text{E} \quad \text{E} \quad \text{E} \quad \text{E} \quad \text{E} \quad \text{E} \quad \text{E} \quad \text{B2} \quad \text{B2} \quad \text{B2} \quad \text{B2} \quad \text{B2} \quad \text{B2} \quad \text{B2} \quad \text{B2} \quad \text{B2} \quad \text{B2} \quad \text{B2} \quad \text{B2} \quad \text{B2}
 \end{array} \right)
 \end{aligned}$$

[illegible]







$$S = 3 \quad n = 12 \quad \lambda = 2$$



$$\mathbf{S} = \mathbf{3}, \mathbf{n}_{occ} = \{1, 3\}$$

[illegible]

$$S = 3, \text{ n}_{\text{occ.}} = \{0, 4\}$$

$$\left( \begin{array}{c} \text{State} \\ \text{Sz} \\ \text{Rx} \\ \text{Ry} \\ \text{R} \\ \text{Landau} \end{array} \begin{array}{cccccccccccccccccccccccc} 460 & 461 & 462 & 463 & 464 & 465 & 466 & 467 & 468 & 469 & 470 & 471 & 472 & 473 & 474 & 475 & 476 & 477 & 478 & 479 & 480 \end{array} \right)$$

$\mathbf{S} = \mathbf{2}, \mathbf{n_{occ.}} = \{4, \mathbf{0}\}$

| State  | 481 | 482 | 483 | 484 | 485 | 486 | 487 | 488 | 489 | 490 | 491 | 492 | 493 | 494 | 495 | 496 | 497 | 498 | 499 | 500 | 501 | 502 | 503 | 504 | 505 | 506 | 507 | 508 | 509 | 510 |
|--------|-----|-----|-----|-----|-----|-----|-----|-----|-----|-----|-----|-----|-----|-----|-----|-----|-----|-----|-----|-----|-----|-----|-----|-----|-----|-----|-----|-----|-----|-----|
| Sz     | 2   | 1   | 0   | -1  | -2  | 2   | 1   | 0   | -1  | -2  | 2   | 1   | 0   | -1  | -2  | 2   | 1   | 0   | -1  | -2  | 2   | 1   | 0   | -1  | -2  | 2   | 1   | 0   | -1  | -2  |
| Rx     | 1   | 1   | 1   | 1   | 1   | 1   | 1   | 1   | 1   | 1   | 1   | 1   | 1   | 1   | 1   | 0   | 0   | 0   | 0   | 0   | 0   | 0   | 0   | 0   | 0   | 0   | -1  | -1  | -1  | -1  |
| Ry     | 1   | 1   | 1   | 1   | 1   | 1   | 1   | 1   | 1   | 1   | 1   | 1   | 1   | 1   | 1   | 0   | 0   | 0   | 0   | 0   | 0   | 0   | 0   | 0   | 0   | 0   | -1  | -1  | -1  | -1  |
| R      | 1   | 1   | 1   | 1   | 1   | 1   | 1   | 1   | 1   | 1   | 1   | -1  | -1  | -1  | -1  | -1  | i   | i   | i   | i   | i   | -i  | -i  | -i  | -i  | -i  | -1  | -1  | -1  | -1  |
| Landau | A1  | A1  | A1  | A1  | A1  | A1  | A1  | A1  | A1  | A1  | B1  | B1  | B1  | B1  | B1  | E   | E   | E   | E   | E   | E   | E   | E   | E   | E   | E   | B2  | B2  | B2  | B2  |

$$S = 2 \quad n = 13 \quad 1$$



$$S = 2 \quad n = 13$$

$\mathbf{S} = \mathbf{2}, \mathbf{n}_{occ.} = \{0, 4\}$

| State  | 931 | 932 | 933 | 934 | 935 | 936 | 937 | 938 | 939 | 940 | 941 | 942 | 943 | 944 | 945 | 946 | 947 | 948 | 949 | 950 | 951 | 952  | 953  | 954  | 955  | 956  | 957 | 958 | 959 | 960 |
|--------|-----|-----|-----|-----|-----|-----|-----|-----|-----|-----|-----|-----|-----|-----|-----|-----|-----|-----|-----|-----|-----|------|------|------|------|------|-----|-----|-----|-----|
| Sz     | 2   | 1   | 0   | -1  | -2  | 2   | 1   | 0   | -1  | -2  | 2   | 1   | 0   | -1  | -2  | 2   | 1   | 0   | -1  | -2  | 2   | 1    | 0    | -1   | -2   | 2    | 1   | 0   | -1  | -2  |
| Rx     | 1   | 1   | 1   | 1   | 1   | 1   | 1   | 1   | 1   | 1   | 1   | 1   | 1   | 1   | 1   | 0   | 0   | 0   | 0   | 0   | 0   | 0    | 0    | 0    | 0    | -1   | -1  | -1  | -1  | -1  |
| Ry     | 1   | 1   | 1   | 1   | 1   | 1   | 1   | 1   | 1   | 1   | 1   | 1   | 1   | 1   | 1   | 0   | 0   | 0   | 0   | 0   | 0   | 0    | 0    | 0    | 0    | 0    | -1  | -1  | -1  | -1  |
| R      | 1   | 1   | 1   | 1   | 1   | 1   | 1   | 1   | 1   | 1   | 1   | -1  | -1  | -1  | -1  | -1  | $i$ | $i$ | $i$ | $i$ | $i$ | $-i$ | $-i$ | $-i$ | $-i$ | $-i$ | -1  | -1  | -1  | -1  |
| Landau | A1  | A1  | A1  | A1  | A1  | A1  | A1  | A1  | A1  | A1  | B1  | B1  | B1  | B1  | B1  | E   | E   | E   | E   | E   | E   | E    | E    | E    | E    | B2   | B2  | B2  | B2  | B2  |

$$S = 1, \text{ n}_{\text{occ.}} = \{4, 0\}$$

$$\left( \begin{array}{c|cccccccccccccccccccc} \text{State} & 961 & 962 & 963 & 964 & 965 & 966 & 967 & 968 & 969 & 970 & 971 & 972 & 973 & 974 & 975 & 976 & 977 & 978 \\ \hline \text{Sz} & 1 & 0 & -1 & 1 & 0 & -1 & 1 & 0 & -1 & 1 & 0 & -1 & 1 & 0 & -1 & 1 & 0 & -1 \\ \text{Rx} & 1 & 1 & 1 & 0 & 0 & 0 & 0 & 0 & 0 & 0 & 0 & 0 & 0 & 0 & 0 & -1 & -1 & -1 \\ \text{Ry} & 1 & 1 & 1 & 0 & 0 & 0 & 0 & 0 & 0 & 0 & 0 & 0 & 0 & 0 & 0 & -1 & -1 & -1 \\ \text{R} & -1 & -1 & -1 & i & i & i & i & i & i & i & -i & -i & -i & -i & -i & 1 & 1 & 1 \\ \text{Landau} & \text{B1} & \text{B1} & \text{B1} & \text{E} & \text{E} & \text{E} & \text{E} & \text{E} & \text{E} & \text{E} & \text{E} & \text{E} & \text{E} & \text{E} & \text{E} & \text{A2} & \text{A2} & \text{A2} \end{array} \right)$$



$$\mathbf{S} = \mathbf{1}, \mathbf{n}_{\text{occ}} = \{\mathbf{3}, \mathbf{1}\}$$

[illegible]

$$S = 1 - \rho = \frac{1}{2} \quad \text{for } \lambda = 1$$

$$S = 1, n_{\text{acc}} = \{1, 3\}$$

[illegible]

$$S = 1, \text{ n}_{\text{occ.}} = \{0, 4\}$$

[illegible]

$$\mathbf{S} = \mathbf{0}, \text{ n}_{\text{occ.}} = \{4, \mathbf{0}\}$$

$$\left( \begin{array}{cccc} \text{State} & 1249 & 1250 & 1251 \\ \text{Sz} & 0 & 0 & 0 \\ \text{Rx} & 1 & 1 & -1 \\ \text{Ry} & 1 & 1 & -1 \\ \text{R} & 1 & 1 & -1 \\ \text{Landau} & \text{A1} & \text{A1} & \text{B2} \end{array} \right)$$

$$\mathbf{S} = \mathbf{0}, \mathbf{n}_{\text{occ.}} = \{\mathbf{3}, \mathbf{1}\}$$

| State  | 1252 | 1253 | 1254 | 1255 | 1256 | 1257 | 1258 | 1259 | 1260 | 1261 | 1262 | 1263 |
|--------|------|------|------|------|------|------|------|------|------|------|------|------|
| Sz     | 0    | 0    | 0    | 0    | 0    | 0    | 0    | 0    | 0    | 0    | 0    | 0    |
| Rx     | 1    | 1    | 1    | 1    | 0    | 0    | 0    | 0    | 0    | 0    | -1   | -1   |
| Ry     | 1    | 1    | 1    | 1    | 0    | 0    | 0    | 0    | 0    | 0    | -1   | -1   |
| R      | 1    | 1    | -1   | -1   | $i$  | $i$  | $i$  | $-i$ | $-i$ | $-i$ | 1    | -1   |
| Landau | A1   | A1   | B1   | B1   | E    | E    | E    | E    | E    | E    | A2   | B2   |

$$\mathbf{S} = \mathbf{0}, \mathbf{n}_{\text{occ.}} = \{\mathbf{2}, \mathbf{2}\}$$

| State  | 1264 | 1265 | 1266 | 1267 | 1268 | 1269 | 1270 | 1271 | 1272 | 1273 | 1274 | 1275 | 1276 | 1277 | 1278 | 1279 | 1280 | 1281 |
|--------|------|------|------|------|------|------|------|------|------|------|------|------|------|------|------|------|------|------|
| Sz     | 0    | 0    | 0    | 0    | 0    | 0    | 0    | 0    | 0    | 0    | 0    | 0    | 0    | 0    | 0    | 0    | 0    | 0    |
| Rx     | 1    | 1    | 1    | 1    | 1    | 1    | 1    | 1    | 0    | 0    | 0    | 0    | 0    | 0    | -1   | -1   | -1   | -1   |
| Ry     | 1    | 1    | 1    | 1    | 1    | 1    | 1    | 1    | 0    | 0    | 0    | 0    | 0    | 0    | -1   | -1   | -1   | -1   |
| R      | 1    | 1    | 1    | 1    | 1    | 1    | -1   | -1   | $i$  | $i$  | $i$  | $-i$ | $-i$ | $-i$ | 1    | -1   | -1   | -1   |
| Landau | A1   | A1   | A1   | A1   | A1   | B1   | B1   | E    | E    | E    | E    | E    | E    | E    | A2   | B2   | B2   | B2   |

$$\mathbf{S} = \mathbf{0}, \mathbf{n}_{\text{occ.}} = \{\mathbf{1}, \mathbf{3}\}$$

| State  | 1282 | 1283 | 1284 | 1285 | 1286 | 1287 | 1288 | 1289 | 1290 | 1291 | 1292 | 1293 |
|--------|------|------|------|------|------|------|------|------|------|------|------|------|
| Sz     | 0    | 0    | 0    | 0    | 0    | 0    | 0    | 0    | 0    | 0    | 0    | 0    |
| Rx     | 1    | 1    | 1    | 1    | 0    | 0    | 0    | 0    | 0    | 0    | -1   | -1   |
| Ry     | 1    | 1    | 1    | 1    | 0    | 0    | 0    | 0    | 0    | 0    | -1   | -1   |
| R      | 1    | 1    | -1   | -1   | $i$  | $i$  | $i$  | $-i$ | $-i$ | $-i$ | 1    | -1   |
| Landau | A1   | A1   | B1   | B1   | E    | E    | E    | E    | E    | E    | A2   | B2   |



$$\mathbf{S} = \mathbf{0}, \text{ n}_{\text{occ.}} = \{0, 4\}$$

$$\left( \begin{array}{cccc} \text{State} & 1294 & 1295 & 1296 \\ \text{Sz} & 0 & 0 & 0 \\ \text{Rx} & 1 & 1 & -1 \\ \text{Ry} & 1 & 1 & -1 \\ \text{R} & 1 & 1 & -1 \\ \text{Landau} & \text{A1} & \text{A1} & \text{B2} \end{array} \right)$$





$$S = 3, \text{ n}_{\text{occ.}} = \{4, 0, 0\}$$

[illegible]

$$\mathbf{S} = \mathbf{3}, \mathbf{n}_{\text{occ.}} = \{\mathbf{3}, \mathbf{0}, \mathbf{1}\}$$

[illegible]

$$\mathbf{S} = \mathbf{3}, \mathbf{n}_{\text{occ.}} = \{\mathbf{2}, \mathbf{2}, \mathbf{0}\}$$

|        |    |    |    |    |    |    |    |    |    |     |     |     |     |     |     |     |     |     |     |     |     |     |     |     |     |     |     |     |     |     |     |     |     |     |     |     |     |     |     |     |     |     |    |    |    |
|--------|----|----|----|----|----|----|----|----|----|-----|-----|-----|-----|-----|-----|-----|-----|-----|-----|-----|-----|-----|-----|-----|-----|-----|-----|-----|-----|-----|-----|-----|-----|-----|-----|-----|-----|-----|-----|-----|-----|-----|----|----|----|
| State  | 91 | 92 | 93 | 94 | 95 | 96 | 97 | 98 | 99 | 100 | 101 | 102 | 103 | 104 | 105 | 106 | 107 | 108 | 109 | 110 | 111 | 112 | 113 | 114 | 115 | 116 | 117 | 118 | 119 | 120 | 121 | 122 | 123 | 124 | 125 | 126 | 127 | 128 | 129 | 130 | 131 | 132 |    |    |    |
| Sz     | 3  | 2  | 1  | 0  | -1 | -2 | -3 | 3  | 2  | 1   | 0   | -1  | -2  | -3  | 3   | 2   | 1   | 0   | -1  | -2  | -3  | 3   | 2   | 1   | 0   | -1  | -2  | -3  | 3   | 2   | 1   | 0   | -1  | -2  | -3  | 3   | 2   | 1   | 0   | -1  | -2  | -3  |    |    |    |
| Rx     | 1  | 1  | 1  | 1  | 1  | 1  | 1  | 1  | 1  | 1   | 1   | 1   | 1   | 1   | 1   | 1   | 1   | 1   | 1   | 1   | 1   | 0   | 0   | 0   | 0   | 0   | 0   | 0   | 0   | 0   | 0   | 0   | 0   | 0   | 0   | 0   | -1  | -1  | -1  | -1  | -1  | -1  | -1 |    |    |
| Ry     | 1  | 1  | 1  | 1  | 1  | 1  | 1  | 1  | 1  | 1   | 1   | 1   | 1   | 1   | 1   | 1   | 1   | 1   | 1   | 1   | 1   | 0   | 0   | 0   | 0   | 0   | 0   | 0   | 0   | 0   | 0   | 0   | 0   | 0   | 0   | 0   | 0   | 0   | -1  | -1  | -1  | -1  | -1 | -1 | -1 |
| R      | 1  | 1  | 1  | 1  | 1  | 1  | 1  | 1  | 1  | 1   | 1   | 1   | 1   | 1   | 1   | -1  | -1  | -1  | -1  | -1  | -1  | -1  | i   | i   | i   | i   | i   | i   | -i  | -i  | -i  | -i  | -i  | -i  | -i  | -1  | -1  | -1  | -1  | -1  | -1  | -1  | -1 |    |    |
| Landau | A1 | A1 | A1 | A1 | A1 | A1 | A1 | A1 | A1 | A1  | A1  | A1  | A1  | A1  | B1  | B1  | B1  | B1  | B1  | B1  | B1  | E   | E   | E   | E   | E   | E   | E   | E   | E   | E   | E   | E   | E   | E   | E   | E   | B2  | B2  | B2  | B2  | B2  | B2 | B2 |    |

$$\mathbf{S} = \mathbf{5}/\mathbf{2}, \mathbf{n}_{\text{occ.}} = \{\mathbf{3}, \mathbf{1}, \mathbf{0}\}$$

[illegible]

$$\mathbf{S} = \mathbf{5}/\mathbf{2}, \mathbf{n}_{\text{occ.}} = \{\mathbf{2}, \mathbf{1}, \mathbf{1}\}$$

[illegible]





$$\mathbf{S} = \mathbf{2}, \mathbf{n}_{\text{occ.}} = \{4, \mathbf{0}, \mathbf{0}\}$$

| State  | 301 | 302 | 303 | 304 | 305 | 306 | 307 | 308 | 309 | 310 | 311 | 312 | 313 | 314 | 315 | 316 | 317 | 318 | 319 | 320 | 321 | 322  | 323  | 324  | 325  | 326  | 327 | 328 | 329 | 330 |
|--------|-----|-----|-----|-----|-----|-----|-----|-----|-----|-----|-----|-----|-----|-----|-----|-----|-----|-----|-----|-----|-----|------|------|------|------|------|-----|-----|-----|-----|
| Sz     | 2   | 1   | 0   | -1  | -2  | 2   | 1   | 0   | -1  | -2  | 2   | 1   | 0   | -1  | -2  | 2   | 1   | 0   | -1  | -2  | 2   | 1    | 0    | -1   | -2   | 2    | 1   | 0   | -1  | -2  |
| Rx     | 1   | 1   | 1   | 1   | 1   | 1   | 1   | 1   | 1   | 1   | 1   | 1   | 1   | 1   | 1   | 0   | 0   | 0   | 0   | 0   | 0   | 0    | 0    | 0    | 0    | 0    | -1  | -1  | -1  | -1  |
| Ry     | 1   | 1   | 1   | 1   | 1   | 1   | 1   | 1   | 1   | 1   | 1   | 1   | 1   | 1   | 1   | 0   | 0   | 0   | 0   | 0   | 0   | 0    | 0    | 0    | 0    | 0    | -1  | -1  | -1  | -1  |
| R      | 1   | 1   | 1   | 1   | 1   | 1   | 1   | 1   | 1   | 1   | 1   | -1  | -1  | -1  | -1  | -1  | $i$ | $i$ | $i$ | $i$ | $i$ | $-i$ | $-i$ | $-i$ | $-i$ | $-i$ | -1  | -1  | -1  | -1  |
| Landau | A1  | A1  | A1  | A1  | A1  | A1  | A1  | A1  | A1  | A1  | B1  | B1  | B1  | B1  | B1  | E   | E   | E   | E   | E   | E   | E    | E    | E    | E    | E    | B2  | B2  | B2  | B2  |

$$\mathbf{S} = \mathbf{2}, \mathbf{n}_{\text{occ.}} = \{\mathbf{3}, \mathbf{0}, \mathbf{1}\}$$

|        |     |     |     |     |     |     |     |     |     |     |     |     |     |     |     |     |     |     |     |     |     |     |     |     |     |     |     |     |     |     |     |     |     |     |     |     |     |     |     |     |    |
|--------|-----|-----|-----|-----|-----|-----|-----|-----|-----|-----|-----|-----|-----|-----|-----|-----|-----|-----|-----|-----|-----|-----|-----|-----|-----|-----|-----|-----|-----|-----|-----|-----|-----|-----|-----|-----|-----|-----|-----|-----|----|
| State  | 331 | 332 | 333 | 334 | 335 | 336 | 337 | 338 | 339 | 340 | 341 | 342 | 343 | 344 | 345 | 346 | 347 | 348 | 349 | 350 | 351 | 352 | 353 | 354 | 355 | 356 | 357 | 358 | 359 | 360 | 361 | 362 | 363 | 364 | 365 | 366 | 367 | 368 | 369 | 370 |    |
| Sz     | 2   | 1   | 0   | -1  | -2  | 2   | 1   | 0   | -1  | -2  | 2   | 1   | 0   | -1  | -2  | 2   | 1   | 0   | -1  | -2  | 2   | 1   | 0   | -1  | -2  | 2   | 1   | 0   | -1  | -2  | 2   | 1   | 0   | -1  | -2  | 2   | 1   | 0   | -1  | -2  |    |
| Rx     | 1   | 1   | 1   | 1   | 1   | 1   | 1   | 1   | 1   | 1   | 0   | 0   | 0   | 0   | 0   | 0   | 0   | 0   | 0   | 0   | 0   | 0   | 0   | 0   | 0   | 0   | 0   | 0   | 0   | 0   | -1  | -1  | -1  | -1  | -1  | -1  | -1  | -1  | -1  | -1  |    |
| Ry     | 1   | 1   | 1   | 1   | 1   | 1   | 1   | 1   | 1   | 1   | 0   | 0   | 0   | 0   | 0   | 0   | 0   | 0   | 0   | 0   | 0   | 0   | 0   | 0   | 0   | 0   | 0   | 0   | 0   | 0   | -1  | -1  | -1  | -1  | -1  | -1  | -1  | -1  | -1  | -1  |    |
| R      | 1   | 1   | 1   | 1   | 1   | -1  | -1  | -1  | -1  | -1  | i   | i   | i   | i   | i   | i   | i   | i   | i   | i   | i   | -i  | -i  | -i  | -i  | -i  | -i  | -i  | -i  | -i  | 1   | 1   | 1   | 1   | 1   | -1  | -1  | -1  | -1  | -1  |    |
| Landau | A1  | A1  | A1  | A1  | A1  | B1  | B1  | B1  | B1  | B1  | E   | E   | E   | E   | E   | E   | E   | E   | E   | E   | E   | E   | E   | E   | E   | E   | E   | E   | E   | E   | A2  | A2  | A2  | A2  | A2  | A2  | B2  | B2  | B2  | B2  | B2 |

$$\mathbf{S} = \mathbf{2}, \mathbf{n}_{\text{acc}} = \{2, 2, 0\}$$

[illegible]

$$\mathbf{S} = \mathbf{2}, \mathbf{n}_{\text{occ.}} = \{\mathbf{2}, \mathbf{0}, \mathbf{2}\}$$

| State  | 461 | 462 | 463 | 464 | 465 | 466 | 467 | 468 | 469 | 470 | 471 | 472 | 473 | 474 | 475 | 476 | 477 | 478 | 479 | 480 | 481 | 482  | 483  | 484  | 485  | 486  | 487 | 488 | 489 | 490 |
|--------|-----|-----|-----|-----|-----|-----|-----|-----|-----|-----|-----|-----|-----|-----|-----|-----|-----|-----|-----|-----|-----|------|------|------|------|------|-----|-----|-----|-----|
| Sz     | 2   | 1   | 0   | -1  | -2  | 2   | 1   | 0   | -1  | -2  | 2   | 1   | 0   | -1  | -2  | 2   | 1   | 0   | -1  | -2  | 2   | 1    | 0    | -1   | -2   | 2    | 1   | 0   | -1  | -2  |
| Rx     | 1   | 1   | 1   | 1   | 1   | 1   | 1   | 1   | 1   | 1   | 1   | 1   | 1   | 1   | 1   | 0   | 0   | 0   | 0   | 0   | 0   | 0    | 0    | 0    | 0    | 0    | -1  | -1  | -1  | -1  |
| Ry     | 1   | 1   | 1   | 1   | 1   | 1   | 1   | 1   | 1   | 1   | 1   | 1   | 1   | 1   | 1   | 0   | 0   | 0   | 0   | 0   | 0   | 0    | 0    | 0    | 0    | 0    | -1  | -1  | -1  | -1  |
| R      | 1   | 1   | 1   | 1   | 1   | 1   | 1   | 1   | 1   | 1   | 1   | -1  | -1  | -1  | -1  | -1  | $i$ | $i$ | $i$ | $i$ | $i$ | $-i$ | $-i$ | $-i$ | $-i$ | $-i$ | -1  | -1  | -1  | -1  |
| Landau | A1  | A1  | A1  | A1  | A1  | A1  | A1  | A1  | A1  | A1  | B1  | B1  | B1  | B1  | B1  | E   | E   | E   | E   | E   | E   | E    | E    | E    | E    | E    | B2  | B2  | B2  | B2  |

$$\mathbf{S} = \mathbf{2}, \mathbf{n}_{\text{occ.}} = \{1, 2, 1\}$$

[illegible]

$$\mathbf{S} = \mathbf{2}, \mathbf{n}_{occ.} = \{\mathbf{0}, 4, \mathbf{0}\}$$

$$\left( \begin{array}{cccccc} \text{State} & 551 & 552 & 553 & 554 & 555 \\ Sz & 2 & 1 & 0 & -1 & -2 \\ Rx & 1 & 1 & 1 & 1 & 1 \\ Ry & 1 & 1 & 1 & 1 & 1 \\ R & 1 & 1 & 1 & 1 & 1 \\ \text{Landau} & A1 & A1 & A1 & A1 & A1 \end{array} \right)$$





$$S = 3/2, n_{occ} = \{2, 1\}$$

[illegible]



$$\mathbf{S} = \mathbf{3}/\mathbf{2}, \mathbf{n}_{\text{occ.}} = \{\mathbf{1}, \mathbf{1}, \mathbf{2}\}$$

$$\left( \begin{array}{cc} \text{State} & 780 & 781 & 782 & 783 & 784 & 785 & 786 & 787 & 788 & 789 & 790 & 791 & 792 & 793 & 794 & 795 & 796 & 797 & 798 & 799 & 800 & 801 & 802 & 803 & 804 & 805 & 806 & 807 & 808 & 809 & 810 & 811 & 812 & 813 & 814 & 815 & 816 & 817 & 818 & 819 & 820 & 821 & 822 & 823 & 824 & 825 & 826 & 827 \\ \text{S}_z & \frac{3}{2} & \frac{1}{2} & -\frac{1}{2} & -\frac{3}{2} & \frac{3}{2} & \frac{1}{2} & -\frac{1}{2} & -\frac{3}{2} & \frac{3}{2} & \frac{1}{2} & -\frac{1}{2} & -\frac{3}{2} & \frac{3}{2} & \frac{1}{2} & -\frac{1}{2} & -\frac{3}{2} & \frac{3}{2} & \frac{1}{2} & -\frac{1}{2} & -\frac{3}{2} & \frac{3}{2} & \frac{1}{2} & -\frac{1}{2} & -\frac{3}{2} & \frac{3}{2} & \frac{1}{2} & -\frac{1}{2} & -\frac{3}{2} & \frac{3}{2} & \frac{1}{2} & -\frac{1}{2} & -\frac{3}{2} & \frac{3}{2} & \frac{1}{2} & -\frac{1}{2} & -\frac{3}{2} & \frac{3}{2} & \frac{1}{2} & -\frac{1}{2} & -\frac{3}{2} & \frac{3}{2} & \frac{1}{2} & -\frac{1}{2} & -\frac{3}{2} \\ \text{R}_x & 1 & 1 & 1 & 1 & 1 & 1 & 1 & 1 & 1 & 1 & 1 & 1 & 1 & 1 & 1 & 1 & 0 & 0 & 0 & 0 & 0 & 0 & 0 & 0 & 0 & 0 & 0 & 0 & 0 & 0 & 0 & 0 & 0 & 0 & 0 & 0 & 0 & 0 & 0 & 0 & -1 & -1 & -1 & -1 & -1 & -1 & -1 & -1 \\ \text{R}_y & 1 & 1 & 1 & 1 & 1 & 1 & 1 & 1 & 1 & 1 & 1 & 1 & 1 & 1 & 1 & 1 & 0 & 0 & 0 & 0 & 0 & 0 & 0 & 0 & 0 & 0 & 0 & 0 & 0 & 0 & 0 & 0 & 0 & 0 & 0 & 0 & 0 & 0 & 0 & 0 & -1 & -1 & -1 & -1 & -1 & -1 & -1 & -1 \\ \text{R} & 1 & 1 & 1 & 1 & 1 & 1 & 1 & 1 & -1 & -1 & -1 & -1 & -1 & -1 & -1 & -1 & i & i & i & i & i & i & i & i & i & i & i & i & -i & -i & -i & -i & -i & -i & -i & -i & -i & -i & 1 & 1 & 1 & 1 & -1 & -1 & -1 & -1 \\ \text{Landau} & \text{A1} & \text{A1} & \text{A1} & \text{A1} & \text{A1} & \text{A1} & \text{A1} & \text{A1} & \text{B1} & \text{B1} & \text{B1} & \text{B1} & \text{B1} & \text{B1} & \text{B1} & \text{B1} & \text{E} & \text{E} & \text{E} & \text{E} & \text{E} & \text{E} & \text{E} & \text{E} & \text{E} & \text{E} & \text{E} & \text{E} & \text{E} & \text{E} & \text{E} & \text{E} & \text{E} & \text{E} & \text{E} & \text{E} & \text{E} & \text{E} & \text{A2} & \text{A2} & \text{A2} & \text{A2} & \text{B2} & \text{B2} & \text{B2} & \text{B2} \end{array} \right)$$

$$\mathbf{S} = \mathbf{3}/\mathbf{2}, \text{ n}_{\text{occ.}} = \{\mathbf{0}, \mathbf{3}, \mathbf{1}\}$$

| State  | 828           | 829           | 830            | 831            | 832           | 833           | 834            | 835            | 836           | 837           | 838            | 839            | 840           | 841           | 842            | 843            |
|--------|---------------|---------------|----------------|----------------|---------------|---------------|----------------|----------------|---------------|---------------|----------------|----------------|---------------|---------------|----------------|----------------|
| Sz     | $\frac{3}{2}$ | $\frac{1}{2}$ | $-\frac{1}{2}$ | $-\frac{3}{2}$ | $\frac{3}{2}$ | $\frac{1}{2}$ | $-\frac{1}{2}$ | $-\frac{3}{2}$ | $\frac{3}{2}$ | $\frac{1}{2}$ | $-\frac{1}{2}$ | $-\frac{3}{2}$ | $\frac{3}{2}$ | $\frac{1}{2}$ | $-\frac{1}{2}$ | $-\frac{3}{2}$ |
| Rx     | 1             | 1             | 1              | 1              | 1             | 1             | 1              | 1              | 0             | 0             | 0              | 0              | 0             | 0             | 0              | 0              |
| Ry     | 1             | 1             | 1              | 1              | 1             | 1             | 1              | 1              | 0             | 0             | 0              | 0              | 0             | 0             | 0              | 0              |
| R      | 1             | 1             | 1              | 1              | -1            | -1            | -1             | -1             | $i$           | $i$           | $i$            | $i$            | $-i$          | $-i$          | $-i$           | $-i$           |
| Landau | A1            | A1            | A1             | A1             | B1            | B1            | B1             | B1             | E             | E             | E              | E              | E             | E             | E              | E              |

$$S = 1, \text{ n}_{\text{occ.}} = \{4, 0, 0\}$$

[illegible]

$\mathbf{S} = \mathbf{1}, \mathbf{n}_{\text{occ.}} = \{\mathbf{3}, \mathbf{0}, \mathbf{1}\}$

|        |     |     |     |     |     |     |     |     |     |     |     |     |     |     |     |     |     |     |     |     |     |      |      |      |      |      |      |      |      |      |     |     |     |     |     |     |
|--------|-----|-----|-----|-----|-----|-----|-----|-----|-----|-----|-----|-----|-----|-----|-----|-----|-----|-----|-----|-----|-----|------|------|------|------|------|------|------|------|------|-----|-----|-----|-----|-----|-----|
| State  | 862 | 863 | 864 | 865 | 866 | 867 | 868 | 869 | 870 | 871 | 872 | 873 | 874 | 875 | 876 | 877 | 878 | 879 | 880 | 881 | 882 | 883  | 884  | 885  | 886  | 887  | 888  | 889  | 890  | 891  | 892 | 893 | 894 | 895 | 896 | 897 |
| Sz     | 1   | 0   | -1  | 1   | 0   | -1  | 1   | 0   | -1  | 1   | 0   | -1  | 1   | 0   | -1  | 1   | 0   | -1  | 1   | 0   | -1  | 1    | 0    | -1   | 1    | 0    | -1   | 1    | 0    | -1   | 1   | 0   | -1  | 1   | 0   | -1  |
| Rx     | 1   | 1   | 1   | 1   | 1   | 1   | 1   | 1   | 1   | 1   | 1   | 1   | 0   | 0   | 0   | 0   | 0   | 0   | 0   | 0   | 0   | 0    | 0    | 0    | 0    | 0    | 0    | 0    | 0    | 0    | -1  | -1  | -1  | -1  | -1  | -1  |
| Ry     | 1   | 1   | 1   | 1   | 1   | 1   | 1   | 1   | 1   | 1   | 1   | 1   | 0   | 0   | 0   | 0   | 0   | 0   | 0   | 0   | 0   | 0    | 0    | 0    | 0    | 0    | 0    | 0    | 0    | 0    | -1  | -1  | -1  | -1  | -1  | -1  |
| R      | 1   | 1   | 1   | 1   | 1   | 1   | -1  | -1  | -1  | -1  | -1  | -1  | $i$ | $i$ | $i$ | $i$ | $i$ | $i$ | $i$ | $i$ | $i$ | $-i$ | $-i$ | $-i$ | $-i$ | $-i$ | $-i$ | $-i$ | $-i$ | $-i$ | 1   | 1   | 1   | -1  | -1  | -1  |
| Landau | A1  | A1  | A1  | A1  | A1  | A1  | B1  | B1  | B1  | B1  | B1  | B1  | E   | E   | E   | E   | E   | E   | E   | E   | E   | E    | E    | E    | E    | E    | E    | E    | E    | E    | A2  | A2  | A2  | B2  | B2  | B2  |



$$S = 1, \text{ n}_{\text{occ.}} = \{2, 0, 2\}$$

$$\left( \begin{array}{c|cccccccccccccccccccc} \text{State} & 970 & 971 & 972 & 973 & 974 & 975 & 976 & 977 & 978 & 979 & 980 & 981 & 982 & 983 & 984 & 985 & 986 & 987 \\ \hline \text{Sz} & 1 & 0 & -1 & 1 & 0 & -1 & 1 & 0 & -1 & 1 & 0 & -1 & 1 & 0 & -1 & 1 & 0 & -1 \\ \text{Rx} & 1 & 1 & 1 & 0 & 0 & 0 & 0 & 0 & 0 & 0 & 0 & 0 & 0 & 0 & 0 & -1 & -1 & -1 \\ \text{Ry} & 1 & 1 & 1 & 0 & 0 & 0 & 0 & 0 & 0 & 0 & 0 & 0 & 0 & 0 & 0 & -1 & -1 & -1 \\ \text{R} & -1 & -1 & -1 & i & i & i & i & i & i & -i & -i & -i & -i & -i & -i & 1 & 1 & 1 \\ \text{Landau} & \text{B1} & \text{B1} & \text{B1} & \text{E} & \text{E} & \text{E} & \text{E} & \text{E} & \text{E} & \text{E} & \text{E} & \text{E} & \text{E} & \text{E} & \text{E} & \text{A2} & \text{A2} & \text{A2} \end{array} \right)$$





$$\mathbf{S} = \mathbf{1}, \mathbf{n}_{\text{occ.}} = \{\mathbf{1}, \mathbf{0}, \mathbf{3}\}$$

| State  | 1060 | 1061 | 1062 | 1063 | 1064 | 1065 | 1066 | 1067 | 1068 | 1069 | 1070 | 1071 |
|--------|------|------|------|------|------|------|------|------|------|------|------|------|
| Sz     | 1    | 0    | -1   | 1    | 0    | -1   | 1    | 0    | -1   | 1    | 0    | -1   |
| Rx     | 1    | 1    | 1    | 1    | 1    | 1    | 0    | 0    | 0    | 0    | 0    | 0    |
| Ry     | 1    | 1    | 1    | 1    | 1    | 1    | 0    | 0    | 0    | 0    | 0    | 0    |
| R      | 1    | 1    | 1    | -1   | -1   | -1   | $i$  | $i$  | $i$  | $-i$ | $-i$ | $-i$ |
| Landau | A1   | A1   | A1   | B1   | B1   | B1   | E    | E    | E    | E    | E    | E    |



$$\mathbf{S} = \mathbf{1}, \mathbf{n}_{\text{occ.}} = \{0, 2, 2\}$$

$$\left( \begin{array}{c} \text{State} \\ \text{Sz} \\ \text{Rx} \\ \text{Ry} \\ \text{R} \\ \text{Landau} \end{array} \begin{array}{cccccccccccccccccccccccc} 1081 & 1082 & 1083 & 1084 & 1085 & 1086 & 1087 & 1088 & 1089 & 1090 & 1091 & 1092 & 1093 & 1094 & 1095 & 1096 & 1097 & 1098 \end{array} \right)$$

$$\mathbf{S} = \mathbf{1}/2, \mathbf{n}_{\text{occ.}} = \{\mathbf{3}, \mathbf{1}, \mathbf{0}\}$$

$$\left( \begin{array}{c|cccccccccccccccccccccccccccccccccccc} \text{State} & 1099 & 1100 & 1101 & 1102 & 1103 & 1104 & 1105 & 1106 & 1107 & 1108 & 1109 & 1110 & 1111 & 1112 & 1113 & 1114 & 1115 & 1116 & 1117 & 1118 & 1119 & 1120 & 1121 & 1122 & 1123 & 1124 & 1125 & 1126 & 1127 & 1128 & 1129 & 1130 \\ \hline S_z & \frac{1}{2} & -\frac{1}{2} & \frac{1}{2} & -\frac{1}{2} & \frac{1}{2} & -\frac{1}{2} & \frac{1}{2} & -\frac{1}{2} & \frac{1}{2} & -\frac{1}{2} & \frac{1}{2} & -\frac{1}{2} & \frac{1}{2} & -\frac{1}{2} & \frac{1}{2} & -\frac{1}{2} & \frac{1}{2} & -\frac{1}{2} & \frac{1}{2} & -\frac{1}{2} & \frac{1}{2} & -\frac{1}{2} & \frac{1}{2} & -\frac{1}{2} & \frac{1}{2} & -\frac{1}{2} & \frac{1}{2} & -\frac{1}{2} & \frac{1}{2} & -\frac{1}{2} \\ R_x & 1 & 1 & 1 & 1 & 1 & 1 & 1 & 1 & 0 & 0 & 0 & 0 & 0 & 0 & 0 & 0 & 0 & 0 & 0 & 0 & 0 & 0 & 0 & 0 & -1 & -1 & -1 & -1 & -1 & -1 & -1 & -1 \\ R_y & 1 & 1 & 1 & 1 & 1 & 1 & 1 & 1 & 0 & 0 & 0 & 0 & 0 & 0 & 0 & 0 & 0 & 0 & 0 & 0 & 0 & 0 & 0 & 0 & -1 & -1 & -1 & -1 & -1 & -1 & -1 & -1 \\ R & 1 & 1 & 1 & 1 & -1 & -1 & -1 & -1 & i & i & i & i & i & i & i & i & -i & -i & -i & -i & -i & -i & -i & -i & 1 & 1 & 1 & 1 & -1 & -1 & -1 & -1 \\ \text{Landau} & A1 & A1 & A1 & A1 & B1 & B1 & B1 & B1 & E & E & E & E & E & E & E & E & E & E & E & E & E & E & E & E & A2 & A2 & A2 & A2 & B2 & B2 & B2 & B2 \end{array} \right)$$

$$\mathbf{S} = \mathbf{1}/2, \mathbf{n}_{\text{occ.}} = \{\mathbf{2}, \mathbf{1}, \mathbf{1}\}$$

| State  | 1131          | 1132           | 1133          | 1134           | 1135          | 1136           | 1137          | 1138           | 1139          | 1140           | 1141          | 1142           | 1143          | 1144           | 1145          | 1146           | 1147          | 1148           | 1149          | 1150           | 1151          | 1152           | 1153          | 1154           | 1155          | 1156           | 1157          | 1158           | 1159          | 1160           | 1161          | 1162           | 1163          | 1164           | 1165          | 1166           | 1167          | 1168           | 1169          | 1170           | 1171          | 1172           | 1173          | 1174           | 1175 | 1176 | 1177 | 1178 |    |    |
|--------|---------------|----------------|---------------|----------------|---------------|----------------|---------------|----------------|---------------|----------------|---------------|----------------|---------------|----------------|---------------|----------------|---------------|----------------|---------------|----------------|---------------|----------------|---------------|----------------|---------------|----------------|---------------|----------------|---------------|----------------|---------------|----------------|---------------|----------------|---------------|----------------|---------------|----------------|---------------|----------------|---------------|----------------|---------------|----------------|------|------|------|------|----|----|
| Sz     | $\frac{1}{2}$ | $-\frac{1}{2}$ | $\frac{1}{2}$ | $-\frac{1}{2}$ | $\frac{1}{2}$ | $-\frac{1}{2}$ | $\frac{1}{2}$ | $-\frac{1}{2}$ | $\frac{1}{2}$ | $-\frac{1}{2}$ | $\frac{1}{2}$ | $-\frac{1}{2}$ | $\frac{1}{2}$ | $-\frac{1}{2}$ | $\frac{1}{2}$ | $-\frac{1}{2}$ | $\frac{1}{2}$ | $-\frac{1}{2}$ | $\frac{1}{2}$ | $-\frac{1}{2}$ | $\frac{1}{2}$ | $-\frac{1}{2}$ | $\frac{1}{2}$ | $-\frac{1}{2}$ | $\frac{1}{2}$ | $-\frac{1}{2}$ | $\frac{1}{2}$ | $-\frac{1}{2}$ | $\frac{1}{2}$ | $-\frac{1}{2}$ | $\frac{1}{2}$ | $-\frac{1}{2}$ | $\frac{1}{2}$ | $-\frac{1}{2}$ | $\frac{1}{2}$ | $-\frac{1}{2}$ | $\frac{1}{2}$ | $-\frac{1}{2}$ | $\frac{1}{2}$ | $-\frac{1}{2}$ | $\frac{1}{2}$ | $-\frac{1}{2}$ | $\frac{1}{2}$ | $-\frac{1}{2}$ |      |      |      |      |    |    |
| Rx     | 1             | 1              | 1             | 1              | 1             | 1              | 1             | 1              | 1             | 1              | 1             | 1              | 0             | 0              | 0             | 0              | 0             | 0              | 0             | 0              | 0             | 0              | 0             | 0              | 0             | 0              | 0             | 0              | 0             | 0              | 0             | 0              | 0             | 0              | 0             | 0              | -1            | -1             | -1            | -1             | -1            | -1             | -1            | -1             | -1   | -1   |      |      |    |    |
| Ry     | 1             | 1              | 1             | 1              | 1             | 1              | 1             | 1              | 1             | 1              | 1             | 1              | 0             | 0              | 0             | 0              | 0             | 0              | 0             | 0              | 0             | 0              | 0             | 0              | 0             | 0              | 0             | 0              | 0             | 0              | 0             | 0              | 0             | 0              | 0             | 0              | 0             | -1             | -1            | -1             | -1            | -1             | -1            | -1             | -1   | -1   | -1   |      |    |    |
| R      | 1             | 1              | 1             | 1              | 1             | 1              | -1            | -1             | -1            | -1             | -1            | -1             | $i$           | $i$            | $i$           | $i$            | $i$           | $i$            | $i$           | $i$            | $i$           | $i$            | $i$           | $i$            | $i$           | $-i$           | $-i$          | $-i$           | $-i$          | $-i$           | $-i$          | $-i$           | $-i$          | $-i$           | $-i$          | 1              | 1             | 1              | 1             | 1              | 1             | -1             | -1            | -1             | -1   |      |      |      |    |    |
| Landau | A1            | A1             | A1            | A1             | A1            | A1             | B1            | B1             | B1            | B1             | B1            | B1             | E             | E              | E             | E              | E             | E              | E             | E              | E             | E              | E             | E              | E             | E              | E             | E              | E             | E              | E             | E              | E             | E              | E             | E              | A2            | A2             | A2            | A2             | A2            | A2             | A2            | A2             | B2   | B2   | B2   | B2   | B2 | B2 |

$$\mathbf{S} = \mathbf{1}/2, \mathbf{n}_{\text{occ.}} = \{\mathbf{1}, \mathbf{3}, \mathbf{0}\}$$

| State  | 1179          | 1180           | 1181          | 1182           | 1183          | 1184           | 1185          | 1186           | 1187          | 1188           | 1189          | 1190           | 1191          | 1192           | 1193          | 1194           | 1195          | 1196           | 1197          | 1198           | 1199          | 1200           | 1201          | 1202           |
|--------|---------------|----------------|---------------|----------------|---------------|----------------|---------------|----------------|---------------|----------------|---------------|----------------|---------------|----------------|---------------|----------------|---------------|----------------|---------------|----------------|---------------|----------------|---------------|----------------|
| Sz     | $\frac{1}{2}$ | $-\frac{1}{2}$ | $\frac{1}{2}$ | $-\frac{1}{2}$ | $\frac{1}{2}$ | $-\frac{1}{2}$ | $\frac{1}{2}$ | $-\frac{1}{2}$ | $\frac{1}{2}$ | $-\frac{1}{2}$ | $\frac{1}{2}$ | $-\frac{1}{2}$ | $\frac{1}{2}$ | $-\frac{1}{2}$ | $\frac{1}{2}$ | $-\frac{1}{2}$ | $\frac{1}{2}$ | $-\frac{1}{2}$ | $\frac{1}{2}$ | $-\frac{1}{2}$ | $\frac{1}{2}$ | $-\frac{1}{2}$ | $\frac{1}{2}$ | $-\frac{1}{2}$ |
| Rx     | 1             | 1              | 1             | 1              | 1             | 1              | 1             | 1              | 0             | 0              | 0             | 0              | 0             | 0              | 0             | 0              | 0             | 0              | 0             | 0              | -1            | -1             | -1            | -1             |
| Ry     | 1             | 1              | 1             | 1              | 1             | 1              | 1             | 1              | 0             | 0              | 0             | 0              | 0             | 0              | 0             | 0              | 0             | 0              | 0             | 0              | -1            | -1             | -1            | -1             |
| R      | 1             | 1              | 1             | 1              | -1            | -1             | -1            | -1             | $i$           | $i$            | $i$           | $i$            | $i$           | $i$            | $-i$          | $-i$           | $-i$          | $-i$           | $-i$          | $-i$           | 1             | 1              | -1            | -1             |
| Landau | A1            | A1             | A1            | A1             | B1            | B1             | B1            | B1             | E             | E              | E             | E              | E             | E              | E             | E              | E             | E              | E             | E              | A2            | A2             | B2            | B2             |

$$\mathbf{S} = \mathbf{1}/2, \mathbf{n}_{\text{occ.}} = \{\mathbf{1}, \mathbf{1}, \mathbf{2}\}$$

| State  | 1203          | 1204           | 1205          | 1206           | 1207          | 1208           | 1209          | 1210           | 1211          | 1212           | 1213          | 1214           | 1215          | 1216           | 1217          | 1218           | 1219          | 1220           | 1221          | 1222           | 1223          | 1224           | 1225          | 1226           |
|--------|---------------|----------------|---------------|----------------|---------------|----------------|---------------|----------------|---------------|----------------|---------------|----------------|---------------|----------------|---------------|----------------|---------------|----------------|---------------|----------------|---------------|----------------|---------------|----------------|
| Sz     | $\frac{1}{2}$ | $-\frac{1}{2}$ | $\frac{1}{2}$ | $-\frac{1}{2}$ | $\frac{1}{2}$ | $-\frac{1}{2}$ | $\frac{1}{2}$ | $-\frac{1}{2}$ | $\frac{1}{2}$ | $-\frac{1}{2}$ | $\frac{1}{2}$ | $-\frac{1}{2}$ | $\frac{1}{2}$ | $-\frac{1}{2}$ | $\frac{1}{2}$ | $-\frac{1}{2}$ | $\frac{1}{2}$ | $-\frac{1}{2}$ | $\frac{1}{2}$ | $-\frac{1}{2}$ | $\frac{1}{2}$ | $-\frac{1}{2}$ | $\frac{1}{2}$ | $-\frac{1}{2}$ |
| Rx     | 1             | 1              | 1             | 1              | 1             | 1              | 1             | 1              | 0             | 0              | 0             | 0              | 0             | 0              | 0             | 0              | 0             | 0              | 0             | 0              | -1            | -1             | -1            | -1             |
| Ry     | 1             | 1              | 1             | 1              | 1             | 1              | 1             | 1              | 0             | 0              | 0             | 0              | 0             | 0              | 0             | 0              | 0             | 0              | 0             | 0              | -1            | -1             | -1            | -1             |
| R      | 1             | 1              | 1             | 1              | -1            | -1             | -1            | -1             | $i$           | $i$            | $i$           | $i$            | $i$           | $i$            | $-i$          | $-i$           | $-i$          | $-i$           | $-i$          | $-i$           | 1             | 1              | -1            | -1             |
| Landau | A1            | A1             | A1            | A1             | B1            | B1             | B1            | B1             | E             | E              | E             | E              | E             | E              | E             | E              | E             | E              | E             | E              | A2            | A2             | B2            | B2             |





$$\mathbf{S} = \mathbf{1}/\mathbf{2}, \text{ n}_{\text{occ.}} = \{\mathbf{0}, \mathbf{1}, \mathbf{3}\}$$

$$\left( \begin{array}{cccccccc} \text{State} & 1243 & 1244 & 1245 & 1246 & 1247 & 1248 & 1249 & 1250 \\ \text{Sz} & \frac{1}{2} & -\frac{1}{2} & \frac{1}{2} & -\frac{1}{2} & \frac{1}{2} & -\frac{1}{2} & \frac{1}{2} & -\frac{1}{2} \\ \text{Rx} & 1 & 1 & 1 & 1 & 0 & 0 & 0 & 0 \\ \text{Ry} & 1 & 1 & 1 & 1 & 0 & 0 & 0 & 0 \\ \text{R} & 1 & 1 & -1 & -1 & i & i & -i & -i \\ \text{Landau} & \text{A1} & \text{A1} & \text{B1} & \text{B1} & \text{E} & \text{E} & \text{E} & \text{E} \end{array} \right)$$

$$\mathbf{S} = \mathbf{0}, \mathbf{n}_{\text{occ.}} = \{4, \mathbf{0}, \mathbf{0}\}$$

$$\left( \begin{array}{cccc} \text{State} & 1251 & 1252 & 1253 \\ S_z & 0 & 0 & 0 \\ R_x & 1 & 1 & -1 \\ R_y & 1 & 1 & -1 \\ R & 1 & 1 & -1 \\ \text{Landau} & A1 & A1 & B2 \end{array} \right)$$

$$\mathbf{S} = \mathbf{0}, \text{ n}_{\text{occ.}} = \{3, 0, 1\}$$

$$\left( \begin{array}{ccccc} \text{State} & 1254 & 1255 & 1256 & 1257 \\ \text{Sz} & 0 & 0 & 0 & 0 \\ \text{Rx} & 0 & 0 & -1 & -1 \\ \text{Ry} & 0 & 0 & -1 & -1 \\ \text{R} & i & -i & 1 & -1 \\ \text{Landau} & \text{E} & \text{E} & \text{A2} & \text{B2} \end{array} \right)$$



$$\mathbf{S} = \mathbf{0}, \mathbf{n}_{\text{occ.}} = \{\mathbf{2}, \mathbf{0}, \mathbf{2}\}$$

| State  | 1270 | 1271 | 1272 | 1273 | 1274 | 1275 |
|--------|------|------|------|------|------|------|
| Sz     | 0    | 0    | 0    | 0    | 0    | 0    |
| Rx     | 1    | 1    | 1    | 0    | 0    | -1   |
| Ry     | 1    | 1    | 1    | 0    | 0    | -1   |
| R      | 1    | 1    | -1   | $i$  | $-i$ | -1   |
| Landau | A1   | A1   | B1   | E    | E    | B2   |

$$\mathbf{S} = \mathbf{0}, \mathbf{n}_{\text{occ.}} = \{\mathbf{1}, \mathbf{2}, \mathbf{1}\}$$

| State  | 1276 | 1277 | 1278 | 1279 | 1280 | 1281 | 1282 | 1283 | 1284 | 1285 | 1286 | 1287 |
|--------|------|------|------|------|------|------|------|------|------|------|------|------|
| Sz     | 0    | 0    | 0    | 0    | 0    | 0    | 0    | 0    | 0    | 0    | 0    | 0    |
| Rx     | 1    | 1    | 1    | 1    | 0    | 0    | 0    | 0    | 0    | 0    | -1   | -1   |
| Ry     | 1    | 1    | 1    | 1    | 0    | 0    | 0    | 0    | 0    | 0    | -1   | -1   |
| R      | 1    | 1    | -1   | -1   | $i$  | $i$  | $i$  | $-i$ | $-i$ | $-i$ | 1    | -1   |
| Landau | A1   | A1   | B1   | B1   | E    | E    | E    | E    | E    | E    | A2   | B2   |

$$\mathbf{S} = \mathbf{0}, \mathbf{n}_{\text{occ.}} = \{0, 4, 0\}$$

$$\left( \begin{array}{ccc} \text{State} & 1288 & 1289 \\ \text{Sz} & 0 & 0 \\ \text{Rx} & 1 & -1 \\ \text{Ry} & 1 & -1 \\ \text{R} & 1 & -1 \\ \text{Landau} & \text{A1} & \text{B2} \end{array} \right)$$



$$\mathbf{S} = \mathbf{0}, \mathbf{n}_{\text{occ.}} = \{\mathbf{0}, \mathbf{2}, \mathbf{2}\}$$

| State  | 1290 | 1291 | 1292 | 1293 | 1294 | 1295 |
|--------|------|------|------|------|------|------|
| Sz     | 0    | 0    | 0    | 0    | 0    | 0    |
| Rx     | 1    | 0    | 0    | 0    | 0    | -1   |
| Ry     | 1    | 0    | 0    | 0    | 0    | -1   |
| R      | -1   | $i$  | $i$  | $-i$ | $-i$ | 1    |
| Landau | B1   | E    | E    | E    | E    | A2   |

$$\mathbf{S} = \mathbf{0}, \text{ n}_{\text{occ.}} = \{0, 0, 4\}$$

$$\left( \begin{array}{cc} \text{State} & 1296 \\ \text{Sz} & 0 \\ \text{Rx} & 1 \\ \text{Ry} & 1 \\ \text{R} & 1 \\ \text{Landau} & \text{A1} \end{array} \right)$$



$$\mathbf{S} = \mathbf{3}, \mathbf{n}_{\text{occ.}} = \{4, \mathbf{0}, \mathbf{0}, \mathbf{0}\}$$

[illegible]

$$\mathbf{S} = \mathbf{3}, \mathbf{n}_{\text{occ.}} = \{\mathbf{3}, \mathbf{1}, \mathbf{0}, \mathbf{0}\}$$

[illegible]

$$\mathbf{S} = \mathbf{3}, \mathbf{n}_{\text{occ.}} = \{\mathbf{3}, \mathbf{0}, \mathbf{1}, \mathbf{0}\}$$

[illegible]



$$\mathbf{S} = \mathbf{2}, \mathbf{n}_{\text{occ.}} = \{4, \mathbf{0}, \mathbf{0}, \mathbf{0}\}$$

| State  | 115 | 116 | 117 | 118 | 119 | 120 | 121 | 122 | 123 | 124 | 125 | 126 | 127 | 128 | 129 | 130 | 131 | 132 | 133 | 134 | 135  | 136  | 137  | 138  | 139  | 140 | 141 | 142 | 143 | 144 |
|--------|-----|-----|-----|-----|-----|-----|-----|-----|-----|-----|-----|-----|-----|-----|-----|-----|-----|-----|-----|-----|------|------|------|------|------|-----|-----|-----|-----|-----|
| Sz     | 2   | 1   | 0   | -1  | -2  | 2   | 1   | 0   | -1  | -2  | 2   | 1   | 0   | -1  | -2  | 2   | 1   | 0   | -1  | -2  | 2    | 1    | 0    | -1   | -2   | 2   | 1   | 0   | -1  | -2  |
| Rx     | 1   | 1   | 1   | 1   | 1   | 1   | 1   | 1   | 1   | 1   | 1   | 1   | 1   | 1   | 1   | 0   | 0   | 0   | 0   | 0   | 0    | 0    | 0    | 0    | 0    | 0   | -1  | -1  | -1  | -1  |
| Ry     | 1   | 1   | 1   | 1   | 1   | 1   | 1   | 1   | 1   | 1   | 1   | 1   | 1   | 1   | 1   | 0   | 0   | 0   | 0   | 0   | 0    | 0    | 0    | 0    | 0    | 0   | -1  | -1  | -1  | -1  |
| R      | 1   | 1   | 1   | 1   | 1   | 1   | 1   | 1   | 1   | 1   | -1  | -1  | -1  | -1  | -1  | $i$ | $i$ | $i$ | $i$ | $i$ | $-i$ | $-i$ | $-i$ | $-i$ | $-i$ | -1  | -1  | -1  | -1  | -1  |
| Landau | A1  | A1  | A1  | A1  | A1  | A1  | A1  | A1  | A1  | A1  | B1  | B1  | B1  | B1  | B1  | E   | E   | E   | E   | E   | E    | E    | E    | E    | E    | B2  | B2  | B2  | B2  | B2  |



$$\mathbf{S} = \mathbf{2}, \mathbf{n}_{\text{occ.}} = \{\mathbf{3}, \mathbf{1}, \mathbf{0}, \mathbf{0}\}$$

|        |     |     |     |     |     |     |     |     |     |     |     |     |     |     |     |     |     |     |     |     |     |     |     |     |     |     |     |     |     |     |     |     |     |     |     |     |     |     |     |     |    |
|--------|-----|-----|-----|-----|-----|-----|-----|-----|-----|-----|-----|-----|-----|-----|-----|-----|-----|-----|-----|-----|-----|-----|-----|-----|-----|-----|-----|-----|-----|-----|-----|-----|-----|-----|-----|-----|-----|-----|-----|-----|----|
| State  | 145 | 146 | 147 | 148 | 149 | 150 | 151 | 152 | 153 | 154 | 155 | 156 | 157 | 158 | 159 | 160 | 161 | 162 | 163 | 164 | 165 | 166 | 167 | 168 | 169 | 170 | 171 | 172 | 173 | 174 | 175 | 176 | 177 | 178 | 179 | 180 | 181 | 182 | 183 | 184 |    |
| Sz     | 2   | 1   | 0   | -1  | -2  | 2   | 1   | 0   | -1  | -2  | 2   | 1   | 0   | -1  | -2  | 2   | 1   | 0   | -1  | -2  | 2   | 1   | 0   | -1  | -2  | 2   | 1   | 0   | -1  | -2  | 2   | 1   | 0   | -1  | -2  | 2   | 1   | 0   | -1  | -2  |    |
| Rx     | 1   | 1   | 1   | 1   | 1   | 1   | 1   | 1   | 1   | 1   | 0   | 0   | 0   | 0   | 0   | 0   | 0   | 0   | 0   | 0   | 0   | 0   | 0   | 0   | 0   | 0   | 0   | 0   | 0   | 0   | -1  | -1  | -1  | -1  | -1  | -1  | -1  | -1  | -1  | -1  |    |
| Ry     | 1   | 1   | 1   | 1   | 1   | 1   | 1   | 1   | 1   | 1   | 0   | 0   | 0   | 0   | 0   | 0   | 0   | 0   | 0   | 0   | 0   | 0   | 0   | 0   | 0   | 0   | 0   | 0   | 0   | 0   | 0   | -1  | -1  | -1  | -1  | -1  | -1  | -1  | -1  | -1  | -1 |
| R      | 1   | 1   | 1   | 1   | 1   | -1  | -1  | -1  | -1  | -1  | i   | i   | i   | i   | i   | i   | i   | i   | i   | i   | i   | -i  | -i  | -i  | -i  | -i  | -i  | -i  | -i  | -i  | 1   | 1   | 1   | 1   | 1   | -1  | -1  | -1  | -1  | -1  |    |
| Landau | A1  | A1  | A1  | A1  | A1  | B1  | B1  | B1  | B1  | B1  | E   | E   | E   | E   | E   | E   | E   | E   | E   | E   | E   | E   | E   | E   | E   | E   | E   | E   | E   | E   | E   | A2  | A2  | A2  | A2  | A2  | B2  | B2  | B2  | B2  | B2 |

$\mathbf{S} = \mathbf{2}, \mathbf{n}_{occ.} = \{\mathbf{3}, \mathbf{0}, \mathbf{1}, \mathbf{0}\}$

| State  | 185 | 186 | 187 | 188 | 189 | 190 | 191 | 192 | 193 | 194 | 195      | 196      | 197      | 198      | 199      | 200      | 201      | 202      | 203      | 204      | 205        | 206        | 207        | 208        | 209        | 210        | 211        | 212        | 213        | 214 | 215 | 216 | 217 | 218 | 219 | 220 | 221 | 222 | 223 | 224 |
|--------|-----|-----|-----|-----|-----|-----|-----|-----|-----|-----|----------|----------|----------|----------|----------|----------|----------|----------|----------|----------|------------|------------|------------|------------|------------|------------|------------|------------|------------|-----|-----|-----|-----|-----|-----|-----|-----|-----|-----|-----|
| Sz     | 2   | 1   | 0   | -1  | -2  | 2   | 1   | 0   | -1  | -2  | 2        | 1        | 0        | -1       | -2       | 2        | 1        | 0        | -1       | -2       | 2          | 1          | 0          | -1         | -2         | 2          | 1          | 0          | -1         | -2  | 2   | 1   | 0   | -1  | -2  | 2   | 1   | 0   | -1  | -2  |
| Rx     | 1   | 1   | 1   | 1   | 1   | 1   | 1   | 1   | 1   | 1   | 0        | 0        | 0        | 0        | 0        | 0        | 0        | 0        | 0        | 0        | 0          | 0          | 0          | 0          | 0          | 0          | 0          | 0          | 0          | 0   | -1  | -1  | -1  | -1  | -1  | -1  | -1  | -1  | -1  | -1  |
| Ry     | 1   | 1   | 1   | 1   | 1   | 1   | 1   | 1   | 1   | 1   | 0        | 0        | 0        | 0        | 0        | 0        | 0        | 0        | 0        | 0        | 0          | 0          | 0          | 0          | 0          | 0          | 0          | 0          | 0          | 0   | -1  | -1  | -1  | -1  | -1  | -1  | -1  | -1  | -1  | -1  |
| R      | 1   | 1   | 1   | 1   | 1   | -1  | -1  | -1  | -1  | -1  | <i>i</i> | <i>i</i> | <i>i</i> | <i>i</i> | <i>i</i> | <i>i</i> | <i>i</i> | <i>i</i> | <i>i</i> | <i>i</i> | - <i>i</i> | - <i>i</i> | - <i>i</i> | - <i>i</i> | - <i>i</i> | - <i>i</i> | - <i>i</i> | - <i>i</i> | - <i>i</i> | 1   | 1   | 1   | 1   | 1   | -1  | -1  | -1  | -1  | -1  |     |
| Landau | A1  | A1  | A1  | A1  | A1  | B1  | B1  | B1  | B1  | B1  | E        | E        | E        | E        | E        | E        | E        | E        | E        | E        | E          | E          | E          | E          | E          | E          | E          | E          | E          | E   | A2  | A2  | A2  | A2  | A2  | B2  | B2  | B2  | B2  | B2  |

$\mathbf{S} = \mathbf{2}, \mathbf{n}_{\text{occ.}} = \{\mathbf{3}, \mathbf{0}, \mathbf{0}, \mathbf{1}\}$

|        |     |     |     |     |     |     |     |     |     |     |          |          |          |          |          |          |          |          |          |          |          |            |            |            |            |            |            |            |            |     |     |     |     |     |     |     |     |     |     |     |    |
|--------|-----|-----|-----|-----|-----|-----|-----|-----|-----|-----|----------|----------|----------|----------|----------|----------|----------|----------|----------|----------|----------|------------|------------|------------|------------|------------|------------|------------|------------|-----|-----|-----|-----|-----|-----|-----|-----|-----|-----|-----|----|
| State  | 225 | 226 | 227 | 228 | 229 | 230 | 231 | 232 | 233 | 234 | 235      | 236      | 237      | 238      | 239      | 240      | 241      | 242      | 243      | 244      | 245      | 246        | 247        | 248        | 249        | 250        | 251        | 252        | 253        | 254 | 255 | 256 | 257 | 258 | 259 | 260 | 261 | 262 | 263 | 264 |    |
| Sz     | 2   | 1   | 0   | -1  | -2  | 2   | 1   | 0   | -1  | -2  | 2        | 1        | 0        | -1       | -2       | 2        | 1        | 0        | -1       | -2       | 2        | 1          | 0          | -1         | -2         | 2          | 1          | 0          | -1         | -2  | 2   | 1   | 0   | -1  | -2  | 2   | 1   | 0   | -1  | -2  |    |
| Rx     | 1   | 1   | 1   | 1   | 1   | 1   | 1   | 1   | 1   | 1   | 0        | 0        | 0        | 0        | 0        | 0        | 0        | 0        | 0        | 0        | 0        | 0          | 0          | 0          | 0          | 0          | 0          | 0          | 0          | 0   | -1  | -1  | -1  | -1  | -1  | -1  | -1  | -1  | -1  | -1  |    |
| Ry     | 1   | 1   | 1   | 1   | 1   | 1   | 1   | 1   | 1   | 1   | 0        | 0        | 0        | 0        | 0        | 0        | 0        | 0        | 0        | 0        | 0        | 0          | 0          | 0          | 0          | 0          | 0          | 0          | 0          | 0   | -1  | -1  | -1  | -1  | -1  | -1  | -1  | -1  | -1  | -1  |    |
| R      | 1   | 1   | 1   | 1   | 1   | -1  | -1  | -1  | -1  | -1  | <i>i</i> | <i>i</i> | <i>i</i> | <i>i</i> | <i>i</i> | <i>i</i> | <i>i</i> | <i>i</i> | <i>i</i> | <i>i</i> | <i>i</i> | - <i>i</i> | - <i>i</i> | - <i>i</i> | - <i>i</i> | - <i>i</i> | - <i>i</i> | - <i>i</i> | - <i>i</i> | 1   | 1   | 1   | 1   | 1   | 1   | -1  | -1  | -1  | -1  | -1  |    |
| Landau | A1  | A1  | A1  | A1  | A1  | B1  | B1  | B1  | B1  | B1  | E        | E        | E        | E        | E        | E        | E        | E        | E        | E        | E        | E          | E          | E          | E          | E          | E          | E          | E          | E   | A2  | A2  | A2  | A2  | A2  | A2  | B2  | B2  | B2  | B2  | B2 |

$$\mathbf{S} = \mathbf{2}, \mathbf{n}_{\text{occ.}} = \{\mathbf{2}, \mathbf{2}, \mathbf{0}, \mathbf{0}\}$$

| State  | 265 | 266 | 267 | 268 | 269 | 270 | 271 | 272 | 273 | 274 | 275 | 276 | 277 | 278 | 279 | 280 | 281 | 282 | 283 | 284 | 285  | 286  | 287  | 288  | 289  | 290 | 291 | 292 | 293 | 294 |
|--------|-----|-----|-----|-----|-----|-----|-----|-----|-----|-----|-----|-----|-----|-----|-----|-----|-----|-----|-----|-----|------|------|------|------|------|-----|-----|-----|-----|-----|
| Sz     | 2   | 1   | 0   | -1  | -2  | 2   | 1   | 0   | -1  | -2  | 2   | 1   | 0   | -1  | -2  | 2   | 1   | 0   | -1  | -2  | 2    | 1    | 0    | -1   | -2   | 2   | 1   | 0   | -1  | -2  |
| Rx     | 1   | 1   | 1   | 1   | 1   | 1   | 1   | 1   | 1   | 1   | 1   | 1   | 1   | 1   | 1   | 0   | 0   | 0   | 0   | 0   | 0    | 0    | 0    | 0    | 0    | 0   | -1  | -1  | -1  | -1  |
| Ry     | 1   | 1   | 1   | 1   | 1   | 1   | 1   | 1   | 1   | 1   | 1   | 1   | 1   | 1   | 1   | 0   | 0   | 0   | 0   | 0   | 0    | 0    | 0    | 0    | 0    | 0   | -1  | -1  | -1  | -1  |
| R      | 1   | 1   | 1   | 1   | 1   | 1   | 1   | 1   | 1   | 1   | -1  | -1  | -1  | -1  | -1  | $i$ | $i$ | $i$ | $i$ | $i$ | $-i$ | $-i$ | $-i$ | $-i$ | $-i$ | -1  | -1  | -1  | -1  | -1  |
| Landau | A1  | A1  | A1  | A1  | A1  | A1  | A1  | A1  | A1  | A1  | B1  | B1  | B1  | B1  | B1  | E   | E   | E   | E   | E   | E    | E    | E    | E    | E    | B2  | B2  | B2  | B2  | B2  |

$$\mathbf{S} = \mathbf{2}, \mathbf{n}_{\text{occ.}} = \{\mathbf{2}, \mathbf{1}, \mathbf{1}, \mathbf{0}\}$$

|        |     |     |     |     |     |     |     |     |     |     |     |     |     |     |     |     |     |     |     |     |     |     |     |     |     |     |     |     |     |     |     |     |     |     |     |     |     |     |     |     |     |     |     |     |     |     |     |     |     |     |     |     |     |     |     |     |     |     |     |     |    |    |
|--------|-----|-----|-----|-----|-----|-----|-----|-----|-----|-----|-----|-----|-----|-----|-----|-----|-----|-----|-----|-----|-----|-----|-----|-----|-----|-----|-----|-----|-----|-----|-----|-----|-----|-----|-----|-----|-----|-----|-----|-----|-----|-----|-----|-----|-----|-----|-----|-----|-----|-----|-----|-----|-----|-----|-----|-----|-----|-----|-----|-----|----|----|
| State  | 295 | 296 | 297 | 298 | 299 | 300 | 301 | 302 | 303 | 304 | 305 | 306 | 307 | 308 | 309 | 310 | 311 | 312 | 313 | 314 | 315 | 316 | 317 | 318 | 319 | 320 | 321 | 322 | 323 | 324 | 325 | 326 | 327 | 328 | 329 | 330 | 331 | 332 | 333 | 334 | 335 | 336 | 337 | 338 | 339 | 340 | 341 | 342 | 343 | 344 | 345 | 346 | 347 | 348 | 349 | 350 | 351 | 352 | 353 | 354 |    |    |
| Sz     | 2   | 1   | 0   | -1  | -2  | 2   | 1   | 0   | -1  | -2  | 2   | 1   | 0   | -1  | -2  | 2   | 1   | 0   | -1  | -2  | 2   | 1   | 0   | -1  | -2  | 2   | 1   | 0   | -1  | -2  | 2   | 1   | 0   | -1  | -2  | 2   | 1   | 0   | -1  | -2  | 2   | 1   | 0   | -1  | -2  | 2   | 1   | 0   | -1  | -2  | 2   | 1   | 0   | -1  | -2  |     |     |     |     |     |    |    |
| Rx     | 1   | 1   | 1   | 1   | 1   | 1   | 1   | 1   | 1   | 1   | 1   | 1   | 1   | 1   | 1   | 1   | 1   | 1   | 1   | 1   | 0   | 0   | 0   | 0   | 0   | 0   | 0   | 0   | 0   | 0   | 0   | 0   | 0   | 0   | 0   | 0   | 0   | 0   | 0   | 0   | 0   | 0   | 0   | 0   | 0   | 0   | 0   | 0   | 0   | 0   | -1  | -1  | -1  | -1  | -1  | -1  | -1  | -1  | -1  |     |    |    |
| Ry     | 1   | 1   | 1   | 1   | 1   | 1   | 1   | 1   | 1   | 1   | 1   | 1   | 1   | 1   | 1   | 1   | 1   | 1   | 1   | 1   | 0   | 0   | 0   | 0   | 0   | 0   | 0   | 0   | 0   | 0   | 0   | 0   | 0   | 0   | 0   | 0   | 0   | 0   | 0   | 0   | 0   | 0   | 0   | 0   | 0   | 0   | 0   | 0   | 0   | 0   | 0   | 0   | 0   | -1  | -1  | -1  | -1  | -1  | -1  | -1  | -1 | -1 |
| R      | 1   | 1   | 1   | 1   | 1   | 1   | 1   | 1   | 1   | 1   | -1  | -1  | -1  | -1  | -1  | -1  | -1  | -1  | -1  | -1  | i   | i   | i   | i   | i   | i   | i   | i   | i   | i   | i   | i   | i   | i   | i   | -i  | -i  | -i  | -i  | -i  | -i  | -i  | -i  | -i  | -i  | -i  | -i  | -i  | -i  | -i  | 1   | 1   | 1   | 1   | 1   | -1  | -1  | -1  | -1  | -1  |    |    |
| Landau | A1  | A1  | A1  | A1  | A1  | A1  | A1  | A1  | A1  | A1  | B1  | B1  | B1  | B1  | B1  | B1  | B1  | B1  | B1  | B1  | E   | E   | E   | E   | E   | E   | E   | E   | E   | E   | E   | E   | E   | E   | E   | E   | E   | E   | E   | E   | E   | E   | E   | E   | E   | E   | E   | E   | E   | E   | E   | E   | A2  | A2  | A2  | A2  | A2  | B2  | B2  | B2  | B2 | B2 |

$$\mathbf{S} = \mathbf{2}, \mathbf{n}_{\text{occ.}} = \{ \mathbf{2}, \mathbf{1}, \mathbf{0}, \mathbf{1} \}$$

[illegible]

$$\mathbf{S} = \mathbf{2}, \mathbf{n}_{\text{occ.}} = \{\mathbf{2}, \mathbf{0}, \mathbf{2}, \mathbf{0}\}$$

| State  | 415 | 416 | 417 | 418 | 419 | 420 | 421 | 422 | 423 | 424 | 425 | 426 | 427 | 428 | 429 | 430 | 431 | 432 | 433 | 434 | 435  | 436  | 437  | 438  | 439  | 440  | 441 | 442 | 443 | 444 |
|--------|-----|-----|-----|-----|-----|-----|-----|-----|-----|-----|-----|-----|-----|-----|-----|-----|-----|-----|-----|-----|------|------|------|------|------|------|-----|-----|-----|-----|
| Sz     | 2   | 1   | 0   | -1  | -2  | 2   | 1   | 0   | -1  | -2  | 2   | 1   | 0   | -1  | -2  | 2   | 1   | 0   | -1  | -2  | 2    | 1    | 0    | -1   | -2   | 2    | 1   | 0   | -1  | -2  |
| Rx     | 1   | 1   | 1   | 1   | 1   | 1   | 1   | 1   | 1   | 1   | 1   | 1   | 1   | 1   | 1   | 0   | 0   | 0   | 0   | 0   | 0    | 0    | 0    | 0    | 0    | 0    | -1  | -1  | -1  | -1  |
| Ry     | 1   | 1   | 1   | 1   | 1   | 1   | 1   | 1   | 1   | 1   | 1   | 1   | 1   | 1   | 1   | 0   | 0   | 0   | 0   | 0   | 0    | 0    | 0    | 0    | 0    | 0    | -1  | -1  | -1  | -1  |
| R      | 1   | 1   | 1   | 1   | 1   | 1   | 1   | 1   | 1   | 1   | -1  | -1  | -1  | -1  | -1  | $i$ | $i$ | $i$ | $i$ | $i$ | $-i$ | $-i$ | $-i$ | $-i$ | $-i$ | $-i$ | -1  | -1  | -1  | -1  |
| Landau | A1  | A1  | A1  | A1  | A1  | A1  | A1  | A1  | A1  | A1  | B1  | B1  | B1  | B1  | B1  | E   | E   | E   | E   | E   | E    | E    | E    | E    | E    | B2   | B2  | B2  | B2  | B2  |

$$\mathbf{S} = \mathbf{2}, \mathbf{n}_{\text{occ.}} = \{\mathbf{2}, \mathbf{0}, \mathbf{1}, \mathbf{1}\}$$

[illegible]



$$\mathbf{S} = \mathbf{2}, \mathbf{n}_{\text{occ.}} = \{\mathbf{2}, \mathbf{0}, \mathbf{0}, \mathbf{2}\}$$

| State  | 505 | 506 | 507 | 508 | 509 | 510 | 511 | 512 | 513 | 514 | 515 | 516 | 517 | 518 | 519 | 520 | 521 | 522 | 523 | 524 | 525  | 526  | 527  | 528  | 529  | 530 | 531 | 532 | 533 | 534 |
|--------|-----|-----|-----|-----|-----|-----|-----|-----|-----|-----|-----|-----|-----|-----|-----|-----|-----|-----|-----|-----|------|------|------|------|------|-----|-----|-----|-----|-----|
| Sz     | 2   | 1   | 0   | -1  | -2  | 2   | 1   | 0   | -1  | -2  | 2   | 1   | 0   | -1  | -2  | 2   | 1   | 0   | -1  | -2  | 2    | 1    | 0    | -1   | -2   | 2   | 1   | 0   | -1  | -2  |
| Rx     | 1   | 1   | 1   | 1   | 1   | 1   | 1   | 1   | 1   | 1   | 1   | 1   | 1   | 1   | 1   | 0   | 0   | 0   | 0   | 0   | 0    | 0    | 0    | 0    | 0    | 0   | -1  | -1  | -1  | -1  |
| Ry     | 1   | 1   | 1   | 1   | 1   | 1   | 1   | 1   | 1   | 1   | 1   | 1   | 1   | 1   | 1   | 0   | 0   | 0   | 0   | 0   | 0    | 0    | 0    | 0    | 0    | 0   | -1  | -1  | -1  | -1  |
| R      | 1   | 1   | 1   | 1   | 1   | 1   | 1   | 1   | 1   | 1   | -1  | -1  | -1  | -1  | -1  | $i$ | $i$ | $i$ | $i$ | $i$ | $-i$ | $-i$ | $-i$ | $-i$ | $-i$ | -1  | -1  | -1  | -1  | -1  |
| Landau | A1  | A1  | A1  | A1  | A1  | A1  | A1  | A1  | A1  | A1  | B1  | B1  | B1  | B1  | B1  | E   | E   | E   | E   | E   | E    | E    | E    | E    | E    | B2  | B2  | B2  | B2  | B2  |

$$S = 1, \text{ n}_{\text{occ.}} = \{4, 0, 0, 0\}$$

[illegible]

$$\mathbf{S} = \mathbf{1}, \mathbf{n}_{\text{occ.}} = \{\mathbf{3}, \mathbf{1}, \mathbf{0}, \mathbf{0}\}$$

| State  | 553 | 554 | 555 | 556 | 557 | 558 | 559 | 560 | 561 | 562 | 563 | 564 | 565      | 566      | 567      | 568      | 569      | 570      | 571      | 572      | 573      | 574      | 575        | 576        | 577        | 578        | 579        | 580        | 581        | 582        | 583 | 584 | 585 | 586 | 587 | 588 |
|--------|-----|-----|-----|-----|-----|-----|-----|-----|-----|-----|-----|-----|----------|----------|----------|----------|----------|----------|----------|----------|----------|----------|------------|------------|------------|------------|------------|------------|------------|------------|-----|-----|-----|-----|-----|-----|
| Sz     | 1   | 0   | -1  | 1   | 0   | -1  | 1   | 0   | -1  | 1   | 0   | -1  | 1        | 0        | -1       | 1        | 0        | -1       | 1        | 0        | -1       | 1        | 0          | -1         | 1          | 0          | -1         | 1          | 0          | -1         | 1   | 0   | -1  | 1   | 0   | -1  |
| Rx     | 1   | 1   | 1   | 1   | 1   | 1   | 1   | 1   | 1   | 1   | 1   | 1   | 0        | 0        | 0        | 0        | 0        | 0        | 0        | 0        | 0        | 0        | 0          | 0          | 0          | 0          | 0          | 0          | 0          | 0          | -1  | -1  | -1  | -1  | -1  | -1  |
| Ry     | 1   | 1   | 1   | 1   | 1   | 1   | 1   | 1   | 1   | 1   | 1   | 1   | 0        | 0        | 0        | 0        | 0        | 0        | 0        | 0        | 0        | 0        | 0          | 0          | 0          | 0          | 0          | 0          | 0          | 0          | -1  | -1  | -1  | -1  | -1  | -1  |
| R      | 1   | 1   | 1   | 1   | 1   | 1   | -1  | -1  | -1  | -1  | -1  | -1  | <i>i</i> | <i>i</i> | <i>i</i> | <i>i</i> | <i>i</i> | <i>i</i> | <i>i</i> | <i>i</i> | <i>i</i> | <i>i</i> | - <i>i</i> | - <i>i</i> | - <i>i</i> | - <i>i</i> | - <i>i</i> | - <i>i</i> | - <i>i</i> | - <i>i</i> | 1   | 1   | 1   | -1  | -1  | -1  |
| Landau | A1  | A1  | A1  | A1  | A1  | A1  | B1  | B1  | B1  | B1  | B1  | B1  | E        | E        | E        | E        | E        | E        | E        | E        | E        | E        | E          | E          | E          | E          | E          | E          | E          | E          | A2  | A2  | A2  | B2  | B2  | B2  |

$$\mathbf{S} = \mathbf{1}, \mathbf{n}_{\text{occ.}} = \{\mathbf{3}, \mathbf{0}, \mathbf{1}, \mathbf{0}\}$$

| State  | 589 | 590 | 591 | 592 | 593 | 594 | 595 | 596 | 597 | 598 | 599 | 600 | 601 | 602 | 603 | 604 | 605 | 606 | 607 | 608 | 609 | 610 | 611 | 612  | 613  | 614  | 615  | 616  | 617  | 618  | 619 | 620 | 621 | 622 | 623 | 624 |
|--------|-----|-----|-----|-----|-----|-----|-----|-----|-----|-----|-----|-----|-----|-----|-----|-----|-----|-----|-----|-----|-----|-----|-----|------|------|------|------|------|------|------|-----|-----|-----|-----|-----|-----|
| Sz     | 1   | 0   | -1  | 1   | 0   | -1  | 1   | 0   | -1  | 1   | 0   | -1  | 1   | 0   | -1  | 1   | 0   | -1  | 1   | 0   | -1  | 1   | 0   | -1   | 1    | 0    | -1   | 1    | 0    | -1   | 1   | 0   | -1  | 1   | 0   | -1  |
| Rx     | 1   | 1   | 1   | 1   | 1   | 1   | 1   | 1   | 1   | 1   | 1   | 1   | 0   | 0   | 0   | 0   | 0   | 0   | 0   | 0   | 0   | 0   | 0   | 0    | 0    | 0    | 0    | 0    | 0    | -1   | -1  | -1  | -1  | -1  | -1  |     |
| Ry     | 1   | 1   | 1   | 1   | 1   | 1   | 1   | 1   | 1   | 1   | 1   | 1   | 0   | 0   | 0   | 0   | 0   | 0   | 0   | 0   | 0   | 0   | 0   | 0    | 0    | 0    | 0    | 0    | 0    | 0    | -1  | -1  | -1  | -1  | -1  | -1  |
| R      | 1   | 1   | 1   | 1   | 1   | 1   | -1  | -1  | -1  | -1  | -1  | -1  | $i$ | $i$ | $i$ | $i$ | $i$ | $i$ | $i$ | $i$ | $i$ | $i$ | $i$ | $-i$ | $-i$ | $-i$ | $-i$ | $-i$ | $-i$ | $-i$ | 1   | 1   | 1   | -1  | -1  | -1  |
| Landau | A1  | A1  | A1  | A1  | A1  | A1  | B1  | B1  | B1  | B1  | B1  | B1  | E   | E   | E   | E   | E   | E   | E   | E   | E   | E   | E   | E    | E    | E    | E    | E    | E    | E    | A2  | A2  | A2  | B2  | B2  | B2  |

$$\mathbf{S} = \mathbf{1}, \mathbf{n}_{\text{occ.}} = \{\mathbf{3}, \mathbf{0}, \mathbf{0}, \mathbf{1}\}$$

| State  | 625 | 626 | 627 | 628 | 629 | 630 | 631 | 632 | 633 | 634 | 635 | 636 | 637 | 638 | 639 | 640 | 641 | 642 | 643 | 644 | 645 | 646 | 647  | 648  | 649  | 650  | 651  | 652  | 653  | 654  | 655 | 656 | 657 | 658 | 659 | 660 |
|--------|-----|-----|-----|-----|-----|-----|-----|-----|-----|-----|-----|-----|-----|-----|-----|-----|-----|-----|-----|-----|-----|-----|------|------|------|------|------|------|------|------|-----|-----|-----|-----|-----|-----|
| Sz     | 1   | 0   | -1  | 1   | 0   | -1  | 1   | 0   | -1  | 1   | 0   | -1  | 1   | 0   | -1  | 1   | 0   | -1  | 1   | 0   | -1  | 1   | 0    | -1   | 1    | 0    | -1   | 1    | 0    | -1   | 1   | 0   | -1  | 1   | 0   | -1  |
| Rx     | 1   | 1   | 1   | 1   | 1   | 1   | 1   | 1   | 1   | 1   | 1   | 1   | 0   | 0   | 0   | 0   | 0   | 0   | 0   | 0   | 0   | 0   | 0    | 0    | 0    | 0    | 0    | 0    | 0    | 0    | -1  | -1  | -1  | -1  | -1  | -1  |
| Ry     | 1   | 1   | 1   | 1   | 1   | 1   | 1   | 1   | 1   | 1   | 1   | 1   | 0   | 0   | 0   | 0   | 0   | 0   | 0   | 0   | 0   | 0   | 0    | 0    | 0    | 0    | 0    | 0    | 0    | 0    | -1  | -1  | -1  | -1  | -1  | -1  |
| R      | 1   | 1   | 1   | 1   | 1   | 1   | -1  | -1  | -1  | -1  | -1  | -1  | $i$ | $i$ | $i$ | $i$ | $i$ | $i$ | $i$ | $i$ | $i$ | $i$ | $-i$ | $-i$ | $-i$ | $-i$ | $-i$ | $-i$ | $-i$ | $-i$ | 1   | 1   | 1   | -1  | -1  | -1  |
| Landau | A1  | A1  | A1  | A1  | A1  | A1  | B1  | B1  | B1  | B1  | B1  | B1  | E   | E   | E   | E   | E   | E   | E   | E   | E   | E   | E    | E    | E    | E    | E    | E    | E    | E    | A2  | A2  | A2  | B2  | B2  | B2  |

$$S = 1, \text{ n}_{\text{occ.}} = \{2, 2, 0, 0\}$$

$$\left( \begin{array}{c|cccccccccccccccccccc} \text{State} & 661 & 662 & 663 & 664 & 665 & 666 & 667 & 668 & 669 & 670 & 671 & 672 & 673 & 674 & 675 & 676 & 677 & 678 \\ \hline \text{Sz} & 1 & 0 & -1 & 1 & 0 & -1 & 1 & 0 & -1 & 1 & 0 & -1 & 1 & 0 & -1 & 1 & 0 & -1 \\ \text{Rx} & 1 & 1 & 1 & 0 & 0 & 0 & 0 & 0 & 0 & 0 & 0 & 0 & 0 & 0 & 0 & -1 & -1 & -1 \\ \text{Ry} & 1 & 1 & 1 & 0 & 0 & 0 & 0 & 0 & 0 & 0 & 0 & 0 & 0 & 0 & 0 & -1 & -1 & -1 \\ \text{R} & -1 & -1 & -1 & i & i & i & i & i & i & i & -i & -i & -i & -i & -i & 1 & 1 & 1 \\ \text{Landau} & \text{B1} & \text{B1} & \text{B1} & \text{E} & \text{E} & \text{E} & \text{E} & \text{E} & \text{E} & \text{E} & \text{E} & \text{E} & \text{E} & \text{E} & \text{E} & \text{A2} & \text{A2} & \text{A2} \end{array} \right)$$

$$\mathbf{S} = \mathbf{1}, \mathbf{n}_{\text{occ.}} = \{\mathbf{2}, \mathbf{1}, \mathbf{1}, \mathbf{0}\}$$

| State  | 679 | 680 | 681 | 682 | 683 | 684 | 685 | 686 | 687 | 688 | 689 | 690 | 691 | 692 | 693 | 694  | 695  | 696  | 697  | 698  | 699  | 700  | 701  | 702  | 703 | 704 | 705 | 706 | 707 | 708 | 709 | 710 | 711 | 712 | 713 | 714 |    |
|--------|-----|-----|-----|-----|-----|-----|-----|-----|-----|-----|-----|-----|-----|-----|-----|------|------|------|------|------|------|------|------|------|-----|-----|-----|-----|-----|-----|-----|-----|-----|-----|-----|-----|----|
| Sz     | 1   | 0   | -1  | 1   | 0   | -1  | 1   | 0   | -1  | 1   | 0   | -1  | 1   | 0   | -1  | 1    | 0    | -1   | 1    | 0    | -1   | 1    | 0    | -1   | 1   | 0   | -1  | 1   | 0   | -1  | 1   | 0   | -1  | 1   | 0   | -1  |    |
| Rx     | 1   | 1   | 1   | 1   | 1   | 1   | 0   | 0   | 0   | 0   | 0   | 0   | 0   | 0   | 0   | 0    | 0    | 0    | 0    | 0    | 0    | 0    | 0    | 0    | -1  | -1  | -1  | -1  | -1  | -1  | -1  | -1  | -1  | -1  | -1  | -1  |    |
| Ry     | 1   | 1   | 1   | 1   | 1   | 1   | 0   | 0   | 0   | 0   | 0   | 0   | 0   | 0   | 0   | 0    | 0    | 0    | 0    | 0    | 0    | 0    | 0    | 0    | -1  | -1  | -1  | -1  | -1  | -1  | -1  | -1  | -1  | -1  | -1  | -1  |    |
| R      | 1   | 1   | 1   | -1  | -1  | -1  | $i$ | $i$ | $i$ | $i$ | $i$ | $i$ | $i$ | $i$ | $i$ | $-i$ | $-i$ | $-i$ | $-i$ | $-i$ | $-i$ | $-i$ | $-i$ | $-i$ | 1   | 1   | 1   | 1   | 1   | 1   | -1  | -1  | -1  | -1  | -1  | -1  |    |
| Landau | A1  | A1  | A1  | B1  | B1  | B1  | E   | E   | E   | E   | E   | E   | E   | E   | E   | E    | E    | E    | E    | E    | E    | E    | E    | E    | E   | A2  | A2  | A2  | A2  | A2  | A2  | B2  | B2  | B2  | B2  | B2  | B2 |

$$\mathbf{S} = \mathbf{1}, \mathbf{n}_{\text{occ.}} = \{\mathbf{2}, \mathbf{1}, \mathbf{0}, \mathbf{1}\}$$

| State  | 715 | 716 | 717 | 718 | 719 | 720 | 721      | 722      | 723      | 724      | 725      | 726      | 727      | 728      | 729      | 730      | 731        | 732        | 733        | 734        | 735        | 736        | 737        | 738        | 739 | 740 | 741 | 742 | 743 | 744 | 745 | 746 | 747 | 748 | 749 | 750 |    |
|--------|-----|-----|-----|-----|-----|-----|----------|----------|----------|----------|----------|----------|----------|----------|----------|----------|------------|------------|------------|------------|------------|------------|------------|------------|-----|-----|-----|-----|-----|-----|-----|-----|-----|-----|-----|-----|----|
| Sz     | 1   | 0   | -1  | 1   | 0   | -1  | 1        | 0        | -1       | 1        | 0        | -1       | 1        | 0        | -1       | 1        | 0          | -1         | 1          | 0          | -1         | 1          | 0          | -1         | 1   | 0   | -1  | 1   | 0   | -1  | 1   | 0   | -1  | 1   | 0   | -1  |    |
| Rx     | 1   | 1   | 1   | 1   | 1   | 1   | 0        | 0        | 0        | 0        | 0        | 0        | 0        | 0        | 0        | 0        | 0          | 0          | 0          | 0          | 0          | 0          | 0          | 0          | -1  | -1  | -1  | -1  | -1  | -1  | -1  | -1  | -1  | -1  | -1  | -1  |    |
| Ry     | 1   | 1   | 1   | 1   | 1   | 1   | 0        | 0        | 0        | 0        | 0        | 0        | 0        | 0        | 0        | 0        | 0          | 0          | 0          | 0          | 0          | 0          | 0          | 0          | -1  | -1  | -1  | -1  | -1  | -1  | -1  | -1  | -1  | -1  | -1  | -1  |    |
| R      | 1   | 1   | 1   | -1  | -1  | -1  | <i>i</i> | <i>i</i> | <i>i</i> | <i>i</i> | <i>i</i> | <i>i</i> | <i>i</i> | <i>i</i> | <i>i</i> | <i>i</i> | - <i>i</i> | - <i>i</i> | - <i>i</i> | - <i>i</i> | - <i>i</i> | - <i>i</i> | - <i>i</i> | - <i>i</i> | 1   | 1   | 1   | 1   | 1   | 1   | -1  | -1  | -1  | -1  | -1  | -1  |    |
| Landau | A1  | A1  | A1  | B1  | B1  | B1  | E        | E        | E        | E        | E        | E        | E        | E        | E        | E        | E          | E          | E          | E          | E          | E          | E          | E          | E   | A2  | A2  | A2  | A2  | A2  | A2  | B2  | B2  | B2  | B2  | B2  | B2 |





$$\mathbf{S} = \mathbf{1}, \mathbf{n}_{\text{occ.}} = \{\mathbf{2}, \mathbf{0}, \mathbf{1}, \mathbf{1}\}$$

| State  | 769 | 770 | 771 | 772 | 773 | 774 | 775      | 776      | 777      | 778      | 779      | 780      | 781      | 782      | 783      | 784      | 785        | 786        | 787        | 788        | 789        | 790        | 791        | 792        | 793 | 794 | 795 | 796 | 797 | 798 | 799 | 800 | 801 | 802 | 803 | 804 |    |
|--------|-----|-----|-----|-----|-----|-----|----------|----------|----------|----------|----------|----------|----------|----------|----------|----------|------------|------------|------------|------------|------------|------------|------------|------------|-----|-----|-----|-----|-----|-----|-----|-----|-----|-----|-----|-----|----|
| Sz     | 1   | 0   | -1  | 1   | 0   | -1  | 1        | 0        | -1       | 1        | 0        | -1       | 1        | 0        | -1       | 1        | 0          | -1         | 1          | 0          | -1         | 1          | 0          | -1         | 1   | 0   | -1  | 1   | 0   | -1  | 1   | 0   | -1  | 1   | 0   | -1  |    |
| Rx     | 1   | 1   | 1   | 1   | 1   | 1   | 0        | 0        | 0        | 0        | 0        | 0        | 0        | 0        | 0        | 0        | 0          | 0          | 0          | 0          | 0          | 0          | 0          | 0          | -1  | -1  | -1  | -1  | -1  | -1  | -1  | -1  | -1  | -1  | -1  | -1  |    |
| Ry     | 1   | 1   | 1   | 1   | 1   | 1   | 0        | 0        | 0        | 0        | 0        | 0        | 0        | 0        | 0        | 0        | 0          | 0          | 0          | 0          | 0          | 0          | 0          | 0          | -1  | -1  | -1  | -1  | -1  | -1  | -1  | -1  | -1  | -1  | -1  | -1  |    |
| R      | 1   | 1   | 1   | -1  | -1  | -1  | <i>i</i> | <i>i</i> | <i>i</i> | <i>i</i> | <i>i</i> | <i>i</i> | <i>i</i> | <i>i</i> | <i>i</i> | <i>i</i> | - <i>i</i> | - <i>i</i> | - <i>i</i> | - <i>i</i> | - <i>i</i> | - <i>i</i> | - <i>i</i> | - <i>i</i> | 1   | 1   | 1   | 1   | 1   | 1   | -1  | -1  | -1  | -1  | -1  | -1  |    |
| Landau | A1  | A1  | A1  | B1  | B1  | B1  | E        | E        | E        | E        | E        | E        | E        | E        | E        | E        | E          | E          | E          | E          | E          | E          | E          | E          | E   | A2  | A2  | A2  | A2  | A2  | A2  | B2  | B2  | B2  | B2  | B2  | B2 |



$$S = 1, \text{ n}_{\text{occ.}} = \{1, 3, 0, 0\}$$

$$\left( \begin{array}{cccccccccccccccc} \text{State} & 823 & 824 & 825 & 826 & 827 & 828 & 829 & 830 & 831 & 832 & 833 & 834 \\ \text{Sz} & 1 & 0 & -1 & 1 & 0 & -1 & 1 & 0 & -1 & 1 & 0 & -1 \\ \text{Rx} & 1 & 1 & 1 & 1 & 1 & 1 & 0 & 0 & 0 & 0 & 0 & 0 \\ \text{Ry} & 1 & 1 & 1 & 1 & 1 & 1 & 0 & 0 & 0 & 0 & 0 & 0 \\ \text{R} & 1 & 1 & 1 & -1 & -1 & -1 & i & i & i & -i & -i & -i \\ \text{Landau} & \text{A1} & \text{A1} & \text{A1} & \text{B1} & \text{B1} & \text{B1} & \text{E} & \text{E} & \text{E} & \text{E} & \text{E} & \text{E} \end{array} \right)$$

$$\mathbf{S} = \mathbf{1}, \mathbf{n}_{\text{occ.}} = \{\mathbf{1}, \mathbf{2}, \mathbf{1}, \mathbf{0}\}$$

| State  | 835 | 836 | 837 | 838 | 839 | 840 | 841 | 842 | 843 | 844 | 845 | 846 | 847 | 848 | 849 | 850 | 851 | 852 | 853 | 854 | 855 | 856 | 857  | 858  | 859  | 860  | 861  | 862  | 863  | 864  | 865 | 866 | 867 | 868 | 869 | 870 |    |
|--------|-----|-----|-----|-----|-----|-----|-----|-----|-----|-----|-----|-----|-----|-----|-----|-----|-----|-----|-----|-----|-----|-----|------|------|------|------|------|------|------|------|-----|-----|-----|-----|-----|-----|----|
| Sz     | 1   | 0   | -1  | 1   | 0   | -1  | 1   | 0   | -1  | 1   | 0   | -1  | 1   | 0   | -1  | 1   | 0   | -1  | 1   | 0   | -1  | 1   | 0    | -1   | 1    | 0    | -1   | 1    | 0    | -1   | 1   | 0   | -1  | 1   | 0   | -1  |    |
| Rx     | 1   | 1   | 1   | 1   | 1   | 1   | 1   | 1   | 1   | 1   | 1   | 1   | 0   | 0   | 0   | 0   | 0   | 0   | 0   | 0   | 0   | 0   | 0    | 0    | 0    | 0    | 0    | 0    | 0    | 0    | -1  | -1  | -1  | -1  | -1  | -1  |    |
| Ry     | 1   | 1   | 1   | 1   | 1   | 1   | 1   | 1   | 1   | 1   | 1   | 1   | 0   | 0   | 0   | 0   | 0   | 0   | 0   | 0   | 0   | 0   | 0    | 0    | 0    | 0    | 0    | 0    | 0    | 0    | 0   | -1  | -1  | -1  | -1  | -1  | -1 |
| R      | 1   | 1   | 1   | 1   | 1   | 1   | -1  | -1  | -1  | -1  | -1  | -1  | $i$ | $i$ | $i$ | $i$ | $i$ | $i$ | $i$ | $i$ | $i$ | $i$ | $-i$ | $-i$ | $-i$ | $-i$ | $-i$ | $-i$ | $-i$ | $-i$ | 1   | 1   | 1   | -1  | -1  | -1  |    |
| Landau | A1  | A1  | A1  | A1  | A1  | A1  | B1  | B1  | B1  | B1  | B1  | B1  | E   | E   | E   | E   | E   | E   | E   | E   | E   | E   | E    | E    | E    | E    | E    | E    | E    | E    | A2  | A2  | A2  | B2  | B2  | B2  |    |

$$\mathbf{S} = \mathbf{1}, \mathbf{n}_{\text{occ.}} = \{\mathbf{1}, \mathbf{2}, \mathbf{0}, \mathbf{1}\}$$

| State  | 871 | 872 | 873 | 874 | 875 | 876 | 877 | 878 | 879 | 880 | 881 | 882 | 883 | 884 | 885 | 886 | 887 | 888 | 889 | 890 | 891 | 892  | 893  | 894  | 895  | 896  | 897  | 898  | 899  | 900 | 901 | 902 | 903 | 904 | 905 | 906 |
|--------|-----|-----|-----|-----|-----|-----|-----|-----|-----|-----|-----|-----|-----|-----|-----|-----|-----|-----|-----|-----|-----|------|------|------|------|------|------|------|------|-----|-----|-----|-----|-----|-----|-----|
| Sz     | 1   | 0   | -1  | 1   | 0   | -1  | 1   | 0   | -1  | 1   | 0   | -1  | 1   | 0   | -1  | 1   | 0   | -1  | 1   | 0   | -1  | 1    | 0    | -1   | 1    | 0    | -1   | 1    | 0    | -1  | 1   | 0   | -1  | 1   | 0   | -1  |
| Rx     | 1   | 1   | 1   | 1   | 1   | 1   | 1   | 1   | 1   | 1   | 1   | 1   | 0   | 0   | 0   | 0   | 0   | 0   | 0   | 0   | 0   | 0    | 0    | 0    | 0    | 0    | 0    | 0    | 0    | 0   | -1  | -1  | -1  | -1  | -1  | -1  |
| Ry     | 1   | 1   | 1   | 1   | 1   | 1   | 1   | 1   | 1   | 1   | 1   | 1   | 0   | 0   | 0   | 0   | 0   | 0   | 0   | 0   | 0   | 0    | 0    | 0    | 0    | 0    | 0    | 0    | 0    | 0   | -1  | -1  | -1  | -1  | -1  | -1  |
| R      | 1   | 1   | 1   | 1   | 1   | 1   | -1  | -1  | -1  | -1  | -1  | -1  | $i$ | $i$ | $i$ | $i$ | $i$ | $i$ | $i$ | $i$ | $i$ | $-i$ | $-i$ | $-i$ | $-i$ | $-i$ | $-i$ | $-i$ | $-i$ | 1   | 1   | 1   | -1  | -1  | -1  |     |
| Landau | A1  | A1  | A1  | A1  | A1  | A1  | B1  | B1  | B1  | B1  | B1  | B1  | E   | E   | E   | E   | E   | E   | E   | E   | E   | E    | E    | E    | E    | E    | E    | E    | E    | A2  | A2  | A2  | B2  | B2  | B2  |     |

$$\mathbf{S} = \mathbf{1}, \mathbf{n}_{\text{occ.}} = \{\mathbf{1}, \mathbf{1}, \mathbf{2}, \mathbf{0}\}$$

| State  | 907 | 908 | 909 | 910 | 911 | 912 | 913 | 914 | 915 | 916 | 917 | 918 | 919      | 920      | 921      | 922      | 923      | 924      | 925      | 926      | 927      | 928      | 929        | 930        | 931        | 932        | 933        | 934        | 935        | 936        | 937 | 938 | 939 | 940 | 941 | 942 |
|--------|-----|-----|-----|-----|-----|-----|-----|-----|-----|-----|-----|-----|----------|----------|----------|----------|----------|----------|----------|----------|----------|----------|------------|------------|------------|------------|------------|------------|------------|------------|-----|-----|-----|-----|-----|-----|
| Sz     | 1   | 0   | -1  | 1   | 0   | -1  | 1   | 0   | -1  | 1   | 0   | -1  | 1        | 0        | -1       | 1        | 0        | -1       | 1        | 0        | -1       | 1        | 0          | -1         | 1          | 0          | -1         | 1          | 0          | -1         | 1   | 0   | -1  | 1   | 0   | -1  |
| Rx     | 1   | 1   | 1   | 1   | 1   | 1   | 1   | 1   | 1   | 1   | 1   | 1   | 0        | 0        | 0        | 0        | 0        | 0        | 0        | 0        | 0        | 0        | 0          | 0          | 0          | 0          | 0          | 0          | 0          | 0          | -1  | -1  | -1  | -1  | -1  | -1  |
| Ry     | 1   | 1   | 1   | 1   | 1   | 1   | 1   | 1   | 1   | 1   | 1   | 1   | 0        | 0        | 0        | 0        | 0        | 0        | 0        | 0        | 0        | 0        | 0          | 0          | 0          | 0          | 0          | 0          | 0          | 0          | -1  | -1  | -1  | -1  | -1  | -1  |
| R      | 1   | 1   | 1   | 1   | 1   | 1   | -1  | -1  | -1  | -1  | -1  | -1  | <i>i</i> | <i>i</i> | <i>i</i> | <i>i</i> | <i>i</i> | <i>i</i> | <i>i</i> | <i>i</i> | <i>i</i> | <i>i</i> | - <i>i</i> | - <i>i</i> | - <i>i</i> | - <i>i</i> | - <i>i</i> | - <i>i</i> | - <i>i</i> | - <i>i</i> | 1   | 1   | 1   | -1  | -1  | -1  |
| Landau | A1  | A1  | A1  | A1  | A1  | A1  | B1  | B1  | B1  | B1  | B1  | B1  | E        | E        | E        | E        | E        | E        | E        | E        | E        | E        | E          | E          | E          | E          | E          | E          | E          | E          | A2  | A2  | A2  | B2  | B2  | B2  |

[illegible]



$$\mathbf{S} = \mathbf{1}, \mathbf{n}_{\text{occ.}} = \{\mathbf{1}, \mathbf{1}, \mathbf{0}, \mathbf{2}\}$$

| State  | 1015 | 1016 | 1017 | 1018 | 1019 | 1020 | 1021 | 1022 | 1023 | 1024 | 1025 | 1026 | 1027     | 1028     | 1029     | 1030     | 1031     | 1032     | 1033     | 1034     | 1035     | 1036     | 1037     | 1038       | 1039       | 1040       | 1041       | 1042       | 1043       | 1044       | 1045       | 1046 | 1047 | 1048 | 1049 | 1050 |    |    |
|--------|------|------|------|------|------|------|------|------|------|------|------|------|----------|----------|----------|----------|----------|----------|----------|----------|----------|----------|----------|------------|------------|------------|------------|------------|------------|------------|------------|------|------|------|------|------|----|----|
| Sz     | 1    | 0    | -1   | 1    | 0    | -1   | 1    | 0    | -1   | 1    | 0    | -1   | 1        | 0        | -1       | 1        | 0        | -1       | 1        | 0        | -1       | 1        | 0        | -1         | 1          | 0          | -1         | 1          | 0          | -1         | 1          | 0    | -1   | 1    | 0    | -1   |    |    |
| Rx     | 1    | 1    | 1    | 1    | 1    | 1    | 1    | 1    | 1    | 1    | 1    | 1    | 1        | 0        | 0        | 0        | 0        | 0        | 0        | 0        | 0        | 0        | 0        | 0          | 0          | 0          | 0          | 0          | 0          | 0          | 0          | -1   | -1   | -1   | -1   | -1   | -1 |    |
| Ry     | 1    | 1    | 1    | 1    | 1    | 1    | 1    | 1    | 1    | 1    | 1    | 1    | 1        | 0        | 0        | 0        | 0        | 0        | 0        | 0        | 0        | 0        | 0        | 0          | 0          | 0          | 0          | 0          | 0          | 0          | 0          | 0    | -1   | -1   | -1   | -1   | -1 | -1 |
| R      | 1    | 1    | 1    | 1    | 1    | 1    | -1   | -1   | -1   | -1   | -1   | -1   | <i>i</i> | <i>i</i> | <i>i</i> | <i>i</i> | <i>i</i> | <i>i</i> | <i>i</i> | <i>i</i> | <i>i</i> | <i>i</i> | <i>i</i> | - <i>i</i> | - <i>i</i> | - <i>i</i> | - <i>i</i> | - <i>i</i> | - <i>i</i> | - <i>i</i> | - <i>i</i> | 1    | 1    | 1    | -1   | -1   | -1 |    |
| Landau | A1   | A1   | A1   | A1   | A1   | A1   | B1   | B1   | B1   | B1   | B1   | B1   | B1       | E        | E        | E        | E        | E        | E        | E        | E        | E        | E        | E          | E          | E          | E          | E          | E          | E          | E          | E    | A2   | A2   | A2   | B2   | B2 | B2 |

$$S = 1, \mathbf{n}_{\text{occ.}} = \{1, 0, 3, 0\}$$

$$\left( \begin{array}{cccccccccccccc} \text{State} & 1051 & 1052 & 1053 & 1054 & 1055 & 1056 & 1057 & 1058 & 1059 & 1060 & 1061 & 1062 \\ \text{Sz} & 1 & 0 & -1 & 1 & 0 & -1 & 1 & 0 & -1 & 1 & 0 & -1 \\ \text{Rx} & 1 & 1 & 1 & 1 & 1 & 1 & 0 & 0 & 0 & 0 & 0 & 0 \\ \text{Ry} & 1 & 1 & 1 & 1 & 1 & 1 & 0 & 0 & 0 & 0 & 0 & 0 \\ \text{R} & 1 & 1 & 1 & -1 & -1 & -1 & i & i & i & -i & -i & -i \\ \text{Landau} & \text{A1} & \text{A1} & \text{A1} & \text{B1} & \text{B1} & \text{B1} & \text{E} & \text{E} & \text{E} & \text{E} & \text{E} & \text{E} \end{array} \right)$$

$$\mathbf{S} = \mathbf{1}, \mathbf{n}_{\text{occ.}} = \{\mathbf{1}, \mathbf{0}, \mathbf{2}, \mathbf{1}\}$$

| State  | 1063 | 1064 | 1065 | 1066 | 1067 | 1068 | 1069 | 1070 | 1071 | 1072 | 1073 | 1074 | 1075 | 1076 | 1077 | 1078 | 1079 | 1080 | 1081 | 1082 | 1083 | 1084 | 1085 | 1086 | 1087 | 1088 | 1089 | 1090 | 1091 | 1092 | 1093 | 1094 | 1095 | 1096 | 1097 | 1098 |    |
|--------|------|------|------|------|------|------|------|------|------|------|------|------|------|------|------|------|------|------|------|------|------|------|------|------|------|------|------|------|------|------|------|------|------|------|------|------|----|
| Sz     | 1    | 0    | -1   | 1    | 0    | -1   | 1    | 0    | -1   | 1    | 0    | -1   | 1    | 0    | -1   | 1    | 0    | -1   | 1    | 0    | -1   | 1    | 0    | -1   | 1    | 0    | -1   | 1    | 0    | -1   | 1    | 0    | -1   | 1    | 0    | -1   |    |
| Rx     | 1    | 1    | 1    | 1    | 1    | 1    | 1    | 1    | 1    | 1    | 1    | 1    | 0    | 0    | 0    | 0    | 0    | 0    | 0    | 0    | 0    | 0    | 0    | 0    | 0    | 0    | 0    | 0    | 0    | 0    | 0    | -1   | -1   | -1   | -1   | -1   |    |
| Ry     | 1    | 1    | 1    | 1    | 1    | 1    | 1    | 1    | 1    | 1    | 1    | 1    | 0    | 0    | 0    | 0    | 0    | 0    | 0    | 0    | 0    | 0    | 0    | 0    | 0    | 0    | 0    | 0    | 0    | 0    | 0    | -1   | -1   | -1   | -1   | -1   |    |
| R      | 1    | 1    | 1    | 1    | 1    | 1    | 1    | -1   | -1   | -1   | -1   | -1   | i    | i    | i    | i    | i    | i    | i    | i    | i    | i    | -i   | -i   | -i   | -i   | -i   | -i   | -i   | -i   | 1    | 1    | 1    | -1   | -1   | -1   |    |
| Landau | A1   | A1   | A1   | A1   | A1   | A1   | B1   | B1   | B1   | B1   | B1   | B1   | E    | E    | E    | E    | E    | E    | E    | E    | E    | E    | E    | E    | E    | E    | E    | E    | E    | E    | E    | A2   | A2   | A2   | B2   | B2   | B2 |

$$\mathbf{S} = \mathbf{1}, \mathbf{n}_{\text{occ.}} = \{\mathbf{1}, \mathbf{0}, \mathbf{1}, \mathbf{2}\}$$

| State  | 1099 | 1100 | 1101 | 1102 | 1103 | 1104 | 1105 | 1106 | 1107 | 1108 | 1109 | 1110 | 1111     | 1112     | 1113     | 1114     | 1115     | 1116     | 1117     | 1118     | 1119     | 1120     | 1121     | 1122       | 1123       | 1124       | 1125       | 1126       | 1127       | 1128       | 1129 | 1130 | 1131 | 1132 | 1133 | 1134 |    |
|--------|------|------|------|------|------|------|------|------|------|------|------|------|----------|----------|----------|----------|----------|----------|----------|----------|----------|----------|----------|------------|------------|------------|------------|------------|------------|------------|------|------|------|------|------|------|----|
| Sz     | 1    | 0    | -1   | 1    | 0    | -1   | 1    | 0    | -1   | 1    | 0    | -1   | 1        | 0        | -1       | 1        | 0        | -1       | 1        | 0        | -1       | 1        | 0        | -1         | 1          | 0          | -1         | 1          | 0          | -1         | 1    | 0    | -1   | 1    | 0    | -1   |    |
| Rx     | 1    | 1    | 1    | 1    | 1    | 1    | 1    | 1    | 1    | 1    | 1    | 1    | 0        | 0        | 0        | 0        | 0        | 0        | 0        | 0        | 0        | 0        | 0        | 0          | 0          | 0          | 0          | 0          | 0          | 0          | 0    | -1   | -1   | -1   | -1   | -1   | -1 |
| Ry     | 1    | 1    | 1    | 1    | 1    | 1    | 1    | 1    | 1    | 1    | 1    | 1    | 0        | 0        | 0        | 0        | 0        | 0        | 0        | 0        | 0        | 0        | 0        | 0          | 0          | 0          | 0          | 0          | 0          | 0          | 0    | -1   | -1   | -1   | -1   | -1   | -1 |
| R      | 1    | 1    | 1    | 1    | 1    | 1    | -1   | -1   | -1   | -1   | -1   | -1   | <i>i</i> | <i>i</i> | <i>i</i> | <i>i</i> | <i>i</i> | <i>i</i> | <i>i</i> | <i>i</i> | <i>i</i> | <i>i</i> | <i>i</i> | - <i>i</i> | - <i>i</i> | - <i>i</i> | - <i>i</i> | - <i>i</i> | - <i>i</i> | - <i>i</i> | 1    | 1    | 1    | -1   | -1   | -1   |    |
| Landau | A1   | A1   | A1   | A1   | A1   | A1   | B1   | B1   | B1   | B1   | B1   | B1   | E        | E        | E        | E        | E        | E        | E        | E        | E        | E        | E        | E          | E          | E          | E          | E          | E          | E          | A2   | A2   | A2   | B2   | B2   | B2   |    |

$$\mathbf{S} = \mathbf{1}, \mathbf{n}_{\text{occ.}} = \{\mathbf{1}, \mathbf{0}, \mathbf{0}, \mathbf{3}\}$$

| State  | 1135 | 1136 | 1137 | 1138 | 1139 | 1140 | 1141 | 1142 | 1143 | 1144 | 1145 | 1146 |
|--------|------|------|------|------|------|------|------|------|------|------|------|------|
| Sz     | 1    | 0    | -1   | 1    | 0    | -1   | 1    | 0    | -1   | 1    | 0    | -1   |
| Rx     | 1    | 1    | 1    | 1    | 1    | 1    | 0    | 0    | 0    | 0    | 0    | 0    |
| Ry     | 1    | 1    | 1    | 1    | 1    | 1    | 0    | 0    | 0    | 0    | 0    | 0    |
| R      | 1    | 1    | 1    | -1   | -1   | -1   | $i$  | $i$  | $i$  | $-i$ | $-i$ | $-i$ |
| Landau | A1   | A1   | A1   | B1   | B1   | B1   | E    | E    | E    | E    | E    | E    |

$$\mathbf{S} = \mathbf{0}, \mathbf{n}_{\text{occ.}} = \{4, \mathbf{0}, \mathbf{0}, \mathbf{0}\}$$

$$\left( \begin{array}{cccc} \text{State} & 1147 & 1148 & 1149 \\ \text{Sz} & 0 & 0 & 0 \\ \text{Rx} & 1 & 1 & -1 \\ \text{Ry} & 1 & 1 & -1 \\ \text{R} & 1 & 1 & -1 \\ \text{Landau} & \text{A1} & \text{A1} & \text{B2} \end{array} \right)$$

$$\mathbf{S} = \mathbf{0}, \mathbf{n}_{\text{occ.}} = \{\mathbf{3}, \mathbf{1}, \mathbf{0}, \mathbf{0}\}$$

$$\left( \begin{array}{ccccc} \text{State} & 1150 & 1151 & 1152 & 1153 \\ \text{Sz} & 0 & 0 & 0 & 0 \\ \text{Rx} & 0 & 0 & -1 & -1 \\ \text{Ry} & 0 & 0 & -1 & -1 \\ \text{R} & i & -i & 1 & -1 \\ \text{Landau} & \text{E} & \text{E} & \text{A2} & \text{B2} \end{array} \right)$$

$$\mathbf{S} = \mathbf{0}, \mathbf{n}_{\text{occ.}} = \{\mathbf{3}, \mathbf{0}, \mathbf{1}, \mathbf{0}\}$$

$$\left( \begin{array}{ccccc} \text{State} & 1154 & 1155 & 1156 & 1157 \\ \text{Sz} & 0 & 0 & 0 & 0 \\ \text{Rx} & 0 & 0 & -1 & -1 \\ \text{Ry} & 0 & 0 & -1 & -1 \\ \text{R} & i & -i & 1 & -1 \\ \text{Landau} & \text{E} & \text{E} & \text{A2} & \text{B2} \end{array} \right)$$



$$\mathbf{S} = \mathbf{0}, \mathbf{n}_{\text{occ.}} = \{\mathbf{3}, \mathbf{0}, \mathbf{0}, \mathbf{1}\}$$

$$\left( \begin{array}{ccccc} \text{State} & 1158 & 1159 & 1160 & 1161 \\ \text{Sz} & 0 & 0 & 0 & 0 \\ \text{Rx} & 0 & 0 & -1 & -1 \\ \text{Ry} & 0 & 0 & -1 & -1 \\ \text{R} & i & -i & 1 & -1 \\ \text{Landau} & \text{E} & \text{E} & \text{A2} & \text{B2} \end{array} \right)$$

$$\mathbf{S} = \mathbf{0}, \mathbf{n}_{\text{occ.}} = \{\mathbf{2}, \mathbf{2}, \mathbf{0}, \mathbf{0}\}$$

| State  | 1162 | 1163 | 1164 | 1165 | 1166 | 1167 |
|--------|------|------|------|------|------|------|
| Sz     | 0    | 0    | 0    | 0    | 0    | 0    |
| Rx     | 1    | 1    | 1    | 0    | 0    | -1   |
| Ry     | 1    | 1    | 1    | 0    | 0    | -1   |
| R      | 1    | 1    | -1   | $i$  | $-i$ | -1   |
| Landau | A1   | A1   | B1   | E    | E    | B2   |

$$\mathbf{S} = \mathbf{0}, \mathbf{n}_{\text{occ.}} = \{\mathbf{2}, \mathbf{1}, \mathbf{1}, \mathbf{0}\}$$

| State  | 1168 | 1169 | 1170 | 1171 | 1172 | 1173 | 1174 | 1175 | 1176 | 1177 | 1178 | 1179 |
|--------|------|------|------|------|------|------|------|------|------|------|------|------|
| Sz     | 0    | 0    | 0    | 0    | 0    | 0    | 0    | 0    | 0    | 0    | 0    | 0    |
| Rx     | 1    | 1    | 1    | 1    | 0    | 0    | 0    | 0    | 0    | 0    | -1   | -1   |
| Ry     | 1    | 1    | 1    | 1    | 0    | 0    | 0    | 0    | 0    | 0    | -1   | -1   |
| R      | 1    | 1    | -1   | -1   | $i$  | $i$  | $i$  | $-i$ | $-i$ | $-i$ | 1    | -1   |
| Landau | A1   | A1   | B1   | B1   | E    | E    | E    | E    | E    | E    | A2   | B2   |

$$\mathbf{S} = \mathbf{0}, \mathbf{n}_{\text{occ.}} = \{\mathbf{2}, \mathbf{1}, \mathbf{0}, \mathbf{1}\}$$

| State  | 1180 | 1181 | 1182 | 1183 | 1184 | 1185 | 1186 | 1187 | 1188 | 1189 | 1190 | 1191 |
|--------|------|------|------|------|------|------|------|------|------|------|------|------|
| Sz     | 0    | 0    | 0    | 0    | 0    | 0    | 0    | 0    | 0    | 0    | 0    | 0    |
| Rx     | 1    | 1    | 1    | 1    | 0    | 0    | 0    | 0    | 0    | 0    | -1   | -1   |
| Ry     | 1    | 1    | 1    | 1    | 0    | 0    | 0    | 0    | 0    | 0    | -1   | -1   |
| R      | 1    | 1    | -1   | -1   | $i$  | $i$  | $i$  | $-i$ | $-i$ | $-i$ | 1    | -1   |
| Landau | A1   | A1   | B1   | B1   | E    | E    | E    | E    | E    | E    | A2   | B2   |

$$\mathbf{S} = \mathbf{0}, \mathbf{n}_{\text{occ.}} = \{\mathbf{2}, \mathbf{0}, \mathbf{2}, \mathbf{0}\}$$

$$\left( \begin{array}{cccccc} \text{State} & 1192 & 1193 & 1194 & 1195 & 1196 & 1197 \\ \text{Sz} & 0 & 0 & 0 & 0 & 0 & 0 \\ \text{Rx} & 1 & 1 & 1 & 0 & 0 & -1 \\ \text{Ry} & 1 & 1 & 1 & 0 & 0 & -1 \\ \text{R} & 1 & 1 & -1 & i & -i & -1 \\ \text{Landau} & \text{A1} & \text{A1} & \text{B1} & \text{E} & \text{E} & \text{B2} \end{array} \right)$$

$$\mathbf{S} = \mathbf{0}, \mathbf{n}_{\text{occ.}} = \{\mathbf{2}, \mathbf{0}, \mathbf{1}, \mathbf{1}\}$$

| State  | 1198 | 1199 | 1200 | 1201 | 1202 | 1203 | 1204 | 1205 | 1206 | 1207 | 1208 | 1209 |
|--------|------|------|------|------|------|------|------|------|------|------|------|------|
| Sz     | 0    | 0    | 0    | 0    | 0    | 0    | 0    | 0    | 0    | 0    | 0    | 0    |
| Rx     | 1    | 1    | 1    | 1    | 0    | 0    | 0    | 0    | 0    | 0    | -1   | -1   |
| Ry     | 1    | 1    | 1    | 1    | 0    | 0    | 0    | 0    | 0    | 0    | -1   | -1   |
| R      | 1    | 1    | -1   | -1   | $i$  | $i$  | $i$  | $-i$ | $-i$ | $-i$ | 1    | -1   |
| Landau | A1   | A1   | B1   | B1   | E    | E    | E    | E    | E    | E    | A2   | B2   |

$$\mathbf{S} = \mathbf{0}, \mathbf{n}_{\text{occ.}} = \{\mathbf{2}, \mathbf{0}, \mathbf{0}, \mathbf{2}\}$$

| State  | 1210 | 1211 | 1212 | 1213 | 1214 | 1215 |
|--------|------|------|------|------|------|------|
| Sz     | 0    | 0    | 0    | 0    | 0    | 0    |
| Rx     | 1    | 1    | 1    | 0    | 0    | -1   |
| Ry     | 1    | 1    | 1    | 0    | 0    | -1   |
| R      | 1    | 1    | -1   | $i$  | $-i$ | -1   |
| Landau | A1   | A1   | B1   | E    | E    | B2   |

$$\mathbf{S} = \mathbf{0}, \text{ n}_{\text{occ.}} = \{\mathbf{0}, 4, \mathbf{0}, \mathbf{0}\}$$

$$\left( \begin{array}{cc} \text{State} & 1216 \\ \text{Sz} & 0 \\ \text{Rx} & 1 \\ \text{Ry} & 1 \\ \text{R} & 1 \\ \text{Landau} & \text{A1} \end{array} \right)$$



$$\mathbf{S} = \mathbf{0}, \mathbf{n}_{\text{occ.}} = \{\mathbf{0}, \mathbf{3}, \mathbf{1}, \mathbf{0}\}$$

$$\left( \begin{array}{ccccc} \text{State} & 1217 & 1218 & 1219 & 1220 \\ \text{Sz} & 0 & 0 & 0 & 0 \\ \text{Rx} & 1 & 1 & 0 & 0 \\ \text{Ry} & 1 & 1 & 0 & 0 \\ \text{R} & 1 & -1 & i & -i \\ \text{Landau} & \text{A1} & \text{B1} & \text{E} & \text{E} \end{array} \right)$$

$$\mathbf{S} = \mathbf{0}, \mathbf{n}_{\text{occ.}} = \{\mathbf{0}, \mathbf{3}, \mathbf{0}, \mathbf{1}\}$$

$$\left( \begin{array}{ccccc} \text{State} & 1221 & 1222 & 1223 & 1224 \\ \text{Sz} & 0 & 0 & 0 & 0 \\ \text{Rx} & 1 & 1 & 0 & 0 \\ \text{Ry} & 1 & 1 & 0 & 0 \\ \text{R} & 1 & -1 & i & -i \\ \text{Landau} & \text{A1} & \text{B1} & \text{E} & \text{E} \end{array} \right)$$

$$\mathbf{S} = \mathbf{0}, \mathbf{n}_{\text{occ.}} = \{\mathbf{0}, \mathbf{2}, \mathbf{2}, \mathbf{0}\}$$

| State  | 1225 | 1226 | 1227 | 1228 | 1229 | 1230 |
|--------|------|------|------|------|------|------|
| Sz     | 0    | 0    | 0    | 0    | 0    | 0    |
| Rx     | 1    | 1    | 1    | 0    | 0    | -1   |
| Ry     | 1    | 1    | 1    | 0    | 0    | -1   |
| R      | 1    | 1    | -1   | $i$  | $-i$ | -1   |
| Landau | A1   | A1   | B1   | E    | E    | B2   |

$$\mathbf{S} = \mathbf{0}, \mathbf{n}_{\text{occ.}} = \{0, 2, 1, 1\}$$

| State  | 1231 | 1232 | 1233 | 1234 | 1235 | 1236 | 1237 | 1238 | 1239 | 1240 | 1241 | 1242 |
|--------|------|------|------|------|------|------|------|------|------|------|------|------|
| Sz     | 0    | 0    | 0    | 0    | 0    | 0    | 0    | 0    | 0    | 0    | 0    | 0    |
| Rx     | 1    | 1    | 1    | 1    | 0    | 0    | 0    | 0    | 0    | 0    | -1   | -1   |
| Ry     | 1    | 1    | 1    | 1    | 0    | 0    | 0    | 0    | 0    | 0    | -1   | -1   |
| R      | 1    | 1    | -1   | -1   | $i$  | $i$  | $i$  | $-i$ | $-i$ | $-i$ | 1    | -1   |
| Landau | A1   | A1   | B1   | B1   | E    | E    | E    | E    | E    | E    | A2   | B2   |

$$\mathbf{S} = \mathbf{0}, \mathbf{n}_{\text{occ.}} = \{\mathbf{0}, \mathbf{2}, \mathbf{0}, \mathbf{2}\}$$

$$\left( \begin{array}{cccccc} \text{State} & 1243 & 1244 & 1245 & 1246 & 1247 & 1248 \\ \text{Sz} & 0 & 0 & 0 & 0 & 0 & 0 \\ \text{Rx} & 1 & 1 & 1 & 0 & 0 & -1 \\ \text{Ry} & 1 & 1 & 1 & 0 & 0 & -1 \\ \text{R} & 1 & 1 & -1 & i & -i & -1 \\ \text{Landau} & \text{A1} & \text{A1} & \text{B1} & \text{E} & \text{E} & \text{B2} \end{array} \right)$$

$$\mathbf{S} = \mathbf{0}, \mathbf{n}_{\text{occ.}} = \{\mathbf{0}, \mathbf{1}, \mathbf{3}, \mathbf{0}\}$$

$$\left( \begin{array}{ccccc} \text{State} & 1249 & 1250 & 1251 & 1252 \\ \text{Sz} & 0 & 0 & 0 & 0 \\ \text{Rx} & 1 & 1 & 0 & 0 \\ \text{Ry} & 1 & 1 & 0 & 0 \\ \text{R} & 1 & -1 & i & -i \\ \text{Landau} & \text{A1} & \text{B1} & \text{E} & \text{E} \end{array} \right)$$

$$\mathbf{S} = \mathbf{0}, \mathbf{n}_{\text{occ.}} = \{0, 1, 2, 1\}$$

| State  | 1253 | 1254 | 1255 | 1256 | 1257 | 1258 | 1259 | 1260 | 1261 | 1262 | 1263 | 1264 |
|--------|------|------|------|------|------|------|------|------|------|------|------|------|
| Sz     | 0    | 0    | 0    | 0    | 0    | 0    | 0    | 0    | 0    | 0    | 0    | 0    |
| Rx     | 1    | 1    | 1    | 1    | 0    | 0    | 0    | 0    | 0    | 0    | -1   | -1   |
| Ry     | 1    | 1    | 1    | 1    | 0    | 0    | 0    | 0    | 0    | 0    | -1   | -1   |
| R      | 1    | 1    | -1   | -1   | $i$  | $i$  | $i$  | $-i$ | $-i$ | $-i$ | 1    | -1   |
| Landau | A1   | A1   | B1   | B1   | E    | E    | E    | E    | E    | E    | A2   | B2   |

$$\mathbf{S} = \mathbf{0}, \mathbf{n}_{\text{occ.}} = \{\mathbf{0}, \mathbf{1}, \mathbf{1}, \mathbf{2}\}$$

| State  | 1265 | 1266 | 1267 | 1268 | 1269 | 1270 | 1271 | 1272 | 1273 | 1274 | 1275 | 1276 |
|--------|------|------|------|------|------|------|------|------|------|------|------|------|
| Sz     | 0    | 0    | 0    | 0    | 0    | 0    | 0    | 0    | 0    | 0    | 0    | 0    |
| Rx     | 1    | 1    | 1    | 1    | 0    | 0    | 0    | 0    | 0    | 0    | -1   | -1   |
| Ry     | 1    | 1    | 1    | 1    | 0    | 0    | 0    | 0    | 0    | 0    | -1   | -1   |
| R      | 1    | 1    | -1   | -1   | $i$  | $i$  | $i$  | $-i$ | $-i$ | $-i$ | 1    | -1   |
| Landau | A1   | A1   | B1   | B1   | E    | E    | E    | E    | E    | E    | A2   | B2   |



$$\mathbf{S} = \mathbf{0}, \text{ n}_{\text{occ.}} = \{\mathbf{0}, \mathbf{0}, \mathbf{4}, \mathbf{0}\}$$

$$\left( \begin{array}{cc} \text{State} & 1277 \\ \text{Sz} & 0 \\ \text{Rx} & 1 \\ \text{Ry} & 1 \\ \text{R} & 1 \\ \text{Landau} & \text{A1} \end{array} \right)$$

$$\mathbf{S} = \mathbf{0}, \mathbf{n}_{\text{occ.}} = \{\mathbf{0}, \mathbf{1}, \mathbf{0}, \mathbf{3}\}$$

$$\left( \begin{array}{ccccc} \text{State} & 1278 & 1279 & 1280 & 1281 \\ \text{Sz} & 0 & 0 & 0 & 0 \\ \text{Rx} & 1 & 1 & 0 & 0 \\ \text{Ry} & 1 & 1 & 0 & 0 \\ \text{R} & 1 & -1 & i & -i \\ \text{Landau} & \text{A1} & \text{B1} & \text{E} & \text{E} \end{array} \right)$$

$$\mathbf{S} = \mathbf{0}, \mathbf{n}_{\text{occ.}} = \{\mathbf{0}, \mathbf{0}, \mathbf{3}, \mathbf{1}\}$$

$$\left( \begin{array}{ccccc} \text{State} & 1282 & 1283 & 1284 & 1285 \\ \text{Sz} & 0 & 0 & 0 & 0 \\ \text{Rx} & 1 & 1 & 0 & 0 \\ \text{Ry} & 1 & 1 & 0 & 0 \\ \text{R} & 1 & -1 & i & -i \\ \text{Landau} & \text{A1} & \text{B1} & \text{E} & \text{E} \end{array} \right)$$

$$\mathbf{S} = \mathbf{0}, \mathbf{n}_{\text{occ.}} = \{\mathbf{0}, \mathbf{0}, \mathbf{2}, \mathbf{2}\}$$

| State  | 1286 | 1287 | 1288 | 1289 | 1290 | 1291 |
|--------|------|------|------|------|------|------|
| Sz     | 0    | 0    | 0    | 0    | 0    | 0    |
| Rx     | 1    | 1    | 1    | 0    | 0    | -1   |
| Ry     | 1    | 1    | 1    | 0    | 0    | -1   |
| R      | 1    | 1    | -1   | $i$  | $-i$ | -1   |
| Landau | A1   | A1   | B1   | E    | E    | B2   |

$$\mathbf{S} = \mathbf{0}, \mathbf{n}_{\text{occ.}} = \{\mathbf{0}, \mathbf{0}, \mathbf{1}, \mathbf{3}\}$$

$$\left( \begin{array}{ccccc} \text{State} & 1292 & 1293 & 1294 & 1295 \\ \text{Sz} & 0 & 0 & 0 & 0 \\ \text{Rx} & 1 & 1 & 0 & 0 \\ \text{Ry} & 1 & 1 & 0 & 0 \\ \text{R} & 1 & -1 & i & -i \\ \text{Landau} & \text{A1} & \text{B1} & \text{E} & \text{E} \end{array} \right)$$

$$\mathbf{S} = \mathbf{0}, \text{ n}_{\text{occ.}} = \{\mathbf{0}, \mathbf{0}, \mathbf{0}, 4\}$$

$$\left( \begin{array}{cc} \text{State} & 1296 \\ \text{Sz} & 0 \\ \text{Rx} & 1 \\ \text{Ry} & 1 \\ \text{R} & 1 \\ \text{Landau} & \text{A1} \end{array} \right)$$

$$\mathbf{S} = \mathbf{2}, \mathbf{n}_{\text{occ.}} = \{4, \mathbf{0}, \mathbf{0}\}$$

$$\left( \begin{array}{ccccc} \text{State} & 1 & 2 & 3 & 4 & 5 \\ \text{Sz} & 2 & 1 & 0 & -1 & -2 \\ \text{Rx} & 1 & 1 & 1 & 1 & 1 \\ \text{Ry} & 1 & 1 & 1 & 1 & 1 \\ \text{R} & 1 & 1 & 1 & 1 & 1 \\ \text{Landau} & \text{A1} & \text{A1} & \text{A1} & \text{A1} & \text{A1} \end{array} \right)$$





$$S = 2, \text{ n}_{\text{occ.}} = \{3, 0, 1\}$$

[illegible]

$$\mathbf{S} = \mathbf{2}, \mathbf{n}_{\text{occ.}} = \{\mathbf{2}, \mathbf{2}, \mathbf{0}\}$$

| State  | 46 | 47 | 48 | 49 | 50 | 51 | 52 | 53 | 54 | 55 | 56 | 57 | 58 | 59 | 60 | 61  | 62  | 63  | 64  | 65  | 66   | 67   | 68   | 69   | 70   | 71 | 72 | 73 | 74 | 75 |
|--------|----|----|----|----|----|----|----|----|----|----|----|----|----|----|----|-----|-----|-----|-----|-----|------|------|------|------|------|----|----|----|----|----|
| Sz     | 2  | 1  | 0  | -1 | -2 | 2  | 1  | 0  | -1 | -2 | 2  | 1  | 0  | -1 | -2 | 2   | 1   | 0   | -1  | -2  | 2    | 1    | 0    | -1   | -2   | 2  | 1  | 0  | -1 | -2 |
| Rx     | 1  | 1  | 1  | 1  | 1  | 1  | 1  | 1  | 1  | 1  | 1  | 1  | 1  | 1  | 1  | 0   | 0   | 0   | 0   | 0   | 0    | 0    | 0    | 0    | 0    | -1 | -1 | -1 | -1 | -1 |
| Ry     | 1  | 1  | 1  | 1  | 1  | 1  | 1  | 1  | 1  | 1  | 1  | 1  | 1  | 1  | 1  | 0   | 0   | 0   | 0   | 0   | 0    | 0    | 0    | 0    | 0    | -1 | -1 | -1 | -1 | -1 |
| R      | 1  | 1  | 1  | 1  | 1  | 1  | 1  | 1  | 1  | 1  | -1 | -1 | -1 | -1 | -1 | $i$ | $i$ | $i$ | $i$ | $i$ | $-i$ | $-i$ | $-i$ | $-i$ | $-i$ | -1 | -1 | -1 | -1 | -1 |
| Landau | A1 | A1 | A1 | A1 | A1 | A1 | A1 | A1 | A1 | A1 | B1 | B1 | B1 | B1 | B1 | E   | E   | E   | E   | E   | E    | E    | E    | E    | E    | B2 | B2 | B2 | B2 | B2 |



$$\mathbf{S} = \mathbf{2}, \mathbf{n}_{\text{occ.}} = \{\mathbf{2}, \mathbf{0}, \mathbf{2}\}$$

| State  | 136 | 137 | 138 | 139 | 140 | 141 | 142 | 143 | 144 | 145 | 146 | 147 | 148 | 149 | 150 | 151 | 152 | 153 | 154 | 155 | 156  | 157  | 158  | 159  | 160  | 161 | 162 | 163 | 164 | 165 |
|--------|-----|-----|-----|-----|-----|-----|-----|-----|-----|-----|-----|-----|-----|-----|-----|-----|-----|-----|-----|-----|------|------|------|------|------|-----|-----|-----|-----|-----|
| Sz     | 2   | 1   | 0   | -1  | -2  | 2   | 1   | 0   | -1  | -2  | 2   | 1   | 0   | -1  | -2  | 2   | 1   | 0   | -1  | -2  | 2    | 1    | 0    | -1   | -2   | 2   | 1   | 0   | -1  | -2  |
| Rx     | 1   | 1   | 1   | 1   | 1   | 1   | 1   | 1   | 1   | 1   | 1   | 1   | 1   | 1   | 1   | 0   | 0   | 0   | 0   | 0   | 0    | 0    | 0    | 0    | 0    | 0   | -1  | -1  | -1  | -1  |
| Ry     | 1   | 1   | 1   | 1   | 1   | 1   | 1   | 1   | 1   | 1   | 1   | 1   | 1   | 1   | 1   | 0   | 0   | 0   | 0   | 0   | 0    | 0    | 0    | 0    | 0    | 0   | -1  | -1  | -1  | -1  |
| R      | 1   | 1   | 1   | 1   | 1   | 1   | 1   | 1   | 1   | 1   | -1  | -1  | -1  | -1  | -1  | $i$ | $i$ | $i$ | $i$ | $i$ | $-i$ | $-i$ | $-i$ | $-i$ | $-i$ | -1  | -1  | -1  | -1  | -1  |
| Landau | A1  | A1  | A1  | A1  | A1  | A1  | A1  | A1  | A1  | A1  | B1  | B1  | B1  | B1  | B1  | E   | E   | E   | E   | E   | E    | E    | E    | E    | E    | B2  | B2  | B2  | B2  | B2  |

$$S = 2, \text{ n}_{\text{occ.}} = \{1, 3, 0\}$$

[illegible]

$$\mathbf{S} = \mathbf{2}, \mathbf{n}_{occ.} = \{1, \mathbf{2}, 1\}$$



$$S = 2, \text{ n}_{\text{occ.}} = \{1, 0, 3\}$$

[illegible]



$$\mathbf{S} = \mathbf{2}, \mathbf{n}_{\text{occ.}} = \{\mathbf{0}, 4, \mathbf{0}\}$$

$$\left( \begin{array}{cccccc} \text{State} & 326 & 327 & 328 & 329 & 330 \\ \text{Sz} & 2 & 1 & 0 & -1 & -2 \\ \text{Rx} & 1 & 1 & 1 & 1 & 1 \\ \text{Ry} & 1 & 1 & 1 & 1 & 1 \\ \text{R} & 1 & 1 & 1 & 1 & 1 \\ \text{Landau} & \text{A1} & \text{A1} & \text{A1} & \text{A1} & \text{A1} \end{array} \right)$$

$$S = 2, \text{ n}_{\text{occ.}} = \{0, 3, 1\}$$

[illegible]

$$\mathbf{S} = \mathbf{2}, \mathbf{n}_{\text{occ.}} = \{\mathbf{0}, \mathbf{2}, \mathbf{2}\}$$

| State  | 351 | 352 | 353 | 354 | 355 | 356 | 357 | 358 | 359 | 360 | 361 | 362 | 363 | 364 | 365 | 366 | 367 | 368 | 369 | 370 | 371  | 372  | 373  | 374  | 375  | 376 | 377 | 378 | 379 | 380 |
|--------|-----|-----|-----|-----|-----|-----|-----|-----|-----|-----|-----|-----|-----|-----|-----|-----|-----|-----|-----|-----|------|------|------|------|------|-----|-----|-----|-----|-----|
| Sz     | 2   | 1   | 0   | -1  | -2  | 2   | 1   | 0   | -1  | -2  | 2   | 1   | 0   | -1  | -2  | 2   | 1   | 0   | -1  | -2  | 2    | 1    | 0    | -1   | -2   | 2   | 1   | 0   | -1  | -2  |
| Rx     | 1   | 1   | 1   | 1   | 1   | 1   | 1   | 1   | 1   | 1   | 1   | 1   | 1   | 1   | 1   | 0   | 0   | 0   | 0   | 0   | 0    | 0    | 0    | 0    | 0    | 0   | -1  | -1  | -1  | -1  |
| Ry     | 1   | 1   | 1   | 1   | 1   | 1   | 1   | 1   | 1   | 1   | 1   | 1   | 1   | 1   | 1   | 0   | 0   | 0   | 0   | 0   | 0    | 0    | 0    | 0    | 0    | 0   | -1  | -1  | -1  | -1  |
| R      | 1   | 1   | 1   | 1   | 1   | 1   | 1   | 1   | 1   | 1   | -1  | -1  | -1  | -1  | -1  | $i$ | $i$ | $i$ | $i$ | $i$ | $-i$ | $-i$ | $-i$ | $-i$ | $-i$ | -1  | -1  | -1  | -1  | -1  |
| Landau | A1  | A1  | A1  | A1  | A1  | A1  | A1  | A1  | A1  | A1  | B1  | B1  | B1  | B1  | B1  | E   | E   | E   | E   | E   | E    | E    | E    | E    | E    | E   | B2  | B2  | B2  | B2  |

$$S = 2, \text{ n}_{\text{occ.}} = \{0, 1, 3\}$$

[illegible]

$$\mathbf{S} = \mathbf{2}, \mathbf{n}_{\text{occ.}} = \{\mathbf{0}, \mathbf{0}, \mathbf{4}\}$$

$$\left( \begin{array}{cccccc} \text{State} & 401 & 402 & 403 & 404 & 405 \\ \text{Sz} & 2 & 1 & 0 & -1 & -2 \\ \text{Rx} & 1 & 1 & 1 & 1 & 1 \\ \text{Ry} & 1 & 1 & 1 & 1 & 1 \\ \text{R} & 1 & 1 & 1 & 1 & 1 \\ \text{Landau} & \text{A1} & \text{A1} & \text{A1} & \text{A1} & \text{A1} \end{array} \right)$$



$\mathbf{S} = \mathbf{1}, \mathbf{n}_{\text{occ.}} = \{\mathbf{3}, \mathbf{1}, \mathbf{0}\}$

|        |     |     |     |     |     |     |     |     |     |     |     |     |     |     |     |     |     |     |     |     |     |     |      |      |      |      |      |      |      |      |     |     |     |     |     |     |
|--------|-----|-----|-----|-----|-----|-----|-----|-----|-----|-----|-----|-----|-----|-----|-----|-----|-----|-----|-----|-----|-----|-----|------|------|------|------|------|------|------|------|-----|-----|-----|-----|-----|-----|
| State  | 415 | 416 | 417 | 418 | 419 | 420 | 421 | 422 | 423 | 424 | 425 | 426 | 427 | 428 | 429 | 430 | 431 | 432 | 433 | 434 | 435 | 436 | 437  | 438  | 439  | 440  | 441  | 442  | 443  | 444  | 445 | 446 | 447 | 448 | 449 | 450 |
| Sz     | 1   | 0   | -1  | 1   | 0   | -1  | 1   | 0   | -1  | 1   | 0   | -1  | 1   | 0   | -1  | 1   | 0   | -1  | 1   | 0   | -1  | 1   | 0    | -1   | 1    | 0    | -1   | 1    | 0    | -1   | 1   | 0   | -1  | 1   | 0   | -1  |
| Rx     | 1   | 1   | 1   | 1   | 1   | 1   | 1   | 1   | 1   | 1   | 1   | 1   | 0   | 0   | 0   | 0   | 0   | 0   | 0   | 0   | 0   | 0   | 0    | 0    | 0    | 0    | 0    | 0    | 0    | 0    | 0   | -1  | -1  | -1  | -1  | -1  |
| Ry     | 1   | 1   | 1   | 1   | 1   | 1   | 1   | 1   | 1   | 1   | 1   | 1   | 0   | 0   | 0   | 0   | 0   | 0   | 0   | 0   | 0   | 0   | 0    | 0    | 0    | 0    | 0    | 0    | 0    | 0    | 0   | -1  | -1  | -1  | -1  | -1  |
| R      | 1   | 1   | 1   | 1   | 1   | 1   | -1  | -1  | -1  | -1  | -1  | -1  | $i$ | $i$ | $i$ | $i$ | $i$ | $i$ | $i$ | $i$ | $i$ | $i$ | $-i$ | $-i$ | $-i$ | $-i$ | $-i$ | $-i$ | $-i$ | $-i$ | 1   | 1   | 1   | -1  | -1  | -1  |
| Landau | A1  | A1  | A1  | A1  | A1  | A1  | B1  | B1  | B1  | B1  | B1  | B1  | E   | E   | E   | E   | E   | E   | E   | E   | E   | E   | E    | E    | E    | E    | E    | E    | E    | E    | A2  | A2  | A2  | B2  | B2  | B2  |

$$\mathbf{S} = \mathbf{1}, \mathbf{n}_{\text{occ.}} = \{\mathbf{3}, \mathbf{0}, \mathbf{1}\}$$

|        |     |     |     |     |     |     |     |     |     |     |     |     |          |          |          |          |          |          |          |          |          |            |            |            |            |            |            |            |            |            |     |     |     |     |     |     |
|--------|-----|-----|-----|-----|-----|-----|-----|-----|-----|-----|-----|-----|----------|----------|----------|----------|----------|----------|----------|----------|----------|------------|------------|------------|------------|------------|------------|------------|------------|------------|-----|-----|-----|-----|-----|-----|
| State  | 451 | 452 | 453 | 454 | 455 | 456 | 457 | 458 | 459 | 460 | 461 | 462 | 463      | 464      | 465      | 466      | 467      | 468      | 469      | 470      | 471      | 472        | 473        | 474        | 475        | 476        | 477        | 478        | 479        | 480        | 481 | 482 | 483 | 484 | 485 | 486 |
| Sz     | 1   | 0   | -1  | 1   | 0   | -1  | 1   | 0   | -1  | 1   | 0   | -1  | 1        | 0        | -1       | 1        | 0        | -1       | 1        | 0        | -1       | 1          | 0          | -1         | 1          | 0          | -1         | 1          | 0          | -1         | 1   | 0   | -1  | 1   | 0   | -1  |
| Rx     | 1   | 1   | 1   | 1   | 1   | 1   | 1   | 1   | 1   | 1   | 1   | 1   | 0        | 0        | 0        | 0        | 0        | 0        | 0        | 0        | 0        | 0          | 0          | 0          | 0          | 0          | 0          | 0          | 0          | 0          | -1  | -1  | -1  | -1  | -1  | -1  |
| Ry     | 1   | 1   | 1   | 1   | 1   | 1   | 1   | 1   | 1   | 1   | 1   | 1   | 0        | 0        | 0        | 0        | 0        | 0        | 0        | 0        | 0        | 0          | 0          | 0          | 0          | 0          | 0          | 0          | 0          | 0          | -1  | -1  | -1  | -1  | -1  | -1  |
| R      | 1   | 1   | 1   | 1   | 1   | 1   | -1  | -1  | -1  | -1  | -1  | -1  | <i>i</i> | <i>i</i> | <i>i</i> | <i>i</i> | <i>i</i> | <i>i</i> | <i>i</i> | <i>i</i> | <i>i</i> | - <i>i</i> | - <i>i</i> | - <i>i</i> | - <i>i</i> | - <i>i</i> | - <i>i</i> | - <i>i</i> | - <i>i</i> | - <i>i</i> | 1   | 1   | 1   | -1  | -1  | -1  |
| Landau | A1  | A1  | A1  | A1  | A1  | A1  | B1  | B1  | B1  | B1  | B1  | B1  | E        | E        | E        | E        | E        | E        | E        | E        | E        | E          | E          | E          | E          | E          | E          | E          | E          | E          | A2  | A2  | A2  | B2  | B2  | B2  |



$$\mathbf{S} = \mathbf{1}, \mathbf{n}_{\text{occ.}} = \{\mathbf{2}, \mathbf{2}, \mathbf{0}\}$$

|        |     |     |     |     |     |     |     |     |     |     |     |     |     |     |     |     |     |     |     |     |     |     |     |     |     |     |     |     |     |     |     |     |     |     |     |     |     |     |     |     |     |     |     |     |     |     |     |     |     |     |     |     |     |     |
|--------|-----|-----|-----|-----|-----|-----|-----|-----|-----|-----|-----|-----|-----|-----|-----|-----|-----|-----|-----|-----|-----|-----|-----|-----|-----|-----|-----|-----|-----|-----|-----|-----|-----|-----|-----|-----|-----|-----|-----|-----|-----|-----|-----|-----|-----|-----|-----|-----|-----|-----|-----|-----|-----|-----|
| State  | 487 | 488 | 489 | 490 | 491 | 492 | 493 | 494 | 495 | 496 | 497 | 498 | 499 | 500 | 501 | 502 | 503 | 504 | 505 | 506 | 507 | 508 | 509 | 510 | 511 | 512 | 513 | 514 | 515 | 516 | 517 | 518 | 519 | 520 | 521 | 522 | 523 | 524 | 525 | 526 | 527 | 528 | 529 | 530 | 531 | 532 | 533 | 534 | 535 | 536 | 537 | 538 | 539 | 540 |
| Sz     | 1   | 0   | -1  | 1   | 0   | -1  | 1   | 0   | -1  | 1   | 0   | -1  | 1   | 0   | -1  | 1   | 0   | -1  | 1   | 0   | -1  | 1   | 0   | -1  | 1   | 0   | -1  | 1   | 0   | -1  | 1   | 0   | -1  | 1   | 0   | -1  | 1   | 0   | -1  | 1   | 0   | -1  | 1   | 0   | -1  | 1   | 0   | -1  | 1   | 0   | -1  |     |     |     |
| Rx     | 1   | 1   | 1   | 1   | 1   | 1   | 1   | 1   | 1   | 1   | 1   | 1   | 1   | 1   | 1   | 0   | 0   | 0   | 0   | 0   | 0   | 0   | 0   | 0   | 0   | 0   | 0   | 0   | 0   | 0   | 0   | 0   | 0   | 0   | 0   | 0   | 0   | 0   | 0   | 0   | 0   | 0   | 0   | -1  | -1  | -1  | -1  | -1  | -1  | -1  | -1  |     |     |     |
| Ry     | 1   | 1   | 1   | 1   | 1   | 1   | 1   | 1   | 1   | 1   | 1   | 1   | 1   | 1   | 1   | 0   | 0   | 0   | 0   | 0   | 0   | 0   | 0   | 0   | 0   | 0   | 0   | 0   | 0   | 0   | 0   | 0   | 0   | 0   | 0   | 0   | 0   | 0   | 0   | 0   | 0   | 0   | 0   | 0   | 0   | -1  | -1  | -1  | -1  | -1  | -1  | -1  | -1  |     |
| R      | 1   | 1   | 1   | 1   | 1   | 1   | -1  | -1  | -1  | -1  | -1  | -1  | -1  | -1  | -1  | i   | i   | i   | i   | i   | i   | i   | i   | i   | i   | i   | i   | i   | i   | i   | -i  | -i  | -i  | -i  | -i  | -i  | -i  | -i  | -i  | -i  | -i  | -i  | -i  | -i  | 1   | 1   | 1   | 1   | 1   | 1   | -1  | -1  | -1  |     |
| Landau | A1  | A1  | A1  | A1  | A1  | A1  | B1  | B1  | B1  | B1  | B1  | B1  | B1  | B1  | B1  | E   | E   | E   | E   | E   | E   | E   | E   | E   | E   | E   | E   | E   | E   | E   | E   | E   | E   | E   | E   | E   | E   | E   | E   | E   | E   | E   | E   | E   | A2  | A2  | A2  | A2  | A2  | A2  | B2  | B2  | B2  |     |





$\mathbf{S} = \mathbf{1}, \mathbf{n}_{\text{occ.}} = \{\mathbf{1}, \mathbf{3}, \mathbf{0}\}$

|        |     |     |     |     |     |     |     |     |     |     |     |     |     |     |     |     |     |     |     |     |     |     |      |      |      |      |      |      |      |      |     |     |     |     |     |     |
|--------|-----|-----|-----|-----|-----|-----|-----|-----|-----|-----|-----|-----|-----|-----|-----|-----|-----|-----|-----|-----|-----|-----|------|------|------|------|------|------|------|------|-----|-----|-----|-----|-----|-----|
| State  | 703 | 704 | 705 | 706 | 707 | 708 | 709 | 710 | 711 | 712 | 713 | 714 | 715 | 716 | 717 | 718 | 719 | 720 | 721 | 722 | 723 | 724 | 725  | 726  | 727  | 728  | 729  | 730  | 731  | 732  | 733 | 734 | 735 | 736 | 737 | 738 |
| Sz     | 1   | 0   | -1  | 1   | 0   | -1  | 1   | 0   | -1  | 1   | 0   | -1  | 1   | 0   | -1  | 1   | 0   | -1  | 1   | 0   | -1  | 1   | 0    | -1   | 1    | 0    | -1   | 1    | 0    | -1   | 1   | 0   | -1  | 1   | 0   | -1  |
| Rx     | 1   | 1   | 1   | 1   | 1   | 1   | 1   | 1   | 1   | 1   | 1   | 1   | 0   | 0   | 0   | 0   | 0   | 0   | 0   | 0   | 0   | 0   | 0    | 0    | 0    | 0    | 0    | 0    | 0    | 0    | -1  | -1  | -1  | -1  | -1  | -1  |
| Ry     | 1   | 1   | 1   | 1   | 1   | 1   | 1   | 1   | 1   | 1   | 1   | 1   | 0   | 0   | 0   | 0   | 0   | 0   | 0   | 0   | 0   | 0   | 0    | 0    | 0    | 0    | 0    | 0    | 0    | 0    | -1  | -1  | -1  | -1  | -1  | -1  |
| R      | 1   | 1   | 1   | 1   | 1   | 1   | -1  | -1  | -1  | -1  | -1  | -1  | $i$ | $i$ | $i$ | $i$ | $i$ | $i$ | $i$ | $i$ | $i$ | $i$ | $-i$ | $-i$ | $-i$ | $-i$ | $-i$ | $-i$ | $-i$ | $-i$ | 1   | 1   | 1   | -1  | -1  | -1  |
| Landau | A1  | A1  | A1  | A1  | A1  | A1  | B1  | B1  | B1  | B1  | B1  | B1  | E   | E   | E   | E   | E   | E   | E   | E   | E   | E   | E    | E    | E    | E    | E    | E    | E    | E    | A2  | A2  | A2  | B2  | B2  | B2  |



$$S = 1, n_{\text{max}} = \{1, 1, 2\}$$

$\mathbf{S} = \mathbf{1}, \mathbf{n}_{\text{occ.}} = \{\mathbf{1}, \mathbf{0}, \mathbf{3}\}$

|        |     |     |     |     |     |     |     |     |     |     |     |     |     |     |     |     |     |     |     |     |     |     |      |      |      |      |      |      |      |      |     |     |     |     |     |     |    |
|--------|-----|-----|-----|-----|-----|-----|-----|-----|-----|-----|-----|-----|-----|-----|-----|-----|-----|-----|-----|-----|-----|-----|------|------|------|------|------|------|------|------|-----|-----|-----|-----|-----|-----|----|
| State  | 955 | 956 | 957 | 958 | 959 | 960 | 961 | 962 | 963 | 964 | 965 | 966 | 967 | 968 | 969 | 970 | 971 | 972 | 973 | 974 | 975 | 976 | 977  | 978  | 979  | 980  | 981  | 982  | 983  | 984  | 985 | 986 | 987 | 988 | 989 | 990 |    |
| Sz     | 1   | 0   | -1  | 1   | 0   | -1  | 1   | 0   | -1  | 1   | 0   | -1  | 1   | 0   | -1  | 1   | 0   | -1  | 1   | 0   | -1  | 1   | 0    | -1   | 1    | 0    | -1   | 1    | 0    | -1   | 1   | 0   | -1  | 1   | 0   | -1  |    |
| Rx     | 1   | 1   | 1   | 1   | 1   | 1   | 1   | 1   | 1   | 1   | 1   | 1   | 0   | 0   | 0   | 0   | 0   | 0   | 0   | 0   | 0   | 0   | 0    | 0    | 0    | 0    | 0    | 0    | 0    | 0    | -1  | -1  | -1  | -1  | -1  | -1  |    |
| Ry     | 1   | 1   | 1   | 1   | 1   | 1   | 1   | 1   | 1   | 1   | 1   | 1   | 0   | 0   | 0   | 0   | 0   | 0   | 0   | 0   | 0   | 0   | 0    | 0    | 0    | 0    | 0    | 0    | 0    | 0    | 0   | -1  | -1  | -1  | -1  | -1  | -1 |
| R      | 1   | 1   | 1   | 1   | 1   | 1   | -1  | -1  | -1  | -1  | -1  | -1  | $i$ | $i$ | $i$ | $i$ | $i$ | $i$ | $i$ | $i$ | $i$ | $i$ | $-i$ | $-i$ | $-i$ | $-i$ | $-i$ | $-i$ | $-i$ | $-i$ | 1   | 1   | 1   | -1  | -1  | -1  |    |
| Landau | A1  | A1  | A1  | A1  | A1  | A1  | B1  | B1  | B1  | B1  | B1  | B1  | E   | E   | E   | E   | E   | E   | E   | E   | E   | E   | E    | E    | E    | E    | E    | E    | E    | E    | A2  | A2  | A2  | B2  | B2  | B2  |    |

$$S = 1, \text{ n}_{\text{occ.}} = \{0, 4, 0\}$$

$$\left( \begin{array}{cccccccccc} \text{State} & 991 & 992 & 993 & 994 & 995 & 996 & 997 & 998 & 999 \\ \text{Sz} & 1 & 0 & -1 & 1 & 0 & -1 & 1 & 0 & -1 \\ \text{Rx} & 1 & 1 & 1 & 0 & 0 & 0 & 0 & 0 & 0 \\ \text{Ry} & 1 & 1 & 1 & 0 & 0 & 0 & 0 & 0 & 0 \\ \text{R} & -1 & -1 & -1 & i & i & i & -i & -i & -i \\ \text{Landau} & \text{B1} & \text{B1} & \text{B1} & \text{E} & \text{E} & \text{E} & \text{E} & \text{E} & \text{E} \end{array} \right)$$



$$\mathbf{S} = \mathbf{1}, \mathbf{n}_{\text{occ.}} = \{\mathbf{0}, \mathbf{3}, \mathbf{1}\}$$

| State  | 1000 | 1001 | 1002 | 1003 | 1004 | 1005 | 1006 | 1007 | 1008 | 1009 | 1010 | 1011 | 1012 | 1013 | 1014 | 1015 | 1016 | 1017 | 1018 | 1019 | 1020 | 1021 | 1022 | 1023 | 1024 | 1025 | 1026 | 1027 | 1028 | 1029 | 1030 | 1031 | 1032 | 1033 | 1034 | 1035 |
|--------|------|------|------|------|------|------|------|------|------|------|------|------|------|------|------|------|------|------|------|------|------|------|------|------|------|------|------|------|------|------|------|------|------|------|------|------|
| Sz     | 1    | 0    | -1   | 1    | 0    | -1   | 1    | 0    | -1   | 1    | 0    | -1   | 1    | 0    | -1   | 1    | 0    | -1   | 1    | 0    | -1   | 1    | 0    | -1   | 1    | 0    | -1   | 1    | 0    | -1   | 1    | 0    | -1   | 1    | 0    | -1   |
| Rx     | 1    | 1    | 1    | 1    | 1    | 1    | 1    | 1    | 1    | 1    | 1    | 1    | 0    | 0    | 0    | 0    | 0    | 0    | 0    | 0    | 0    | 0    | 0    | 0    | 0    | 0    | 0    | 0    | 0    | 0    | -1   | -1   | -1   | -1   | -1   | -1   |
| Ry     | 1    | 1    | 1    | 1    | 1    | 1    | 1    | 1    | 1    | 1    | 1    | 1    | 0    | 0    | 0    | 0    | 0    | 0    | 0    | 0    | 0    | 0    | 0    | 0    | 0    | 0    | 0    | 0    | 0    | 0    | -1   | -1   | -1   | -1   | -1   | -1   |
| R      | 1    | 1    | 1    | 1    | 1    | 1    | -1   | -1   | -1   | -1   | -1   | -1   | $i$  | $i$  | $i$  | $i$  | $i$  | $i$  | $i$  | $i$  | $i$  | $i$  | $i$  | $-i$ | $-i$ | $-i$ | $-i$ | $-i$ | $-i$ | $-i$ | 1    | 1    | 1    | -1   | -1   | -1   |
| Landau | A1   | A1   | A1   | A1   | A1   | A1   | B1   | B1   | B1   | B1   | B1   | B1   | E    | E    | E    | E    | E    | E    | E    | E    | E    | E    | E    | E    | E    | E    | E    | E    | E    | E    | A2   | A2   | A2   | B2   | B2   | B2   |

$$S = 1, \mathbf{n}_{occ.} = \{0, 2, 2\}$$

[illegible]

$$\mathbf{S} = \mathbf{1}, \mathbf{n}_{\text{occ.}} = \{\mathbf{0}, \mathbf{1}, \mathbf{3}\}$$

| State  | 1090 | 1091 | 1092 | 1093 | 1094 | 1095 | 1096 | 1097 | 1098 | 1099 | 1100 | 1101 | 1102 | 1103 | 1104 | 1105 | 1106 | 1107 | 1108 | 1109 | 1110 | 1111 | 1112 | 1113 | 1114 | 1115 | 1116 | 1117 | 1118 | 1119 | 1120 | 1121 | 1122 | 1123 | 1124 | 1125 |
|--------|------|------|------|------|------|------|------|------|------|------|------|------|------|------|------|------|------|------|------|------|------|------|------|------|------|------|------|------|------|------|------|------|------|------|------|------|
| Sz     | 1    | 0    | -1   | 1    | 0    | -1   | 1    | 0    | -1   | 1    | 0    | -1   | 1    | 0    | -1   | 1    | 0    | -1   | 1    | 0    | -1   | 1    | 0    | -1   | 1    | 0    | -1   | 1    | 0    | -1   | 1    | 0    | -1   | 1    | 0    | -1   |
| Rx     | 1    | 1    | 1    | 1    | 1    | 1    | 1    | 1    | 1    | 1    | 1    | 1    | 0    | 0    | 0    | 0    | 0    | 0    | 0    | 0    | 0    | 0    | 0    | 0    | 0    | 0    | 0    | 0    | 0    | 0    | 0    | -1   | -1   | -1   | -1   | -1   |
| Ry     | 1    | 1    | 1    | 1    | 1    | 1    | 1    | 1    | 1    | 1    | 1    | 1    | 0    | 0    | 0    | 0    | 0    | 0    | 0    | 0    | 0    | 0    | 0    | 0    | 0    | 0    | 0    | 0    | 0    | 0    | 0    | -1   | -1   | -1   | -1   | -1   |
| R      | 1    | 1    | 1    | 1    | 1    | 1    | -1   | -1   | -1   | -1   | -1   | -1   | $i$  | $i$  | $i$  | $i$  | $i$  | $i$  | $i$  | $i$  | $i$  | $i$  | $i$  | $-i$ | $-i$ | $-i$ | $-i$ | $-i$ | $-i$ | $-i$ | 1    | 1    | 1    | -1   | -1   | -1   |
| Landau | A1   | A1   | A1   | A1   | A1   | A1   | B1   | B1   | B1   | B1   | B1   | B1   | E    | E    | E    | E    | E    | E    | E    | E    | E    | E    | E    | E    | E    | E    | E    | E    | E    | E    | A2   | A2   | A2   | B2   | B2   | B2   |

$$S = 1, \text{ n}_{\text{occ.}} = \{0, 0, 4\}$$

$$\left( \begin{array}{cccccccccc} \text{State} & 1126 & 1127 & 1128 & 1129 & 1130 & 1131 & 1132 & 1133 & 1134 \\ S_z & 1 & 0 & -1 & 1 & 0 & -1 & 1 & 0 & -1 \\ R_x & 1 & 1 & 1 & 0 & 0 & 0 & 0 & 0 & 0 \\ R_y & 1 & 1 & 1 & 0 & 0 & 0 & 0 & 0 & 0 \\ R & -1 & -1 & -1 & i & i & i & -i & -i & -i \\ \text{Landau} & B1 & B1 & B1 & E & E & E & E & E & E \end{array} \right)$$

$$\mathbf{S} = \mathbf{0}, \mathbf{n}_{\text{occ.}} = \{4, 0, 0\}$$

$$\left( \begin{array}{ccc} \text{State} & 1135 & 1136 \\ \text{Sz} & 0 & 0 \\ \text{Rx} & 1 & -1 \\ \text{Ry} & 1 & -1 \\ \text{R} & 1 & -1 \\ \text{Landau} & \text{A1} & \text{B2} \end{array} \right)$$

$$\mathbf{S} = \mathbf{0}, \mathbf{n}_{\text{occ.}} = \{\mathbf{3}, \mathbf{1}, \mathbf{0}\}$$

$$\left( \begin{array}{cccccccccc} \text{State} & 1137 & 1138 & 1139 & 1140 & 1141 & 1142 & 1143 & 1144 \\ \text{Sz} & 0 & 0 & 0 & 0 & 0 & 0 & 0 & 0 \\ \text{Rx} & 1 & 1 & 0 & 0 & 0 & 0 & -1 & -1 \\ \text{Ry} & 1 & 1 & 0 & 0 & 0 & 0 & -1 & -1 \\ \text{R} & 1 & -1 & i & i & -i & -i & 1 & -1 \\ \text{Landau} & \text{A1} & \text{B1} & \text{E} & \text{E} & \text{E} & \text{E} & \text{A2} & \text{B2} \end{array} \right)$$

$$\mathbf{S} = \mathbf{0}, \mathbf{n}_{\text{occ.}} = \{\mathbf{3}, \mathbf{0}, \mathbf{1}\}$$

$$\left( \begin{array}{cccccccccc} \text{State} & 1145 & 1146 & 1147 & 1148 & 1149 & 1150 & 1151 & 1152 \\ \text{Sz} & 0 & 0 & 0 & 0 & 0 & 0 & 0 & 0 \\ \text{Rx} & 1 & 1 & 0 & 0 & 0 & 0 & -1 & -1 \\ \text{Ry} & 1 & 1 & 0 & 0 & 0 & 0 & -1 & -1 \\ \text{R} & 1 & -1 & i & i & -i & -i & 1 & -1 \\ \text{Landau} & \text{A1} & \text{B1} & \text{E} & \text{E} & \text{E} & \text{E} & \text{A2} & \text{B2} \end{array} \right)$$

$$\mathbf{S} = \mathbf{0}, \mathbf{n}_{\text{occ.}} = \{\mathbf{2}, \mathbf{2}, \mathbf{0}\}$$

| State  | 1153 | 1154 | 1155 | 1156 | 1157 | 1158 | 1159 | 1160 | 1161 | 1162 | 1163 | 1164 |
|--------|------|------|------|------|------|------|------|------|------|------|------|------|
| Sz     | 0    | 0    | 0    | 0    | 0    | 0    | 0    | 0    | 0    | 0    | 0    | 0    |
| Rx     | 1    | 1    | 1    | 1    | 0    | 0    | 0    | 0    | -1   | -1   | -1   | -1   |
| Ry     | 1    | 1    | 1    | 1    | 0    | 0    | 0    | 0    | -1   | -1   | -1   | -1   |
| R      | 1    | 1    | 1    | -1   | $i$  | $i$  | $-i$ | $-i$ | 1    | -1   | -1   | -1   |
| Landau | A1   | A1   | A1   | B1   | E    | E    | E    | E    | A2   | B2   | B2   | B2   |



$$\mathbf{S} = \mathbf{0}, \mathbf{n}_{\text{occ.}} = \{2, 1, 1\}$$

| State  | 1165 | 1166 | 1167 | 1168 | 1169 | 1170 | 1171 | 1172 | 1173 | 1174 | 1175 | 1176 | 1177 | 1178 | 1179 | 1180 | 1181 | 1182 | 1183 | 1184 | 1185 | 1186 | 1187 | 1188 |
|--------|------|------|------|------|------|------|------|------|------|------|------|------|------|------|------|------|------|------|------|------|------|------|------|------|
| Sz     | 0    | 0    | 0    | 0    | 0    | 0    | 0    | 0    | 0    | 0    | 0    | 0    | 0    | 0    | 0    | 0    | 0    | 0    | 0    | 0    | 0    | 0    | 0    | 0    |
| Rx     | 1    | 1    | 1    | 1    | 1    | 1    | 0    | 0    | 0    | 0    | 0    | 0    | 0    | 0    | 0    | 0    | 0    | 0    | -1   | -1   | -1   | -1   | -1   | -1   |
| Ry     | 1    | 1    | 1    | 1    | 1    | 1    | 0    | 0    | 0    | 0    | 0    | 0    | 0    | 0    | 0    | 0    | 0    | 0    | -1   | -1   | -1   | -1   | -1   | -1   |
| R      | 1    | 1    | 1    | -1   | -1   | -1   | $i$  | $i$  | $i$  | $i$  | $i$  | $i$  | $i$  | $-i$ | $-i$ | $-i$ | $-i$ | $-i$ | 1    | 1    | 1    | -1   | -1   | -1   |
| Landau | A1   | A1   | A1   | B1   | B1   | B1   | E    | E    | E    | E    | E    | E    | E    | E    | E    | E    | E    | E    | A2   | A2   | A2   | B2   | B2   | B2   |

$$\mathbf{S} = \mathbf{0}, \mathbf{n}_{\text{occ.}} = \{\mathbf{2}, \mathbf{0}, \mathbf{2}\}$$

| State  | 1189 | 1190 | 1191 | 1192 | 1193 | 1194 | 1195 | 1196 | 1197 | 1198 | 1199 | 1200 |
|--------|------|------|------|------|------|------|------|------|------|------|------|------|
| Sz     | 0    | 0    | 0    | 0    | 0    | 0    | 0    | 0    | 0    | 0    | 0    | 0    |
| Rx     | 1    | 1    | 1    | 1    | 0    | 0    | 0    | 0    | -1   | -1   | -1   | -1   |
| Ry     | 1    | 1    | 1    | 1    | 0    | 0    | 0    | 0    | -1   | -1   | -1   | -1   |
| R      | 1    | 1    | 1    | -1   | $i$  | $i$  | $-i$ | $-i$ | 1    | -1   | -1   | -1   |
| Landau | A1   | A1   | A1   | B1   | E    | E    | E    | E    | A2   | B2   | B2   | B2   |

$$\mathbf{S} = \mathbf{0}, \mathbf{n}_{\text{occ.}} = \{\mathbf{1}, \mathbf{3}, \mathbf{0}\}$$

$$\left( \begin{array}{cccccccccc} \text{State} & 1201 & 1202 & 1203 & 1204 & 1205 & 1206 & 1207 & 1208 \\ \text{Sz} & 0 & 0 & 0 & 0 & 0 & 0 & 0 & 0 \\ \text{Rx} & 1 & 1 & 0 & 0 & 0 & 0 & -1 & -1 \\ \text{Ry} & 1 & 1 & 0 & 0 & 0 & 0 & -1 & -1 \\ \text{R} & 1 & -1 & i & i & -i & -i & 1 & -1 \\ \text{Landau} & \text{A1} & \text{B1} & \text{E} & \text{E} & \text{E} & \text{E} & \text{A2} & \text{B2} \end{array} \right)$$

$$\mathbf{S} = \mathbf{0}, \mathbf{n}_{\text{occ.}} = \{1, 2, 1\}$$

| State  | 1209 | 1210 | 1211 | 1212 | 1213 | 1214 | 1215 | 1216 | 1217 | 1218 | 1219 | 1220 | 1221 | 1222 | 1223 | 1224 | 1225 | 1226 | 1227 | 1228 | 1229 | 1230 | 1231 | 1232 |
|--------|------|------|------|------|------|------|------|------|------|------|------|------|------|------|------|------|------|------|------|------|------|------|------|------|
| Sz     | 0    | 0    | 0    | 0    | 0    | 0    | 0    | 0    | 0    | 0    | 0    | 0    | 0    | 0    | 0    | 0    | 0    | 0    | 0    | 0    | 0    | 0    | 0    | 0    |
| Rx     | 1    | 1    | 1    | 1    | 1    | 1    | 0    | 0    | 0    | 0    | 0    | 0    | 0    | 0    | 0    | 0    | 0    | 0    | -1   | -1   | -1   | -1   | -1   | -1   |
| Ry     | 1    | 1    | 1    | 1    | 1    | 1    | 0    | 0    | 0    | 0    | 0    | 0    | 0    | 0    | 0    | 0    | 0    | 0    | -1   | -1   | -1   | -1   | -1   | -1   |
| R      | 1    | 1    | 1    | -1   | -1   | -1   | $i$  | $i$  | $i$  | $i$  | $i$  | $i$  | $-i$ | $-i$ | $-i$ | $-i$ | $-i$ | $-i$ | 1    | 1    | 1    | -1   | -1   | -1   |
| Landau | A1   | A1   | A1   | B1   | B1   | B1   | E    | E    | E    | E    | E    | E    | E    | E    | E    | E    | E    | E    | A2   | A2   | A2   | B2   | B2   | B2   |

$$\mathbf{S} = \mathbf{0}, \mathbf{n}_{\text{occ.}} = \{1, 1, 2\}$$

| State  | 1233 | 1234 | 1235 | 1236 | 1237 | 1238 | 1239 | 1240 | 1241 | 1242 | 1243 | 1244 | 1245 | 1246 | 1247 | 1248 | 1249 | 1250 | 1251 | 1252 | 1253 | 1254 | 1255 | 1256 |
|--------|------|------|------|------|------|------|------|------|------|------|------|------|------|------|------|------|------|------|------|------|------|------|------|------|
| Sz     | 0    | 0    | 0    | 0    | 0    | 0    | 0    | 0    | 0    | 0    | 0    | 0    | 0    | 0    | 0    | 0    | 0    | 0    | 0    | 0    | 0    | 0    | 0    | 0    |
| Rx     | 1    | 1    | 1    | 1    | 1    | 1    | 0    | 0    | 0    | 0    | 0    | 0    | 0    | 0    | 0    | 0    | 0    | 0    | -1   | -1   | -1   | -1   | -1   | -1   |
| Ry     | 1    | 1    | 1    | 1    | 1    | 1    | 0    | 0    | 0    | 0    | 0    | 0    | 0    | 0    | 0    | 0    | 0    | 0    | -1   | -1   | -1   | -1   | -1   | -1   |
| R      | 1    | 1    | 1    | -1   | -1   | -1   | $i$  | $i$  | $i$  | $i$  | $i$  | $i$  | $i$  | $i$  | $-i$ | $-i$ | $-i$ | $-i$ | 1    | 1    | 1    | -1   | -1   | -1   |
| Landau | A1   | A1   | A1   | B1   | B1   | B1   | E    | E    | E    | E    | E    | E    | E    | E    | E    | E    | E    | E    | A2   | A2   | A2   | B2   | B2   | B2   |

$$\mathbf{S} = \mathbf{0}, \mathbf{n}_{\text{occ.}} = \{\mathbf{1}, \mathbf{0}, \mathbf{3}\}$$

$$\left( \begin{array}{cccccccc} \text{State} & 1257 & 1258 & 1259 & 1260 & 1261 & 1262 & 1263 & 1264 \\ \text{Sz} & 0 & 0 & 0 & 0 & 0 & 0 & 0 & 0 \\ \text{Rx} & 1 & 1 & 0 & 0 & 0 & 0 & -1 & -1 \\ \text{Ry} & 1 & 1 & 0 & 0 & 0 & 0 & -1 & -1 \\ \text{R} & 1 & -1 & i & i & -i & -i & 1 & -1 \\ \text{Landau} & \text{A1} & \text{B1} & \text{E} & \text{E} & \text{E} & \text{E} & \text{A2} & \text{B2} \end{array} \right)$$

$$\mathbf{S} = \mathbf{0}, \text{ n}_{\text{occ.}} = \{0, 4, 0\}$$

$$\left( \begin{array}{ccc} \text{State} & 1265 & 1266 \\ \text{Sz} & 0 & 0 \\ \text{Rx} & 1 & -1 \\ \text{Ry} & 1 & -1 \\ \text{R} & 1 & -1 \\ \text{Landau} & \text{A1} & \text{B2} \end{array} \right)$$

$$\mathbf{S} = \mathbf{0}, \mathbf{n}_{\text{occ.}} = \{\mathbf{0}, \mathbf{3}, \mathbf{1}\}$$

$$\left( \begin{array}{cccccccccc} \text{State} & 1267 & 1268 & 1269 & 1270 & 1271 & 1272 & 1273 & 1274 \\ \text{Sz} & 0 & 0 & 0 & 0 & 0 & 0 & 0 & 0 \\ \text{Rx} & 1 & 1 & 0 & 0 & 0 & 0 & -1 & -1 \\ \text{Ry} & 1 & 1 & 0 & 0 & 0 & 0 & -1 & -1 \\ \text{R} & 1 & -1 & i & i & -i & -i & 1 & -1 \\ \text{Landau} & \text{A1} & \text{B1} & \text{E} & \text{E} & \text{E} & \text{E} & \text{A2} & \text{B2} \end{array} \right)$$



$$\mathbf{S} = \mathbf{0}, \mathbf{n}_{\text{occ.}} = \{\mathbf{0}, \mathbf{2}, \mathbf{2}\}$$

| State  | 1275 | 1276 | 1277 | 1278 | 1279 | 1280 | 1281 | 1282 | 1283 | 1284 | 1285 | 1286 |
|--------|------|------|------|------|------|------|------|------|------|------|------|------|
| Sz     | 0    | 0    | 0    | 0    | 0    | 0    | 0    | 0    | 0    | 0    | 0    | 0    |
| Rx     | 1    | 1    | 1    | 1    | 0    | 0    | 0    | 0    | -1   | -1   | -1   | -1   |
| Ry     | 1    | 1    | 1    | 1    | 0    | 0    | 0    | 0    | -1   | -1   | -1   | -1   |
| R      | 1    | 1    | 1    | -1   | $i$  | $i$  | $-i$ | $-i$ | 1    | -1   | -1   | -1   |
| Landau | A1   | A1   | A1   | B1   | E    | E    | E    | E    | A2   | B2   | B2   | B2   |

$$\mathbf{S} = \mathbf{0}, \mathbf{n}_{\text{occ.}} = \{\mathbf{0}, \mathbf{1}, \mathbf{3}\}$$

$$\left( \begin{array}{cccccccccc} \text{State} & 1287 & 1288 & 1289 & 1290 & 1291 & 1292 & 1293 & 1294 \\ \text{Sz} & 0 & 0 & 0 & 0 & 0 & 0 & 0 & 0 \\ \text{Rx} & 1 & 1 & 0 & 0 & 0 & 0 & -1 & -1 \\ \text{Ry} & 1 & 1 & 0 & 0 & 0 & 0 & -1 & -1 \\ \text{R} & 1 & -1 & i & i & -i & -i & 1 & -1 \\ \text{Landau} & \text{A1} & \text{B1} & \text{E} & \text{E} & \text{E} & \text{E} & \text{A2} & \text{B2} \end{array} \right)$$

$$\mathbf{S} = \mathbf{0}, \text{ n}_{\text{occ.}} = \{0, 0, 4\}$$

$$\left( \begin{array}{ccc} \text{State} & 1295 & 1296 \\ \text{Sz} & 0 & 0 \\ \text{Rx} & 1 & -1 \\ \text{Ry} & 1 & -1 \\ \text{R} & 1 & -1 \\ \text{Landau} & \text{A1} & \text{B2} \end{array} \right)$$

$$\mathbf{S} = \mathbf{2}, \mathbf{n}_{\text{occ.}} = \{4, \mathbf{0}, \mathbf{0}, \mathbf{0}\}$$

$$\left( \begin{array}{ccccc} \text{State} & 1 & 2 & 3 & 4 & 5 \\ \text{Sz} & 2 & 1 & 0 & -1 & -2 \\ \text{Rx} & 1 & 1 & 1 & 1 & 1 \\ \text{Ry} & 1 & 1 & 1 & 1 & 1 \\ \text{R} & 1 & 1 & 1 & 1 & 1 \\ \text{Landau} & \text{A1} & \text{A1} & \text{A1} & \text{A1} & \text{A1} \end{array} \right)$$



$$\mathbf{S} = \mathbf{2}, \mathbf{n}_{\text{occ.}} = \{\mathbf{2}, \mathbf{2}, \mathbf{0}, \mathbf{0}\}$$

| State  | 26 | 27 | 28 | 29 | 30 | 31 | 32 | 33 | 34 | 35 | 36 | 37 | 38 | 39 | 40 | 41  | 42  | 43  | 44  | 45  | 46   | 47   | 48   | 49   | 50   | 51 | 52 | 53 | 54 | 55 |
|--------|----|----|----|----|----|----|----|----|----|----|----|----|----|----|----|-----|-----|-----|-----|-----|------|------|------|------|------|----|----|----|----|----|
| Sz     | 2  | 1  | 0  | -1 | -2 | 2  | 1  | 0  | -1 | -2 | 2  | 1  | 0  | -1 | -2 | 2   | 1   | 0   | -1  | -2  | 2    | 1    | 0    | -1   | -2   | 2  | 1  | 0  | -1 | -2 |
| Rx     | 1  | 1  | 1  | 1  | 1  | 1  | 1  | 1  | 1  | 1  | 1  | 1  | 1  | 1  | 1  | 0   | 0   | 0   | 0   | 0   | 0    | 0    | 0    | 0    | 0    | -1 | -1 | -1 | -1 | -1 |
| Ry     | 1  | 1  | 1  | 1  | 1  | 1  | 1  | 1  | 1  | 1  | 1  | 1  | 1  | 1  | 1  | 0   | 0   | 0   | 0   | 0   | 0    | 0    | 0    | 0    | 0    | -1 | -1 | -1 | -1 | -1 |
| R      | 1  | 1  | 1  | 1  | 1  | 1  | 1  | 1  | 1  | 1  | -1 | -1 | -1 | -1 | -1 | $i$ | $i$ | $i$ | $i$ | $i$ | $-i$ | $-i$ | $-i$ | $-i$ | $-i$ | -1 | -1 | -1 | -1 | -1 |
| Landau | A1 | A1 | A1 | A1 | A1 | A1 | A1 | A1 | A1 | A1 | B1 | B1 | B1 | B1 | B1 | E   | E   | E   | E   | E   | E    | E    | E    | E    | E    | B2 | B2 | B2 | B2 | B2 |



$$\mathbf{S} = \mathbf{2}, \mathbf{n}_{\text{occ.}} = \{\mathbf{0}, \mathbf{4}, \mathbf{0}, \mathbf{0}\}$$

$$\left( \begin{array}{cccccc} \text{State} & 76 & 77 & 78 & 79 & 80 \\ \text{Sz} & 2 & 1 & 0 & -1 & -2 \\ \text{Rx} & 1 & 1 & 1 & 1 & 1 \\ \text{Ry} & 1 & 1 & 1 & 1 & 1 \\ \text{R} & 1 & 1 & 1 & 1 & 1 \\ \text{Landau} & \text{A1} & \text{A1} & \text{A1} & \text{A1} & \text{A1} \end{array} \right)$$



$$\mathbf{S} = \mathbf{3}/\mathbf{2}, \mathbf{n}_{\text{occ.}} = \{\mathbf{3}, \mathbf{0}, \mathbf{1}, \mathbf{0}\}$$

| State  | 81            | 82            | 83             | 84             | 85            | 86            | 87             | 88             | 89            | 90            | 91             | 92             | 93            | 94            | 95             | 96             |
|--------|---------------|---------------|----------------|----------------|---------------|---------------|----------------|----------------|---------------|---------------|----------------|----------------|---------------|---------------|----------------|----------------|
| Sz     | $\frac{3}{2}$ | $\frac{1}{2}$ | $-\frac{1}{2}$ | $-\frac{3}{2}$ | $\frac{3}{2}$ | $\frac{1}{2}$ | $-\frac{1}{2}$ | $-\frac{3}{2}$ | $\frac{3}{2}$ | $\frac{1}{2}$ | $-\frac{1}{2}$ | $-\frac{3}{2}$ | $\frac{3}{2}$ | $\frac{1}{2}$ | $-\frac{1}{2}$ | $-\frac{3}{2}$ |
| Rx     | 1             | 1             | 1              | 1              | 1             | 1             | 1              | 1              | 0             | 0             | 0              | 0              | 0             | 0             | 0              | 0              |
| Ry     | 1             | 1             | 1              | 1              | 1             | 1             | 1              | 1              | 0             | 0             | 0              | 0              | 0             | 0             | 0              | 0              |
| R      | 1             | 1             | 1              | 1              | -1            | -1            | -1             | -1             | $i$           | $i$           | $i$            | $i$            | $-i$          | $-i$          | $-i$           | $-i$           |
| Landau | A1            | A1            | A1             | A1             | B1            | B1            | B1             | B1             | E             | E             | E              | E              | E             | E             | E              | E              |

$$\mathbf{S} = \mathbf{3}/\mathbf{2}, \text{ n}_{\text{occ.}} = \{\mathbf{3}, \mathbf{0}, \mathbf{0}, \mathbf{1}\}$$

| State  | 97            | 98            | 99             | 100            | 101           | 102           | 103            | 104            | 105           | 106           | 107            | 108            | 109           | 110           | 111            | 112            |
|--------|---------------|---------------|----------------|----------------|---------------|---------------|----------------|----------------|---------------|---------------|----------------|----------------|---------------|---------------|----------------|----------------|
| Sz     | $\frac{3}{2}$ | $\frac{1}{2}$ | $-\frac{1}{2}$ | $-\frac{3}{2}$ | $\frac{3}{2}$ | $\frac{1}{2}$ | $-\frac{1}{2}$ | $-\frac{3}{2}$ | $\frac{3}{2}$ | $\frac{1}{2}$ | $-\frac{1}{2}$ | $-\frac{3}{2}$ | $\frac{3}{2}$ | $\frac{1}{2}$ | $-\frac{1}{2}$ | $-\frac{3}{2}$ |
| Rx     | 1             | 1             | 1              | 1              | 1             | 1             | 1              | 1              | 0             | 0             | 0              | 0              | 0             | 0             | 0              | 0              |
| Ry     | 1             | 1             | 1              | 1              | 1             | 1             | 1              | 1              | 0             | 0             | 0              | 0              | 0             | 0             | 0              | 0              |
| R      | 1             | 1             | 1              | 1              | -1            | -1            | -1             | -1             | $i$           | $i$           | $i$            | $i$            | $-i$          | $-i$          | $-i$           | $-i$           |
| Landau | A1            | A1            | A1             | A1             | B1            | B1            | B1             | B1             | E             | E             | E              | E              | E             | E             | E              | E              |



$$\mathbf{S} = \mathbf{3}/\mathbf{2}, \mathbf{n}_{\text{occ.}} = \{\mathbf{2}, \mathbf{1}, \mathbf{0}, \mathbf{1}\}$$

| State  | 161           | 162           | 163            | 164            | 165           | 166           | 167            | 168            | 169           | 170           | 171            | 172            | 173           | 174           | 175            | 176            | 177           | 178           | 179            | 180            | 181           | 182           | 183            | 184            | 185           | 186           | 187            | 188            | 189           | 190           | 191            | 192            | 193           | 194           | 195            | 196            | 197           | 198           | 199            | 200            | 201           | 202           | 203            | 204            | 205 | 206 | 207 | 208 |    |
|--------|---------------|---------------|----------------|----------------|---------------|---------------|----------------|----------------|---------------|---------------|----------------|----------------|---------------|---------------|----------------|----------------|---------------|---------------|----------------|----------------|---------------|---------------|----------------|----------------|---------------|---------------|----------------|----------------|---------------|---------------|----------------|----------------|---------------|---------------|----------------|----------------|---------------|---------------|----------------|----------------|---------------|---------------|----------------|----------------|-----|-----|-----|-----|----|
| Sz     | $\frac{3}{2}$ | $\frac{1}{2}$ | $-\frac{1}{2}$ | $-\frac{3}{2}$ | $\frac{3}{2}$ | $\frac{1}{2}$ | $-\frac{1}{2}$ | $-\frac{3}{2}$ | $\frac{3}{2}$ | $\frac{1}{2}$ | $-\frac{1}{2}$ | $-\frac{3}{2}$ | $\frac{3}{2}$ | $\frac{1}{2}$ | $-\frac{1}{2}$ | $-\frac{3}{2}$ | $\frac{3}{2}$ | $\frac{1}{2}$ | $-\frac{1}{2}$ | $-\frac{3}{2}$ | $\frac{3}{2}$ | $\frac{1}{2}$ | $-\frac{1}{2}$ | $-\frac{3}{2}$ | $\frac{3}{2}$ | $\frac{1}{2}$ | $-\frac{1}{2}$ | $-\frac{3}{2}$ | $\frac{3}{2}$ | $\frac{1}{2}$ | $-\frac{1}{2}$ | $-\frac{3}{2}$ | $\frac{3}{2}$ | $\frac{1}{2}$ | $-\frac{1}{2}$ | $-\frac{3}{2}$ | $\frac{3}{2}$ | $\frac{1}{2}$ | $-\frac{1}{2}$ | $-\frac{3}{2}$ | $\frac{3}{2}$ | $\frac{1}{2}$ | $-\frac{1}{2}$ | $-\frac{3}{2}$ |     |     |     |     |    |
| Rx     | 1             | 1             | 1              | 1              | 1             | 1             | 1              | 1              | 1             | 1             | 1              | 1              | 1             | 1             | 1              | 1              | 0             | 0             | 0              | 0              | 0             | 0             | 0              | 0              | 0             | 0             | 0              | 0              | 0             | 0             | 0              | 0              | 0             | 0             | 0              | 0              | 0             | 0             | 0              | -1             | -1            | -1            | -1             | -1             | -1  | -1  | -1  |     |    |
| Ry     | 1             | 1             | 1              | 1              | 1             | 1             | 1              | 1              | 1             | 1             | 1              | 1              | 1             | 1             | 1              | 1              | 0             | 0             | 0              | 0              | 0             | 0             | 0              | 0              | 0             | 0             | 0              | 0              | 0             | 0             | 0              | 0              | 0             | 0             | 0              | 0              | 0             | 0             | 0              | 0              | 0             | -1            | -1             | -1             | -1  | -1  | -1  | -1  | -1 |
| R      | 1             | 1             | 1              | 1              | 1             | 1             | 1              | 1              | -1            | -1            | -1             | -1             | -1            | -1            | -1             | -1             | $i$           | $i$           | $i$            | $i$            | $i$           | $i$           | $i$            | $i$            | $i$           | $i$           | $i$            | $i$            | $-i$          | $-i$          | $-i$           | $-i$           | $-i$          | $-i$          | $-i$           | $-i$           | $-i$          | $-i$          | $-i$           | 1              | 1             | 1             | 1              | -1             | -1  | -1  | -1  |     |    |
| Landau | A1            | A1            | A1             | A1             | A1            | A1            | A1             | A1             | B1            | B1            | B1             | B1             | B1            | B1            | B1             | B1             | E             | E             | E              | E              | E             | E             | E              | E              | E             | E             | E              | E              | E             | E             | E              | E              | E             | E             | E              | E              | E             | E             | E              | E              | A2            | A2            | A2             | A2             | B2  | B2  | B2  | B2  |    |

$$\mathbf{S} = \mathbf{3}/\mathbf{2}, \mathbf{n}_{\text{occ.}} = \{\mathbf{1}, \mathbf{2}, \mathbf{1}, \mathbf{0}\}$$

|        | 209           | 210           | 211            | 212            | 213           | 214           | 215            | 216            | 217           | 218           | 219            | 220            | 221           | 222           | 223            | 224            | 225           | 226           | 227            | 228            | 229           | 230           | 231            | 232            | 233           | 234           | 235            | 236            | 237           | 238           | 239            | 240            | 241           | 242           | 243            | 244            | 245           | 246           | 247            | 248            | 249           | 250           | 251            | 252            | 253           | 254           | 255            | 256            |    |    |    |
|--------|---------------|---------------|----------------|----------------|---------------|---------------|----------------|----------------|---------------|---------------|----------------|----------------|---------------|---------------|----------------|----------------|---------------|---------------|----------------|----------------|---------------|---------------|----------------|----------------|---------------|---------------|----------------|----------------|---------------|---------------|----------------|----------------|---------------|---------------|----------------|----------------|---------------|---------------|----------------|----------------|---------------|---------------|----------------|----------------|---------------|---------------|----------------|----------------|----|----|----|
| State  | 209           | 210           | 211            | 212            | 213           | 214           | 215            | 216            | 217           | 218           | 219            | 220            | 221           | 222           | 223            | 224            | 225           | 226           | 227            | 228            | 229           | 230           | 231            | 232            | 233           | 234           | 235            | 236            | 237           | 238           | 239            | 240            | 241           | 242           | 243            | 244            | 245           | 246           | 247            | 248            | 249           | 250           | 251            | 252            | 253           | 254           | 255            | 256            |    |    |    |
| Sz     | $\frac{3}{2}$ | $\frac{1}{2}$ | $-\frac{1}{2}$ | $-\frac{3}{2}$ | $\frac{3}{2}$ | $\frac{1}{2}$ | $-\frac{1}{2}$ | $-\frac{3}{2}$ | $\frac{3}{2}$ | $\frac{1}{2}$ | $-\frac{1}{2}$ | $-\frac{3}{2}$ | $\frac{3}{2}$ | $\frac{1}{2}$ | $-\frac{1}{2}$ | $-\frac{3}{2}$ | $\frac{3}{2}$ | $\frac{1}{2}$ | $-\frac{1}{2}$ | $-\frac{3}{2}$ | $\frac{3}{2}$ | $\frac{1}{2}$ | $-\frac{1}{2}$ | $-\frac{3}{2}$ | $\frac{3}{2}$ | $\frac{1}{2}$ | $-\frac{1}{2}$ | $-\frac{3}{2}$ | $\frac{3}{2}$ | $\frac{1}{2}$ | $-\frac{1}{2}$ | $-\frac{3}{2}$ | $\frac{3}{2}$ | $\frac{1}{2}$ | $-\frac{1}{2}$ | $-\frac{3}{2}$ | $\frac{3}{2}$ | $\frac{1}{2}$ | $-\frac{1}{2}$ | $-\frac{3}{2}$ | $\frac{3}{2}$ | $\frac{1}{2}$ | $-\frac{1}{2}$ | $-\frac{3}{2}$ | $\frac{3}{2}$ | $\frac{1}{2}$ | $-\frac{1}{2}$ | $-\frac{3}{2}$ |    |    |    |
| Rx     | 1             | 1             | 1              | 1              | 1             | 1             | 1              | 1              | 1             | 1             | 1              | 1              | 1             | 1             | 1              | 1              | 0             | 0             | 0              | 0              | 0             | 0             | 0              | 0              | 0             | 0             | 0              | 0              | 0             | 0             | 0              | 0              | 0             | 0             | 0              | 0              | 0             | 0             | 0              | -1             | -1            | -1            | -1             | -1             | -1            | -1            | -1             | -1             | -1 |    |    |
| Ry     | 1             | 1             | 1              | 1              | 1             | 1             | 1              | 1              | 1             | 1             | 1              | 1              | 1             | 1             | 1              | 1              | 0             | 0             | 0              | 0              | 0             | 0             | 0              | 0              | 0             | 0             | 0              | 0              | 0             | 0             | 0              | 0              | 0             | 0             | 0              | 0              | 0             | 0             | 0              | 0              | 0             | -1            | -1             | -1             | -1            | -1            | -1             | -1             | -1 | -1 | -1 |
| R      | 1             | 1             | 1              | 1              | 1             | 1             | 1              | 1              | -1            | -1            | -1             | -1             | -1            | -1            | -1             | -1             | i             | i             | i              | i              | i             | i             | i              | i              | i             | i             | i              | i              | -i            | -i            | -i             | -i             | -i            | -i            | -i             | -i             | -i            | -i            | -i             | -i             | 1             | 1             | 1              | 1              | -1            | -1            | -1             | -1             | -1 | -1 |    |
| Landau | A1            | A1            | A1             | A1             | A1            | A1            | A1             | A1             | B1            | B1            | B1             | B1             | B1            | B1            | B1             | B1             | E             | E             | E              | E              | E             | E             | E              | E              | E             | E             | E              | E              | E             | E             | E              | E              | E             | E             | E              | E              | E             | E             | E              | E              | A2            | A2            | A2             | A2             | B2            | B2            | B2             | B2             | B2 | B2 |    |



$$\mathbf{S} = \mathbf{3}/\mathbf{2}, \mathbf{n}_{\text{occ.}} = \{\mathbf{0}, \mathbf{3}, \mathbf{1}, \mathbf{0}\}$$

| State  | 305           | 306           | 307            | 308            | 309           | 310           | 311            | 312            | 313           | 314           | 315            | 316            | 317           | 318           | 319            | 320            |
|--------|---------------|---------------|----------------|----------------|---------------|---------------|----------------|----------------|---------------|---------------|----------------|----------------|---------------|---------------|----------------|----------------|
| Sz     | $\frac{3}{2}$ | $\frac{1}{2}$ | $-\frac{1}{2}$ | $-\frac{3}{2}$ | $\frac{3}{2}$ | $\frac{1}{2}$ | $-\frac{1}{2}$ | $-\frac{3}{2}$ | $\frac{3}{2}$ | $\frac{1}{2}$ | $-\frac{1}{2}$ | $-\frac{3}{2}$ | $\frac{3}{2}$ | $\frac{1}{2}$ | $-\frac{1}{2}$ | $-\frac{3}{2}$ |
| Rx     | 1             | 1             | 1              | 1              | 1             | 1             | 1              | 1              | 0             | 0             | 0              | 0              | 0             | 0             | 0              | 0              |
| Ry     | 1             | 1             | 1              | 1              | 1             | 1             | 1              | 1              | 0             | 0             | 0              | 0              | 0             | 0             | 0              | 0              |
| R      | 1             | 1             | 1              | 1              | -1            | -1            | -1             | -1             | $i$           | $i$           | $i$            | $i$            | $-i$          | $-i$          | $-i$           | $-i$           |
| Landau | A1            | A1            | A1             | A1             | B1            | B1            | B1             | B1             | E             | E             | E              | E              | E             | E             | E              | E              |

$$\mathbf{S} = \mathbf{3}/\mathbf{2}, \text{ n}_{\text{occ.}} = \{\mathbf{0}, \mathbf{3}, \mathbf{0}, \mathbf{1}\}$$

| State  | 321           | 322           | 323            | 324            | 325           | 326           | 327            | 328            | 329           | 330           | 331            | 332            | 333           | 334           | 335            | 336            |
|--------|---------------|---------------|----------------|----------------|---------------|---------------|----------------|----------------|---------------|---------------|----------------|----------------|---------------|---------------|----------------|----------------|
| Sz     | $\frac{3}{2}$ | $\frac{1}{2}$ | $-\frac{1}{2}$ | $-\frac{3}{2}$ | $\frac{3}{2}$ | $\frac{1}{2}$ | $-\frac{1}{2}$ | $-\frac{3}{2}$ | $\frac{3}{2}$ | $\frac{1}{2}$ | $-\frac{1}{2}$ | $-\frac{3}{2}$ | $\frac{3}{2}$ | $\frac{1}{2}$ | $-\frac{1}{2}$ | $-\frac{3}{2}$ |
| Rx     | 1             | 1             | 1              | 1              | 1             | 1             | 1              | 1              | 0             | 0             | 0              | 0              | 0             | 0             | 0              | 0              |
| Ry     | 1             | 1             | 1              | 1              | 1             | 1             | 1              | 1              | 0             | 0             | 0              | 0              | 0             | 0             | 0              | 0              |
| R      | 1             | 1             | 1              | 1              | -1            | -1            | -1             | -1             | $i$           | $i$           | $i$            | $i$            | $-i$          | $-i$          | $-i$           | $-i$           |
| Landau | A1            | A1            | A1             | A1             | B1            | B1            | B1             | B1             | E             | E             | E              | E              | E             | E             | E              | E              |





$$\mathbf{S} = \mathbf{1}, \mathbf{n}_{\text{occ.}} = \{\mathbf{3}, \mathbf{1}, \mathbf{0}, \mathbf{0}\}$$

| State  | 346 | 347 | 348 | 349 | 350 | 351 | 352 | 353 | 354 | 355 | 356 | 357 | 358      | 359      | 360      | 361      | 362      | 363      | 364      | 365      | 366      | 367      | 368        | 369        | 370        | 371        | 372        | 373        | 374        | 375        | 376 | 377 | 378 | 379 | 380 | 381 |    |
|--------|-----|-----|-----|-----|-----|-----|-----|-----|-----|-----|-----|-----|----------|----------|----------|----------|----------|----------|----------|----------|----------|----------|------------|------------|------------|------------|------------|------------|------------|------------|-----|-----|-----|-----|-----|-----|----|
| Sz     | 1   | 0   | -1  | 1   | 0   | -1  | 1   | 0   | -1  | 1   | 0   | -1  | 1        | 0        | -1       | 1        | 0        | -1       | 1        | 0        | -1       | 1        | 0          | -1         | 1          | 0          | -1         | 1          | 0          | -1         | 1   | 0   | -1  | 1   | 0   | -1  |    |
| Rx     | 1   | 1   | 1   | 1   | 1   | 1   | 1   | 1   | 1   | 1   | 1   | 1   | 0        | 0        | 0        | 0        | 0        | 0        | 0        | 0        | 0        | 0        | 0          | 0          | 0          | 0          | 0          | 0          | 0          | 0          | -1  | -1  | -1  | -1  | -1  | -1  |    |
| Ry     | 1   | 1   | 1   | 1   | 1   | 1   | 1   | 1   | 1   | 1   | 1   | 1   | 0        | 0        | 0        | 0        | 0        | 0        | 0        | 0        | 0        | 0        | 0          | 0          | 0          | 0          | 0          | 0          | 0          | 0          | 0   | -1  | -1  | -1  | -1  | -1  | -1 |
| R      | 1   | 1   | 1   | 1   | 1   | 1   | -1  | -1  | -1  | -1  | -1  | -1  | <i>i</i> | <i>i</i> | <i>i</i> | <i>i</i> | <i>i</i> | <i>i</i> | <i>i</i> | <i>i</i> | <i>i</i> | <i>i</i> | - <i>i</i> | - <i>i</i> | - <i>i</i> | - <i>i</i> | - <i>i</i> | - <i>i</i> | - <i>i</i> | - <i>i</i> | 1   | 1   | 1   | -1  | -1  | -1  |    |
| Landau | A1  | A1  | A1  | A1  | A1  | A1  | B1  | B1  | B1  | B1  | B1  | B1  | E        | E        | E        | E        | E        | E        | E        | E        | E        | E        | E          | E          | E          | E          | E          | E          | E          | E          | A2  | A2  | A2  | B2  | B2  | B2  |    |

$$\mathbf{S} = \mathbf{1}, \mathbf{n}_{\text{occ.}} = \{\mathbf{2}, \mathbf{2}, \mathbf{0}, \mathbf{0}\}$$

|        |     |     |     |     |     |     |     |     |     |     |     |     |     |     |     |          |          |          |          |          |          |          |          |          |          |          |          |          |          |          |          |            |            |            |            |            |            |            |            |            |            |            |            |            |            |     |     |     |     |     |     |     |     |     |    |    |    |    |    |
|--------|-----|-----|-----|-----|-----|-----|-----|-----|-----|-----|-----|-----|-----|-----|-----|----------|----------|----------|----------|----------|----------|----------|----------|----------|----------|----------|----------|----------|----------|----------|----------|------------|------------|------------|------------|------------|------------|------------|------------|------------|------------|------------|------------|------------|------------|-----|-----|-----|-----|-----|-----|-----|-----|-----|----|----|----|----|----|
| State  | 382 | 383 | 384 | 385 | 386 | 387 | 388 | 389 | 390 | 391 | 392 | 393 | 394 | 395 | 396 | 397      | 398      | 399      | 400      | 401      | 402      | 403      | 404      | 405      | 406      | 407      | 408      | 409      | 410      | 411      | 412      | 413        | 414        | 415        | 416        | 417        | 418        | 419        | 420        | 421        | 422        | 423        | 424        | 425        | 426        | 427 | 428 | 429 | 430 | 431 | 432 | 433 | 434 | 435 |    |    |    |    |    |
| Sz     | 1   | 0   | -1  | 1   | 0   | -1  | 1   | 0   | -1  | 1   | 0   | -1  | 1   | 0   | -1  | 1        | 0        | -1       | 1        | 0        | -1       | 1        | 0        | -1       | 1        | 0        | -1       | 1        | 0        | -1       | 1        | 0          | -1         | 1          | 0          | -1         | 1          | 0          | -1         | 1          | 0          | -1         | 1          | 0          | -1         | 1   | 0   | -1  | 1   | 0   | -1  |     |     |     |    |    |    |    |    |
| Rx     | 1   | 1   | 1   | 1   | 1   | 1   | 1   | 1   | 1   | 1   | 1   | 1   | 1   | 1   | 1   | 0        | 0        | 0        | 0        | 0        | 0        | 0        | 0        | 0        | 0        | 0        | 0        | 0        | 0        | 0        | 0        | 0          | 0          | 0          | 0          | 0          | 0          | 0          | 0          | 0          | 0          | 0          | 0          | -1         | -1         | -1  | -1  | -1  | -1  | -1  | -1  |     |     |     |    |    |    |    |    |
| Ry     | 1   | 1   | 1   | 1   | 1   | 1   | 1   | 1   | 1   | 1   | 1   | 1   | 1   | 1   | 1   | 0        | 0        | 0        | 0        | 0        | 0        | 0        | 0        | 0        | 0        | 0        | 0        | 0        | 0        | 0        | 0        | 0          | 0          | 0          | 0          | 0          | 0          | 0          | 0          | 0          | 0          | 0          | 0          | 0          | 0          | 0   | 0   | -1  | -1  | -1  | -1  | -1  | -1  | -1  | -1 |    |    |    |    |
| R      | 1   | 1   | 1   | 1   | 1   | 1   | -1  | -1  | -1  | -1  | -1  | -1  | -1  | -1  | -1  | <i>i</i> | <i>i</i> | <i>i</i> | <i>i</i> | <i>i</i> | <i>i</i> | <i>i</i> | <i>i</i> | <i>i</i> | <i>i</i> | <i>i</i> | <i>i</i> | <i>i</i> | <i>i</i> | <i>i</i> | <i>i</i> | - <i>i</i> | - <i>i</i> | - <i>i</i> | - <i>i</i> | - <i>i</i> | - <i>i</i> | - <i>i</i> | - <i>i</i> | - <i>i</i> | - <i>i</i> | - <i>i</i> | - <i>i</i> | - <i>i</i> | - <i>i</i> | 1   | 1   | 1   | 1   | 1   | 1   | -1  | -1  | -1  |    |    |    |    |    |
| Landau | A1  | A1  | A1  | A1  | A1  | A1  | B1  | B1  | B1  | B1  | B1  | B1  | B1  | B1  | B1  | E        | E        | E        | E        | E        | E        | E        | E        | E        | E        | E        | E        | E        | E        | E        | E        | E          | E          | E          | E          | E          | E          | E          | E          | E          | E          | E          | E          | E          | E          | E   | E   | E   | E   | E   | A2  | A2  | A2  | A2  | A2 | A2 | B2 | B2 | B2 |

$$S = 1, \text{ n}_{\text{occ.}} = \{2, 0, 2, 0\}$$

[illegible]

$$\mathbf{S} = \mathbf{1}, \mathbf{n}_{\text{occ.}} = \{\mathbf{2}, \mathbf{0}, \mathbf{1}, \mathbf{1}\}$$

| State  | 454 | 455 | 456 | 457 | 458 | 459 | 460 | 461 | 462 | 463 | 464 | 465 | 466      | 467      | 468      | 469      | 470      | 471      | 472      | 473      | 474      | 475        | 476        | 477        | 478        | 479        | 480        | 481        | 482        | 483        | 484 | 485 | 486 | 487 | 488 | 489 |
|--------|-----|-----|-----|-----|-----|-----|-----|-----|-----|-----|-----|-----|----------|----------|----------|----------|----------|----------|----------|----------|----------|------------|------------|------------|------------|------------|------------|------------|------------|------------|-----|-----|-----|-----|-----|-----|
| Sz     | 1   | 0   | -1  | 1   | 0   | -1  | 1   | 0   | -1  | 1   | 0   | -1  | 1        | 0        | -1       | 1        | 0        | -1       | 1        | 0        | -1       | 1          | 0          | -1         | 1          | 0          | -1         | 1          | 0          | -1         | 1   | 0   | -1  | 1   | 0   | -1  |
| Rx     | 1   | 1   | 1   | 1   | 1   | 1   | 1   | 1   | 1   | 1   | 1   | 1   | 0        | 0        | 0        | 0        | 0        | 0        | 0        | 0        | 0        | 0          | 0          | 0          | 0          | 0          | 0          | 0          | 0          | 0          | -1  | -1  | -1  | -1  | -1  | -1  |
| Ry     | 1   | 1   | 1   | 1   | 1   | 1   | 1   | 1   | 1   | 1   | 1   | 1   | 0        | 0        | 0        | 0        | 0        | 0        | 0        | 0        | 0        | 0          | 0          | 0          | 0          | 0          | 0          | 0          | 0          | 0          | -1  | -1  | -1  | -1  | -1  | -1  |
| R      | 1   | 1   | 1   | 1   | 1   | 1   | -1  | -1  | -1  | -1  | -1  | -1  | <i>i</i> | <i>i</i> | <i>i</i> | <i>i</i> | <i>i</i> | <i>i</i> | <i>i</i> | <i>i</i> | <i>i</i> | - <i>i</i> | - <i>i</i> | - <i>i</i> | - <i>i</i> | - <i>i</i> | - <i>i</i> | - <i>i</i> | - <i>i</i> | - <i>i</i> | 1   | 1   | 1   | -1  | -1  | -1  |
| Landau | A1  | A1  | A1  | A1  | A1  | A1  | B1  | B1  | B1  | B1  | B1  | B1  | E        | E        | E        | E        | E        | E        | E        | E        | E        | E          | E          | E          | E          | E          | E          | E          | E          | E          | A2  | A2  | A2  | B2  | B2  | B2  |



$$\mathbf{S} = \mathbf{1}, \mathbf{n}_{\text{occ.}} = \{\mathbf{1}, \mathbf{3}, \mathbf{0}, \mathbf{0}\}$$

| State  | 508 | 509 | 510 | 511 | 512 | 513 | 514 | 515 | 516 | 517 | 518 | 519 | 520 | 521 | 522 | 523 | 524 | 525 | 526 | 527 | 528 | 529  | 530  | 531  | 532  | 533  | 534  | 535  | 536  | 537 | 538 | 539 | 540 | 541 | 542 | 543 |
|--------|-----|-----|-----|-----|-----|-----|-----|-----|-----|-----|-----|-----|-----|-----|-----|-----|-----|-----|-----|-----|-----|------|------|------|------|------|------|------|------|-----|-----|-----|-----|-----|-----|-----|
| Sz     | 1   | 0   | -1  | 1   | 0   | -1  | 1   | 0   | -1  | 1   | 0   | -1  | 1   | 0   | -1  | 1   | 0   | -1  | 1   | 0   | -1  | 1    | 0    | -1   | 1    | 0    | -1   | 1    | 0    | -1  | 1   | 0   | -1  | 1   | 0   | -1  |
| Rx     | 1   | 1   | 1   | 1   | 1   | 1   | 1   | 1   | 1   | 1   | 1   | 1   | 0   | 0   | 0   | 0   | 0   | 0   | 0   | 0   | 0   | 0    | 0    | 0    | 0    | 0    | 0    | 0    | 0    | 0   | -1  | -1  | -1  | -1  | -1  | -1  |
| Ry     | 1   | 1   | 1   | 1   | 1   | 1   | 1   | 1   | 1   | 1   | 1   | 1   | 0   | 0   | 0   | 0   | 0   | 0   | 0   | 0   | 0   | 0    | 0    | 0    | 0    | 0    | 0    | 0    | 0    | 0   | -1  | -1  | -1  | -1  | -1  | -1  |
| R      | 1   | 1   | 1   | 1   | 1   | 1   | -1  | -1  | -1  | -1  | -1  | -1  | $i$ | $i$ | $i$ | $i$ | $i$ | $i$ | $i$ | $i$ | $i$ | $-i$ | $-i$ | $-i$ | $-i$ | $-i$ | $-i$ | $-i$ | $-i$ | 1   | 1   | 1   | -1  | -1  | -1  |     |
| Landau | A1  | A1  | A1  | A1  | A1  | A1  | B1  | B1  | B1  | B1  | B1  | B1  | E   | E   | E   | E   | E   | E   | E   | E   | E   | E    | E    | E    | E    | E    | E    | E    | E    | E   | A2  | A2  | A2  | B2  | B2  | B2  |

$$\mathbf{S} = \mathbf{1}, \mathbf{n}_{\text{occ.}} = \{\mathbf{1}, \mathbf{1}, \mathbf{2}, \mathbf{0}\}$$

| State  | 544 | 545 | 546 | 547 | 548 | 549 | 550 | 551 | 552 | 553 | 554 | 555 | 556      | 557      | 558      | 559      | 560      | 561      | 562      | 563      | 564      | 565        | 566        | 567        | 568        | 569        | 570        | 571        | 572        | 573        | 574 | 575 | 576 | 577 | 578 | 579 |
|--------|-----|-----|-----|-----|-----|-----|-----|-----|-----|-----|-----|-----|----------|----------|----------|----------|----------|----------|----------|----------|----------|------------|------------|------------|------------|------------|------------|------------|------------|------------|-----|-----|-----|-----|-----|-----|
| Sz     | 1   | 0   | -1  | 1   | 0   | -1  | 1   | 0   | -1  | 1   | 0   | -1  | 1        | 0        | -1       | 1        | 0        | -1       | 1        | 0        | -1       | 1          | 0          | -1         | 1          | 0          | -1         | 1          | 0          | -1         | 1   | 0   | -1  | 1   | 0   | -1  |
| Rx     | 1   | 1   | 1   | 1   | 1   | 1   | 1   | 1   | 1   | 1   | 1   | 1   | 0        | 0        | 0        | 0        | 0        | 0        | 0        | 0        | 0        | 0          | 0          | 0          | 0          | 0          | 0          | 0          | 0          | 0          | -1  | -1  | -1  | -1  | -1  | -1  |
| Ry     | 1   | 1   | 1   | 1   | 1   | 1   | 1   | 1   | 1   | 1   | 1   | 1   | 0        | 0        | 0        | 0        | 0        | 0        | 0        | 0        | 0        | 0          | 0          | 0          | 0          | 0          | 0          | 0          | 0          | 0          | -1  | -1  | -1  | -1  | -1  | -1  |
| R      | 1   | 1   | 1   | 1   | 1   | 1   | -1  | -1  | -1  | -1  | -1  | -1  | <i>i</i> | <i>i</i> | <i>i</i> | <i>i</i> | <i>i</i> | <i>i</i> | <i>i</i> | <i>i</i> | <i>i</i> | - <i>i</i> | - <i>i</i> | - <i>i</i> | - <i>i</i> | - <i>i</i> | - <i>i</i> | - <i>i</i> | - <i>i</i> | - <i>i</i> | 1   | 1   | 1   | -1  | -1  | -1  |
| Landau | A1  | A1  | A1  | A1  | A1  | A1  | B1  | B1  | B1  | B1  | B1  | B1  | E        | E        | E        | E        | E        | E        | E        | E        | E        | E          | E          | E          | E          | E          | E          | E          | E          | E          | A2  | A2  | A2  | B2  | B2  | B2  |





$$\mathbf{S} = \mathbf{1}, \mathbf{n}_{\text{occ.}} = \{\mathbf{1}, \mathbf{1}, \mathbf{0}, \mathbf{2}\}$$

| State  | 652 | 653 | 654 | 655 | 656 | 657 | 658 | 659 | 660 | 661 | 662 | 663 | 664 | 665 | 666 | 667 | 668 | 669 | 670 | 671 | 672 | 673  | 674  | 675  | 676  | 677  | 678  | 679  | 680  | 681 | 682 | 683 | 684 | 685 | 686 | 687 |
|--------|-----|-----|-----|-----|-----|-----|-----|-----|-----|-----|-----|-----|-----|-----|-----|-----|-----|-----|-----|-----|-----|------|------|------|------|------|------|------|------|-----|-----|-----|-----|-----|-----|-----|
| Sz     | 1   | 0   | -1  | 1   | 0   | -1  | 1   | 0   | -1  | 1   | 0   | -1  | 1   | 0   | -1  | 1   | 0   | -1  | 1   | 0   | -1  | 1    | 0    | -1   | 1    | 0    | -1   | 1    | 0    | -1  | 1   | 0   | -1  | 1   | 0   | -1  |
| Rx     | 1   | 1   | 1   | 1   | 1   | 1   | 1   | 1   | 1   | 1   | 1   | 1   | 0   | 0   | 0   | 0   | 0   | 0   | 0   | 0   | 0   | 0    | 0    | 0    | 0    | 0    | 0    | 0    | 0    | 0   | -1  | -1  | -1  | -1  | -1  | -1  |
| Ry     | 1   | 1   | 1   | 1   | 1   | 1   | 1   | 1   | 1   | 1   | 1   | 1   | 0   | 0   | 0   | 0   | 0   | 0   | 0   | 0   | 0   | 0    | 0    | 0    | 0    | 0    | 0    | 0    | 0    | 0   | -1  | -1  | -1  | -1  | -1  | -1  |
| R      | 1   | 1   | 1   | 1   | 1   | 1   | -1  | -1  | -1  | -1  | -1  | -1  | $i$ | $i$ | $i$ | $i$ | $i$ | $i$ | $i$ | $i$ | $i$ | $-i$ | $-i$ | $-i$ | $-i$ | $-i$ | $-i$ | $-i$ | $-i$ | 1   | 1   | 1   | -1  | -1  | -1  |     |
| Landau | A1  | A1  | A1  | A1  | A1  | A1  | B1  | B1  | B1  | B1  | B1  | B1  | E   | E   | E   | E   | E   | E   | E   | E   | E   | E    | E    | E    | E    | E    | E    | E    | E    | E   | A2  | A2  | A2  | B2  | B2  | B2  |

$$S = 1, \mathbf{n}_{\text{occ.}} = \{0, 4, 0, 0\}$$

$$\left( \begin{array}{cccccccccc} \text{State} & 688 & 689 & 690 & 691 & 692 & 693 & 694 & 695 & 696 \\ \text{Sz} & 1 & 0 & -1 & 1 & 0 & -1 & 1 & 0 & -1 \\ \text{Rx} & 1 & 1 & 1 & 0 & 0 & 0 & 0 & 0 & 0 \\ \text{Ry} & 1 & 1 & 1 & 0 & 0 & 0 & 0 & 0 & 0 \\ \text{R} & -1 & -1 & -1 & i & i & i & -i & -i & -i \\ \text{Landau} & \text{B1} & \text{B1} & \text{B1} & \text{E} & \text{E} & \text{E} & \text{E} & \text{E} & \text{E} \end{array} \right)$$

$$S = 1, \text{ n}_{\text{occ.}} = \{0, 2, 2, 0\}$$

|  |        |     |     |     |     |     |     |     |     |     |     |     |     |     |     |     |     |     |     |   |
|--|--------|-----|-----|-----|-----|-----|-----|-----|-----|-----|-----|-----|-----|-----|-----|-----|-----|-----|-----|---|
|  | State  | 697 | 698 | 699 | 700 | 701 | 702 | 703 | 704 | 705 | 706 | 707 | 708 | 709 | 710 | 711 | 712 | 713 | 714 | \ |
|  | Sz     | 1   | 0   | -1  | 1   | 0   | -1  | 1   | 0   | -1  | 1   | 0   | -1  | 1   | 0   | -1  | 1   | 0   | -1  |   |
|  | Rx     | 1   | 1   | 1   | 1   | 1   | 1   | 1   | 1   | 1   | 0   | 0   | 0   | 0   | 0   | 0   | -1  | -1  | -1  |   |
|  | Ry     | 1   | 1   | 1   | 1   | 1   | 1   | 1   | 1   | 1   | 0   | 0   | 0   | 0   | 0   | 0   | -1  | -1  | -1  |   |
|  | R      | 1   | 1   | 1   | 1   | 1   | 1   | -1  | -1  | -1  | i   | i   | i   | -i  | -i  | -i  | -1  | -1  | -1  |   |
|  | Landau | A1  | A1  | A1  | A1  | A1  | A1  | B1  | B1  | B1  | E   | E   | E   | E   | E   | E   | B2  | B2  | B2  | / |

$$\mathbf{S} = \mathbf{1}, \mathbf{n}_{\text{occ.}} = \{\mathbf{0}, \mathbf{2}, \mathbf{1}, \mathbf{1}\}$$

| State  | 715 | 716 | 717 | 718 | 719 | 720 | 721 | 722 | 723 | 724 | 725 | 726 | 727      | 728      | 729      | 730      | 731      | 732      | 733      | 734      | 735      | 736      | 737        | 738        | 739        | 740        | 741        | 742        | 743        | 744        | 745 | 746 | 747 | 748 | 749 | 750 |    |
|--------|-----|-----|-----|-----|-----|-----|-----|-----|-----|-----|-----|-----|----------|----------|----------|----------|----------|----------|----------|----------|----------|----------|------------|------------|------------|------------|------------|------------|------------|------------|-----|-----|-----|-----|-----|-----|----|
| Sz     | 1   | 0   | -1  | 1   | 0   | -1  | 1   | 0   | -1  | 1   | 0   | -1  | 1        | 0        | -1       | 1        | 0        | -1       | 1        | 0        | -1       | 1        | 0          | -1         | 1          | 0          | -1         | 1          | 0          | -1         | 1   | 0   | -1  | 1   | 0   | -1  |    |
| Rx     | 1   | 1   | 1   | 1   | 1   | 1   | 1   | 1   | 1   | 1   | 1   | 1   | 0        | 0        | 0        | 0        | 0        | 0        | 0        | 0        | 0        | 0        | 0          | 0          | 0          | 0          | 0          | 0          | 0          | 0          | -1  | -1  | -1  | -1  | -1  | -1  |    |
| Ry     | 1   | 1   | 1   | 1   | 1   | 1   | 1   | 1   | 1   | 1   | 1   | 1   | 0        | 0        | 0        | 0        | 0        | 0        | 0        | 0        | 0        | 0        | 0          | 0          | 0          | 0          | 0          | 0          | 0          | 0          | 0   | -1  | -1  | -1  | -1  | -1  | -1 |
| R      | 1   | 1   | 1   | 1   | 1   | 1   | -1  | -1  | -1  | -1  | -1  | -1  | <i>i</i> | <i>i</i> | <i>i</i> | <i>i</i> | <i>i</i> | <i>i</i> | <i>i</i> | <i>i</i> | <i>i</i> | <i>i</i> | - <i>i</i> | - <i>i</i> | - <i>i</i> | - <i>i</i> | - <i>i</i> | - <i>i</i> | - <i>i</i> | - <i>i</i> | 1   | 1   | 1   | -1  | -1  | -1  |    |
| Landau | A1  | A1  | A1  | A1  | A1  | A1  | B1  | B1  | B1  | B1  | B1  | B1  | E        | E        | E        | E        | E        | E        | E        | E        | E        | E        | E          | E          | E          | E          | E          | E          | E          | E          | A2  | A2  | A2  | B2  | B2  | B2  |    |

$$S = 1, \text{ n}_{\text{occ.}} = \{0, 2, 0, 2\}$$

[illegible]

$$\mathbf{S} = 1/2, \mathbf{n}_{\text{occ.}} = \{3, 0, 1, 0\}$$

| State  | 769           | 770            | 771           | 772            | 773           | 774            | 775           | 776            | 777           | 778            | 779           | 780            | 781           | 782            | 783           | 784            |    |    |
|--------|---------------|----------------|---------------|----------------|---------------|----------------|---------------|----------------|---------------|----------------|---------------|----------------|---------------|----------------|---------------|----------------|----|----|
| Sz     | $\frac{1}{2}$ | $-\frac{1}{2}$ | $\frac{1}{2}$ | $-\frac{1}{2}$ | $\frac{1}{2}$ | $-\frac{1}{2}$ | $\frac{1}{2}$ | $-\frac{1}{2}$ | $\frac{1}{2}$ | $-\frac{1}{2}$ | $\frac{1}{2}$ | $-\frac{1}{2}$ | $\frac{1}{2}$ | $-\frac{1}{2}$ | $\frac{1}{2}$ | $-\frac{1}{2}$ |    |    |
| Rx     | 1             | 1              | 1             | 1              | 0             | 0              | 0             | 0              | 0             | 0              | 0             | 0              | -1            | -1             | -1            | -1             |    |    |
| Ry     | 1             | 1              | 1             | 1              | 0             | 0              | 0             | 0              | 0             | 0              | 0             | 0              | -1            | -1             | -1            | -1             |    |    |
| R      | 1             | 1              | -1            | -1             | $i$           | $i$            | $i$           | $i$            | $-i$          | $-i$           | $-i$          | $-i$           | 1             | 1              | -1            | -1             |    |    |
| Landau | A1            | A1             | B1            | B1             | E             | E              | E             | E              | E             | E              | E             | E              | E             | E              | A2            | A2             | B2 | B2 |

$$\mathbf{S} = 1/2, \text{ n}_{\text{occ.}} = \{3, 0, 0, 1\}$$

| State  | 785           | 786            | 787           | 788            | 789           | 790            | 791           | 792            | 793           | 794            | 795           | 796            | 797           | 798            | 799           | 800            |
|--------|---------------|----------------|---------------|----------------|---------------|----------------|---------------|----------------|---------------|----------------|---------------|----------------|---------------|----------------|---------------|----------------|
| Sz     | $\frac{1}{2}$ | $-\frac{1}{2}$ | $\frac{1}{2}$ | $-\frac{1}{2}$ | $\frac{1}{2}$ | $-\frac{1}{2}$ | $\frac{1}{2}$ | $-\frac{1}{2}$ | $\frac{1}{2}$ | $-\frac{1}{2}$ | $\frac{1}{2}$ | $-\frac{1}{2}$ | $\frac{1}{2}$ | $-\frac{1}{2}$ | $\frac{1}{2}$ | $-\frac{1}{2}$ |
| Rx     | 1             | 1              | 1             | 1              | 0             | 0              | 0             | 0              | 0             | 0              | 0             | 0              | 0             | -1             | -1            | -1             |
| Ry     | 1             | 1              | 1             | 1              | 0             | 0              | 0             | 0              | 0             | 0              | 0             | 0              | 0             | -1             | -1            | -1             |
| R      | 1             | 1              | -1            | -1             | $i$           | $i$            | $i$           | $i$            | $-i$          | $-i$           | $-i$          | $-i$           | 1             | 1              | -1            | -1             |
| Landau | A1            | A1             | B1            | B1             | E             | E              | E             | E              | E             | E              | E             | E              | E             | A2             | A2            | B2             |



$\mathbf{S} = \mathbf{1}/\mathbf{2}, \mathbf{n}_{\text{occ.}} = \{\mathbf{2}, \mathbf{1}, \mathbf{1}, \mathbf{0}\}$

  

|  |        |               |                |               |                |               |                |               |                |               |                |               |                |               |                |               |                |               |                |               |                |               |                |               |                |               |                |               |                |               |                |               |                |               |                |               |                |               |                |               |                |               |                |               |                |               |                |     |     |    |    |
|--|--------|---------------|----------------|---------------|----------------|---------------|----------------|---------------|----------------|---------------|----------------|---------------|----------------|---------------|----------------|---------------|----------------|---------------|----------------|---------------|----------------|---------------|----------------|---------------|----------------|---------------|----------------|---------------|----------------|---------------|----------------|---------------|----------------|---------------|----------------|---------------|----------------|---------------|----------------|---------------|----------------|---------------|----------------|---------------|----------------|---------------|----------------|-----|-----|----|----|
|  | State  | 801           | 802            | 803           | 804            | 805           | 806            | 807           | 808            | 809           | 810            | 811           | 812            | 813           | 814            | 815           | 816            | 817           | 818            | 819           | 820            | 821           | 822            | 823           | 824            | 825           | 826            | 827           | 828            | 829           | 830            | 831           | 832            | 833           | 834            | 835           | 836            | 837           | 838            | 839           | 840            | 841           | 842            | 843           | 844            | 845           | 846            | 847 | 848 |    |    |
|  | Sz     | $\frac{1}{2}$ | $-\frac{1}{2}$ | $\frac{1}{2}$ | $-\frac{1}{2}$ | $\frac{1}{2}$ | $-\frac{1}{2}$ | $\frac{1}{2}$ | $-\frac{1}{2}$ | $\frac{1}{2}$ | $-\frac{1}{2}$ | $\frac{1}{2}$ | $-\frac{1}{2}$ | $\frac{1}{2}$ | $-\frac{1}{2}$ | $\frac{1}{2}$ | $-\frac{1}{2}$ | $\frac{1}{2}$ | $-\frac{1}{2}$ | $\frac{1}{2}$ | $-\frac{1}{2}$ | $\frac{1}{2}$ | $-\frac{1}{2}$ | $\frac{1}{2}$ | $-\frac{1}{2}$ | $\frac{1}{2}$ | $-\frac{1}{2}$ | $\frac{1}{2}$ | $-\frac{1}{2}$ | $\frac{1}{2}$ | $-\frac{1}{2}$ | $\frac{1}{2}$ | $-\frac{1}{2}$ | $\frac{1}{2}$ | $-\frac{1}{2}$ | $\frac{1}{2}$ | $-\frac{1}{2}$ | $\frac{1}{2}$ | $-\frac{1}{2}$ | $\frac{1}{2}$ | $-\frac{1}{2}$ | $\frac{1}{2}$ | $-\frac{1}{2}$ | $\frac{1}{2}$ | $-\frac{1}{2}$ | $\frac{1}{2}$ | $-\frac{1}{2}$ |     |     |    |    |
|  | Rx     | 1             | 1              | 1             | 1              | 1             | 1              | 1             | 1              | 1             | 1              | 1             | 1              | 0             | 0              | 0             | 0              | 0             | 0              | 0             | 0              | 0             | 0              | 0             | 0              | 0             | 0              | 0             | 0              | 0             | 0              | 0             | 0              | 0             | 0              | 0             | -1             | -1            | -1             | -1            | -1             | -1            | -1             | -1            | -1             | -1            | -1             | -1  |     |    |    |
|  | Ry     | 1             | 1              | 1             | 1              | 1             | 1              | 1             | 1              | 1             | 1              | 1             | 1              | 0             | 0              | 0             | 0              | 0             | 0              | 0             | 0              | 0             | 0              | 0             | 0              | 0             | 0              | 0             | 0              | 0             | 0              | 0             | 0              | 0             | 0              | 0             | 0              | 0             | -1             | -1            | -1             | -1            | -1             | -1            | -1             | -1            | -1             | -1  | -1  |    |    |
|  | R      | 1             | 1              | 1             | 1              | 1             | 1              | -1            | -1             | -1            | -1             | -1            | -1             | i             | i              | i             | i              | i             | i              | i             | i              | i             | i              | i             | i              | i             | -i             | -i            | -i             | -i            | -i             | -i            | -i             | -i            | -i             | -i            | -i             | -i            | 1              | 1             | 1              | 1             | 1              | 1             | -1             | -1            | -1             | -1  | -1  | -1 |    |
|  | Landau | A1            | A1             | A1            | A1             | A1            | A1             | B1            | B1             | B1            | B1             | B1            | B1             | E             | E              | E             | E              | E             | E              | E             | E              | E             | E              | E             | E              | E             | E              | E             | E              | E             | E              | E             | E              | E             | E              | E             | E              | E             | A2             | A2            | A2             | A2            | A2             | A2            | B2             | B2            | B2             | B2  | B2  | B2 | B2 |



$\mathbf{S} = \mathbf{1}/\mathbf{2}, \mathbf{n}_{\text{occ.}} = \{\mathbf{1}, \mathbf{2}, \mathbf{1}, \mathbf{0}\}$   
  

|        | 897 | 898           | 899            | 900           | 901            | 902           | 903            | 904           | 905            | 906           | 907            | 908           | 909            | 910           | 911            | 912           | 913            | 914           | 915            | 916           | 917            | 918           | 919            | 920           | 921            | 922           | 923            | 924           | 925            | 926           | 927            | 928           | 929            | 930           | 931            | 932           | 933            | 934           | 935            | 936           | 937            | 938           | 939            | 940           | 941            | 942 | 943 | 944 |
|--------|-----|---------------|----------------|---------------|----------------|---------------|----------------|---------------|----------------|---------------|----------------|---------------|----------------|---------------|----------------|---------------|----------------|---------------|----------------|---------------|----------------|---------------|----------------|---------------|----------------|---------------|----------------|---------------|----------------|---------------|----------------|---------------|----------------|---------------|----------------|---------------|----------------|---------------|----------------|---------------|----------------|---------------|----------------|---------------|----------------|-----|-----|-----|
| State  | Sz  | $\frac{1}{2}$ | $-\frac{1}{2}$ | $\frac{1}{2}$ | $-\frac{1}{2}$ | $\frac{1}{2}$ | $-\frac{1}{2}$ | $\frac{1}{2}$ | $-\frac{1}{2}$ | $\frac{1}{2}$ | $-\frac{1}{2}$ | $\frac{1}{2}$ | $-\frac{1}{2}$ | $\frac{1}{2}$ | $-\frac{1}{2}$ | $\frac{1}{2}$ | $-\frac{1}{2}$ | $\frac{1}{2}$ | $-\frac{1}{2}$ | $\frac{1}{2}$ | $-\frac{1}{2}$ | $\frac{1}{2}$ | $-\frac{1}{2}$ | $\frac{1}{2}$ | $-\frac{1}{2}$ | $\frac{1}{2}$ | $-\frac{1}{2}$ | $\frac{1}{2}$ | $-\frac{1}{2}$ | $\frac{1}{2}$ | $-\frac{1}{2}$ | $\frac{1}{2}$ | $-\frac{1}{2}$ | $\frac{1}{2}$ | $-\frac{1}{2}$ | $\frac{1}{2}$ | $-\frac{1}{2}$ | $\frac{1}{2}$ | $-\frac{1}{2}$ | $\frac{1}{2}$ | $-\frac{1}{2}$ | $\frac{1}{2}$ | $-\frac{1}{2}$ | $\frac{1}{2}$ | $-\frac{1}{2}$ |     |     |     |
| Rx     | 1   | 1             | 1              | 1             | 1              | 1             | 1              | 1             | 1              | 1             | 1              | 1             | 0              | 0             | 0              | 0             | 0              | 0             | 0              | 0             | 0              | 0             | 0              | 0             | 0              | 0             | 0              | 0             | 0              | 0             | 0              | 0             | 0              | 0             | -1             | -1            | -1             | -1            | -1             | -1            | -1             | -1            | -1             | -1            | -1             | -1  |     |     |
| Ry     | 1   | 1             | 1              | 1             | 1              | 1             | 1              | 1             | 1              | 1             | 1              | 1             | 0              | 0             | 0              | 0             | 0              | 0             | 0              | 0             | 0              | 0             | 0              | 0             | 0              | 0             | 0              | 0             | 0              | 0             | 0              | 0             | 0              | 0             | -1             | -1            | -1             | -1            | -1             | -1            | -1             | -1            | -1             | -1            | -1             | -1  |     |     |
| R      | 1   | 1             | 1              | 1             | 1              | 1             | -1             | -1            | -1             | -1            | -1             | -1            | i              | i             | i              | i             | i              | i             | i              | i             | i              | i             | i              | i             | -i             | -i            | -i             | -i            | -i             | -i            | -i             | -i            | -i             | -i            | 1              | 1             | 1              | 1             | 1              | 1             | -1             | -1            | -1             | -1            | -1             | -1  |     |     |
| Landau | A1  | A1            | A1             | A1            | A1             | A1            | B1             | B1            | B1             | B1            | B1             | B1            | E              | E             | E              | E             | E              | E             | E              | E             | E              | E             | E              | E             | E              | E             | E              | E             | E              | E             | E              | E             | E              | E             | E              | A2            | A2             | A2            | A2             | A2            | A2             | B2            | B2             | B2            | B2             | B2  | B2  |     |

[illegible]

$$\mathbf{S} = \mathbf{1}/\mathbf{2}, \mathbf{n}_{\text{occ.}} = \{\mathbf{1}, \mathbf{0}, \mathbf{3}, \mathbf{0}\}$$

| State  | 993           | 994            | 995           | 996            | 997           | 998            | 999           | 1000           |
|--------|---------------|----------------|---------------|----------------|---------------|----------------|---------------|----------------|
| Sz     | $\frac{1}{2}$ | $-\frac{1}{2}$ | $\frac{1}{2}$ | $-\frac{1}{2}$ | $\frac{1}{2}$ | $-\frac{1}{2}$ | $\frac{1}{2}$ | $-\frac{1}{2}$ |
| Rx     | 1             | 1              | 1             | 1              | 0             | 0              | 0             | 0              |
| Ry     | 1             | 1              | 1             | 1              | 0             | 0              | 0             | 0              |
| R      | 1             | 1              | -1            | -1             | $i$           | $i$            | $-i$          | $-i$           |
| Landau | A1            | A1             | B1            | B1             | E             | E              | E             | E              |

$$\mathbf{S} = \mathbf{1}/2, \mathbf{n}_{\text{occ.}} = \{\mathbf{1}, \mathbf{0}, \mathbf{2}, \mathbf{1}\}$$

| State  | 1001          | 1002           | 1003          | 1004           | 1005          | 1006           | 1007          | 1008           | 1009          | 1010           | 1011          | 1012           | 1013          | 1014           | 1015          | 1016           | 1017          | 1018           | 1019          | 1020           | 1021          | 1022           | 1023          | 1024           |
|--------|---------------|----------------|---------------|----------------|---------------|----------------|---------------|----------------|---------------|----------------|---------------|----------------|---------------|----------------|---------------|----------------|---------------|----------------|---------------|----------------|---------------|----------------|---------------|----------------|
| Sz     | $\frac{1}{2}$ | $-\frac{1}{2}$ | $\frac{1}{2}$ | $-\frac{1}{2}$ | $\frac{1}{2}$ | $-\frac{1}{2}$ | $\frac{1}{2}$ | $-\frac{1}{2}$ | $\frac{1}{2}$ | $-\frac{1}{2}$ | $\frac{1}{2}$ | $-\frac{1}{2}$ | $\frac{1}{2}$ | $-\frac{1}{2}$ | $\frac{1}{2}$ | $-\frac{1}{2}$ | $\frac{1}{2}$ | $-\frac{1}{2}$ | $\frac{1}{2}$ | $-\frac{1}{2}$ | $\frac{1}{2}$ | $-\frac{1}{2}$ | $\frac{1}{2}$ | $-\frac{1}{2}$ |
| Rx     | 1             | 1              | 1             | 1              | 1             | 1              | 1             | 1              | 0             | 0              | 0             | 0              | 0             | 0              | 0             | 0              | 0             | 0              | 0             | 0              | -1            | -1             | -1            | -1             |
| Ry     | 1             | 1              | 1             | 1              | 1             | 1              | 1             | 1              | 0             | 0              | 0             | 0              | 0             | 0              | 0             | 0              | 0             | 0              | 0             | 0              | -1            | -1             | -1            | -1             |
| R      | 1             | 1              | 1             | 1              | -1            | -1             | -1            | -1             | $i$           | $i$            | $i$           | $i$            | $i$           | $i$            | $-i$          | $-i$           | $-i$          | $-i$           | $-i$          | $-i$           | 1             | 1              | -1            | -1             |
| Landau | A1            | A1             | A1            | A1             | B1            | B1             | B1            | B1             | E             | E              | E             | E              | E             | E              | E             | E              | E             | E              | E             | E              | A2            | A2             | B2            | B2             |

$$\mathbf{S} = \mathbf{1}/2, \mathbf{n}_{\text{occ.}} = \{\mathbf{1}, \mathbf{0}, \mathbf{1}, \mathbf{2}\}$$

| State  | 1025          | 1026           | 1027          | 1028           | 1029          | 1030           | 1031          | 1032           | 1033          | 1034           | 1035          | 1036           | 1037          | 1038           | 1039          | 1040           | 1041          | 1042           | 1043          | 1044           | 1045          | 1046           | 1047          | 1048           |
|--------|---------------|----------------|---------------|----------------|---------------|----------------|---------------|----------------|---------------|----------------|---------------|----------------|---------------|----------------|---------------|----------------|---------------|----------------|---------------|----------------|---------------|----------------|---------------|----------------|
| Sz     | $\frac{1}{2}$ | $-\frac{1}{2}$ | $\frac{1}{2}$ | $-\frac{1}{2}$ | $\frac{1}{2}$ | $-\frac{1}{2}$ | $\frac{1}{2}$ | $-\frac{1}{2}$ | $\frac{1}{2}$ | $-\frac{1}{2}$ | $\frac{1}{2}$ | $-\frac{1}{2}$ | $\frac{1}{2}$ | $-\frac{1}{2}$ | $\frac{1}{2}$ | $-\frac{1}{2}$ | $\frac{1}{2}$ | $-\frac{1}{2}$ | $\frac{1}{2}$ | $-\frac{1}{2}$ | $\frac{1}{2}$ | $-\frac{1}{2}$ | $\frac{1}{2}$ | $-\frac{1}{2}$ |
| Rx     | 1             | 1              | 1             | 1              | 1             | 1              | 1             | 1              | 0             | 0              | 0             | 0              | 0             | 0              | 0             | 0              | 0             | 0              | 0             | 0              | -1            | -1             | -1            | -1             |
| Ry     | 1             | 1              | 1             | 1              | 1             | 1              | 1             | 1              | 0             | 0              | 0             | 0              | 0             | 0              | 0             | 0              | 0             | 0              | 0             | 0              | -1            | -1             | -1            | -1             |
| R      | 1             | 1              | 1             | 1              | -1            | -1             | -1            | -1             | $i$           | $i$            | $i$           | $i$            | $i$           | $i$            | $-i$          | $-i$           | $-i$          | $-i$           | $-i$          | $-i$           | 1             | 1              | -1            | -1             |
| Landau | A1            | A1             | A1            | A1             | B1            | B1             | B1            | B1             | E             | E              | E             | E              | E             | E              | E             | E              | E             | E              | E             | E              | A2            | A2             | B2            | B2             |

$$\mathbf{S} = 1/2, \mathbf{n}_{\text{occ.}} = \{1, 0, 0, 3\}$$

$$\left( \begin{array}{ccc} \text{State} & 1049 & 1050 \\ \text{Sz} & \frac{1}{2} & -\frac{1}{2} \\ \text{Rx} & 1 & 1 \\ \text{Ry} & 1 & 1 \\ \text{R} & 1 & 1 \\ \text{Landau} & \text{A1} & \text{A1} \end{array} \right)$$



$$\mathbf{S} = \mathbf{1}/\mathbf{2}, \text{ n}_{\text{occ.}} = \{\mathbf{0}, \mathbf{3}, \mathbf{1}, \mathbf{0}\}$$

$$\left( \begin{array}{ccc} \text{State} & 1051 & 1052 \\ \text{Sz} & \frac{1}{2} & -\frac{1}{2} \\ \text{Rx} & 1 & 1 \\ \text{Ry} & 1 & 1 \\ \text{R} & 1 & 1 \\ \text{Landau} & \text{A1} & \text{A1} \end{array} \right)$$

$$\mathbf{S} = \mathbf{1}/\mathbf{2}, \text{ n}_{\text{occ.}} = \{\mathbf{1}, \mathbf{0}, \mathbf{0}, \mathbf{3}\}$$

$$\left( \begin{array}{ccc} \text{State} & 1053 & 1054 \\ \text{Sz} & \frac{1}{2} & -\frac{1}{2} \\ \text{Rx} & 1 & 1 \\ \text{Ry} & 1 & 1 \\ \text{R} & -1 & -1 \\ \text{Landau} & \text{B1} & \text{B1} \end{array} \right)$$

$$\mathbf{S} = \mathbf{1}/\mathbf{2}, \text{ } \mathbf{n}_{\text{occ.}} = \{\mathbf{0}, \mathbf{3}, \mathbf{1}, \mathbf{0}\}$$

$$\left( \begin{array}{ccc} \text{State} & 1055 & 1056 \\ \text{Sz} & \frac{1}{2} & -\frac{1}{2} \\ \text{Rx} & 1 & 1 \\ \text{Ry} & 1 & 1 \\ \text{R} & -1 & -1 \\ \text{Landau} & \text{B1} & \text{B1} \end{array} \right)$$

$$\mathbf{S} = 1/2, \mathbf{n}_{\text{occ.}} = \{1, 0, 0, 3\}$$

$$\left( \begin{array}{ccc} \text{State} & 1057 & 1058 \\ \text{Sz} & \frac{1}{2} & -\frac{1}{2} \\ \text{Rx} & 0 & 0 \\ \text{Ry} & 0 & 0 \\ \text{R} & i & i \\ \text{Landau} & \text{E} & \text{E} \end{array} \right)$$

$$\mathbf{S} = \mathbf{1}/2, \mathbf{n}_{\text{occ.}} = \{\mathbf{0}, \mathbf{3}, \mathbf{1}, \mathbf{0}\}$$

| State  | 1059          | 1060           | 1061          | 1062           |
|--------|---------------|----------------|---------------|----------------|
| Sz     | $\frac{1}{2}$ | $-\frac{1}{2}$ | $\frac{1}{2}$ | $-\frac{1}{2}$ |
| Rx     | 0             | 0              | 0             | 0              |
| Ry     | 0             | 0              | 0             | 0              |
| R      | $i$           | $i$            | $i$           | $i$            |
| Landau | E             | E              | E             | E              |

$$\mathbf{S} = \mathbf{1}/\mathbf{2}, \text{ n}_{\text{occ.}} = \{1, 0, 0, 3\}$$

$$\left( \begin{array}{ccc} \text{State} & 1063 & 1064 \\ \text{Sz} & \frac{1}{2} & -\frac{1}{2} \\ \text{Rx} & 0 & 0 \\ \text{Ry} & 0 & 0 \\ \text{R} & -i & -i \\ \text{Landau} & \text{E} & \text{E} \end{array} \right)$$

$$\mathbf{S} = \mathbf{1}/\mathbf{2}, \mathbf{n}_{\text{occ.}} = \{\mathbf{0}, \mathbf{3}, \mathbf{1}, \mathbf{0}\}$$

| State  | 1065          | 1066           | 1067          | 1068           | 1069          | 1070           | 1071          | 1072           |
|--------|---------------|----------------|---------------|----------------|---------------|----------------|---------------|----------------|
| Sz     | $\frac{1}{2}$ | $-\frac{1}{2}$ | $\frac{1}{2}$ | $-\frac{1}{2}$ | $\frac{1}{2}$ | $-\frac{1}{2}$ | $\frac{1}{2}$ | $-\frac{1}{2}$ |
| Rx     | 0             | 0              | 0             | 0              | -1            | -1             | -1            | -1             |
| Ry     | 0             | 0              | 0             | 0              | -1            | -1             | -1            | -1             |
| R      | $-i$          | $-i$           | $-i$          | $-i$           | 1             | 1              | -1            | -1             |
| Landau | E             | E              | E             | E              | A2            | A2             | B2            | B2             |

$$\mathbf{S} = \mathbf{1}/2, \mathbf{n}_{\text{occ.}} = \{\mathbf{0}, \mathbf{3}, \mathbf{0}, \mathbf{1}\}$$

| State  | 1073          | 1074           | 1075          | 1076           | 1077          | 1078           | 1079          | 1080           | 1081          | 1082           | 1083          | 1084           | 1085          | 1086           | 1087          | 1088           |
|--------|---------------|----------------|---------------|----------------|---------------|----------------|---------------|----------------|---------------|----------------|---------------|----------------|---------------|----------------|---------------|----------------|
| Sz     | $\frac{1}{2}$ | $-\frac{1}{2}$ | $\frac{1}{2}$ | $-\frac{1}{2}$ | $\frac{1}{2}$ | $-\frac{1}{2}$ | $\frac{1}{2}$ | $-\frac{1}{2}$ | $\frac{1}{2}$ | $-\frac{1}{2}$ | $\frac{1}{2}$ | $-\frac{1}{2}$ | $\frac{1}{2}$ | $-\frac{1}{2}$ | $\frac{1}{2}$ | $-\frac{1}{2}$ |
| Rx     | 1             | 1              | 1             | 1              | 0             | 0              | 0             | 0              | 0             | 0              | 0             | 0              | -1            | -1             | -1            | -1             |
| Ry     | 1             | 1              | 1             | 1              | 0             | 0              | 0             | 0              | 0             | 0              | 0             | 0              | -1            | -1             | -1            | -1             |
| R      | 1             | 1              | -1            | -1             | $i$           | $i$            | $i$           | $i$            | $-i$          | $-i$           | $-i$          | $-i$           | 1             | 1              | -1            | -1             |
| Landau | A1            | A1             | B1            | B1             | E             | E              | E             | E              | E             | E              | E             | E              | A2            | A2             | B2            | B2             |



$$\mathbf{S} = \mathbf{1}/\mathbf{2}, \text{ n}_{\text{occ.}} = \{\mathbf{0}, \mathbf{1}, \mathbf{3}, \mathbf{0}\}$$

$$\left( \begin{array}{c|cccccccc} \text{State} & 1089 & 1090 & 1091 & 1092 & 1093 & 1094 & 1095 & 1096 \\ \hline \text{Sz} & \frac{1}{2} & -\frac{1}{2} & \frac{1}{2} & -\frac{1}{2} & \frac{1}{2} & -\frac{1}{2} & \frac{1}{2} & -\frac{1}{2} \\ \text{Rx} & 1 & 1 & 1 & 1 & 0 & 0 & 0 & 0 \\ \text{Ry} & 1 & 1 & 1 & 1 & 0 & 0 & 0 & 0 \\ \text{R} & 1 & 1 & -1 & -1 & i & i & -i & -i \\ \text{Landau} & \text{A1} & \text{A1} & \text{B1} & \text{B1} & \text{E} & \text{E} & \text{E} & \text{E} \end{array} \right)$$

$$\mathbf{S} = \mathbf{1}/2, \mathbf{n}_{\text{occ.}} = \{\mathbf{0}, \mathbf{1}, \mathbf{2}, \mathbf{1}\}$$

| State  | 1097          | 1098           | 1099          | 1100           | 1101          | 1102           | 1103          | 1104           | 1105          | 1106           | 1107          | 1108           | 1109          | 1110           | 1111          | 1112           | 1113          | 1114           | 1115          | 1116           | 1117          | 1118           | 1119          | 1120           |
|--------|---------------|----------------|---------------|----------------|---------------|----------------|---------------|----------------|---------------|----------------|---------------|----------------|---------------|----------------|---------------|----------------|---------------|----------------|---------------|----------------|---------------|----------------|---------------|----------------|
| Sz     | $\frac{1}{2}$ | $-\frac{1}{2}$ | $\frac{1}{2}$ | $-\frac{1}{2}$ | $\frac{1}{2}$ | $-\frac{1}{2}$ | $\frac{1}{2}$ | $-\frac{1}{2}$ | $\frac{1}{2}$ | $-\frac{1}{2}$ | $\frac{1}{2}$ | $-\frac{1}{2}$ | $\frac{1}{2}$ | $-\frac{1}{2}$ | $\frac{1}{2}$ | $-\frac{1}{2}$ | $\frac{1}{2}$ | $-\frac{1}{2}$ | $\frac{1}{2}$ | $-\frac{1}{2}$ | $\frac{1}{2}$ | $-\frac{1}{2}$ | $\frac{1}{2}$ | $-\frac{1}{2}$ |
| Rx     | 1             | 1              | 1             | 1              | 1             | 1              | 1             | 1              | 0             | 0              | 0             | 0              | 0             | 0              | 0             | 0              | 0             | 0              | 0             | 0              | -1            | -1             | -1            | -1             |
| Ry     | 1             | 1              | 1             | 1              | 1             | 1              | 1             | 1              | 0             | 0              | 0             | 0              | 0             | 0              | 0             | 0              | 0             | 0              | 0             | 0              | -1            | -1             | -1            | -1             |
| R      | 1             | 1              | 1             | 1              | -1            | -1             | -1            | -1             | $i$           | $i$            | $i$           | $i$            | $i$           | $i$            | $-i$          | $-i$           | $-i$          | $-i$           | $-i$          | $-i$           | 1             | 1              | -1            | -1             |
| Landau | A1            | A1             | A1            | A1             | B1            | B1             | B1            | B1             | E             | E              | E             | E              | E             | E              | E             | E              | E             | E              | E             | E              | A2            | A2             | B2            | B2             |

$$\mathbf{S} = \mathbf{1}/2, \mathbf{n}_{\text{occ.}} = \{\mathbf{0}, \mathbf{1}, \mathbf{1}, \mathbf{2}\}$$

| State  | 1121          | 1122           | 1123          | 1124           | 1125          | 1126           | 1127          | 1128           | 1129          | 1130           | 1131          | 1132           | 1133          | 1134           | 1135          | 1136           | 1137          | 1138           | 1139          | 1140           | 1141          | 1142           | 1143          | 1144           |
|--------|---------------|----------------|---------------|----------------|---------------|----------------|---------------|----------------|---------------|----------------|---------------|----------------|---------------|----------------|---------------|----------------|---------------|----------------|---------------|----------------|---------------|----------------|---------------|----------------|
| Sz     | $\frac{1}{2}$ | $-\frac{1}{2}$ | $\frac{1}{2}$ | $-\frac{1}{2}$ | $\frac{1}{2}$ | $-\frac{1}{2}$ | $\frac{1}{2}$ | $-\frac{1}{2}$ | $\frac{1}{2}$ | $-\frac{1}{2}$ | $\frac{1}{2}$ | $-\frac{1}{2}$ | $\frac{1}{2}$ | $-\frac{1}{2}$ | $\frac{1}{2}$ | $-\frac{1}{2}$ | $\frac{1}{2}$ | $-\frac{1}{2}$ | $\frac{1}{2}$ | $-\frac{1}{2}$ | $\frac{1}{2}$ | $-\frac{1}{2}$ | $\frac{1}{2}$ | $-\frac{1}{2}$ |
| Rx     | 1             | 1              | 1             | 1              | 1             | 1              | 1             | 1              | 0             | 0              | 0             | 0              | 0             | 0              | 0             | 0              | 0             | 0              | 0             | 0              | -1            | -1             | -1            | -1             |
| Ry     | 1             | 1              | 1             | 1              | 1             | 1              | 1             | 1              | 0             | 0              | 0             | 0              | 0             | 0              | 0             | 0              | 0             | 0              | 0             | 0              | -1            | -1             | -1            | -1             |
| R      | 1             | 1              | 1             | 1              | -1            | -1             | -1            | -1             | $i$           | $i$            | $i$           | $i$            | $i$           | $i$            | $-i$          | $-i$           | $-i$          | $-i$           | $-i$          | $-i$           | 1             | 1              | -1            | -1             |
| Landau | A1            | A1             | A1            | A1             | B1            | B1             | B1            | B1             | E             | E              | E             | E              | E             | E              | E             | E              | E             | E              | E             | E              | A2            | A2             | B2            | B2             |

$$\mathbf{S} = \mathbf{1}/\mathbf{2}, \text{ n}_{\text{occ.}} = \{\mathbf{0}, \mathbf{1}, \mathbf{0}, \mathbf{3}\}$$

$$\left( \begin{array}{c|ccccccccc} \text{State} & 1145 & 1146 & 1147 & 1148 & 1149 & 1150 & 1151 & 1152 \\ \hline \text{Sz} & \frac{1}{2} & -\frac{1}{2} & \frac{1}{2} & -\frac{1}{2} & \frac{1}{2} & -\frac{1}{2} & \frac{1}{2} & -\frac{1}{2} \\ \text{Rx} & 1 & 1 & 1 & 1 & 0 & 0 & 0 & 0 \\ \text{Ry} & 1 & 1 & 1 & 1 & 0 & 0 & 0 & 0 \\ \text{R} & 1 & 1 & -1 & -1 & i & i & -i & -i \\ \text{Landau} & \text{A1} & \text{A1} & \text{B1} & \text{B1} & \text{E} & \text{E} & \text{E} & \text{E} \end{array} \right)$$

$$\mathbf{S} = \mathbf{0}, \mathbf{n}_{\text{occ.}} = \{4, 0, 0, 0\}$$

$$\left( \begin{array}{ccc} \text{State} & 1153 & 1154 \\ \text{Sz} & 0 & 0 \\ \text{Rx} & 1 & -1 \\ \text{Ry} & 1 & -1 \\ \text{R} & 1 & -1 \\ \text{Landau} & \text{A1} & \text{B2} \end{array} \right)$$

$$\mathbf{S} = \mathbf{0}, \mathbf{n}_{\text{occ.}} = \{\mathbf{3}, \mathbf{1}, \mathbf{0}, \mathbf{0}\}$$

$$\left( \begin{array}{cccccccccc} \text{State} & 1155 & 1156 & 1157 & 1158 & 1159 & 1160 & 1161 & 1162 \\ \text{Sz} & 0 & 0 & 0 & 0 & 0 & 0 & 0 & 0 \\ \text{Rx} & 1 & 1 & 0 & 0 & 0 & 0 & -1 & -1 \\ \text{Ry} & 1 & 1 & 0 & 0 & 0 & 0 & -1 & -1 \\ \text{R} & 1 & -1 & i & i & -i & -i & 1 & -1 \\ \text{Landau} & \text{A1} & \text{B1} & \text{E} & \text{E} & \text{E} & \text{E} & \text{A2} & \text{B2} \end{array} \right)$$

$$\mathbf{S} = \mathbf{0}, \mathbf{n}_{\text{occ.}} = \{\mathbf{2}, \mathbf{2}, \mathbf{0}, \mathbf{0}\}$$

| State  | 1163 | 1164 | 1165 | 1166 | 1167 | 1168 | 1169 | 1170 | 1171 | 1172 | 1173 | 1174 |
|--------|------|------|------|------|------|------|------|------|------|------|------|------|
| Sz     | 0    | 0    | 0    | 0    | 0    | 0    | 0    | 0    | 0    | 0    | 0    | 0    |
| Rx     | 1    | 1    | 1    | 1    | 0    | 0    | 0    | 0    | -1   | -1   | -1   | -1   |
| Ry     | 1    | 1    | 1    | 1    | 0    | 0    | 0    | 0    | -1   | -1   | -1   | -1   |
| R      | 1    | 1    | 1    | -1   | $i$  | $i$  | $-i$ | $-i$ | 1    | -1   | -1   | -1   |
| Landau | A1   | A1   | A1   | B1   | E    | E    | E    | E    | A2   | B2   | B2   | B2   |

$$\mathbf{S} = \mathbf{0}, \mathbf{n}_{\text{occ.}} = \{\mathbf{2}, \mathbf{0}, \mathbf{2}, \mathbf{0}\}$$

| State  | 1175 | 1176 | 1177 | 1178 | 1179 | 1180 |
|--------|------|------|------|------|------|------|
| Sz     | 0    | 0    | 0    | 0    | 0    | 0    |
| Rx     | 1    | 0    | 0    | 0    | 0    | -1   |
| Ry     | 1    | 0    | 0    | 0    | 0    | -1   |
| R      | -1   | $i$  | $i$  | $-i$ | $-i$ | 1    |
| Landau | B1   | E    | E    | E    | E    | A2   |



$$\mathbf{S} = \mathbf{0}, \mathbf{n}_{\text{occ.}} = \{\mathbf{2}, \mathbf{0}, \mathbf{1}, \mathbf{1}\}$$

| State  | 1181 | 1182 | 1183 | 1184 | 1185 | 1186 | 1187 | 1188 | 1189 | 1190 | 1191 | 1192 |
|--------|------|------|------|------|------|------|------|------|------|------|------|------|
| Sz     | 0    | 0    | 0    | 0    | 0    | 0    | 0    | 0    | 0    | 0    | 0    | 0    |
| Rx     | 1    | 1    | 0    | 0    | 0    | 0    | 0    | 0    | -1   | -1   | -1   | -1   |
| Ry     | 1    | 1    | 0    | 0    | 0    | 0    | 0    | 0    | -1   | -1   | -1   | -1   |
| R      | 1    | -1   | $i$  | $i$  | $i$  | $-i$ | $-i$ | $-i$ | 1    | 1    | -1   | -1   |
| Landau | A1   | B1   | E    | E    | E    | E    | E    | E    | A2   | A2   | B2   | B2   |

$$\mathbf{S} = \mathbf{0}, \mathbf{n}_{\text{occ.}} = \{\mathbf{2}, \mathbf{0}, \mathbf{0}, \mathbf{2}\}$$

| State  | 1193 | 1194 | 1195 | 1196 | 1197 | 1198 |
|--------|------|------|------|------|------|------|
| Sz     | 0    | 0    | 0    | 0    | 0    | 0    |
| Rx     | 1    | 0    | 0    | 0    | 0    | -1   |
| Ry     | 1    | 0    | 0    | 0    | 0    | -1   |
| R      | -1   | $i$  | $i$  | $-i$ | $-i$ | 1    |
| Landau | B1   | E    | E    | E    | E    | A2   |

$$\mathbf{S} = \mathbf{0}, \mathbf{n}_{\text{occ.}} = \{\mathbf{1}, \mathbf{3}, \mathbf{0}, \mathbf{0}\}$$

$$\left( \begin{array}{cccccccccc} \text{State} & 1199 & 1200 & 1201 & 1202 & 1203 & 1204 & 1205 & 1206 \\ \text{Sz} & 0 & 0 & 0 & 0 & 0 & 0 & 0 & 0 \\ \text{Rx} & 1 & 1 & 0 & 0 & 0 & 0 & -1 & -1 \\ \text{Ry} & 1 & 1 & 0 & 0 & 0 & 0 & -1 & -1 \\ \text{R} & 1 & -1 & i & i & -i & -i & 1 & -1 \\ \text{Landau} & A1 & B1 & E & E & E & E & A2 & B2 \end{array} \right)$$

$$\mathbf{S} = \mathbf{0}, \mathbf{n}_{\text{occ.}} = \{1, 1, 2, 0\}$$

| State  | 1207 | 1208 | 1209 | 1210 | 1211 | 1212 | 1213 | 1214 | 1215 | 1216 | 1217 | 1218 |
|--------|------|------|------|------|------|------|------|------|------|------|------|------|
| Sz     | 0    | 0    | 0    | 0    | 0    | 0    | 0    | 0    | 0    | 0    | 0    | 0    |
| Rx     | 1    | 1    | 1    | 1    | 0    | 0    | 0    | 0    | 0    | 0    | -1   | -1   |
| Ry     | 1    | 1    | 1    | 1    | 0    | 0    | 0    | 0    | 0    | 0    | -1   | -1   |
| R      | 1    | 1    | -1   | -1   | $i$  | $i$  | $i$  | $-i$ | $-i$ | $-i$ | 1    | -1   |
| Landau | A1   | A1   | B1   | B1   | E    | E    | E    | E    | E    | E    | A2   | B2   |

$$\mathbf{S} = \mathbf{0}, \mathbf{n}_{\text{occ.}} = \{1, 1, 1, 1\}$$

| State  | 1219 | 1220 | 1221 | 1222 | 1223 | 1224 | 1225 | 1226 | 1227 | 1228 | 1229 | 1230 | 1231 | 1232 | 1233 | 1234 | 1235 | 1236 | 1237 | 1238 | 1239 | 1240 | 1241 | 1242 |
|--------|------|------|------|------|------|------|------|------|------|------|------|------|------|------|------|------|------|------|------|------|------|------|------|------|
| Sz     | 0    | 0    | 0    | 0    | 0    | 0    | 0    | 0    | 0    | 0    | 0    | 0    | 0    | 0    | 0    | 0    | 0    | 0    | 0    | 0    | 0    | 0    | 0    | 0    |
| Rx     | 1    | 1    | 1    | 1    | 1    | 1    | 0    | 0    | 0    | 0    | 0    | 0    | 0    | 0    | 0    | 0    | 0    | 0    | -1   | -1   | -1   | -1   | -1   | -1   |
| Ry     | 1    | 1    | 1    | 1    | 1    | 1    | 0    | 0    | 0    | 0    | 0    | 0    | 0    | 0    | 0    | 0    | 0    | 0    | -1   | -1   | -1   | -1   | -1   | -1   |
| R      | 1    | 1    | 1    | -1   | -1   | -1   | $i$  | $i$  | $i$  | $i$  | $i$  | $i$  | $-i$ | $-i$ | $-i$ | $-i$ | $-i$ | $-i$ | 1    | 1    | 1    | -1   | -1   | -1   |
| Landau | A1   | A1   | A1   | B1   | B1   | B1   | E    | E    | E    | E    | E    | E    | E    | E    | E    | E    | E    | E    | A2   | A2   | A2   | B2   | B2   | B2   |

$$\mathbf{S} = \mathbf{0}, \mathbf{n}_{\text{occ.}} = \{1, 1, 0, 2\}$$

| State  | 1243 | 1244 | 1245 | 1246 | 1247 | 1248 | 1249 | 1250 | 1251 | 1252 | 1253 | 1254 |
|--------|------|------|------|------|------|------|------|------|------|------|------|------|
| Sz     | 0    | 0    | 0    | 0    | 0    | 0    | 0    | 0    | 0    | 0    | 0    | 0    |
| Rx     | 1    | 1    | 1    | 1    | 0    | 0    | 0    | 0    | 0    | 0    | -1   | -1   |
| Ry     | 1    | 1    | 1    | 1    | 0    | 0    | 0    | 0    | 0    | 0    | -1   | -1   |
| R      | 1    | 1    | -1   | -1   | $i$  | $i$  | $i$  | $-i$ | $-i$ | $-i$ | 1    | -1   |
| Landau | A1   | A1   | B1   | B1   | E    | E    | E    | E    | E    | E    | A2   | B2   |

$$\mathbf{S} = \mathbf{0}, \mathbf{n}_{\text{occ.}} = \{0, 4, 0, 0\}$$

$$\left( \begin{array}{ccc} \text{State} & 1255 & 1256 \\ \text{Sz} & 0 & 0 \\ \text{Rx} & 1 & -1 \\ \text{Ry} & 1 & -1 \\ \text{R} & 1 & -1 \\ \text{Landau} & \text{A1} & \text{B2} \end{array} \right)$$

$$\mathbf{S} = \mathbf{0}, \mathbf{n}_{\text{occ.}} = \{\mathbf{0}, \mathbf{2}, \mathbf{2}, \mathbf{0}\}$$

| State  | 1257 | 1258 | 1259 | 1260 | 1261 | 1262 |
|--------|------|------|------|------|------|------|
| Sz     | 0    | 0    | 0    | 0    | 0    | 0    |
| Rx     | 1    | 0    | 0    | 0    | 0    | -1   |
| Ry     | 1    | 0    | 0    | 0    | 0    | -1   |
| R      | -1   | $i$  | $i$  | $-i$ | $-i$ | 1    |
| Landau | B1   | E    | E    | E    | E    | A2   |



$$\mathbf{S} = \mathbf{0}, \mathbf{n}_{\text{occ.}} = \{\mathbf{0}, \mathbf{2}, \mathbf{1}, \mathbf{1}\}$$

| State  | 1263 | 1264 | 1265 | 1266 | 1267 | 1268 | 1269 | 1270 | 1271 | 1272 | 1273 | 1274 |
|--------|------|------|------|------|------|------|------|------|------|------|------|------|
| Sz     | 0    | 0    | 0    | 0    | 0    | 0    | 0    | 0    | 0    | 0    | 0    | 0    |
| Rx     | 1    | 1    | 0    | 0    | 0    | 0    | 0    | 0    | 0    | -1   | -1   | -1   |
| Ry     | 1    | 1    | 0    | 0    | 0    | 0    | 0    | 0    | 0    | -1   | -1   | -1   |
| R      | 1    | -1   | $i$  | $i$  | $i$  | $-i$ | $-i$ | $-i$ | 1    | 1    | -1   | -1   |
| Landau | A1   | B1   | E    | E    | E    | E    | E    | E    | A2   | A2   | B2   | B2   |

$$\mathbf{S} = \mathbf{0}, \mathbf{n}_{\text{occ.}} = \{\mathbf{0}, \mathbf{2}, \mathbf{0}, \mathbf{2}\}$$

| State  | 1275 | 1276 | 1277 | 1278 | 1279 | 1280 |
|--------|------|------|------|------|------|------|
| Sz     | 0    | 0    | 0    | 0    | 0    | 0    |
| Rx     | 1    | 0    | 0    | 0    | 0    | -1   |
| Ry     | 1    | 0    | 0    | 0    | 0    | -1   |
| R      | -1   | $i$  | $i$  | $-i$ | $-i$ | 1    |
| Landau | B1   | E    | E    | E    | E    | A2   |

$$\mathbf{S} = \mathbf{0}, \text{ n}_{\text{occ.}} = \{\mathbf{0}, \mathbf{0}, \mathbf{4}, \mathbf{0}\}$$

$$\left( \begin{array}{cc} \text{State} & 1281 \\ \text{Sz} & 0 \\ \text{Rx} & 1 \\ \text{Ry} & 1 \\ \text{R} & 1 \\ \text{Landau} & \text{A1} \end{array} \right)$$

$$\mathbf{S} = \mathbf{0}, \mathbf{n}_{\text{occ.}} = \{\mathbf{0}, \mathbf{0}, \mathbf{3}, \mathbf{1}\}$$

$$\left( \begin{array}{ccccc} \text{State} & 1282 & 1283 & 1284 & 1285 \\ \text{Sz} & 0 & 0 & 0 & 0 \\ \text{Rx} & 1 & 1 & 0 & 0 \\ \text{Ry} & 1 & 1 & 0 & 0 \\ \text{R} & 1 & -1 & i & -i \\ \text{Landau} & \text{A1} & \text{B1} & \text{E} & \text{E} \end{array} \right)$$

$$\mathbf{S} = \mathbf{0}, \mathbf{n}_{\text{occ.}} = \{\mathbf{0}, \mathbf{0}, \mathbf{2}, \mathbf{2}\}$$

| State  | 1286 | 1287 | 1288 | 1289 | 1290 | 1291 |
|--------|------|------|------|------|------|------|
| Sz     | 0    | 0    | 0    | 0    | 0    | 0    |
| Rx     | 1    | 1    | 1    | 0    | 0    | -1   |
| Ry     | 1    | 1    | 1    | 0    | 0    | -1   |
| R      | 1    | 1    | -1   | $i$  | $-i$ | -1   |
| Landau | A1   | A1   | B1   | E    | E    | B2   |

$$\mathbf{S} = \mathbf{0}, \mathbf{n}_{\text{occ.}} = \{\mathbf{0}, \mathbf{0}, \mathbf{1}, \mathbf{3}\}$$

$$\left( \begin{array}{ccccc} \text{State} & 1292 & 1293 & 1294 & 1295 \\ \text{Sz} & 0 & 0 & 0 & 0 \\ \text{Rx} & 1 & 1 & 0 & 0 \\ \text{Ry} & 1 & 1 & 0 & 0 \\ \text{R} & 1 & -1 & i & -i \\ \text{Landau} & \text{A1} & \text{B1} & \text{E} & \text{E} \end{array} \right)$$

$$\mathbf{S} = \mathbf{0}, \text{ n}_{\text{occ.}} = \{\mathbf{0}, \mathbf{0}, \mathbf{0}, 4\}$$

$$\left( \begin{array}{cc} \text{State} & 1296 \\ \text{Sz} & 0 \\ \text{Rx} & 1 \\ \text{Ry} & 1 \\ \text{R} & 1 \\ \text{Landau} & \text{A1} \end{array} \right)$$

$$\mathbf{S} = \mathbf{2}, \mathbf{n}_{\text{occ.}} = \{4, \mathbf{0}, \mathbf{0}, \mathbf{0}, \mathbf{0}\}$$

$$\left( \begin{array}{ccccc} \text{State} & 1 & 2 & 3 & 4 & 5 \\ \text{Sz} & 2 & 1 & 0 & -1 & -2 \\ \text{Rx} & 1 & 1 & 1 & 1 & 1 \\ \text{Ry} & 1 & 1 & 1 & 1 & 1 \\ \text{R} & 1 & 1 & 1 & 1 & 1 \\ \text{Landau} & \text{A1} & \text{A1} & \text{A1} & \text{A1} & \text{A1} \end{array} \right)$$







$$\mathbf{S} = \mathbf{3}/\mathbf{2}, \mathbf{n}_{\text{occ.}} = \{\mathbf{3}, \mathbf{0}, \mathbf{0}, \mathbf{1}, \mathbf{0}\}$$

| State  | 38            | 39            | 40             | 41             | 42            | 43            | 44             | 45             | 46            | 47            | 48             | 49             | 50            | 51            | 52             | 53             |
|--------|---------------|---------------|----------------|----------------|---------------|---------------|----------------|----------------|---------------|---------------|----------------|----------------|---------------|---------------|----------------|----------------|
| Sz     | $\frac{3}{2}$ | $\frac{1}{2}$ | $-\frac{1}{2}$ | $-\frac{3}{2}$ | $\frac{3}{2}$ | $\frac{1}{2}$ | $-\frac{1}{2}$ | $-\frac{3}{2}$ | $\frac{3}{2}$ | $\frac{1}{2}$ | $-\frac{1}{2}$ | $-\frac{3}{2}$ | $\frac{3}{2}$ | $\frac{1}{2}$ | $-\frac{1}{2}$ | $-\frac{3}{2}$ |
| Rx     | 1             | 1             | 1              | 1              | 1             | 1             | 1              | 1              | 0             | 0             | 0              | 0              | 0             | 0             | 0              | 0              |
| Ry     | 1             | 1             | 1              | 1              | 1             | 1             | 1              | 1              | 0             | 0             | 0              | 0              | 0             | 0             | 0              | 0              |
| R      | 1             | 1             | 1              | 1              | -1            | -1            | -1             | -1             | $i$           | $i$           | $i$            | $i$            | $-i$          | $-i$          | $-i$           | $-i$           |
| Landau | A1            | A1            | A1             | A1             | B1            | B1            | B1             | B1             | E             | E             | E              | E              | E             | E             | E              | E              |

$$\mathbf{S} = \mathbf{3}/\mathbf{2}, \text{ } \mathbf{n}_{\text{occ.}} = \{\mathbf{3}, \mathbf{0}, \mathbf{0}, \mathbf{0}, \mathbf{1}\}$$

| State  | 54            | 55            | 56             | 57             | 58            | 59            | 60             | 61             | 62            | 63            | 64             | 65             | 66            | 67            | 68             | 69             |
|--------|---------------|---------------|----------------|----------------|---------------|---------------|----------------|----------------|---------------|---------------|----------------|----------------|---------------|---------------|----------------|----------------|
| Sz     | $\frac{3}{2}$ | $\frac{1}{2}$ | $-\frac{1}{2}$ | $-\frac{3}{2}$ | $\frac{3}{2}$ | $\frac{1}{2}$ | $-\frac{1}{2}$ | $-\frac{3}{2}$ | $\frac{3}{2}$ | $\frac{1}{2}$ | $-\frac{1}{2}$ | $-\frac{3}{2}$ | $\frac{3}{2}$ | $\frac{1}{2}$ | $-\frac{1}{2}$ | $-\frac{3}{2}$ |
| Rx     | 1             | 1             | 1              | 1              | 1             | 1             | 1              | 1              | 0             | 0             | 0              | 0              | 0             | 0             | 0              | 0              |
| Ry     | 1             | 1             | 1              | 1              | 1             | 1             | 1              | 1              | 0             | 0             | 0              | 0              | 0             | 0             | 0              | 0              |
| R      | 1             | 1             | 1              | 1              | -1            | -1            | -1             | -1             | $i$           | $i$           | $i$            | $i$            | $-i$          | $-i$          | $-i$           | $-i$           |
| Landau | A1            | A1            | A1             | A1             | B1            | B1            | B1             | B1             | E             | E             | E              | E              | E             | E             | E              | E              |



$$\mathbf{S} = \mathbf{1}, \mathbf{n}_{\text{occ.}} = \{\mathbf{2}, \mathbf{2}, \mathbf{0}, \mathbf{0}, \mathbf{0}\}$$

$$\left( \begin{array}{c|cccccccccccccccccccc} \text{State} & 79 & 80 & 81 & 82 & 83 & 84 & 85 & 86 & 87 & 88 & 89 & 90 & 91 & 92 & 93 & 94 & 95 & 96 \\ \hline \text{Sz} & 1 & 0 & -1 & 1 & 0 & -1 & 1 & 0 & -1 & 1 & 0 & -1 & 1 & 0 & -1 & 1 & 0 & -1 \\ \text{Rx} & 1 & 1 & 1 & 1 & 1 & 1 & 1 & 1 & 1 & 0 & 0 & 0 & 0 & 0 & 0 & -1 & -1 & -1 \\ \text{Ry} & 1 & 1 & 1 & 1 & 1 & 1 & 1 & 1 & 1 & 0 & 0 & 0 & 0 & 0 & 0 & -1 & -1 & -1 \\ \text{R} & 1 & 1 & 1 & 1 & 1 & 1 & -1 & -1 & -1 & i & i & i & -i & -i & -i & -1 & -1 & -1 \\ \text{Landau} & \text{A1} & \text{A1} & \text{A1} & \text{A1} & \text{A1} & \text{A1} & \text{B1} & \text{B1} & \text{B1} & \text{E} & \text{E} & \text{E} & \text{E} & \text{E} & \text{E} & \text{B2} & \text{B2} & \text{B2} \end{array} \right)$$

$$\mathbf{S} = \mathbf{1}, \mathbf{n}_{\text{occ.}} = \{\mathbf{2}, \mathbf{1}, \mathbf{1}, \mathbf{0}, \mathbf{0}\}$$

| State  | 97 | 98 | 99 | 100 | 101 | 102 | 103 | 104 | 105 | 106 | 107 | 108 | 109 | 110 | 111 | 112 | 113 | 114 | 115 | 116 | 117 | 118  | 119  | 120  | 121  | 122  | 123  | 124  | 125  | 126  | 127 | 128 | 129 | 130 | 131 | 132 |
|--------|----|----|----|-----|-----|-----|-----|-----|-----|-----|-----|-----|-----|-----|-----|-----|-----|-----|-----|-----|-----|------|------|------|------|------|------|------|------|------|-----|-----|-----|-----|-----|-----|
| Sz     | 1  | 0  | -1 | 1   | 0   | -1  | 1   | 0   | -1  | 1   | 0   | -1  | 1   | 0   | -1  | 1   | 0   | -1  | 1   | 0   | -1  | 1    | 0    | -1   | 1    | 0    | -1   | 1    | 0    | -1   | 1   | 0   | -1  | 1   | 0   | -1  |
| Rx     | 1  | 1  | 1  | 1   | 1   | 1   | 1   | 1   | 1   | 1   | 1   | 1   | 0   | 0   | 0   | 0   | 0   | 0   | 0   | 0   | 0   | 0    | 0    | 0    | 0    | 0    | 0    | 0    | 0    | 0    | -1  | -1  | -1  | -1  | -1  | -1  |
| Ry     | 1  | 1  | 1  | 1   | 1   | 1   | 1   | 1   | 1   | 1   | 1   | 1   | 0   | 0   | 0   | 0   | 0   | 0   | 0   | 0   | 0   | 0    | 0    | 0    | 0    | 0    | 0    | 0    | 0    | 0    | -1  | -1  | -1  | -1  | -1  | -1  |
| R      | 1  | 1  | 1  | 1   | 1   | 1   | -1  | -1  | -1  | -1  | -1  | -1  | $i$ | $i$ | $i$ | $i$ | $i$ | $i$ | $i$ | $i$ | $i$ | $-i$ | $-i$ | $-i$ | $-i$ | $-i$ | $-i$ | $-i$ | $-i$ | $-i$ | 1   | 1   | 1   | -1  | -1  | -1  |
| Landau | A1 | A1 | A1 | A1  | A1  | A1  | B1  | B1  | B1  | B1  | B1  | B1  | E   | E   | E   | E   | E   | E   | E   | E   | E   | E    | E    | E    | E    | E    | E    | E    | E    | E    | A2  | A2  | A2  | B2  | B2  | B2  |

$$\mathbf{S} = \mathbf{1}, \mathbf{n}_{\text{occ.}} = \{\mathbf{2}, \mathbf{1}, \mathbf{0}, \mathbf{1}, \mathbf{0}\}$$

| State  | 133 | 134 | 135 | 136 | 137 | 138 | 139 | 140 | 141 | 142 | 143 | 144 | 145 | 146 | 147 | 148 | 149 | 150 | 151 | 152 | 153 | 154 | 155  | 156  | 157  | 158  | 159  | 160  | 161  | 162  | 163 | 164 | 165 | 166 | 167 | 168 |
|--------|-----|-----|-----|-----|-----|-----|-----|-----|-----|-----|-----|-----|-----|-----|-----|-----|-----|-----|-----|-----|-----|-----|------|------|------|------|------|------|------|------|-----|-----|-----|-----|-----|-----|
| Sz     | 1   | 0   | -1  | 1   | 0   | -1  | 1   | 0   | -1  | 1   | 0   | -1  | 1   | 0   | -1  | 1   | 0   | -1  | 1   | 0   | -1  | 1   | 0    | -1   | 1    | 0    | -1   | 1    | 0    | -1   | 1   | 0   | -1  | 1   | 0   | -1  |
| Rx     | 1   | 1   | 1   | 1   | 1   | 1   | 1   | 1   | 1   | 1   | 1   | 1   | 0   | 0   | 0   | 0   | 0   | 0   | 0   | 0   | 0   | 0   | 0    | 0    | 0    | 0    | 0    | 0    | 0    | 0    | -1  | -1  | -1  | -1  | -1  | -1  |
| Ry     | 1   | 1   | 1   | 1   | 1   | 1   | 1   | 1   | 1   | 1   | 1   | 1   | 0   | 0   | 0   | 0   | 0   | 0   | 0   | 0   | 0   | 0   | 0    | 0    | 0    | 0    | 0    | 0    | 0    | 0    | -1  | -1  | -1  | -1  | -1  | -1  |
| R      | 1   | 1   | 1   | 1   | 1   | 1   | -1  | -1  | -1  | -1  | -1  | -1  | $i$ | $i$ | $i$ | $i$ | $i$ | $i$ | $i$ | $i$ | $i$ | $i$ | $-i$ | $-i$ | $-i$ | $-i$ | $-i$ | $-i$ | $-i$ | $-i$ | 1   | 1   | 1   | -1  | -1  | -1  |
| Landau | A1  | A1  | A1  | A1  | A1  | A1  | B1  | B1  | B1  | B1  | B1  | B1  | E   | E   | E   | E   | E   | E   | E   | E   | E   | E   | E    | E    | E    | E    | E    | E    | E    | E    | A2  | A2  | A2  | B2  | B2  | B2  |



$$\mathbf{S} = \mathbf{1}, \mathbf{n}_{\text{occ.}} = \{\mathbf{2}, \mathbf{1}, \mathbf{0}, \mathbf{0}, \mathbf{1}\}$$

| State  | 169 | 170 | 171 | 172 | 173 | 174 | 175 | 176 | 177 | 178 | 179 | 180 | 181 | 182 | 183 | 184 | 185 | 186 | 187 | 188 | 189 | 190 | 191  | 192  | 193  | 194  | 195  | 196  | 197  | 198  | 199 | 200 | 201 | 202 | 203 | 204 |
|--------|-----|-----|-----|-----|-----|-----|-----|-----|-----|-----|-----|-----|-----|-----|-----|-----|-----|-----|-----|-----|-----|-----|------|------|------|------|------|------|------|------|-----|-----|-----|-----|-----|-----|
| Sz     | 1   | 0   | -1  | 1   | 0   | -1  | 1   | 0   | -1  | 1   | 0   | -1  | 1   | 0   | -1  | 1   | 0   | -1  | 1   | 0   | -1  | 1   | 0    | -1   | 1    | 0    | -1   | 1    | 0    | -1   | 1   | 0   | -1  | 1   | 0   | -1  |
| Rx     | 1   | 1   | 1   | 1   | 1   | 1   | 1   | 1   | 1   | 1   | 1   | 1   | 0   | 0   | 0   | 0   | 0   | 0   | 0   | 0   | 0   | 0   | 0    | 0    | 0    | 0    | 0    | 0    | 0    | 0    | -1  | -1  | -1  | -1  | -1  | -1  |
| Ry     | 1   | 1   | 1   | 1   | 1   | 1   | 1   | 1   | 1   | 1   | 1   | 1   | 0   | 0   | 0   | 0   | 0   | 0   | 0   | 0   | 0   | 0   | 0    | 0    | 0    | 0    | 0    | 0    | 0    | 0    | -1  | -1  | -1  | -1  | -1  | -1  |
| R      | 1   | 1   | 1   | 1   | 1   | 1   | -1  | -1  | -1  | -1  | -1  | -1  | $i$ | $i$ | $i$ | $i$ | $i$ | $i$ | $i$ | $i$ | $i$ | $i$ | $-i$ | $-i$ | $-i$ | $-i$ | $-i$ | $-i$ | $-i$ | $-i$ | 1   | 1   | 1   | -1  | -1  | -1  |
| Landau | A1  | A1  | A1  | A1  | A1  | A1  | B1  | B1  | B1  | B1  | B1  | B1  | E   | E   | E   | E   | E   | E   | E   | E   | E   | E   | E    | E    | E    | E    | E    | E    | E    | E    | A2  | A2  | A2  | B2  | B2  | B2  |

$$S = 1, \text{ n}_{\text{occ.}} = \{2, 0, 2, 0, 0\}$$

[illegible]

$$\mathbf{S} = \mathbf{1}, \mathbf{n}_{\text{occ.}} = \{\mathbf{2}, \mathbf{0}, \mathbf{1}, \mathbf{1}, \mathbf{0}\}$$

| State  | 223 | 224 | 225 | 226 | 227 | 228 | 229 | 230 | 231 | 232 | 233 | 234 | 235 | 236 | 237 | 238 | 239 | 240 | 241 | 242 | 243 | 244 | 245  | 246  | 247  | 248  | 249  | 250  | 251  | 252 | 253 | 254 | 255 | 256 | 257 | 258 |
|--------|-----|-----|-----|-----|-----|-----|-----|-----|-----|-----|-----|-----|-----|-----|-----|-----|-----|-----|-----|-----|-----|-----|------|------|------|------|------|------|------|-----|-----|-----|-----|-----|-----|-----|
| Sz     | 1   | 0   | -1  | 1   | 0   | -1  | 1   | 0   | -1  | 1   | 0   | -1  | 1   | 0   | -1  | 1   | 0   | -1  | 1   | 0   | -1  | 1   | 0    | -1   | 1    | 0    | -1   | 1    | 0    | -1  | 1   | 0   | -1  | 1   | 0   | -1  |
| Rx     | 1   | 1   | 1   | 1   | 1   | 1   | 1   | 1   | 1   | 1   | 1   | 1   | 0   | 0   | 0   | 0   | 0   | 0   | 0   | 0   | 0   | 0   | 0    | 0    | 0    | 0    | 0    | 0    | 0    | 0   | -1  | -1  | -1  | -1  | -1  | -1  |
| Ry     | 1   | 1   | 1   | 1   | 1   | 1   | 1   | 1   | 1   | 1   | 1   | 1   | 0   | 0   | 0   | 0   | 0   | 0   | 0   | 0   | 0   | 0   | 0    | 0    | 0    | 0    | 0    | 0    | 0    | 0   | -1  | -1  | -1  | -1  | -1  | -1  |
| R      | 1   | 1   | 1   | 1   | 1   | 1   | -1  | -1  | -1  | -1  | -1  | -1  | $i$ | $i$ | $i$ | $i$ | $i$ | $i$ | $i$ | $i$ | $i$ | $i$ | $-i$ | $-i$ | $-i$ | $-i$ | $-i$ | $-i$ | $-i$ | 1   | 1   | 1   | -1  | -1  | -1  |     |
| Landau | A1  | A1  | A1  | A1  | A1  | A1  | B1  | B1  | B1  | B1  | B1  | B1  | E   | E   | E   | E   | E   | E   | E   | E   | E   | E   | E    | E    | E    | E    | E    | E    | E    | E   | A2  | A2  | A2  | B2  | B2  | B2  |

$$\mathbf{S} = \mathbf{1}, \mathbf{n}_{\text{occ.}} = \{\mathbf{2}, \mathbf{0}, \mathbf{1}, \mathbf{0}, \mathbf{1}\}$$

| State  | 259 | 260 | 261 | 262 | 263 | 264 | 265 | 266 | 267 | 268 | 269 | 270 | 271 | 272 | 273 | 274 | 275 | 276 | 277 | 278 | 279 | 280 | 281  | 282  | 283  | 284  | 285  | 286  | 287  | 288  | 289 | 290 | 291 | 292 | 293 | 294 |
|--------|-----|-----|-----|-----|-----|-----|-----|-----|-----|-----|-----|-----|-----|-----|-----|-----|-----|-----|-----|-----|-----|-----|------|------|------|------|------|------|------|------|-----|-----|-----|-----|-----|-----|
| Sz     | 1   | 0   | -1  | 1   | 0   | -1  | 1   | 0   | -1  | 1   | 0   | -1  | 1   | 0   | -1  | 1   | 0   | -1  | 1   | 0   | -1  | 1   | 0    | -1   | 1    | 0    | -1   | 1    | 0    | -1   | 1   | 0   | -1  | 1   | 0   | -1  |
| Rx     | 1   | 1   | 1   | 1   | 1   | 1   | 1   | 1   | 1   | 1   | 1   | 1   | 0   | 0   | 0   | 0   | 0   | 0   | 0   | 0   | 0   | 0   | 0    | 0    | 0    | 0    | 0    | 0    | 0    | 0    | -1  | -1  | -1  | -1  | -1  | -1  |
| Ry     | 1   | 1   | 1   | 1   | 1   | 1   | 1   | 1   | 1   | 1   | 1   | 1   | 0   | 0   | 0   | 0   | 0   | 0   | 0   | 0   | 0   | 0   | 0    | 0    | 0    | 0    | 0    | 0    | 0    | 0    | -1  | -1  | -1  | -1  | -1  | -1  |
| R      | 1   | 1   | 1   | 1   | 1   | 1   | -1  | -1  | -1  | -1  | -1  | -1  | $i$ | $i$ | $i$ | $i$ | $i$ | $i$ | $i$ | $i$ | $i$ | $i$ | $-i$ | $-i$ | $-i$ | $-i$ | $-i$ | $-i$ | $-i$ | $-i$ | 1   | 1   | 1   | -1  | -1  | -1  |
| Landau | A1  | A1  | A1  | A1  | A1  | A1  | B1  | B1  | B1  | B1  | B1  | B1  | E   | E   | E   | E   | E   | E   | E   | E   | E   | E   | E    | E    | E    | E    | E    | E    | E    | E    | A2  | A2  | A2  | B2  | B2  | B2  |

$$S = 1, \mathbf{n}_{\text{occ.}} = \{2, 0, 0, 2, 0\}$$

[illegible]

$$\mathbf{S} = \mathbf{1}, \mathbf{n}_{\text{occ.}} = \{\mathbf{2}, \mathbf{0}, \mathbf{0}, \mathbf{1}, \mathbf{1}\}$$

| State  | 313 | 314 | 315 | 316 | 317 | 318 | 319 | 320 | 321 | 322 | 323 | 324 | 325      | 326      | 327      | 328      | 329      | 330      | 331      | 332      | 333      | 334      | 335        | 336        | 337        | 338        | 339        | 340        | 341        | 342        | 343 | 344 | 345 | 346 | 347 | 348 |
|--------|-----|-----|-----|-----|-----|-----|-----|-----|-----|-----|-----|-----|----------|----------|----------|----------|----------|----------|----------|----------|----------|----------|------------|------------|------------|------------|------------|------------|------------|------------|-----|-----|-----|-----|-----|-----|
| Sz     | 1   | 0   | -1  | 1   | 0   | -1  | 1   | 0   | -1  | 1   | 0   | -1  | 1        | 0        | -1       | 1        | 0        | -1       | 1        | 0        | -1       | 1        | 0          | -1         | 1          | 0          | -1         | 1          | 0          | -1         | 1   | 0   | -1  | 1   | 0   | -1  |
| Rx     | 1   | 1   | 1   | 1   | 1   | 1   | 1   | 1   | 1   | 1   | 1   | 1   | 0        | 0        | 0        | 0        | 0        | 0        | 0        | 0        | 0        | 0        | 0          | 0          | 0          | 0          | 0          | 0          | 0          | 0          | -1  | -1  | -1  | -1  | -1  | -1  |
| Ry     | 1   | 1   | 1   | 1   | 1   | 1   | 1   | 1   | 1   | 1   | 1   | 1   | 0        | 0        | 0        | 0        | 0        | 0        | 0        | 0        | 0        | 0        | 0          | 0          | 0          | 0          | 0          | 0          | 0          | 0          | -1  | -1  | -1  | -1  | -1  | -1  |
| R      | 1   | 1   | 1   | 1   | 1   | 1   | -1  | -1  | -1  | -1  | -1  | -1  | <i>i</i> | <i>i</i> | <i>i</i> | <i>i</i> | <i>i</i> | <i>i</i> | <i>i</i> | <i>i</i> | <i>i</i> | <i>i</i> | - <i>i</i> | - <i>i</i> | - <i>i</i> | - <i>i</i> | - <i>i</i> | - <i>i</i> | - <i>i</i> | - <i>i</i> | 1   | 1   | 1   | -1  | -1  | -1  |
| Landau | A1  | A1  | A1  | A1  | A1  | A1  | B1  | B1  | B1  | B1  | B1  | B1  | E        | E        | E        | E        | E        | E        | E        | E        | E        | E        | E          | E          | E          | E          | E          | E          | E          | E          | A2  | A2  | A2  | B2  | B2  | B2  |

$$S = 1, \text{ n}_{\text{occ.}} = \{2, 0, 0, 0, 2\}$$

[illegible]







$$\mathbf{S} = \mathbf{1}/2, \mathbf{n}_{\text{occ.}} = \{\mathbf{3}, \mathbf{0}, \mathbf{0}, \mathbf{1}, \mathbf{0}\}$$

| State  | 399           | 400            | 401           | 402            | 403           | 404            | 405           | 406            | 407           | 408            | 409           | 410            | 411           | 412            | 413           | 414            |    |
|--------|---------------|----------------|---------------|----------------|---------------|----------------|---------------|----------------|---------------|----------------|---------------|----------------|---------------|----------------|---------------|----------------|----|
| Sz     | $\frac{1}{2}$ | $-\frac{1}{2}$ | $\frac{1}{2}$ | $-\frac{1}{2}$ | $\frac{1}{2}$ | $-\frac{1}{2}$ | $\frac{1}{2}$ | $-\frac{1}{2}$ | $\frac{1}{2}$ | $-\frac{1}{2}$ | $\frac{1}{2}$ | $-\frac{1}{2}$ | $\frac{1}{2}$ | $-\frac{1}{2}$ | $\frac{1}{2}$ | $-\frac{1}{2}$ |    |
| Rx     | 1             | 1              | 1             | 1              | 0             | 0              | 0             | 0              | 0             | 0              | 0             | 0              | -1            | -1             | -1            | -1             |    |
| Ry     | 1             | 1              | 1             | 1              | 0             | 0              | 0             | 0              | 0             | 0              | 0             | 0              | -1            | -1             | -1            | -1             |    |
| R      | 1             | 1              | -1            | -1             | $i$           | $i$            | $i$           | $i$            | $-i$          | $-i$           | $-i$          | $-i$           | 1             | 1              | -1            | -1             |    |
| Landau | A1            | A1             | B1            | B1             | E             | E              | E             | E              | E             | E              | E             | E              | E             | A2             | A2            | B2             | B2 |

$$\mathbf{S} = 1/2, \text{ n}_{\text{occ.}} = \{3, 0, 0, 0, 1\}$$

| State  | 415           | 416            | 417           | 418            | 419           | 420            | 421           | 422            | 423           | 424            | 425           | 426            | 427           | 428            | 429           | 430            |
|--------|---------------|----------------|---------------|----------------|---------------|----------------|---------------|----------------|---------------|----------------|---------------|----------------|---------------|----------------|---------------|----------------|
| Sz     | $\frac{1}{2}$ | $-\frac{1}{2}$ | $\frac{1}{2}$ | $-\frac{1}{2}$ | $\frac{1}{2}$ | $-\frac{1}{2}$ | $\frac{1}{2}$ | $-\frac{1}{2}$ | $\frac{1}{2}$ | $-\frac{1}{2}$ | $\frac{1}{2}$ | $-\frac{1}{2}$ | $\frac{1}{2}$ | $-\frac{1}{2}$ | $\frac{1}{2}$ | $-\frac{1}{2}$ |
| Rx     | 1             | 1              | 1             | 1              | 0             | 0              | 0             | 0              | 0             | 0              | 0             | 0              | -1            | -1             | -1            | -1             |
| Ry     | 1             | 1              | 1             | 1              | 0             | 0              | 0             | 0              | 0             | 0              | 0             | 0              | -1            | -1             | -1            | -1             |
| R      | 1             | 1              | -1            | -1             | $i$           | $i$            | $i$           | $i$            | $-i$          | $-i$           | $-i$          | $-i$           | 1             | 1              | -1            | -1             |
| Landau | A1            | A1             | B1            | B1             | E             | E              | E             | E              | E             | E              | E             | E              | A2            | A2             | B2            | B2             |

$$\mathbf{S} = \mathbf{1}/2, \mathbf{n}_{\text{occ.}} = \{\mathbf{1}, \mathbf{3}, \mathbf{0}, \mathbf{0}, \mathbf{0}\}$$

$$\left( \begin{array}{c|cccccccc} \text{State} & 431 & 432 & 433 & 434 & 435 & 436 & 437 & 438 \\ \hline \text{Sz} & \frac{1}{2} & -\frac{1}{2} & \frac{1}{2} & -\frac{1}{2} & \frac{1}{2} & -\frac{1}{2} & \frac{1}{2} & -\frac{1}{2} \\ \text{Rx} & 1 & 1 & 1 & 1 & 0 & 0 & 0 & 0 \\ \text{Ry} & 1 & 1 & 1 & 1 & 0 & 0 & 0 & 0 \\ \text{R} & 1 & 1 & -1 & -1 & i & i & -i & -i \\ \text{Landau} & \text{A1} & \text{A1} & \text{B1} & \text{B1} & \text{E} & \text{E} & \text{E} & \text{E} \end{array} \right)$$

$$\mathbf{S} = \mathbf{1}/2, \mathbf{n}_{\text{occ.}} = \{\mathbf{1}, \mathbf{2}, \mathbf{1}, \mathbf{0}, \mathbf{0}\}$$

| State  | 439           | 440            | 441           | 442            | 443           | 444            | 445           | 446            | 447           | 448            | 449           | 450            | 451           | 452            | 453           | 454            | 455           | 456            | 457           | 458            | 459           | 460            | 461           | 462            |
|--------|---------------|----------------|---------------|----------------|---------------|----------------|---------------|----------------|---------------|----------------|---------------|----------------|---------------|----------------|---------------|----------------|---------------|----------------|---------------|----------------|---------------|----------------|---------------|----------------|
| Sz     | $\frac{1}{2}$ | $-\frac{1}{2}$ | $\frac{1}{2}$ | $-\frac{1}{2}$ | $\frac{1}{2}$ | $-\frac{1}{2}$ | $\frac{1}{2}$ | $-\frac{1}{2}$ | $\frac{1}{2}$ | $-\frac{1}{2}$ | $\frac{1}{2}$ | $-\frac{1}{2}$ | $\frac{1}{2}$ | $-\frac{1}{2}$ | $\frac{1}{2}$ | $-\frac{1}{2}$ | $\frac{1}{2}$ | $-\frac{1}{2}$ | $\frac{1}{2}$ | $-\frac{1}{2}$ | $\frac{1}{2}$ | $-\frac{1}{2}$ | $\frac{1}{2}$ | $-\frac{1}{2}$ |
| Rx     | 1             | 1              | 1             | 1              | 1             | 1              | 1             | 1              | 0             | 0              | 0             | 0              | 0             | 0              | 0             | 0              | 0             | 0              | 0             | 0              | -1            | -1             | -1            | -1             |
| Ry     | 1             | 1              | 1             | 1              | 1             | 1              | 1             | 1              | 0             | 0              | 0             | 0              | 0             | 0              | 0             | 0              | 0             | 0              | 0             | 0              | -1            | -1             | -1            | -1             |
| R      | 1             | 1              | 1             | 1              | -1            | -1             | -1            | -1             | $i$           | $i$            | $i$           | $i$            | $i$           | $i$            | $-i$          | $-i$           | $-i$          | $-i$           | $-i$          | $-i$           | 1             | 1              | -1            | -1             |
| Landau | A1            | A1             | A1            | A1             | B1            | B1             | B1            | B1             | E             | E              | E             | E              | E             | E              | E             | E              | E             | E              | E             | E              | A2            | A2             | B2            | B2             |

$$\mathbf{S} = \mathbf{1}/2, \mathbf{n}_{\text{occ.}} = \{\mathbf{1}, \mathbf{2}, \mathbf{0}, \mathbf{1}, \mathbf{0}\}$$

| State  | 463           | 464            | 465           | 466            | 467           | 468            | 469           | 470            | 471           | 472            | 473           | 474            | 475           | 476            | 477           | 478            | 479           | 480            | 481           | 482            | 483           | 484            | 485           | 486            |
|--------|---------------|----------------|---------------|----------------|---------------|----------------|---------------|----------------|---------------|----------------|---------------|----------------|---------------|----------------|---------------|----------------|---------------|----------------|---------------|----------------|---------------|----------------|---------------|----------------|
| Sz     | $\frac{1}{2}$ | $-\frac{1}{2}$ | $\frac{1}{2}$ | $-\frac{1}{2}$ | $\frac{1}{2}$ | $-\frac{1}{2}$ | $\frac{1}{2}$ | $-\frac{1}{2}$ | $\frac{1}{2}$ | $-\frac{1}{2}$ | $\frac{1}{2}$ | $-\frac{1}{2}$ | $\frac{1}{2}$ | $-\frac{1}{2}$ | $\frac{1}{2}$ | $-\frac{1}{2}$ | $\frac{1}{2}$ | $-\frac{1}{2}$ | $\frac{1}{2}$ | $-\frac{1}{2}$ | $\frac{1}{2}$ | $-\frac{1}{2}$ | $\frac{1}{2}$ | $-\frac{1}{2}$ |
| Rx     | 1             | 1              | 1             | 1              | 1             | 1              | 1             | 1              | 0             | 0              | 0             | 0              | 0             | 0              | 0             | 0              | 0             | 0              | 0             | 0              | -1            | -1             | -1            | -1             |
| Ry     | 1             | 1              | 1             | 1              | 1             | 1              | 1             | 1              | 0             | 0              | 0             | 0              | 0             | 0              | 0             | 0              | 0             | 0              | 0             | 0              | -1            | -1             | -1            | -1             |
| R      | 1             | 1              | 1             | 1              | -1            | -1             | -1            | -1             | $i$           | $i$            | $i$           | $i$            | $i$           | $i$            | $-i$          | $-i$           | $-i$          | $-i$           | $-i$          | $-i$           | 1             | 1              | -1            | -1             |
| Landau | A1            | A1             | A1            | A1             | B1            | B1             | B1            | B1             | E             | E              | E             | E              | E             | E              | E             | E              | E             | E              | E             | E              | A2            | A2             | B2            | B2             |

$$\mathbf{S} = \mathbf{1}/2, \mathbf{n}_{\text{occ.}} = \{1, 2, 0, 0, 1\}$$

| State  | 487           | 488            | 489           | 490            | 491           | 492            | 493           | 494            | 495           | 496            | 497           | 498            | 499           | 500            | 501           | 502            | 503           | 504            | 505           | 506            | 507           | 508            | 509           | 510            |
|--------|---------------|----------------|---------------|----------------|---------------|----------------|---------------|----------------|---------------|----------------|---------------|----------------|---------------|----------------|---------------|----------------|---------------|----------------|---------------|----------------|---------------|----------------|---------------|----------------|
| Sz     | $\frac{1}{2}$ | $-\frac{1}{2}$ | $\frac{1}{2}$ | $-\frac{1}{2}$ | $\frac{1}{2}$ | $-\frac{1}{2}$ | $\frac{1}{2}$ | $-\frac{1}{2}$ | $\frac{1}{2}$ | $-\frac{1}{2}$ | $\frac{1}{2}$ | $-\frac{1}{2}$ | $\frac{1}{2}$ | $-\frac{1}{2}$ | $\frac{1}{2}$ | $-\frac{1}{2}$ | $\frac{1}{2}$ | $-\frac{1}{2}$ | $\frac{1}{2}$ | $-\frac{1}{2}$ | $\frac{1}{2}$ | $-\frac{1}{2}$ | $\frac{1}{2}$ | $-\frac{1}{2}$ |
| Rx     | 1             | 1              | 1             | 1              | 1             | 1              | 1             | 1              | 0             | 0              | 0             | 0              | 0             | 0              | 0             | 0              | 0             | 0              | 0             | 0              | -1            | -1             | -1            | -1             |
| Ry     | 1             | 1              | 1             | 1              | 1             | 1              | 1             | 1              | 0             | 0              | 0             | 0              | 0             | 0              | 0             | 0              | 0             | 0              | 0             | 0              | -1            | -1             | -1            | -1             |
| R      | 1             | 1              | 1             | 1              | -1            | -1             | -1            | -1             | $i$           | $i$            | $i$           | $i$            | $i$           | $i$            | $-i$          | $-i$           | $-i$          | $-i$           | $-i$          | $-i$           | 1             | 1              | -1            | -1             |
| Landau | A1            | A1             | A1            | A1             | B1            | B1             | B1            | B1             | E             | E              | E             | E              | E             | E              | E             | E              | E             | E              | E             | E              | A2            | A2             | B2            | B2             |

$$\mathbf{S} = \mathbf{1}/2, \mathbf{n}_{\text{occ.}} = \{\mathbf{1}, \mathbf{1}, \mathbf{2}, \mathbf{0}, \mathbf{0}\}$$

| State  | 511           | 512            | 513           | 514            | 515           | 516            | 517           | 518            | 519           | 520            | 521           | 522            | 523           | 524            | 525           | 526            | 527           | 528            | 529           | 530            | 531           | 532            | 533           | 534            |
|--------|---------------|----------------|---------------|----------------|---------------|----------------|---------------|----------------|---------------|----------------|---------------|----------------|---------------|----------------|---------------|----------------|---------------|----------------|---------------|----------------|---------------|----------------|---------------|----------------|
| Sz     | $\frac{1}{2}$ | $-\frac{1}{2}$ | $\frac{1}{2}$ | $-\frac{1}{2}$ | $\frac{1}{2}$ | $-\frac{1}{2}$ | $\frac{1}{2}$ | $-\frac{1}{2}$ | $\frac{1}{2}$ | $-\frac{1}{2}$ | $\frac{1}{2}$ | $-\frac{1}{2}$ | $\frac{1}{2}$ | $-\frac{1}{2}$ | $\frac{1}{2}$ | $-\frac{1}{2}$ | $\frac{1}{2}$ | $-\frac{1}{2}$ | $\frac{1}{2}$ | $-\frac{1}{2}$ | $\frac{1}{2}$ | $-\frac{1}{2}$ | $\frac{1}{2}$ | $-\frac{1}{2}$ |
| Rx     | 1             | 1              | 1             | 1              | 1             | 1              | 1             | 1              | 0             | 0              | 0             | 0              | 0             | 0              | 0             | 0              | 0             | 0              | 0             | 0              | -1            | -1             | -1            | -1             |
| Ry     | 1             | 1              | 1             | 1              | 1             | 1              | 1             | 1              | 0             | 0              | 0             | 0              | 0             | 0              | 0             | 0              | 0             | 0              | 0             | 0              | -1            | -1             | -1            | -1             |
| R      | 1             | 1              | 1             | 1              | -1            | -1             | -1            | -1             | $i$           | $i$            | $i$           | $i$            | $i$           | $i$            | $-i$          | $-i$           | $-i$          | $-i$           | $-i$          | $-i$           | 1             | 1              | -1            | -1             |
| Landau | A1            | A1             | A1            | A1             | B1            | B1             | B1            | B1             | E             | E              | E             | E              | E             | E              | E             | E              | E             | E              | E             | E              | A2            | A2             | B2            | B2             |



$\mathbf{S} = \mathbf{1}/\mathbf{2}, \mathbf{n}_{\text{occ.}} = \{\mathbf{1}, \mathbf{1}, \mathbf{1}, \mathbf{1}, \mathbf{0}\}$   

|        | 535           | 536            | 537           | 538            | 539           | 540            | 541           | 542            | 543           | 544            | 545           | 546            | 547           | 548            | 549           | 550            | 551           | 552            | 553           | 554            | 555           | 556            | 557           | 558            | 559           | 560            | 561           | 562            | 563           | 564            | 565           | 566            | 567           | 568            | 569           | 570            | 571           | 572            | 573           | 574            | 575           | 576            | 577           | 578            | 579           | 580            | 581 | 582 |
|--------|---------------|----------------|---------------|----------------|---------------|----------------|---------------|----------------|---------------|----------------|---------------|----------------|---------------|----------------|---------------|----------------|---------------|----------------|---------------|----------------|---------------|----------------|---------------|----------------|---------------|----------------|---------------|----------------|---------------|----------------|---------------|----------------|---------------|----------------|---------------|----------------|---------------|----------------|---------------|----------------|---------------|----------------|---------------|----------------|---------------|----------------|-----|-----|
| State  | 535           | 536            | 537           | 538            | 539           | 540            | 541           | 542            | 543           | 544            | 545           | 546            | 547           | 548            | 549           | 550            | 551           | 552            | 553           | 554            | 555           | 556            | 557           | 558            | 559           | 560            | 561           | 562            | 563           | 564            | 565           | 566            | 567           | 568            | 569           | 570            | 571           | 572            | 573           | 574            | 575           | 576            | 577           | 578            | 579           | 580            | 581 | 582 |
| Sz     | $\frac{1}{2}$ | $-\frac{1}{2}$ | $\frac{1}{2}$ | $-\frac{1}{2}$ | $\frac{1}{2}$ | $-\frac{1}{2}$ | $\frac{1}{2}$ | $-\frac{1}{2}$ | $\frac{1}{2}$ | $-\frac{1}{2}$ | $\frac{1}{2}$ | $-\frac{1}{2}$ | $\frac{1}{2}$ | $-\frac{1}{2}$ | $\frac{1}{2}$ | $-\frac{1}{2}$ | $\frac{1}{2}$ | $-\frac{1}{2}$ | $\frac{1}{2}$ | $-\frac{1}{2}$ | $\frac{1}{2}$ | $-\frac{1}{2}$ | $\frac{1}{2}$ | $-\frac{1}{2}$ | $\frac{1}{2}$ | $-\frac{1}{2}$ | $\frac{1}{2}$ | $-\frac{1}{2}$ | $\frac{1}{2}$ | $-\frac{1}{2}$ | $\frac{1}{2}$ | $-\frac{1}{2}$ | $\frac{1}{2}$ | $-\frac{1}{2}$ | $\frac{1}{2}$ | $-\frac{1}{2}$ | $\frac{1}{2}$ | $-\frac{1}{2}$ | $\frac{1}{2}$ | $-\frac{1}{2}$ | $\frac{1}{2}$ | $-\frac{1}{2}$ | $\frac{1}{2}$ | $-\frac{1}{2}$ | $\frac{1}{2}$ | $-\frac{1}{2}$ |     |     |
| Rx     | 1             | 1              | 1             | 1              | 1             | 1              | 1             | 1              | 1             | 1              | 1             | 1              | 0             | 0              | 0             | 0              | 0             | 0              | 0             | 0              | 0             | 0              | 0             | 0              | 0             | 0              | 0             | 0              | 0             | 0              | 0             | 0              | 0             | 0              | -1            | -1             | -1            | -1             | -1            | -1             | -1            | -1             | -1            | -1             | -1            | -1             |     |     |
| Ry     | 1             | 1              | 1             | 1              | 1             | 1              | 1             | 1              | 1             | 1              | 1             | 1              | 0             | 0              | 0             | 0              | 0             | 0              | 0             | 0              | 0             | 0              | 0             | 0              | 0             | 0              | 0             | 0              | 0             | 0              | 0             | 0              | 0             | 0              | 0             | -1             | -1            | -1             | -1            | -1             | -1            | -1             | -1            | -1             | -1            | -1             | -1  |     |
| R      | 1             | 1              | 1             | 1              | 1             | 1              | -1            | -1             | -1            | -1             | -1            | -1             | i             | i              | i             | i              | i             | i              | i             | i              | i             | i              | i             | i              | -i            | -i             | -i            | -i             | -i            | -i             | -i            | -i             | -i            | -i             | -i            | 1              | 1             | 1              | 1             | 1              | 1             | -1             | -1            | -1             | -1            | -1             | -1  |     |
| Landau | A1            | A1             | A1            | A1             | A1            | A1             | B1            | B1             | B1            | B1             | B1            | B1             | E             | E              | E             | E              | E             | E              | E             | E              | E             | E              | E             | E              | E             | E              | E             | E              | E             | E              | E             | E              | E             | E              | E             | E              | A2            | A2             | A2            | A2             | A2            | A2             | B2            | B2             | B2            | B2             | B2  | B2  |

$\mathbf{S} = \mathbf{1}/\mathbf{2}, \mathbf{n}_{\text{occ.}} = \{\mathbf{1}, \mathbf{1}, \mathbf{1}, \mathbf{0}, \mathbf{1}\}$

|        | State | 583           | 584            | 585           | 586            | 587           | 588            | 589           | 590            | 591           | 592            | 593           | 594            | 595           | 596            | 597           | 598            | 599           | 600            | 601           | 602            | 603           | 604            | 605           | 606            | 607           | 608            | 609           | 610            | 611           | 612            | 613           | 614            | 615           | 616            | 617           | 618            | 619           | 620            | 621           | 622            | 623           | 624            | 625           | 626            | 627 | 628 | 629 | 630 |    |    |
|--------|-------|---------------|----------------|---------------|----------------|---------------|----------------|---------------|----------------|---------------|----------------|---------------|----------------|---------------|----------------|---------------|----------------|---------------|----------------|---------------|----------------|---------------|----------------|---------------|----------------|---------------|----------------|---------------|----------------|---------------|----------------|---------------|----------------|---------------|----------------|---------------|----------------|---------------|----------------|---------------|----------------|---------------|----------------|---------------|----------------|-----|-----|-----|-----|----|----|
| Sz     |       | $\frac{1}{2}$ | $-\frac{1}{2}$ | $\frac{1}{2}$ | $-\frac{1}{2}$ | $\frac{1}{2}$ | $-\frac{1}{2}$ | $\frac{1}{2}$ | $-\frac{1}{2}$ | $\frac{1}{2}$ | $-\frac{1}{2}$ | $\frac{1}{2}$ | $-\frac{1}{2}$ | $\frac{1}{2}$ | $-\frac{1}{2}$ | $\frac{1}{2}$ | $-\frac{1}{2}$ | $\frac{1}{2}$ | $-\frac{1}{2}$ | $\frac{1}{2}$ | $-\frac{1}{2}$ | $\frac{1}{2}$ | $-\frac{1}{2}$ | $\frac{1}{2}$ | $-\frac{1}{2}$ | $\frac{1}{2}$ | $-\frac{1}{2}$ | $\frac{1}{2}$ | $-\frac{1}{2}$ | $\frac{1}{2}$ | $-\frac{1}{2}$ | $\frac{1}{2}$ | $-\frac{1}{2}$ | $\frac{1}{2}$ | $-\frac{1}{2}$ | $\frac{1}{2}$ | $-\frac{1}{2}$ | $\frac{1}{2}$ | $-\frac{1}{2}$ | $\frac{1}{2}$ | $-\frac{1}{2}$ | $\frac{1}{2}$ | $-\frac{1}{2}$ | $\frac{1}{2}$ | $-\frac{1}{2}$ |     |     |     |     |    |    |
| Rx     |       | 1             | 1              | 1             | 1              | 1             | 1              | 1             | 1              | 1             | 1              | 1             | 1              | 0             | 0              | 0             | 0              | 0             | 0              | 0             | 0              | 0             | 0              | 0             | 0              | 0             | 0              | 0             | 0              | 0             | 0              | 0             | 0              | 0             | 0              | 0             | -1             | -1            | -1             | -1            | -1             | -1            | -1             | -1            | -1             | -1  | -1  |     |     |    |    |
| Ry     |       | 1             | 1              | 1             | 1              | 1             | 1              | 1             | 1              | 1             | 1              | 1             | 1              | 0             | 0              | 0             | 0              | 0             | 0              | 0             | 0              | 0             | 0              | 0             | 0              | 0             | 0              | 0             | 0              | 0             | 0              | 0             | 0              | 0             | 0              | 0             | 0              | 0             | 0              | -1            | -1             | -1            | -1             | -1            | -1             | -1  | -1  | -1  | -1  |    |    |
| R      |       | 1             | 1              | 1             | 1              | 1             | 1              | -1            | -1             | -1            | -1             | -1            | -1             | i             | i              | i             | i              | i             | i              | i             | i              | i             | i              | i             | i              | -i            | -i             | -i            | -i             | -i            | -i             | -i            | -i             | -i            | -i             | -i            | -i             | 1             | 1              | 1             | 1              | 1             | 1              | -1            | -1             | -1  | -1  | -1  | -1  |    |    |
| Landau |       | A1            | A1             | A1            | A1             | A1            | A1             | B1            | B1             | B1            | B1             | B1            | B1             | E             | E              | E             | E              | E             | E              | E             | E              | E             | E              | E             | E              | E             | E              | E             | E              | E             | E              | E             | E              | E             | E              | E             | E              | E             | E              | A2            | A2             | A2            | A2             | A2            | A2             | B2  | B2  | B2  | B2  | B2 | B2 |

$$\mathbf{S} = \mathbf{1}/2, \mathbf{n}_{\text{occ.}} = \{\mathbf{1}, \mathbf{1}, \mathbf{0}, \mathbf{2}, \mathbf{0}\}$$

| State  | 631           | 632            | 633           | 634            | 635           | 636            | 637           | 638            | 639           | 640            | 641           | 642            | 643           | 644            | 645           | 646            | 647           | 648            | 649           | 650            | 651           | 652            | 653           | 654            |
|--------|---------------|----------------|---------------|----------------|---------------|----------------|---------------|----------------|---------------|----------------|---------------|----------------|---------------|----------------|---------------|----------------|---------------|----------------|---------------|----------------|---------------|----------------|---------------|----------------|
| Sz     | $\frac{1}{2}$ | $-\frac{1}{2}$ | $\frac{1}{2}$ | $-\frac{1}{2}$ | $\frac{1}{2}$ | $-\frac{1}{2}$ | $\frac{1}{2}$ | $-\frac{1}{2}$ | $\frac{1}{2}$ | $-\frac{1}{2}$ | $\frac{1}{2}$ | $-\frac{1}{2}$ | $\frac{1}{2}$ | $-\frac{1}{2}$ | $\frac{1}{2}$ | $-\frac{1}{2}$ | $\frac{1}{2}$ | $-\frac{1}{2}$ | $\frac{1}{2}$ | $-\frac{1}{2}$ | $\frac{1}{2}$ | $-\frac{1}{2}$ | $\frac{1}{2}$ | $-\frac{1}{2}$ |
| Rx     | 1             | 1              | 1             | 1              | 1             | 1              | 1             | 1              | 0             | 0              | 0             | 0              | 0             | 0              | 0             | 0              | 0             | 0              | 0             | 0              | -1            | -1             | -1            | -1             |
| Ry     | 1             | 1              | 1             | 1              | 1             | 1              | 1             | 1              | 0             | 0              | 0             | 0              | 0             | 0              | 0             | 0              | 0             | 0              | 0             | 0              | -1            | -1             | -1            | -1             |
| R      | 1             | 1              | 1             | 1              | -1            | -1             | -1            | -1             | $i$           | $i$            | $i$           | $i$            | $i$           | $i$            | $-i$          | $-i$           | $-i$          | $-i$           | $-i$          | $-i$           | 1             | 1              | -1            | -1             |
| Landau | A1            | A1             | A1            | A1             | B1            | B1             | B1            | B1             | E             | E              | E             | E              | E             | E              | E             | E              | E             | E              | E             | E              | A2            | A2             | B2            | B2             |

$$\begin{aligned}
&\mathbf{S} = \mathbf{1}/2, \mathbf{n}_{\text{occ.}} = \{1, 1, 0, 1, 1\} \\
&\left( \begin{array}{cc} \text{State} & \begin{matrix} 655 & 656 & 657 & 658 & 659 & 660 & 661 & 662 & 663 & 664 & 665 & 666 & 667 & 668 & 669 & 670 & 671 & 672 & 673 & 674 & 675 & 676 & 677 & 678 & 679 & 680 & 681 & 682 & 683 & 684 & 685 & 686 & 687 & 688 & 689 & 690 & 691 & 692 & 693 & 694 & 695 & 696 & 697 & 698 & 699 & 700 & 701 & 702 \end{matrix} \\ \text{Sz} & \begin{matrix} \frac{1}{2} & -\frac{1}{2} & \frac{1}{2} & -\frac{1}{2} & \frac{1}{2} & -\frac{1}{2} & \frac{1}{2} & -\frac{1}{2} & \frac{1}{2} & -\frac{1}{2} & \frac{1}{2} & -\frac{1}{2} & \frac{1}{2} & -\frac{1}{2} & \frac{1}{2} & -\frac{1}{2} & \frac{1}{2} & -\frac{1}{2} & \frac{1}{2} & -\frac{1}{2} & \frac{1}{2} & -\frac{1}{2} & \frac{1}{2} & -\frac{1}{2} & \frac{1}{2} & -\frac{1}{2} & \frac{1}{2} & -\frac{1}{2} & \frac{1}{2} & -\frac{1}{2} & \frac{1}{2} & -\frac{1}{2} & \frac{1}{2} & -\frac{1}{2} & \frac{1}{2} & -\frac{1}{2} & \frac{1}{2} & -\frac{1}{2} & \frac{1}{2} & -\frac{1}{2} & \frac{1}{2} & -\frac{1}{2} & \frac{1}{2} & -\frac{1}{2} \end{matrix} \\ \text{Rx} & \begin{matrix} 1 & 1 & 1 & 1 & 1 & 1 & 1 & 1 & 1 & 1 & 1 & 1 & 0 & 0 & 0 & 0 & 0 & 0 & 0 & 0 & 0 & 0 & 0 & 0 & 0 & 0 & 0 & 0 & 0 & 0 & 0 & 0 & 0 & 0 & -1 & -1 & -1 & -1 & -1 & -1 & -1 & -1 & -1 & -1 & -1 \end{matrix} \\ \text{Ry} & \begin{matrix} 1 & 1 & 1 & 1 & 1 & 1 & 1 & 1 & 1 & 1 & 1 & 1 & 0 & 0 & 0 & 0 & 0 & 0 & 0 & 0 & 0 & 0 & 0 & 0 & 0 & 0 & 0 & 0 & 0 & 0 & 0 & 0 & 0 & 0 & -1 & -1 & -1 & -1 & -1 & -1 & -1 & -1 & -1 & -1 \end{matrix} \\ \text{R} & \begin{matrix} 1 & 1 & 1 & 1 & 1 & 1 & -1 & -1 & -1 & -1 & -1 & -1 & i & i & i & i & i & i & i & i & i & i & i & -i & -i & -i & -i & -i & -i & -i & -i & -i & -i & 1 & 1 & 1 & 1 & 1 & 1 & -1 & -1 & -1 & -1 & -1 \end{matrix} \\ \text{Landau} & \begin{matrix} \text{A1} & \text{A1} & \text{A1} & \text{A1} & \text{A1} & \text{A1} & \text{B1} & \text{B1} & \text{B1} & \text{B1} & \text{B1} & \text{B1} & \text{E} & \text{E} & \text{E} & \text{E} & \text{E} & \text{E} & \text{E} & \text{E} & \text{E} & \text{E} & \text{E} & \text{E} & \text{E} & \text{E} & \text{E} & \text{E} & \text{E} & \text{E} & \text{E} & \text{E} & \text{E} & \text{A2} & \text{A2} & \text{A2} & \text{A2} & \text{A2} & \text{A2} & \text{B2} & \text{B2} & \text{B2} & \text{B2} & \text{B2} & \text{B2} \end{matrix} \end{array} \right)
\end{aligned}$$

$$\mathbf{S} = \mathbf{1}/2, \mathbf{n}_{\text{occ.}} = \{\mathbf{1}, \mathbf{1}, \mathbf{0}, \mathbf{0}, \mathbf{2}\}$$

| State  | 703           | 704            | 705           | 706            | 707           | 708            | 709           | 710            | 711           | 712            | 713           | 714            | 715           | 716            | 717           | 718            | 719           | 720            | 721           | 722            | 723           | 724            | 725           | 726            |
|--------|---------------|----------------|---------------|----------------|---------------|----------------|---------------|----------------|---------------|----------------|---------------|----------------|---------------|----------------|---------------|----------------|---------------|----------------|---------------|----------------|---------------|----------------|---------------|----------------|
| Sz     | $\frac{1}{2}$ | $-\frac{1}{2}$ | $\frac{1}{2}$ | $-\frac{1}{2}$ | $\frac{1}{2}$ | $-\frac{1}{2}$ | $\frac{1}{2}$ | $-\frac{1}{2}$ | $\frac{1}{2}$ | $-\frac{1}{2}$ | $\frac{1}{2}$ | $-\frac{1}{2}$ | $\frac{1}{2}$ | $-\frac{1}{2}$ | $\frac{1}{2}$ | $-\frac{1}{2}$ | $\frac{1}{2}$ | $-\frac{1}{2}$ | $\frac{1}{2}$ | $-\frac{1}{2}$ | $\frac{1}{2}$ | $-\frac{1}{2}$ | $\frac{1}{2}$ | $-\frac{1}{2}$ |
| Rx     | 1             | 1              | 1             | 1              | 1             | 1              | 1             | 1              | 0             | 0              | 0             | 0              | 0             | 0              | 0             | 0              | 0             | 0              | 0             | 0              | -1            | -1             | -1            | -1             |
| Ry     | 1             | 1              | 1             | 1              | 1             | 1              | 1             | 1              | 0             | 0              | 0             | 0              | 0             | 0              | 0             | 0              | 0             | 0              | 0             | 0              | -1            | -1             | -1            | -1             |
| R      | 1             | 1              | 1             | 1              | -1            | -1             | -1            | -1             | $i$           | $i$            | $i$           | $i$            | $i$           | $i$            | $-i$          | $-i$           | $-i$          | $-i$           | $-i$          | $-i$           | 1             | 1              | -1            | -1             |
| Landau | A1            | A1             | A1            | A1             | B1            | B1             | B1            | B1             | E             | E              | E             | E              | E             | E              | E             | E              | E             | E              | E             | E              | A2            | A2             | B2            | B2             |

$$\mathbf{S} = \mathbf{1}/\mathbf{2}, \mathbf{n}_{\text{occ.}} = \{\mathbf{1}, \mathbf{0}, \mathbf{3}, \mathbf{0}, \mathbf{0}\}$$

$$\left( \begin{array}{c|ccccccccc} \text{State} & 727 & 728 & 729 & 730 & 731 & 732 & 733 & 734 \\ \hline \text{Sz} & \frac{1}{2} & -\frac{1}{2} & \frac{1}{2} & -\frac{1}{2} & \frac{1}{2} & -\frac{1}{2} & \frac{1}{2} & -\frac{1}{2} \\ \text{Rx} & 1 & 1 & 1 & 1 & 0 & 0 & 0 & 0 \\ \text{Ry} & 1 & 1 & 1 & 1 & 0 & 0 & 0 & 0 \\ \text{R} & 1 & 1 & -1 & -1 & i & i & -i & -i \\ \text{Landau} & \text{A1} & \text{A1} & \text{B1} & \text{B1} & \text{E} & \text{E} & \text{E} & \text{E} \end{array} \right)$$

$$\mathbf{S} = \mathbf{1}/2, \mathbf{n}_{\text{occ.}} = \{1, 0, 2, 1, 0\}$$

| State  | 735           | 736            | 737           | 738            | 739           | 740            | 741           | 742            | 743           | 744            | 745           | 746            | 747           | 748            | 749           | 750            | 751           | 752            | 753           | 754            | 755           | 756            | 757           | 758            |
|--------|---------------|----------------|---------------|----------------|---------------|----------------|---------------|----------------|---------------|----------------|---------------|----------------|---------------|----------------|---------------|----------------|---------------|----------------|---------------|----------------|---------------|----------------|---------------|----------------|
| Sz     | $\frac{1}{2}$ | $-\frac{1}{2}$ | $\frac{1}{2}$ | $-\frac{1}{2}$ | $\frac{1}{2}$ | $-\frac{1}{2}$ | $\frac{1}{2}$ | $-\frac{1}{2}$ | $\frac{1}{2}$ | $-\frac{1}{2}$ | $\frac{1}{2}$ | $-\frac{1}{2}$ | $\frac{1}{2}$ | $-\frac{1}{2}$ | $\frac{1}{2}$ | $-\frac{1}{2}$ | $\frac{1}{2}$ | $-\frac{1}{2}$ | $\frac{1}{2}$ | $-\frac{1}{2}$ | $\frac{1}{2}$ | $-\frac{1}{2}$ | $\frac{1}{2}$ | $-\frac{1}{2}$ |
| Rx     | 1             | 1              | 1             | 1              | 1             | 1              | 1             | 1              | 0             | 0              | 0             | 0              | 0             | 0              | 0             | 0              | 0             | 0              | 0             | 0              | -1            | -1             | -1            | -1             |
| Ry     | 1             | 1              | 1             | 1              | 1             | 1              | 1             | 1              | 0             | 0              | 0             | 0              | 0             | 0              | 0             | 0              | 0             | 0              | 0             | 0              | -1            | -1             | -1            | -1             |
| R      | 1             | 1              | 1             | 1              | -1            | -1             | -1            | -1             | $i$           | $i$            | $i$           | $i$            | $i$           | $i$            | $-i$          | $-i$           | $-i$          | $-i$           | $-i$          | $-i$           | 1             | 1              | -1            | -1             |
| Landau | A1            | A1             | A1            | A1             | B1            | B1             | B1            | B1             | E             | E              | E             | E              | E             | E              | E             | E              | E             | E              | E             | E              | A2            | A2             | B2            | B2             |

$$\mathbf{S} = \mathbf{1}/2, \mathbf{n}_{\text{occ.}} = \{1, 0, 2, 0, 1\}$$

| State  | 759           | 760            | 761           | 762            | 763           | 764            | 765           | 766            | 767           | 768            | 769           | 770            | 771           | 772            | 773           | 774            | 775           | 776            | 777           | 778            | 779           | 780            | 781           | 782            |
|--------|---------------|----------------|---------------|----------------|---------------|----------------|---------------|----------------|---------------|----------------|---------------|----------------|---------------|----------------|---------------|----------------|---------------|----------------|---------------|----------------|---------------|----------------|---------------|----------------|
| Sz     | $\frac{1}{2}$ | $-\frac{1}{2}$ | $\frac{1}{2}$ | $-\frac{1}{2}$ | $\frac{1}{2}$ | $-\frac{1}{2}$ | $\frac{1}{2}$ | $-\frac{1}{2}$ | $\frac{1}{2}$ | $-\frac{1}{2}$ | $\frac{1}{2}$ | $-\frac{1}{2}$ | $\frac{1}{2}$ | $-\frac{1}{2}$ | $\frac{1}{2}$ | $-\frac{1}{2}$ | $\frac{1}{2}$ | $-\frac{1}{2}$ | $\frac{1}{2}$ | $-\frac{1}{2}$ | $\frac{1}{2}$ | $-\frac{1}{2}$ | $\frac{1}{2}$ | $-\frac{1}{2}$ |
| Rx     | 1             | 1              | 1             | 1              | 1             | 1              | 1             | 1              | 0             | 0              | 0             | 0              | 0             | 0              | 0             | 0              | 0             | 0              | 0             | 0              | -1            | -1             | -1            | -1             |
| Ry     | 1             | 1              | 1             | 1              | 1             | 1              | 1             | 1              | 0             | 0              | 0             | 0              | 0             | 0              | 0             | 0              | 0             | 0              | 0             | 0              | -1            | -1             | -1            | -1             |
| R      | 1             | 1              | 1             | 1              | -1            | -1             | -1            | -1             | $i$           | $i$            | $i$           | $i$            | $i$           | $i$            | $-i$          | $-i$           | $-i$          | $-i$           | $-i$          | $-i$           | 1             | 1              | -1            | -1             |
| Landau | A1            | A1             | A1            | A1             | B1            | B1             | B1            | B1             | E             | E              | E             | E              | E             | E              | E             | E              | E             | E              | E             | E              | A2            | A2             | B2            | B2             |



$$\mathbf{S} = \mathbf{1}/2, \mathbf{n}_{\text{occ.}} = \{\mathbf{1}, \mathbf{0}, \mathbf{1}, \mathbf{2}, \mathbf{0}\}$$

| State  | 783           | 784            | 785           | 786            | 787           | 788            | 789           | 790            | 791           | 792            | 793           | 794            | 795           | 796            | 797           | 798            | 799           | 800            | 801           | 802            | 803           | 804            | 805           | 806            |
|--------|---------------|----------------|---------------|----------------|---------------|----------------|---------------|----------------|---------------|----------------|---------------|----------------|---------------|----------------|---------------|----------------|---------------|----------------|---------------|----------------|---------------|----------------|---------------|----------------|
| Sz     | $\frac{1}{2}$ | $-\frac{1}{2}$ | $\frac{1}{2}$ | $-\frac{1}{2}$ | $\frac{1}{2}$ | $-\frac{1}{2}$ | $\frac{1}{2}$ | $-\frac{1}{2}$ | $\frac{1}{2}$ | $-\frac{1}{2}$ | $\frac{1}{2}$ | $-\frac{1}{2}$ | $\frac{1}{2}$ | $-\frac{1}{2}$ | $\frac{1}{2}$ | $-\frac{1}{2}$ | $\frac{1}{2}$ | $-\frac{1}{2}$ | $\frac{1}{2}$ | $-\frac{1}{2}$ | $\frac{1}{2}$ | $-\frac{1}{2}$ | $\frac{1}{2}$ | $-\frac{1}{2}$ |
| Rx     | 1             | 1              | 1             | 1              | 1             | 1              | 1             | 1              | 0             | 0              | 0             | 0              | 0             | 0              | 0             | 0              | 0             | 0              | 0             | 0              | -1            | -1             | -1            | -1             |
| Ry     | 1             | 1              | 1             | 1              | 1             | 1              | 1             | 1              | 0             | 0              | 0             | 0              | 0             | 0              | 0             | 0              | 0             | 0              | 0             | 0              | -1            | -1             | -1            | -1             |
| R      | 1             | 1              | 1             | 1              | -1            | -1             | -1            | -1             | $i$           | $i$            | $i$           | $i$            | $i$           | $i$            | $-i$          | $-i$           | $-i$          | $-i$           | $-i$          | $-i$           | 1             | 1              | -1            | -1             |
| Landau | A1            | A1             | A1            | A1             | B1            | B1             | B1            | B1             | E             | E              | E             | E              | E             | E              | E             | E              | E             | E              | E             | E              | A2            | A2             | B2            | B2             |



$$\mathbf{S} = \mathbf{1}/2, \mathbf{n}_{\text{occ.}} = \{\mathbf{1}, \mathbf{0}, \mathbf{1}, \mathbf{0}, \mathbf{2}\}$$

| State  | 855           | 856            | 857           | 858            | 859           | 860            | 861           | 862            | 863           | 864            | 865           | 866            | 867           | 868            | 869           | 870            | 871           | 872            | 873           | 874            | 875           | 876            | 877           | 878            |
|--------|---------------|----------------|---------------|----------------|---------------|----------------|---------------|----------------|---------------|----------------|---------------|----------------|---------------|----------------|---------------|----------------|---------------|----------------|---------------|----------------|---------------|----------------|---------------|----------------|
| Sz     | $\frac{1}{2}$ | $-\frac{1}{2}$ | $\frac{1}{2}$ | $-\frac{1}{2}$ | $\frac{1}{2}$ | $-\frac{1}{2}$ | $\frac{1}{2}$ | $-\frac{1}{2}$ | $\frac{1}{2}$ | $-\frac{1}{2}$ | $\frac{1}{2}$ | $-\frac{1}{2}$ | $\frac{1}{2}$ | $-\frac{1}{2}$ | $\frac{1}{2}$ | $-\frac{1}{2}$ | $\frac{1}{2}$ | $-\frac{1}{2}$ | $\frac{1}{2}$ | $-\frac{1}{2}$ | $\frac{1}{2}$ | $-\frac{1}{2}$ | $\frac{1}{2}$ | $-\frac{1}{2}$ |
| Rx     | 1             | 1              | 1             | 1              | 1             | 1              | 1             | 1              | 0             | 0              | 0             | 0              | 0             | 0              | 0             | 0              | 0             | 0              | 0             | 0              | -1            | -1             | -1            | -1             |
| Ry     | 1             | 1              | 1             | 1              | 1             | 1              | 1             | 1              | 0             | 0              | 0             | 0              | 0             | 0              | 0             | 0              | 0             | 0              | 0             | 0              | -1            | -1             | -1            | -1             |
| R      | 1             | 1              | 1             | 1              | -1            | -1             | -1            | -1             | $i$           | $i$            | $i$           | $i$            | $i$           | $i$            | $-i$          | $-i$           | $-i$          | $-i$           | $-i$          | $-i$           | 1             | 1              | -1            | -1             |
| Landau | A1            | A1             | A1            | A1             | B1            | B1             | B1            | B1             | E             | E              | E             | E              | E             | E              | E             | E              | E             | E              | E             | E              | A2            | A2             | B2            | B2             |

$$\mathbf{S} = \mathbf{1}/\mathbf{2}, \mathbf{n}_{\text{occ.}} = \{\mathbf{1}, \mathbf{0}, \mathbf{0}, \mathbf{3}, \mathbf{0}\}$$

| State  | 879           | 880            | 881           | 882            | 883           | 884            | 885           | 886            |
|--------|---------------|----------------|---------------|----------------|---------------|----------------|---------------|----------------|
| Sz     | $\frac{1}{2}$ | $-\frac{1}{2}$ | $\frac{1}{2}$ | $-\frac{1}{2}$ | $\frac{1}{2}$ | $-\frac{1}{2}$ | $\frac{1}{2}$ | $-\frac{1}{2}$ |
| Rx     | 1             | 1              | 1             | 1              | 0             | 0              | 0             | 0              |
| Ry     | 1             | 1              | 1             | 1              | 0             | 0              | 0             | 0              |
| R      | 1             | 1              | -1            | -1             | $i$           | $i$            | $-i$          | $-i$           |
| Landau | A1            | A1             | B1            | B1             | E             | E              | E             | E              |

$$\mathbf{S} = \mathbf{1}/2, \mathbf{n}_{\text{occ.}} = \{1, 0, 0, 2, 1\}$$

| State  | 887           | 888            | 889           | 890            | 891           | 892            | 893           | 894            | 895           | 896            | 897           | 898            | 899           | 900            | 901           | 902            | 903           | 904            | 905           | 906            | 907           | 908            | 909           | 910            |
|--------|---------------|----------------|---------------|----------------|---------------|----------------|---------------|----------------|---------------|----------------|---------------|----------------|---------------|----------------|---------------|----------------|---------------|----------------|---------------|----------------|---------------|----------------|---------------|----------------|
| Sz     | $\frac{1}{2}$ | $-\frac{1}{2}$ | $\frac{1}{2}$ | $-\frac{1}{2}$ | $\frac{1}{2}$ | $-\frac{1}{2}$ | $\frac{1}{2}$ | $-\frac{1}{2}$ | $\frac{1}{2}$ | $-\frac{1}{2}$ | $\frac{1}{2}$ | $-\frac{1}{2}$ | $\frac{1}{2}$ | $-\frac{1}{2}$ | $\frac{1}{2}$ | $-\frac{1}{2}$ | $\frac{1}{2}$ | $-\frac{1}{2}$ | $\frac{1}{2}$ | $-\frac{1}{2}$ | $\frac{1}{2}$ | $-\frac{1}{2}$ | $\frac{1}{2}$ | $-\frac{1}{2}$ |
| Rx     | 1             | 1              | 1             | 1              | 1             | 1              | 1             | 1              | 0             | 0              | 0             | 0              | 0             | 0              | 0             | 0              | 0             | 0              | 0             | 0              | -1            | -1             | -1            | -1             |
| Ry     | 1             | 1              | 1             | 1              | 1             | 1              | 1             | 1              | 0             | 0              | 0             | 0              | 0             | 0              | 0             | 0              | 0             | 0              | 0             | 0              | -1            | -1             | -1            | -1             |
| R      | 1             | 1              | 1             | 1              | -1            | -1             | -1            | -1             | $i$           | $i$            | $i$           | $i$            | $i$           | $i$            | $-i$          | $-i$           | $-i$          | $-i$           | $-i$          | $-i$           | 1             | 1              | -1            | -1             |
| Landau | A1            | A1             | A1            | A1             | B1            | B1             | B1            | B1             | E             | E              | E             | E              | E             | E              | E             | E              | E             | E              | E             | E              | A2            | A2             | B2            | B2             |

$$\mathbf{S} = \mathbf{1}/2, \mathbf{n}_{\text{occ.}} = \{\mathbf{1}, \mathbf{0}, \mathbf{0}, \mathbf{1}, \mathbf{2}\}$$

| State  | 911           | 912            | 913           | 914            | 915           | 916            | 917           | 918            | 919           | 920            | 921           | 922            | 923           | 924            | 925           | 926            | 927           | 928            | 929           | 930            | 931           | 932            | 933           | 934            |
|--------|---------------|----------------|---------------|----------------|---------------|----------------|---------------|----------------|---------------|----------------|---------------|----------------|---------------|----------------|---------------|----------------|---------------|----------------|---------------|----------------|---------------|----------------|---------------|----------------|
| Sz     | $\frac{1}{2}$ | $-\frac{1}{2}$ | $\frac{1}{2}$ | $-\frac{1}{2}$ | $\frac{1}{2}$ | $-\frac{1}{2}$ | $\frac{1}{2}$ | $-\frac{1}{2}$ | $\frac{1}{2}$ | $-\frac{1}{2}$ | $\frac{1}{2}$ | $-\frac{1}{2}$ | $\frac{1}{2}$ | $-\frac{1}{2}$ | $\frac{1}{2}$ | $-\frac{1}{2}$ | $\frac{1}{2}$ | $-\frac{1}{2}$ | $\frac{1}{2}$ | $-\frac{1}{2}$ | $\frac{1}{2}$ | $-\frac{1}{2}$ | $\frac{1}{2}$ | $-\frac{1}{2}$ |
| Rx     | 1             | 1              | 1             | 1              | 1             | 1              | 1             | 1              | 0             | 0              | 0             | 0              | 0             | 0              | 0             | 0              | 0             | 0              | 0             | 0              | -1            | -1             | -1            | -1             |
| Ry     | 1             | 1              | 1             | 1              | 1             | 1              | 1             | 1              | 0             | 0              | 0             | 0              | 0             | 0              | 0             | 0              | 0             | 0              | 0             | 0              | -1            | -1             | -1            | -1             |
| R      | 1             | 1              | 1             | 1              | -1            | -1             | -1            | -1             | $i$           | $i$            | $i$           | $i$            | $i$           | $i$            | $-i$          | $-i$           | $-i$          | $-i$           | $-i$          | $-i$           | 1             | 1              | -1            | -1             |
| Landau | A1            | A1             | A1            | A1             | B1            | B1             | B1            | B1             | E             | E              | E             | E              | E             | E              | E             | E              | E             | E              | E             | E              | A2            | A2             | B2            | B2             |

$$\mathbf{S} = \mathbf{1}/\mathbf{2}, \mathbf{n}_{\text{occ.}} = \{\mathbf{1}, \mathbf{0}, \mathbf{0}, \mathbf{0}, \mathbf{3}\}$$

$$\left( \begin{array}{c|cccccccc} \text{State} & 935 & 936 & 937 & 938 & 939 & 940 & 941 & 942 \\ \hline \text{Sz} & \frac{1}{2} & -\frac{1}{2} & \frac{1}{2} & -\frac{1}{2} & \frac{1}{2} & -\frac{1}{2} & \frac{1}{2} & -\frac{1}{2} \\ \text{Rx} & 1 & 1 & 1 & 1 & 0 & 0 & 0 & 0 \\ \text{Ry} & 1 & 1 & 1 & 1 & 0 & 0 & 0 & 0 \\ \text{R} & 1 & 1 & -1 & -1 & i & i & -i & -i \\ \text{Landau} & \text{A1} & \text{A1} & \text{B1} & \text{B1} & \text{E} & \text{E} & \text{E} & \text{E} \end{array} \right)$$

$$\mathbf{S} = \mathbf{0}, \mathbf{n}_{\text{occ.}} = \{4, 0, 0, 0, 0\}$$

$$\left( \begin{array}{ccc} \text{State} & 943 & 944 \\ \text{Sz} & 0 & 0 \\ \text{Rx} & 1 & -1 \\ \text{Ry} & 1 & -1 \\ \text{R} & 1 & -1 \\ \text{Landau} & \text{A1} & \text{B2} \end{array} \right)$$



$$\mathbf{S} = \mathbf{0}, \mathbf{n}_{\text{occ.}} = \{\mathbf{2}, \mathbf{2}, \mathbf{0}, \mathbf{0}, \mathbf{0}\}$$

$$\left( \begin{array}{ccccccccc} \text{State} & 945 & 946 & 947 & 948 & 949 & 950 \\ \text{Sz} & 0 & 0 & 0 & 0 & 0 & 0 \\ \text{Rx} & 1 & 0 & 0 & 0 & 0 & -1 \\ \text{Ry} & 1 & 0 & 0 & 0 & 0 & -1 \\ \text{R} & -1 & i & i & -i & -i & 1 \\ \text{Landau} & \text{B1} & \text{E} & \text{E} & \text{E} & \text{E} & \text{A2} \end{array} \right)$$

$$\mathbf{S} = \mathbf{0}, \mathbf{n}_{\text{occ.}} = \{\mathbf{2}, \mathbf{1}, \mathbf{1}, \mathbf{0}, \mathbf{0}\}$$

| State  | 951 | 952 | 953 | 954 | 955 | 956  | 957  | 958  | 959 | 960 | 961 | 962 |
|--------|-----|-----|-----|-----|-----|------|------|------|-----|-----|-----|-----|
| Sz     | 0   | 0   | 0   | 0   | 0   | 0    | 0    | 0    | 0   | 0   | 0   | 0   |
| Rx     | 1   | 1   | 0   | 0   | 0   | 0    | 0    | 0    | -1  | -1  | -1  | -1  |
| Ry     | 1   | 1   | 0   | 0   | 0   | 0    | 0    | 0    | -1  | -1  | -1  | -1  |
| R      | 1   | -1  | $i$ | $i$ | $i$ | $-i$ | $-i$ | $-i$ | 1   | 1   | -1  | -1  |
| Landau | A1  | B1  | E   | E   | E   | E    | E    | E    | A2  | A2  | B2  | B2  |

$$\mathbf{S} = \mathbf{0}, \mathbf{n}_{\text{occ.}} = \{\mathbf{2}, \mathbf{1}, \mathbf{0}, \mathbf{1}, \mathbf{0}\}$$

$$\left( \begin{array}{cccccccccccccccc} \text{State} & 963 & 964 & 965 & 966 & 967 & 968 & 969 & 970 & 971 & 972 & 973 & 974 \\ \text{Sz} & 0 & 0 & 0 & 0 & 0 & 0 & 0 & 0 & 0 & 0 & 0 & 0 \\ \text{Rx} & 1 & 1 & 0 & 0 & 0 & 0 & 0 & 0 & -1 & -1 & -1 & -1 \\ \text{Ry} & 1 & 1 & 0 & 0 & 0 & 0 & 0 & 0 & -1 & -1 & -1 & -1 \\ \text{R} & 1 & -1 & i & i & i & -i & -i & -i & 1 & 1 & -1 & -1 \\ \text{Landau} & \text{A1} & \text{B1} & \text{E} & \text{E} & \text{E} & \text{E} & \text{E} & \text{E} & \text{A2} & \text{A2} & \text{B2} & \text{B2} \end{array} \right)$$

$$\mathbf{S} = \mathbf{0}, \mathbf{n}_{\text{occ.}} = \{\mathbf{2}, \mathbf{1}, \mathbf{0}, \mathbf{0}, \mathbf{1}\}$$

| State  | 975 | 976 | 977 | 978 | 979 | 980  | 981  | 982  | 983 | 984 | 985 | 986 |
|--------|-----|-----|-----|-----|-----|------|------|------|-----|-----|-----|-----|
| Sz     | 0   | 0   | 0   | 0   | 0   | 0    | 0    | 0    | 0   | 0   | 0   | 0   |
| Rx     | 1   | 1   | 0   | 0   | 0   | 0    | 0    | 0    | -1  | -1  | -1  | -1  |
| Ry     | 1   | 1   | 0   | 0   | 0   | 0    | 0    | 0    | -1  | -1  | -1  | -1  |
| R      | 1   | -1  | $i$ | $i$ | $i$ | $-i$ | $-i$ | $-i$ | 1   | 1   | -1  | -1  |
| Landau | A1  | B1  | E   | E   | E   | E    | E    | E    | A2  | A2  | B2  | B2  |

$$\mathbf{S} = \mathbf{0}, \mathbf{n}_{\text{occ.}} = \{\mathbf{2}, \mathbf{0}, \mathbf{2}, \mathbf{0}, \mathbf{0}\}$$

$$\left( \begin{array}{cccccc} \text{State} & 987 & 988 & 989 & 990 & 991 & 992 \\ \text{Sz} & 0 & 0 & 0 & 0 & 0 & 0 \\ \text{Rx} & 1 & 0 & 0 & 0 & 0 & -1 \\ \text{Ry} & 1 & 0 & 0 & 0 & 0 & -1 \\ \text{R} & -1 & i & i & -i & -i & 1 \\ \text{Landau} & \text{B1} & \text{E} & \text{E} & \text{E} & \text{E} & \text{A2} \end{array} \right)$$



$$\mathbf{S} = \mathbf{0}, \mathbf{n}_{\text{occ.}} = \{\mathbf{2}, \mathbf{0}, \mathbf{1}, \mathbf{0}, \mathbf{1}\}$$

| State  | 1005 | 1006 | 1007 | 1008 | 1009 | 1010 | 1011 | 1012 | 1013 | 1014 | 1015 | 1016 |
|--------|------|------|------|------|------|------|------|------|------|------|------|------|
| Sz     | 0    | 0    | 0    | 0    | 0    | 0    | 0    | 0    | 0    | 0    | 0    | 0    |
| Rx     | 1    | 1    | 0    | 0    | 0    | 0    | 0    | 0    | -1   | -1   | -1   | -1   |
| Ry     | 1    | 1    | 0    | 0    | 0    | 0    | 0    | 0    | -1   | -1   | -1   | -1   |
| R      | 1    | -1   | $i$  | $i$  | $i$  | $-i$ | $-i$ | $-i$ | 1    | 1    | -1   | -1   |
| Landau | A1   | B1   | E    | E    | E    | E    | E    | E    | A2   | A2   | B2   | B2   |

$$\mathbf{S} = \mathbf{0}, \mathbf{n}_{\text{occ.}} = \{\mathbf{2}, \mathbf{0}, \mathbf{0}, \mathbf{2}, \mathbf{0}\}$$

$$\left( \begin{array}{cccccc} \text{State} & 1017 & 1018 & 1019 & 1020 & 1021 & 1022 \\ \text{Sz} & 0 & 0 & 0 & 0 & 0 & 0 \\ \text{Rx} & 1 & 0 & 0 & 0 & 0 & -1 \\ \text{Ry} & 1 & 0 & 0 & 0 & 0 & -1 \\ \text{R} & -1 & i & i & -i & -i & 1 \\ \text{Landau} & \text{B1} & \text{E} & \text{E} & \text{E} & \text{E} & \text{A2} \end{array} \right)$$





$$\mathbf{S} = \mathbf{0}, \mathbf{n}_{\text{occ.}} = \{\mathbf{2}, \mathbf{0}, \mathbf{0}, \mathbf{0}, \mathbf{2}\}$$

| State  | 1035 | 1036 | 1037 | 1038 | 1039 | 1040 |
|--------|------|------|------|------|------|------|
| Sz     | 0    | 0    | 0    | 0    | 0    | 0    |
| Rx     | 1    | 0    | 0    | 0    | 0    | -1   |
| Ry     | 1    | 0    | 0    | 0    | 0    | -1   |
| R      | -1   | $i$  | $i$  | $-i$ | $-i$ | 1    |
| Landau | B1   | E    | E    | E    | E    | A2   |

$$\mathbf{S} = \mathbf{0}, \text{ n}_{\text{occ.}} = \{0, 4, 0, 0, 0\}$$

$$\left( \begin{array}{cc} \text{State} & 1041 \\ \text{Sz} & 0 \\ \text{Rx} & 1 \\ \text{Ry} & 1 \\ \text{R} & 1 \\ \text{Landau} & \text{A1} \end{array} \right)$$

$$\mathbf{S} = \mathbf{0}, \text{ n}_{\text{occ.}} = \{0, 3, 1, 0, 0\}$$

$$\left( \begin{array}{ccccc} \text{State} & 1042 & 1043 & 1044 & 1045 \\ \text{Sz} & 0 & 0 & 0 & 0 \\ \text{Rx} & 1 & 1 & 0 & 0 \\ \text{Ry} & 1 & 1 & 0 & 0 \\ \text{R} & 1 & -1 & i & -i \\ \text{Landau} & \text{A1} & \text{B1} & \text{E} & \text{E} \end{array} \right)$$

$$\mathbf{S} = \mathbf{0}, \mathbf{n}_{\text{occ.}} = \{\mathbf{0}, \mathbf{3}, \mathbf{0}, \mathbf{1}, \mathbf{0}\}$$

$$\left( \begin{array}{ccccc} \text{State} & 1046 & 1047 & 1048 & 1049 \\ \text{Sz} & 0 & 0 & 0 & 0 \\ \text{Rx} & 1 & 1 & 0 & 0 \\ \text{Ry} & 1 & 1 & 0 & 0 \\ \text{R} & 1 & -1 & i & -i \\ \text{Landau} & \text{A1} & \text{B1} & \text{E} & \text{E} \end{array} \right)$$

$$\mathbf{S} = \mathbf{0}, \mathbf{n}_{\text{occ.}} = \{\mathbf{0}, \mathbf{3}, \mathbf{0}, \mathbf{0}, \mathbf{1}\}$$

$$\left( \begin{array}{ccccc} \text{State} & 1050 & 1051 & 1052 & 1053 \\ \text{Sz} & 0 & 0 & 0 & 0 \\ \text{Rx} & 1 & 1 & 0 & 0 \\ \text{Ry} & 1 & 1 & 0 & 0 \\ \text{R} & 1 & -1 & i & -i \\ \text{Landau} & \text{A1} & \text{B1} & \text{E} & \text{E} \end{array} \right)$$

$$\mathbf{S} = \mathbf{0}, \mathbf{n}_{\text{occ.}} = \{\mathbf{0}, \mathbf{2}, \mathbf{2}, \mathbf{0}, \mathbf{0}\}$$

| State  | 1054 | 1055 | 1056 | 1057 | 1058 | 1059 |
|--------|------|------|------|------|------|------|
| Sz     | 0    | 0    | 0    | 0    | 0    | 0    |
| Rx     | 1    | 1    | 1    | 0    | 0    | -1   |
| Ry     | 1    | 1    | 1    | 0    | 0    | -1   |
| R      | 1    | 1    | -1   | $i$  | $-i$ | -1   |
| Landau | A1   | A1   | B1   | E    | E    | B2   |

$$\mathbf{S} = \mathbf{0}, \mathbf{n}_{\text{occ.}} = \{\mathbf{0}, \mathbf{2}, \mathbf{1}, \mathbf{1}, \mathbf{0}\}$$

| State  | 1060 | 1061 | 1062 | 1063 | 1064 | 1065 | 1066 | 1067 | 1068 | 1069 | 1070 | 1071 |
|--------|------|------|------|------|------|------|------|------|------|------|------|------|
| Sz     | 0    | 0    | 0    | 0    | 0    | 0    | 0    | 0    | 0    | 0    | 0    | 0    |
| Rx     | 1    | 1    | 1    | 1    | 0    | 0    | 0    | 0    | 0    | 0    | -1   | -1   |
| Ry     | 1    | 1    | 1    | 1    | 0    | 0    | 0    | 0    | 0    | 0    | -1   | -1   |
| R      | 1    | 1    | -1   | -1   | $i$  | $i$  | $i$  | $-i$ | $-i$ | $-i$ | 1    | -1   |
| Landau | A1   | A1   | B1   | B1   | E    | E    | E    | E    | E    | E    | A2   | B2   |



$$\mathbf{S} = \mathbf{0}, \mathbf{n}_{\text{occ.}} = \{\mathbf{0}, \mathbf{2}, \mathbf{1}, \mathbf{0}, \mathbf{1}\}$$

| State  | 1072 | 1073 | 1074 | 1075 | 1076 | 1077 | 1078 | 1079 | 1080 | 1081 | 1082 | 1083 |
|--------|------|------|------|------|------|------|------|------|------|------|------|------|
| Sz     | 0    | 0    | 0    | 0    | 0    | 0    | 0    | 0    | 0    | 0    | 0    | 0    |
| Rx     | 1    | 1    | 1    | 1    | 0    | 0    | 0    | 0    | 0    | 0    | -1   | -1   |
| Ry     | 1    | 1    | 1    | 1    | 0    | 0    | 0    | 0    | 0    | 0    | -1   | -1   |
| R      | 1    | 1    | -1   | -1   | $i$  | $i$  | $i$  | $-i$ | $-i$ | $-i$ | 1    | -1   |
| Landau | A1   | A1   | B1   | B1   | E    | E    | E    | E    | E    | E    | A2   | B2   |

$$\mathbf{S} = \mathbf{0}, \mathbf{n}_{\text{occ.}} = \{\mathbf{0}, \mathbf{2}, \mathbf{0}, \mathbf{2}, \mathbf{0}\}$$

| State  | 1084 | 1085 | 1086 | 1087 | 1088 | 1089 |
|--------|------|------|------|------|------|------|
| Sz     | 0    | 0    | 0    | 0    | 0    | 0    |
| Rx     | 1    | 1    | 1    | 0    | 0    | -1   |
| Ry     | 1    | 1    | 1    | 0    | 0    | -1   |
| R      | 1    | 1    | -1   | $i$  | $-i$ | -1   |
| Landau | A1   | A1   | B1   | E    | E    | B2   |

$$\mathbf{S} = \mathbf{0}, \mathbf{n}_{\text{occ.}} = \{\mathbf{0}, \mathbf{2}, \mathbf{0}, \mathbf{1}, \mathbf{1}\}$$

| State  | 1090 | 1091 | 1092 | 1093 | 1094 | 1095 | 1096 | 1097 | 1098 | 1099 | 1100 | 1101 |
|--------|------|------|------|------|------|------|------|------|------|------|------|------|
| Sz     | 0    | 0    | 0    | 0    | 0    | 0    | 0    | 0    | 0    | 0    | 0    | 0    |
| Rx     | 1    | 1    | 1    | 1    | 0    | 0    | 0    | 0    | 0    | 0    | -1   | -1   |
| Ry     | 1    | 1    | 1    | 1    | 0    | 0    | 0    | 0    | 0    | 0    | -1   | -1   |
| R      | 1    | 1    | -1   | -1   | $i$  | $i$  | $i$  | $-i$ | $-i$ | $-i$ | 1    | -1   |
| Landau | A1   | A1   | B1   | B1   | E    | E    | E    | E    | E    | E    | A2   | B2   |

$$\mathbf{S} = \mathbf{0}, \mathbf{n}_{\text{occ.}} = \{\mathbf{0}, \mathbf{2}, \mathbf{0}, \mathbf{0}, \mathbf{2}\}$$

$$\left( \begin{array}{cccccc} \text{State} & 1102 & 1103 & 1104 & 1105 & 1106 & 1107 \\ \text{Sz} & 0 & 0 & 0 & 0 & 0 & 0 \\ \text{Rx} & 1 & 1 & 1 & 0 & 0 & -1 \\ \text{Ry} & 1 & 1 & 1 & 0 & 0 & -1 \\ \text{R} & 1 & 1 & -1 & i & -i & -1 \\ \text{Landau} & \text{A1} & \text{A1} & \text{B1} & \text{E} & \text{E} & \text{B2} \end{array} \right)$$

$$\mathbf{S} = \mathbf{0}, \mathbf{n}_{\text{occ.}} = \{0, 1, 3, 0, 0\}$$

$$\left( \begin{array}{ccccc} \text{State} & 1108 & 1109 & 1110 & 1111 \\ \text{Sz} & 0 & 0 & 0 & 0 \\ \text{Rx} & 1 & 1 & 0 & 0 \\ \text{Ry} & 1 & 1 & 0 & 0 \\ \text{R} & 1 & -1 & i & -i \\ \text{Landau} & \text{A1} & \text{B1} & \text{E} & \text{E} \end{array} \right)$$

$$\mathbf{S} = \mathbf{0}, \mathbf{n}_{\text{occ.}} = \{\mathbf{0}, \mathbf{1}, \mathbf{2}, \mathbf{1}, \mathbf{0}\}$$

| State  | 1112 | 1113 | 1114 | 1115 | 1116 | 1117 | 1118 | 1119 | 1120 | 1121 | 1122 | 1123 |
|--------|------|------|------|------|------|------|------|------|------|------|------|------|
| Sz     | 0    | 0    | 0    | 0    | 0    | 0    | 0    | 0    | 0    | 0    | 0    | 0    |
| Rx     | 1    | 1    | 1    | 1    | 0    | 0    | 0    | 0    | 0    | 0    | -1   | -1   |
| Ry     | 1    | 1    | 1    | 1    | 0    | 0    | 0    | 0    | 0    | 0    | -1   | -1   |
| R      | 1    | 1    | -1   | -1   | $i$  | $i$  | $i$  | $-i$ | $-i$ | $-i$ | 1    | -1   |
| Landau | A1   | A1   | B1   | B1   | E    | E    | E    | E    | E    | E    | A2   | B2   |

$$\mathbf{S} = \mathbf{0}, \mathbf{n}_{\text{occ.}} = \{0, 1, 2, 0, 1\}$$

| State  | 1124 | 1125 | 1126 | 1127 | 1128 | 1129 | 1130 | 1131 | 1132 | 1133 | 1134 | 1135 |
|--------|------|------|------|------|------|------|------|------|------|------|------|------|
| Sz     | 0    | 0    | 0    | 0    | 0    | 0    | 0    | 0    | 0    | 0    | 0    | 0    |
| Rx     | 1    | 1    | 1    | 1    | 0    | 0    | 0    | 0    | 0    | 0    | -1   | -1   |
| Ry     | 1    | 1    | 1    | 1    | 0    | 0    | 0    | 0    | 0    | 0    | -1   | -1   |
| R      | 1    | 1    | -1   | -1   | $i$  | $i$  | $i$  | $-i$ | $-i$ | $-i$ | 1    | -1   |
| Landau | A1   | A1   | B1   | B1   | E    | E    | E    | E    | E    | E    | A2   | B2   |

$$\mathbf{S} = \mathbf{0}, \mathbf{n}_{\text{occ.}} = \{0, 1, 1, 2, 0\}$$

| State  | 1136 | 1137 | 1138 | 1139 | 1140 | 1141 | 1142 | 1143 | 1144 | 1145 | 1146 | 1147 |
|--------|------|------|------|------|------|------|------|------|------|------|------|------|
| Sz     | 0    | 0    | 0    | 0    | 0    | 0    | 0    | 0    | 0    | 0    | 0    | 0    |
| Rx     | 1    | 1    | 1    | 1    | 0    | 0    | 0    | 0    | 0    | 0    | -1   | -1   |
| Ry     | 1    | 1    | 1    | 1    | 0    | 0    | 0    | 0    | 0    | 0    | -1   | -1   |
| R      | 1    | 1    | -1   | -1   | $i$  | $i$  | $i$  | $-i$ | $-i$ | $-i$ | 1    | -1   |
| Landau | A1   | A1   | B1   | B1   | E    | E    | E    | E    | E    | E    | A2   | B2   |



$$\mathbf{S} = \mathbf{0}, \mathbf{n}_{\text{occ.}} = \{0, 1, 1, 1, 1\}$$

| State  | 1148 | 1149 | 1150 | 1151 | 1152 | 1153 | 1154 | 1155 | 1156 | 1157 | 1158 | 1159 | 1160 | 1161 | 1162 | 1163 | 1164 | 1165 | 1166 | 1167 | 1168 | 1169 | 1170 | 1171 |
|--------|------|------|------|------|------|------|------|------|------|------|------|------|------|------|------|------|------|------|------|------|------|------|------|------|
| Sz     | 0    | 0    | 0    | 0    | 0    | 0    | 0    | 0    | 0    | 0    | 0    | 0    | 0    | 0    | 0    | 0    | 0    | 0    | 0    | 0    | 0    | 0    | 0    | 0    |
| Rx     | 1    | 1    | 1    | 1    | 1    | 1    | 0    | 0    | 0    | 0    | 0    | 0    | 0    | 0    | 0    | 0    | 0    | 0    | -1   | -1   | -1   | -1   | -1   | -1   |
| Ry     | 1    | 1    | 1    | 1    | 1    | 1    | 0    | 0    | 0    | 0    | 0    | 0    | 0    | 0    | 0    | 0    | 0    | 0    | -1   | -1   | -1   | -1   | -1   | -1   |
| R      | 1    | 1    | 1    | -1   | -1   | -1   | $i$  | $i$  | $i$  | $i$  | $i$  | $i$  | $i$  | $-i$ | $-i$ | $-i$ | $-i$ | $-i$ | 1    | 1    | 1    | -1   | -1   | -1   |
| Landau | A1   | A1   | A1   | B1   | B1   | B1   | E    | E    | E    | E    | E    | E    | E    | E    | E    | E    | E    | E    | A2   | A2   | A2   | B2   | B2   | B2   |

$$\mathbf{S} = \mathbf{0}, \mathbf{n}_{\text{occ.}} = \{\mathbf{0}, \mathbf{1}, \mathbf{1}, \mathbf{0}, \mathbf{2}\}$$

| State  | 1172 | 1173 | 1174 | 1175 | 1176 | 1177 | 1178 | 1179 | 1180 | 1181 | 1182 | 1183 |
|--------|------|------|------|------|------|------|------|------|------|------|------|------|
| Sz     | 0    | 0    | 0    | 0    | 0    | 0    | 0    | 0    | 0    | 0    | 0    | 0    |
| Rx     | 1    | 1    | 1    | 1    | 0    | 0    | 0    | 0    | 0    | 0    | -1   | -1   |
| Ry     | 1    | 1    | 1    | 1    | 0    | 0    | 0    | 0    | 0    | 0    | -1   | -1   |
| R      | 1    | 1    | -1   | -1   | $i$  | $i$  | $i$  | $-i$ | $-i$ | $-i$ | 1    | -1   |
| Landau | A1   | A1   | B1   | B1   | E    | E    | E    | E    | E    | E    | A2   | B2   |

$$\mathbf{S} = \mathbf{0}, \mathbf{n}_{\text{occ.}} = \{0, 1, 0, 3, 0\}$$

$$\left( \begin{array}{ccccc} \text{State} & 1184 & 1185 & 1186 & 1187 \\ \text{Sz} & 0 & 0 & 0 & 0 \\ \text{Rx} & 1 & 1 & 0 & 0 \\ \text{Ry} & 1 & 1 & 0 & 0 \\ \text{R} & 1 & -1 & i & -i \\ \text{Landau} & \text{A1} & \text{B1} & \text{E} & \text{E} \end{array} \right)$$

$$\mathbf{S} = \mathbf{0}, \mathbf{n}_{\text{occ.}} = \{\mathbf{0}, \mathbf{1}, \mathbf{0}, \mathbf{2}, \mathbf{1}\}$$

| State  | 1188 | 1189 | 1190 | 1191 | 1192 | 1193 | 1194 | 1195 | 1196 | 1197 | 1198 | 1199 |
|--------|------|------|------|------|------|------|------|------|------|------|------|------|
| Sz     | 0    | 0    | 0    | 0    | 0    | 0    | 0    | 0    | 0    | 0    | 0    | 0    |
| Rx     | 1    | 1    | 1    | 1    | 0    | 0    | 0    | 0    | 0    | 0    | -1   | -1   |
| Ry     | 1    | 1    | 1    | 1    | 0    | 0    | 0    | 0    | 0    | 0    | -1   | -1   |
| R      | 1    | 1    | -1   | -1   | $i$  | $i$  | $i$  | $-i$ | $-i$ | $-i$ | 1    | -1   |
| Landau | A1   | A1   | B1   | B1   | E    | E    | E    | E    | E    | E    | A2   | B2   |

$$\mathbf{S} = \mathbf{0}, \mathbf{n}_{\text{occ.}} = \{\mathbf{0}, \mathbf{1}, \mathbf{0}, \mathbf{1}, \mathbf{2}\}$$

| State  | 1200 | 1201 | 1202 | 1203 | 1204 | 1205 | 1206 | 1207 | 1208 | 1209 | 1210 | 1211 |
|--------|------|------|------|------|------|------|------|------|------|------|------|------|
| Sz     | 0    | 0    | 0    | 0    | 0    | 0    | 0    | 0    | 0    | 0    | 0    | 0    |
| Rx     | 1    | 1    | 1    | 1    | 0    | 0    | 0    | 0    | 0    | 0    | -1   | -1   |
| Ry     | 1    | 1    | 1    | 1    | 0    | 0    | 0    | 0    | 0    | 0    | -1   | -1   |
| R      | 1    | 1    | -1   | -1   | $i$  | $i$  | $i$  | $-i$ | $-i$ | $-i$ | 1    | -1   |
| Landau | A1   | A1   | B1   | B1   | E    | E    | E    | E    | E    | E    | A2   | B2   |

$$\mathbf{S} = \mathbf{0}, \mathbf{n}_{\text{occ.}} = \{\mathbf{0}, \mathbf{1}, \mathbf{0}, \mathbf{0}, \mathbf{3}\}$$

$$\left( \begin{array}{ccccc} \text{State} & 1212 & 1213 & 1214 & 1215 \\ \text{Sz} & 0 & 0 & 0 & 0 \\ \text{Rx} & 1 & 1 & 0 & 0 \\ \text{Ry} & 1 & 1 & 0 & 0 \\ \text{R} & 1 & -1 & i & -i \\ \text{Landau} & \text{A1} & \text{B1} & \text{E} & \text{E} \end{array} \right)$$

$$\mathbf{S} = \mathbf{0}, \text{ n}_{\text{occ.}} = \{0, 0, 4, 0, 0\}$$

$$\left( \begin{array}{cc} \text{State} & 1216 \\ \text{Sz} & 0 \\ \text{Rx} & 1 \\ \text{Ry} & 1 \\ \text{R} & 1 \\ \text{Landau} & \text{A1} \end{array} \right)$$

$$\mathbf{S} = \mathbf{0}, \mathbf{n}_{\text{occ.}} = \{\mathbf{0}, \mathbf{0}, \mathbf{3}, \mathbf{1}, \mathbf{0}\}$$

$$\left( \begin{array}{ccccc} \text{State} & 1217 & 1218 & 1219 & 1220 \\ \text{Sz} & 0 & 0 & 0 & 0 \\ \text{Rx} & 1 & 1 & 0 & 0 \\ \text{Ry} & 1 & 1 & 0 & 0 \\ \text{R} & 1 & -1 & i & -i \\ \text{Landau} & \text{A1} & \text{B1} & \text{E} & \text{E} \end{array} \right)$$



$$\mathbf{S} = \mathbf{0}, \mathbf{n}_{\text{occ.}} = \{0, 0, 3, 0, 1\}$$

$$\left( \begin{array}{ccccc} \text{State} & 1221 & 1222 & 1223 & 1224 \\ \text{Sz} & 0 & 0 & 0 & 0 \\ \text{Rx} & 1 & 1 & 0 & 0 \\ \text{Ry} & 1 & 1 & 0 & 0 \\ \text{R} & 1 & -1 & i & -i \\ \text{Landau} & \text{A1} & \text{B1} & \text{E} & \text{E} \end{array} \right)$$

$$\mathbf{S} = \mathbf{0}, \mathbf{n}_{\text{occ.}} = \{\mathbf{0}, \mathbf{0}, \mathbf{2}, \mathbf{2}, \mathbf{0}\}$$

| State  | 1225 | 1226 | 1227 | 1228 | 1229 | 1230 |
|--------|------|------|------|------|------|------|
| Sz     | 0    | 0    | 0    | 0    | 0    | 0    |
| Rx     | 1    | 1    | 1    | 0    | 0    | -1   |
| Ry     | 1    | 1    | 1    | 0    | 0    | -1   |
| R      | 1    | 1    | -1   | $i$  | $-i$ | -1   |
| Landau | A1   | A1   | B1   | E    | E    | B2   |

$$\mathbf{S} = \mathbf{0}, \mathbf{n}_{\text{occ.}} = \{\mathbf{0}, \mathbf{0}, \mathbf{2}, \mathbf{1}, \mathbf{1}\}$$

| State  | 1231 | 1232 | 1233 | 1234 | 1235 | 1236 | 1237 | 1238 | 1239 | 1240 | 1241 | 1242 |
|--------|------|------|------|------|------|------|------|------|------|------|------|------|
| Sz     | 0    | 0    | 0    | 0    | 0    | 0    | 0    | 0    | 0    | 0    | 0    | 0    |
| Rx     | 1    | 1    | 1    | 1    | 0    | 0    | 0    | 0    | 0    | 0    | -1   | -1   |
| Ry     | 1    | 1    | 1    | 1    | 0    | 0    | 0    | 0    | 0    | 0    | -1   | -1   |
| R      | 1    | 1    | -1   | -1   | $i$  | $i$  | $i$  | $-i$ | $-i$ | $-i$ | 1    | -1   |
| Landau | A1   | A1   | B1   | B1   | E    | E    | E    | E    | E    | E    | A2   | B2   |

$$\mathbf{S} = \mathbf{0}, \mathbf{n}_{\text{occ.}} = \{\mathbf{0}, \mathbf{0}, \mathbf{2}, \mathbf{0}, \mathbf{2}\}$$

| State  | 1243 | 1244 | 1245 | 1246 | 1247 | 1248 |
|--------|------|------|------|------|------|------|
| Sz     | 0    | 0    | 0    | 0    | 0    | 0    |
| Rx     | 1    | 1    | 1    | 0    | 0    | -1   |
| Ry     | 1    | 1    | 1    | 0    | 0    | -1   |
| R      | 1    | 1    | -1   | $i$  | $-i$ | -1   |
| Landau | A1   | A1   | B1   | E    | E    | B2   |

$$\mathbf{S} = \mathbf{0}, \mathbf{n}_{\text{occ.}} = \{0, 0, 1, 3, 0\}$$

$$\left( \begin{array}{ccccc} \text{State} & 1249 & 1250 & 1251 & 1252 \\ \text{Sz} & 0 & 0 & 0 & 0 \\ \text{Rx} & 1 & 1 & 0 & 0 \\ \text{Ry} & 1 & 1 & 0 & 0 \\ \text{R} & 1 & -1 & i & -i \\ \text{Landau} & \text{A1} & \text{B1} & \text{E} & \text{E} \end{array} \right)$$

$$\mathbf{S} = \mathbf{0}, \mathbf{n}_{\text{occ.}} = \{0, 0, 1, 2, 1\}$$

| State  | 1253 | 1254 | 1255 | 1256 | 1257 | 1258 | 1259 | 1260 | 1261 | 1262 | 1263 | 1264 |
|--------|------|------|------|------|------|------|------|------|------|------|------|------|
| Sz     | 0    | 0    | 0    | 0    | 0    | 0    | 0    | 0    | 0    | 0    | 0    | 0    |
| Rx     | 1    | 1    | 1    | 1    | 0    | 0    | 0    | 0    | 0    | 0    | -1   | -1   |
| Ry     | 1    | 1    | 1    | 1    | 0    | 0    | 0    | 0    | 0    | 0    | -1   | -1   |
| R      | 1    | 1    | -1   | -1   | $i$  | $i$  | $i$  | $-i$ | $-i$ | $-i$ | 1    | -1   |
| Landau | A1   | A1   | B1   | B1   | E    | E    | E    | E    | E    | E    | A2   | B2   |

$$\mathbf{S} = \mathbf{0}, \mathbf{n}_{\text{occ.}} = \{\mathbf{0}, \mathbf{0}, \mathbf{1}, \mathbf{1}, \mathbf{2}\}$$

| State  | 1265 | 1266 | 1267 | 1268 | 1269 | 1270 | 1271 | 1272 | 1273 | 1274 | 1275 | 1276 |
|--------|------|------|------|------|------|------|------|------|------|------|------|------|
| Sz     | 0    | 0    | 0    | 0    | 0    | 0    | 0    | 0    | 0    | 0    | 0    | 0    |
| Rx     | 1    | 1    | 1    | 1    | 0    | 0    | 0    | 0    | 0    | 0    | -1   | -1   |
| Ry     | 1    | 1    | 1    | 1    | 0    | 0    | 0    | 0    | 0    | 0    | -1   | -1   |
| R      | 1    | 1    | -1   | -1   | $i$  | $i$  | $i$  | $-i$ | $-i$ | $-i$ | 1    | -1   |
| Landau | A1   | A1   | B1   | B1   | E    | E    | E    | E    | E    | E    | A2   | B2   |

$$\mathbf{S} = \mathbf{0}, \mathbf{n}_{\text{occ.}} = \{\mathbf{0}, \mathbf{0}, \mathbf{1}, \mathbf{0}, \mathbf{3}\}$$

$$\left( \begin{array}{ccccc} \text{State} & 1277 & 1278 & 1279 & 1280 \\ \text{Sz} & 0 & 0 & 0 & 0 \\ \text{Rx} & 1 & 1 & 0 & 0 \\ \text{Ry} & 1 & 1 & 0 & 0 \\ \text{R} & 1 & -1 & i & -i \\ \text{Landau} & \text{A1} & \text{B1} & \text{E} & \text{E} \end{array} \right)$$



$$\mathbf{S} = \mathbf{0}, \mathbf{n}_{\text{occ.}} = \{\mathbf{0}, \mathbf{0}, \mathbf{0}, 4, \mathbf{0}\}$$

$$\left( \begin{array}{cc} \text{State} & 1281 \\ \text{Sz} & 0 \\ \text{Rx} & 1 \\ \text{Ry} & 1 \\ \text{R} & 1 \\ \text{Landau} & \text{A1} \end{array} \right)$$

$$\mathbf{S} = \mathbf{0}, \mathbf{n}_{\text{occ.}} = \{0, 0, 0, 3, 1\}$$

$$\left( \begin{array}{ccccc} \text{State} & 1282 & 1283 & 1284 & 1285 \\ \text{Sz} & 0 & 0 & 0 & 0 \\ \text{Rx} & 1 & 1 & 0 & 0 \\ \text{Ry} & 1 & 1 & 0 & 0 \\ \text{R} & 1 & -1 & i & -i \\ \text{Landau} & \text{A1} & \text{B1} & \text{E} & \text{E} \end{array} \right)$$

$$\mathbf{S} = \mathbf{0}, \mathbf{n}_{\text{occ.}} = \{\mathbf{0}, \mathbf{0}, \mathbf{0}, \mathbf{2}, \mathbf{2}\}$$

| State  | 1286 | 1287 | 1288 | 1289 | 1290 | 1291 |
|--------|------|------|------|------|------|------|
| Sz     | 0    | 0    | 0    | 0    | 0    | 0    |
| Rx     | 1    | 1    | 1    | 0    | 0    | -1   |
| Ry     | 1    | 1    | 1    | 0    | 0    | -1   |
| R      | 1    | 1    | -1   | $i$  | $-i$ | -1   |
| Landau | A1   | A1   | B1   | E    | E    | B2   |

$$\mathbf{S} = \mathbf{0}, \mathbf{n}_{\text{occ.}} = \{0, 0, 0, 1, 3\}$$

$$\left( \begin{array}{ccccc} \text{State} & 1292 & 1293 & 1294 & 1295 \\ \text{Sz} & 0 & 0 & 0 & 0 \\ \text{Rx} & 1 & 1 & 0 & 0 \\ \text{Ry} & 1 & 1 & 0 & 0 \\ \text{R} & 1 & -1 & i & -i \\ \text{Landau} & \text{A1} & \text{B1} & \text{E} & \text{E} \end{array} \right)$$

$$\mathbf{S} = \mathbf{0}, \mathbf{n}_{\text{occ.}} = \{\mathbf{0}, \mathbf{0}, \mathbf{0}, \mathbf{0}, 4\}$$

$$\left( \begin{array}{cc} \text{State} & 1296 \\ \text{Sz} & 0 \\ \text{Rx} & 1 \\ \text{Ry} & 1 \\ \text{R} & 1 \\ \text{Landau} & \text{A1} \end{array} \right)$$
